# Supplementary material for: Magnetic Dipole and Electric Quadrupole Transitions in the Trivalent Lanthanide Series: Calculated Emission Rates and Oscillator Strengths
Source: arXiv:1208.2642 ancillary file (2012-09-20)
Supplement: Supplementary file 1 [file CDodson_Supplementary_Information.pdf]

# Supplemental Material
# Magnetic Dipole and Electric Quadrupole Transitions in Trivalent Lanthanide Ions: Calculated Emission Rates and Oscillator Strengths

Christopher M. Dodson* and Rashid Zia†

*School of Engineering, Brown University, Providence, RI 02912 USA*

## Abstract

This supplemental material contains a complete tabulation of magnetic dipole (MD) and electric quadrupole (EQ) transitions between 300 and 1700 nm in trivalent lanthanide ions. The tables include the vacuum oscillator strengths ($P'_{md}$, $P'_{eq}$) for all ground state MD and EQ absorptions lines as well as the vacuum spontaneous emission rates ($A'_{md}$, $A'_{eq}$) for all MD and EQ emission lines in this wavelength range. Transitions are organized by their originating level. These levels are labelled according to their dominant $LS$ term(s). If no single $LS$ term has a fractional contribution of at least 50%, then the level is labelled by the two $LS$ terms with the greatest fractional contributions. (Note that $Ce^{3+}$ exhibits no transitions in the considered wavelength range, and therefore does not appear in the following tables.)

* Email: christopher_dodson@brown.edu

† Email: rashid_zia@brown.edu

**LIST OF TABLES**


S1 Magnetic Dipole Absorption Lines . . . . 3

S2 $Pr^{3+}$ Magnetic Dipole Emission Lines . . . . 4

S3 $Nd^{3+}$ Magnetic Dipole Emission Lines . . . . 5

S4 $Pm^{3+}$ Magnetic Dipole Emission Lines . . . . 7

S5 $Sm^{3+}$ Magnetic Dipole Emission Lines . . . . 12

S6 $Eu^{3+}$ Magnetic Dipole Emission Lines . . . . 19

S7 $Gd^{3+}$ Magnetic Dipole Emission Lines . . . . 21

S8 $Tb^{3+}$ Magnetic Dipole Emission Lines . . . . 22

S9 $Dy^{3+}$ Magnetic Dipole Emission Lines . . . . 24

S10 $Ho^{3+}$ Magnetic Dipole Emission Lines . . . . 28

S11 $Er^{3+}$ Magnetic Dipole Emission Lines . . . . 31

S12 $Tm^{3+}$ Magnetic Dipole Emission Lines . . . . 32

S13 $Yb^{3+}$ Magnetic Dipole Emission Lines . . . . 32

S14 Electric Quadrupole Absorption Lines . . . . 33

S15 $Pr^{3+}$ Electric Quadrupole Emission Lines . . . . 35

S16 $Nd^{3+}$ Electric Quadrupole Emission Lines . . . . 36

S17 $Pm^{3+}$ Electric Quadrupole Emission Lines . . . . 39

S18 $Sm^{3+}$ Electric Quadrupole Emission Lines . . . . 46

S19 $Eu^{3+}$ Electric Quadrupole Emission Lines . . . . 56

S20 $Gd^{3+}$ Electric Quadrupole Emission Lines . . . . 59

S21 $Tb^{3+}$ Electric Quadrupole Emission Lines . . . . 60

S22 $Dy^{3+}$ Electric Quadrupole Emission Lines . . . . 63

S23 $Ho^{3+}$ Electric Quadrupole Emission Lines . . . . 69

S24 $Er^{3+}$ Electric Quadrupole Emission Lines . . . . 73

S25 $Tm^{3+}$ Electric Quadrupole Emission Lines . . . . 74

S26 $Yb^{3+}$ Electric Quadrupole Emission Lines . . . . 75

TABLE S1: Magnetic dipole ground state absorption lines between 300 and 10000 nm.

| | $SLJ$ | $S'L'J'$ | E($cm^{-1}$) | $\lambda(nm)$ | $P'_{md}$ [a] |
|---|---|---|---|---|---|
| $Ce^{3+}$ | $^2F_{5/2}$ | $^2F_{7/2}$ | 2266 | 4414 | $5.24 \times 10^{-8}$ |
| $Pr^{3+}$ | $^3H_4$ | $^3H_5$ | 2092 | 4781 | $9.86 \times 10^{-8}$ |
| | | $^3F_3$ | 6290 | 1590 | $1.85 \times 10^{-10}$ |
| | | $^3F_4$ | 6720 | 1488 | $5.04 \times 10^{-9}$ |
| | | $^1G_4$ | 9734 | 1027 | $2.66 \times 10^{-9}$ |
| $Nd^{3+}$ | $^4I_{9/2}$ | $^4I_{11/2}$ | 1829 | 5468 | $1.37 \times 10^{-7}$ |
| | | $^2H_{9/2}$ | 12167 | 822 | $1.25 \times 10^{-8}$ |
| | | $^4F_{7/2}$ | 13277 | 753 | $3.76 \times 10^{-11}$ |
| | | $^4F_{9/2}$ | 14540 | 688 | $1.76 \times 10^{-9}$ |
| | | $^2H_{11/2}$ | 15445 | 647 | $1.16 \times 10^{-11}$ |
| | | $^2G_{7/2}$ | 16892 | 592 | $2.23 \times 10^{-10}$ |
| | | $^4G_{7/2}$ | 18925 | 528 | $8.44 \times 10^{-14}$ |
| | | $^4G_{9/2}$ | 19266 | 519 | $1.53 \times 10^{-10}$ |
| | | $^2G_{9/2}$ | 20810 | 481 | $8.17 \times 10^{-11}$ |
| | | $^4G_{11/2}$ | 21354 | 468 | $5.85 \times 10^{-12}$ |
| | | $^2I_{11/2}$ | 29454 | 340 | $4.52 \times 10^{-9}$ |
| | | $^4D_{7/2}$ | 30290 | 330 | $2.78 \times 10^{-18}$ |
| | | $^2H_{9/2}$ | 33253 | 301 | $3.78 \times 10^{-11}$ |
| $Pm^{3+}$ | $^5I_4$ | $^5I_5$ | 1462 | 6841 | $1.62 \times 10^{-7}$ |
| | | $^5F_3$ | 13466 | 743 | $9.96 \times 10^{-12}$ |
| | | $^5F_4$ | 14432 | 693 | $6.99 \times 10^{-10}$ |
| | | $^5F_5$ | 15793 | 633 | $2.86 \times 10^{-12}$ |
| | | $(^3H, {}^5G)_4$ | 17376 | 575 | $1.23 \times 10^{-8}$ |
| | | $^5G_3$ | 17896 | 559 | $1.84 \times 10^{-10}$ |
| | | $(^3H, {}^5G)_5$ | 19610 | 510 | $4.54 \times 10^{-11}$ |
| | | $^5G_4$ | 20038 | 499 | $4.6 \times 10^{-9}$ |
| | | $^3G_3$ | 21688 | 461 | $1.03 \times 10^{-10}$ |
| | | $^5G_5$ | 21885 | 457 | $3.84 \times 10^{-11}$ |
| | | $^3G_4$ | 24499 | 408 | $9.26 \times 10^{-10}$ |
| | | $^3D_3$ | 25695 | 389 | $2.21 \times 10^{-13}$ |
| | | $^3G_5$ | 27022 | 370 | $1.77 \times 10^{-10}$ |
| | | $^3F_4$ | 27046 | 370 | $3.42 \times 10^{-15}$ |
| | | $^3I_5$ | 28207 | 355 | $4.9 \times 10^{-9}$ |
| | | $^3F_3$ | 29121 | 343 | $5.2 \times 10^{-13}$ |
| | | $^5D_3$ | 31821 | 314 | $4.92 \times 10^{-14}$ |
| | | $^5D_4$ | 32302 | 310 | $5.52 \times 10^{-12}$ |
| | | $^3F_3$ | 32958 | 303 | $7.47 \times 10^{-16}$ |
| $Sm^{3+}$ | $^6H_{5/2}$ | $^6H_{7/2}$ | 1069 | 9355 | $1.81 \times 10^{-7}$ |
| | | $^6F_{3/2}$ | 6416 | 1559 | $2.5 \times 10^{-10}$ |
| | | $^6F_{5/2}$ | 6883 | 1453 | $1.06 \times 10^{-9}$ |
| | | $^6F_{7/2}$ | 7756 | 1289 | $3.43 \times 10^{-11}$ |
| | | $^4G_{5/2}$ | 18115 | 552 | $1.73 \times 10^{-8}$ |
| $Sm^{3+}$ | $^6H_{5/2}$ | $^4F_{3/2}$ | 18918 | 529 | $3.24 \times 10^{-10}$ |
| | | $^4G_{7/2}$ | 20172 | 496 | $1. \times 10^{-9}$ |
| | | $^4F_{5/2}$ | 22177 | 451 | $4.51 \times 10^{-9}$ |
| | | $(^6P, {}^4P)_{5/2}$ | 23849 | 419 | $4.08 \times 10^{-11}$ |
| | | $^6P_{3/2}$ | 24698 | 405 | $8.67 \times 10^{-13}$ |
| | | $^4F_{7/2}$ | 24889 | 402 | $1.72 \times 10^{-10}$ |
| | | $^6P_{7/2}$ | 26443 | 378 | $4.95 \times 10^{-12}$ |
| | | $^4D_{3/2}$ | 27403 | 365 | $4.36 \times 10^{-12}$ |
| | | $(^4D, {}^6P)_{5/2}$ | 27469 | 364 | $1.08 \times 10^{-12}$ |
| | | $^4H_{7/2}$ | 28715 | 348 | $4.14 \times 10^{-10}$ |
| | | $^4D_{7/2}$ | 28813 | 347 | $4.82 \times 10^{-13}$ |
| | | $^4G_{7/2}$ | 29992 | 333 | $6.23 \times 10^{-14}$ |
| | | $^4G_{5/2}$ | 30079 | 332 | $3.78 \times 10^{-10}$ |
| | | $^4P_{3/2}$ | 31340 | 319 | $6.22 \times 10^{-14}$ |
| | | $^4P_{5/2}$ | 32581 | 307 | $9.77 \times 10^{-13}$ |
| $Eu^{3+}$ | $^7F_0$ | $^5D_1$ | 19264 | 519 | $1.69 \times 10^{-8}$ |
| $Gd^{3+}$ | $^8S_{7/2}$ | $^6P_{7/2}$ | 32557 | 307 | $4.28 \times 10^{-8}$ |
| | | $^6P_{5/2}$ | 33169 | 301 | $2.42 \times 10^{-8}$ |
| $Tb^{3+}$ | $^7F_6$ | $^7F_5$ | 1999 | 5003 | $1.19 \times 10^{-7}$ |
| | | $^5G_6$ | 27004 | 370 | $5.01 \times 10^{-8}$ |
| | | $^5G_5$ | 28252 | 354 | $3.81 \times 10^{-9}$ |
| | | $^5L_7$ | 29678 | 337 | $4.8 \times 10^{-11}$ |
| | | $^5L_6$ | 30042 | 333 | $1.41 \times 10^{-9}$ |
| | | $^5H_7$ | 31843 | 314 | $4.84 \times 10^{-10}$ |
| | | $^5H_6$ | 33279 | 300 | $3.67 \times 10^{-9}$ |
| $Dy^{3+}$ | $^6H_{15/2}$ | $^6H_{13/2}$ | 3316 | 3016 | $2.17 \times 10^{-7}$ |
| | | $^4I_{15/2}$ | 22691 | 441 | $5.48 \times 10^{-8}$ |
| | | $^4K_{17/2}$ | 25967 | 385 | $9.58 \times 10^{-10}$ |
| | | $^4I_{13/2}$ | 26050 | 384 | $5.12 \times 10^{-9}$ |
| | | $^4M_{15/2}$ | 29534 | 339 | $6.13 \times 10^{-9}$ |
| | | $^4M_{17/2}$ | 29740 | 336 | $1.9 \times 10^{-10}$ |
| | | $^4K_{15/2}$ | 30846 | 324 | $2.25 \times 10^{-9}$ |
| | | $(^4K, {}^4L)_{13/2}$ | 33321 | 300 | $1.97 \times 10^{-9}$ |
| $Ho^{3+}$ | $^5I_8$ | $^5I_7$ | 5064 | 1975 | $2.97 \times 10^{-7}$ |
| | | $^3K_8$ | 20715 | 483 | $6.46 \times 10^{-8}$ |
| | | $^3K_7$ | 25636 | 390 | $2.81 \times 10^{-9}$ |
| | | $^3L_9$ | 28873 | 346 | $1.35 \times 10^{-9}$ |
| $Er^{3+}$ | $^4I_{15/2}$ | $^4I_{13/2}$ | 6543 | 1528 | $3.12 \times 10^{-7}$ |
| | | $^2K_{15/2}$ | 27315 | 366 | $3.66 \times 10^{-8}$ |
| | | $^2K_{13/2}$ | 32597 | 307 | $4.97 \times 10^{-10}$ |
| $Tm^{3+}$ | $^3H_6$ | $^3H_5$ | 8205 | 1219 | $2.74 \times 10^{-7}$ |
| $Yb^{3+}$ | $^2F_{7/2}$ | $^2F_{5/2}$ | 10248 | 976 | $1.78 \times 10^{-7}$ |

[a] The oscillator strength, $P_{md}$, inside a host material with refractive index $n_r$ would be: $P_{md} = P'_{md}\, n_r$

TABLE S2: Calculated $Pr^{3+}$ MD spontaneous emission lines between 300 and 1700 nm.

| $SLJ$ | $E_{SLJ}(cm^{-1})$ | $S'L'J'$ | $\lambda$ (nm) | $A'_{md}$ $(s^{-1})$ [a] | $SLJ$ | $E_{SLJ}(cm^{-1})$ | $S'L'J'$ | $\lambda$ (nm) | $A'_{md}$ $(s^{-1})$ [a] |
|---|---|---|---|---|---|---|---|---|---|
| $^3P_2$ | 22467 | $^3F_2$ | 569 | $1.04 \times 10^{-2}$ | $^1D_2$ | 16815 | $^3F_3$ | 950 | $9.54 \times 10^{-1}$ |
| | | $^3F_3$ | 618 | $1.53 \times 10^{-1}$ | $^1G_4$ | 9734 | $^3H_4$ | 1027 | $1.68 \times 10^{-1}$ |
| $^1I_6$ | 21302 | $^3H_5$ | 521 | $4.84 \times 10^{-1}$ | | | $^3H_5$ | 1308 | $1.96 \times 10^{-1}$ |
| | | $^3H_6$ | 587 | $4.72 \times 10^{-1}$ | $^3F_4$ | 6720 | $^3H_4$ | 1488 | $1.52 \times 10^{-1}$ |
| $^3P_1$ | 21288 | $^3F_2$ | 610 | $2.12 \times 10^{-2}$ | $^3F_3$ | 6290 | $^3H_4$ | 1590 | $6.27 \times 10^{-3}$ |
| $^1D_2$ | 16815 | $^3F_2$ | 839 | $7.37 \times 10^{-1}$ | | | | | |

[a] The emission rate, $A_{md}$, inside a host material with refractive index $n_r$ would be: $A_{md} = A'_{md}\ n_r^3$

TABLE S3: Calculated $Nd^{3+}$ MD spontaneous emission lines between 300 and 1700 nm.

| $SLJ$ | $E_{SLJ}(cm^{-1})$ | $S'L'J'$ | $\lambda$ (nm) | $A'_{md}$ $(s^{-1})$ [a] | $SLJ$ | $E_{SLJ}(cm^{-1})$ | $S'L'J'$ | $\lambda$ (nm) | $A'_{md}$ $(s^{-1})$ [a] |
|---|---|---|---|---|---|---|---|---|---|
| $^2F_{5/2}$ | 38707 | $^4F_{3/2}$ | 365 | 1.6 | $^2H_{9/2}$ | 33253 | $^2G_{9/2}$ | 804 | $3.53\times10^{-1}$ |
| | | $^4F_{5/2}$ | 379 | $2.03\times10^{-1}$ | | | $^4G_{11/2}$ | 840 | $4.66\times10^{-2}$ |
| | | $^4F_{7/2}$ | 393 | $3.83\times10^{-1}$ | $^2D_{3/2}$ | 33241 | $^4F_{3/2}$ | 457 | $1.37\times10^{-2}$ |
| | | $^4S_{3/2}$ | 395 | $1.07\times10^{-2}$ | | | $^4F_{5/2}$ | 479 | $1.8\times10^{-1}$ |
| | | $^2G_{7/2}$ | 458 | 2.02 | | | $^4S_{3/2}$ | 504 | $1.1\times10^{-2}$ |
| | | $^4G_{5/2}$ | 463 | 1.57 | | | $^4G_{5/2}$ | 620 | $4.83\times10^{-3}$ |
| | | $^4G_{7/2}$ | 506 | $7.02\times10^{-1}$ | | | $^2D_{3/2}$ | 825 | $3.24\times10^{-2}$ |
| | | $^2D_{3/2}$ | 569 | $2.65\times10^{-1}$ | | | $^2P_{1/2}$ | 997 | $1.11\times10^{-1}$ |
| | | $^2D_{5/2}$ | 668 | $2.55\times10^{-2}$ | | | $^2D_{5/2}$ | 1053 | $9.32\times10^{-1}$ |
| | | $^2P_{3/2}$ | 797 | $2.1\times10^{-1}$ | | | $^2P_{3/2}$ | 1412 | $3.19\times10^{-2}$ |
| | | $^4D_{3/2}$ | 948 | $4.55\times10^{-2}$ | $^2L_{17/2}$ | 31674 | $^4I_{15/2}$ | 388 | $1.6\times10^{-2}$ |
| | | $^4D_{5/2}$ | 960 | $3.71\times10^{-1}$ | | | $^2K_{15/2}$ | 986 | $5.87\times10^{-1}$ |
| | | $^4D_{7/2}$ | 1188 | $2.62\times10^{-1}$ | $^2I_{13/2}$ | 30777 | $^4I_{11/2}$ | 345 | $8.16\times10^{-1}$ |
| $^2H_{11/2}$ | 34646 | $^4I_{11/2}$ | 305 | $2.4\times10^{-3}$ | | | $^4I_{13/2}$ | 371 | $9.95\times10^{-3}$ |
| | | $^4I_{13/2}$ | 324 | $2.41\times10^{-1}$ | | | $^4I_{15/2}$ | 402 | 1.82 |
| | | $^2H_{9/2}$ | 445 | $1.61\times10^{-1}$ | | | $^2H_{11/2}$ | 652 | $8.27\times10^{-2}$ |
| | | $^4F_{9/2}$ | 497 | $1.55\times10^{-1}$ | | | $^2K_{13/2}$ | 891 | $3.67\times10^{-1}$ |
| | | $^2H_{11/2}$ | 521 | $8.61\times10^{-3}$ | | | $^4G_{11/2}$ | 1061 | $8.16\times10^{-4}$ |
| | | $^4G_{9/2}$ | 650 | $7.94\times10^{-1}$ | | | $^2K_{15/2}$ | 1081 | $8.38\times10^{-2}$ |
| | | $^2K_{13/2}$ | 662 | $7.67\times10^{-2}$ | $^4D_{7/2}$ | 30290 | $^4I_{9/2}$ | 330 | $2.12\times10^{-9}$ |
| | | $^2G_{9/2}$ | 723 | $6.13\times10^{-3}$ | | | $^2H_{9/2}$ | 552 | $1.33\times10^{-3}$ |
| | | $^4G_{11/2}$ | 752 | $7.42\times10^{-1}$ | | | $^4F_{5/2}$ | 557 | $1.99\times10^{-2}$ |
| $^2D_{5/2}$ | 34177 | $^4F_{3/2}$ | 438 | $3.84\times10^{-1}$ | | | $^4F_{7/2}$ | 588 | $1.29\times10^{-3}$ |
| | | $^4F_{5/2}$ | 458 | $9.54\times10^{-2}$ | | | $^4F_{9/2}$ | 635 | $1.21\times10^{-2}$ |
| | | $^4F_{7/2}$ | 478 | $6.24\times10^{-2}$ | | | $^2G_{7/2}$ | 746 | $1.12\times10^{-5}$ |
| | | $^4S_{3/2}$ | 481 | $6.6\times10^{-3}$ | | | $^4G_{5/2}$ | 759 | $4.98\times10^{-4}$ |
| | | $^2G_{7/2}$ | 579 | $2.24\times10^{-1}$ | | | $^4G_{7/2}$ | 880 | $2.03\times10^{-2}$ |
| | | $^4G_{5/2}$ | 586 | $3.83\times10^{-1}$ | | | $^4G_{9/2}$ | 907 | $1.16\times10^{-2}$ |
| | | $^4G_{7/2}$ | 656 | $2.18\times10^{-1}$ | | | $^2G_{9/2}$ | 1055 | $5.16\times10^{-3}$ |
| | | $^2D_{3/2}$ | 766 | $2.72\times10^{-2}$ | | | $^2D_{5/2}$ | 1528 | $1.28\times10^{-2}$ |
| | | $^2D_{5/2}$ | 959 | $7.92\times10^{-4}$ | $^2L_{15/2}$ | 30204 | $^4I_{13/2}$ | 379 | $2.98\times10^{-2}$ |
| | | $^2P_{3/2}$ | 1247 | $3.28\times10^{-1}$ | | | $^4I_{15/2}$ | 412 | $2.55\times10^{-2}$ |
| | | $^4D_{3/2}$ | 1660 | $5.16\times10^{-1}$ | | | $^2K_{13/2}$ | 939 | $6.74\times10^{-1}$ |
| | | $^4D_{5/2}$ | 1700 | $3.58\times10^{-1}$ | | | $^2K_{15/2}$ | 1153 | $7.62\times10^{-1}$ |
| $^2H_{9/2}$ | 33253 | $^4I_{9/2}$ | 301 | $2.79\times10^{-2}$ | $^2I_{11/2}$ | 29454 | $^4I_{9/2}$ | 340 | 2.18 |
| | | $^4I_{11/2}$ | 318 | $7.66\times10^{-2}$ | | | $^4I_{11/2}$ | 362 | $3.58\times10^{-2}$ |
| | | $^2H_{9/2}$ | 474 | $1.35\times10^{-2}$ | | | $^4I_{13/2}$ | 390 | $3.9\times10^{-1}$ |
| | | $^4F_{7/2}$ | 501 | $1.42\times10^{-3}$ | | | $^2H_{9/2}$ | 578 | $1.39\times10^{-1}$ |
| | | $^4F_{9/2}$ | 534 | $2.62\times10^{-3}$ | | | $^4F_{9/2}$ | 671 | $7.29\times10^{-3}$ |
| | | $^2H_{11/2}$ | 562 | $2.53\times10^{-1}$ | | | $^2H_{11/2}$ | 714 | $2.76\times10^{-1}$ |
| | | $^2G_{7/2}$ | 611 | $3.41\times10^{-2}$ | | | $^4G_{9/2}$ | 982 | $5.\times10^{-2}$ |
| | | $^4G_{7/2}$ | 698 | $5.35\times10^{-1}$ | | | $^2K_{13/2}$ | 1010 | $1.23\times10^{-1}$ |
| | | $^4G_{9/2}$ | 715 | $1.03\times10^{-1}$ | | | $^2G_{9/2}$ | 1157 | $9.86\times10^{-3}$ |

[a] The emission rate, $A_{md}$, inside a host material with refractive index $n_r$ would be: $A_{md} = A'_{md}\ n_r^3$

TABLE S3: Continued: $Nd^{3+}$ MD spontaneous emission lines between 300 and 1700 nm.

| $SLJ$ | $E_{SLJ}(cm^{-1})$ | $S'L'J'$ | $\lambda$ (nm) | $A'_{md}$ $(s^{-1})$ [a] | $SLJ$ | $E_{SLJ}(cm^{-1})$ | $S'L'J'$ | $\lambda$ (nm) | $A'_{md}$ $(s^{-1})$ [a] |
|---|---|---|---|---|---|---|---|---|---|
| $^2I_{11/2}$ | 29454 | $^4G_{11/2}$ | 1235 | $7.98 \times 10^{-2}$ | $^4G_{11/2}$ | 21354 | $^4I_{11/2}$ | 512 | $3.47 \times 10^{-3}$ |
| $^4D_{1/2}$ | 28569 | $^4F_{3/2}$ | 580 | $1.48 \times 10^{-2}$ | | | $^4I_{13/2}$ | 570 | $7.69 \times 10^{-2}$ |
| | | $^4S_{3/2}$ | 659 | $4.88 \times 10^{-2}$ | | | $^2H_{9/2}$ | 1089 | $1.21 \times 10^{-2}$ |
| | | $^2D_{3/2}$ | 1344 | $1.22 \times 10^{-1}$ | | | $^4F_{9/2}$ | 1468 | $1.97 \times 10^{-2}$ |
| $^4D_{5/2}$ | 28293 | $^4F_{3/2}$ | 590 | $1.09 \times 10^{-1}$ | | | $^2H_{11/2}$ | 1692 | $3.02 \times 10^{-1}$ |
| | | $^4F_{5/2}$ | 627 | $5.89 \times 10^{-3}$ | $^2D_{3/2}$ | 21126 | $^4F_{3/2}$ | 1022 | $7.13 \times 10^{-1}$ |
| | | $^4F_{7/2}$ | 666 | $8.07 \times 10^{-3}$ | | | $^4F_{5/2}$ | 1139 | $9.22 \times 10^{-1}$ |
| | | $^4S_{3/2}$ | 671 | $2.27 \times 10^{-2}$ | | | $^4S_{3/2}$ | 1293 | 1.08 |
| | | $^2G_{7/2}$ | 877 | $1.9 \times 10^{-2}$ | $^2G_{9/2}$ | 20810 | $^4I_{9/2}$ | 481 | $2.36 \times 10^{-2}$ |
| | | $^4G_{5/2}$ | 894 | $7.8 \times 10^{-2}$ | | | $^4I_{11/2}$ | 527 | $2.64 \times 10^{-2}$ |
| | | $^4G_{7/2}$ | 1067 | $1.02 \times 10^{-2}$ | | | $^2H_{9/2}$ | 1157 | $2.77 \times 10^{-2}$ |
| | | $^2D_{3/2}$ | 1395 | $3.19 \times 10^{-1}$ | | | $^4F_{7/2}$ | 1327 | $2.52 \times 10^{-1}$ |
| $^4D_{3/2}$ | 28154 | $^4F_{3/2}$ | 595 | $4.08 \times 10^{-6}$ | | | $^4F_{9/2}$ | 1595 | $7.8 \times 10^{-1}$ |
| | | $^4F_{5/2}$ | 633 | $1.96 \times 10^{-4}$ | $^2K_{13/2}$ | 19550 | $^4I_{11/2}$ | 564 | 1.24 |
| | | $^4S_{3/2}$ | 677 | $5.73 \times 10^{-2}$ | | | $^4I_{13/2}$ | 635 | $6.69 \times 10^{-1}$ |
| | | $^4G_{5/2}$ | 905 | $1.03 \times 10^{-2}$ | | | $^4I_{15/2}$ | 734 | $8.97 \times 10^{-5}$ |
| | | $^2D_{3/2}$ | 1423 | $3.05 \times 10^{-3}$ | $^4G_{9/2}$ | 19266 | $^4I_{9/2}$ | 519 | $3.8 \times 10^{-2}$ |
| $^2P_{3/2}$ | 26157 | $^4F_{3/2}$ | 675 | $3.22 \times 10^{-1}$ | | | $^4I_{11/2}$ | 573 | $1.67 \times 10^{-1}$ |
| | | $^4F_{5/2}$ | 724 | $8.57 \times 10^{-1}$ | | | $^2H_{9/2}$ | 1409 | $3.83 \times 10^{-1}$ |
| | | $^4S_{3/2}$ | 784 | $7.87 \times 10^{-1}$ | | | $^4F_{7/2}$ | 1670 | $4.77 \times 10^{-2}$ |
| | | $^4G_{5/2}$ | 1105 | $3.46 \times 10^{-4}$ | $^4G_{7/2}$ | 18925 | $^4I_{9/2}$ | 528 | $2.52 \times 10^{-5}$ |
| $^2D_{5/2}$ | 23747 | $^4F_{3/2}$ | 806 | $8.43 \times 10^{-2}$ | | | $^2H_{9/2}$ | 1480 | $1.44 \times 10^{-2}$ |
| | | $^4F_{5/2}$ | 877 | $2.15 \times 10^{-1}$ | | | $^4F_{5/2}$ | 1520 | $1.32 \times 10^{-1}$ |
| | | $^4F_{7/2}$ | 955 | 1.3 | $^2G_{7/2}$ | 16892 | $^4I_{9/2}$ | 592 | $5.3 \times 10^{-2}$ |
| | | $^4S_{3/2}$ | 966 | $4.81 \times 10^{-2}$ | $^2H_{11/2}$ | 15445 | $^4I_{9/2}$ | 647 | $1.54 \times 10^{-3}$ |
| | | $^2G_{7/2}$ | 1459 | $3.1 \times 10^{-2}$ | | | $^4I_{11/2}$ | 734 | $4.26 \times 10^{-1}$ |
| | | $^4G_{5/2}$ | 1506 | $4.83 \times 10^{-4}$ | | | $^4I_{13/2}$ | 859 | $9.23 \times 10^{-1}$ |
| $^2P_{1/2}$ | 23209 | $^4F_{3/2}$ | 843 | $1.23 \times 10^{-1}$ | $^4F_{9/2}$ | 14540 | $^4I_{9/2}$ | 688 | $2.48 \times 10^{-1}$ |
| | | $^4S_{3/2}$ | 1019 | $8.19 \times 10^{-1}$ | | | $^4I_{11/2}$ | 787 | $2.51 \times 10^{-1}$ |
| $^2K_{15/2}$ | 21530 | $^4I_{13/2}$ | 564 | $9.75 \times 10^{-1}$ | $^4F_{7/2}$ | 13277 | $^4I_{9/2}$ | 753 | $5.53 \times 10^{-3}$ |
| | | $^4I_{15/2}$ | 641 | 1.52 | $^2H_{9/2}$ | 12167 | $^4I_{9/2}$ | 822 | 1.23 |
| $^4G_{11/2}$ | 21354 | $^4I_{9/2}$ | 468 | $1.48 \times 10^{-3}$ | | | $^4I_{11/2}$ | 967 | $7.61 \times 10^{-1}$ |

[a] The emission rate, $A_{md}$, inside a host material with refractive index $n_r$ would be: $A_{md} = A'_{md}\ n_r^3$

TABLE S4: Calculated $Pm^{3+}$ MD spontaneous emission lines between 300 and 1700 nm.

| $SLJ$ | $E_{SLJ}(cm^{-1})$ | $S'L'J'$ | $\lambda$ (nm) | $A'_{md}$ $(s^{-1})$ [a] | $SLJ$ | $E_{SLJ}(cm^{-1})$ | $S'L'J'$ | $\lambda$ (nm) | $A'_{md}$ $(s^{-1})$ [a] |
|---|---|---|---|---|---|---|---|---|---|
| $^1I_6$ | 39524 | $^5F_5$ | 421 | $3.24\times10^{-3}$ | $(^1H, ^3H)_5$ | 37739 | $^5F_4$ | 429 | $1.58\times10^{-1}$ |
| | | $^3K_6$ | 425 | $9.82\times10^{-1}$ | | | $^5F_5$ | 456 | $4.76\times10^{-1}$ |
| | | $^3K_7$ | 450 | $6.89\times10^{-1}$ | | | $^3K_6$ | 459 | $4.57\times10^{-2}$ |
| | | $(^3H, ^5G)_5$ | 502 | $1.2\times10^{-2}$ | | | $(^3H, ^5G)_4$ | 491 | $6.6\times10^{-2}$ |
| | | $^5G_5$ | 567 | $2.88\times10^{-1}$ | | | $(^3H, ^5G)_5$ | 552 | $1.53\times10^{-2}$ |
| | | $^5G_6$ | 577 | $7.57\times10^{-3}$ | | | $^5G_4$ | 565 | $1.26\times10^{-1}$ |
| | | $^3L_7$ | 626 | $2.75\times10^{-2}$ | | | $^5G_5$ | 631 | $7.74\times10^{-3}$ |
| | | $^3H_6$ | 645 | $3.42\times10^{-1}$ | | | $^5G_6$ | 643 | $3.9\times10^{-2}$ |
| | | $^3G_5$ | 800 | $3.23\times10^{-2}$ | | | $^3H_6$ | 728 | $9.54\times10^{-2}$ |
| | | $^3I_5$ | 884 | $2.45\times10^{-2}$ | | | $^3G_4$ | 755 | $8.45\times10^{-1}$ |
| | | $^3I_6$ | 981 | $2.38\times10^{-1}$ | | | $^3G_5$ | 933 | $2.8\times10^{-1}$ |
| | | $^3I_7$ | 1032 | $1.15\times10^{-1}$ | | | $^3F_4$ | 935 | $1.24\times10^{-3}$ |
| $^1D_2$ | 39005 | $^5F_1$ | 374 | $5.18\times10^{-2}$ | | | $^3I_5$ | 1049 | 1.44 |
| | | $^5F_2$ | 379 | $1.91\times10^{-2}$ | | | $^3I_6$ | 1189 | $4.32\times10^{-1}$ |
| | | $^5F_3$ | 392 | $1.09\times10^{-5}$ | $^3H_5$ | 36501 | $^5F_4$ | 453 | $9.22\times10^{-3}$ |
| | | $^5S_2$ | 402 | $1.96\times10^{-2}$ | | | $^5F_5$ | 483 | $1.32\times10^{-2}$ |
| | | $^5G_2$ | 467 | $3.03\times10^{-2}$ | | | $^3K_6$ | 487 | $5.62\times10^{-2}$ |
| | | $^5G_3$ | 474 | $1.44\times10^{-2}$ | | | $(^3H, ^5G)_4$ | 523 | $3.01\times10^{-5}$ |
| | | $^3G_3$ | 577 | $1.88\times10^{-2}$ | | | $(^3H, ^5G)_5$ | 592 | $2.37\times10^{-1}$ |
| | | $^3D_2$ | 627 | $5.74\times10^{-1}$ | | | $^5G_4$ | 607 | $4.9\times10^{-1}$ |
| | | $(^3P, ^3D)_1$ | 667 | $9.22\times10^{-1}$ | | | $^5G_5$ | 684 | $8.01\times10^{-2}$ |
| | | $^3D_3$ | 751 | 1.11 | | | $^5G_6$ | 698 | $1.41\times10^{-1}$ |
| | | $(^1D, ^3F)_2$ | 782 | $2.61\times10^{-1}$ | | | $^3H_6$ | 801 | $2.91\times10^{-2}$ |
| | | $(^3P, ^3D)_1$ | 894 | $1.55\times10^{-1}$ | | | $^3G_4$ | 833 | $4.78\times10^{-1}$ |
| | | $(^3F, ^3P)_2$ | 960 | $9.21\times10^{-1}$ | | | $^3G_5$ | 1055 | $1.21\times10^{-1}$ |
| | | $^3F_3$ | 1012 | $6.59\times10^{-1}$ | | | $^3F_4$ | 1058 | $5.09\times10^{-2}$ |
| | | $^3F_2$ | 1067 | 1.36 | | | $^3I_5$ | 1206 | $9.7\times10^{-2}$ |
| | | $^5D_1$ | 1142 | $5.96\times10^{-3}$ | | | $^3I_6$ | 1394 | $4.18\times10^{-1}$ |
| | | $^5D_2$ | 1262 | $8.36\times10^{-2}$ | $^3H_4$ | 36389 | $^5F_3$ | 436 | $4.53\times10^{-2}$ |
| | | $^5D_3$ | 1392 | $6.55\times10^{-2}$ | | | $^5F_4$ | 455 | $5.58\times10^{-2}$ |
| | | $^3F_3$ | 1654 | $5.08\times10^{-1}$ | | | $^5F_5$ | 486 | $1.37\times10^{-1}$ |
| $^1K_7$ | 38569 | $^5I_8$ | 312 | $1.09\times10^{-4}$ | | | $(^3H, ^5G)_4$ | 526 | $1.7\times10^{-3}$ |
| | | $^3K_6$ | 442 | $6.74\times10^{-1}$ | | | $^5G_3$ | 541 | $2.31\times10^{-2}$ |
| | | $^3K_7$ | 470 | $9.83\times10^{-3}$ | | | $(^3H, ^5G)_5$ | 596 | $1.11\times10^{-2}$ |
| | | $^3K_8$ | 505 | $8.36\times10^{-1}$ | | | $^5G_4$ | 612 | $4.17\times10^{-2}$ |
| | | $^5G_6$ | 610 | $1.64\times10^{-2}$ | | | $^3G_3$ | 680 | $3.61\times10^{-1}$ |
| | | $^3L_7$ | 666 | $6.44\times10^{-1}$ | | | $^5G_5$ | 689 | $4.07\times10^{-6}$ |
| | | $^3H_6$ | 687 | $4.42\times10^{-2}$ | | | $^3G_4$ | 841 | $1.47\times10^{-1}$ |
| | | $(^3L, ^3M)_8$ | 703 | $1.67\times10^{-1}$ | | | $^3D_3$ | 935 | $9.95\times10^{-3}$ |
| | | $(^3M, ^3L)_8$ | 880 | $1.51\times10^{-1}$ | | | $^3G_5$ | 1068 | $8.51\times10^{-3}$ |
| | | $^3I_6$ | 1082 | $5.79\times10^{-1}$ | | | $^3F_4$ | 1070 | $3.43\times10^{-2}$ |
| | | $^3I_7$ | 1145 | $6.39\times10^{-1}$ | | | $^3I_5$ | 1222 | $1.41\times10^{-1}$ |
| | | $^1L_8$ | 1343 | $2.02\times10^{-3}$ | | | $^3F_3$ | 1376 | $2.42\times10^{-2}$ |

[a] The emission rate, $A_{md}$, inside a host material with refractive index $n_r$ would be: $A_{md} = A'_{md}\, n_r^3$

TABLE S4: Continued: $Pm^{3+}$ MD spontaneous emission lines between 300 and 1700 nm.

| $SLJ$ | $E_{SLJ}(cm^{-1})$ | $S'L'J'$ | $\lambda$ (nm) | $A'_{md}$ $(s^{-1})$ [a] | $SLJ$ | $E_{SLJ}(cm^{-1})$ | $S'L'J'$ | $\lambda$ (nm) | $A'_{md}$ $(s^{-1})$ [a] |
|---|---|---|---|---|---|---|---|---|---|
| $^3H_6$ | 36252 | $^5I_6$ | 301 | $8.94 \times 10^{-4}$ | $^1G_4$ | 33415 | $^5F_5$ | 567 | $1.05 \times 10^{-1}$ |
| | | $^5I_7$ | 317 | 2.51 | | | $\left(^3H,\,^5G\right)_4$ | 623 | $2.53 \times 10^{-1}$ |
| | | $^5F_5$ | 489 | $4.45 \times 10^{-2}$ | | | $^5G_3$ | 644 | $4.08 \times 10^{-1}$ |
| | | $^3K_6$ | 493 | $5.87 \times 10^{-1}$ | | | $\left(^3H,\,^5G\right)_5$ | 724 | 1.72 |
| | | $^3K_7$ | 528 | $4.37 \times 10^{-1}$ | | | $^5G_4$ | 748 | $7.22 \times 10^{-1}$ |
| | | $\left(^3H,\,^5G\right)_5$ | 601 | $3.85 \times 10^{-1}$ | | | $^3G_3$ | 853 | $6.17 \times 10^{-2}$ |
| | | $^5G_5$ | 696 | $8.11 \times 10^{-9}$ | | | $^5G_5$ | 867 | $4.01 \times 10^{-1}$ |
| | | $^5G_6$ | 711 | $5.45 \times 10^{-1}$ | | | $^3G_4$ | 1122 | $4.79 \times 10^{-1}$ |
| | | $^3L_7$ | 787 | $1.53 \times 10^{-2}$ | | | $^3D_3$ | 1295 | $2.35 \times 10^{-2}$ |
| | | $^3H_6$ | 817 | $2.8 \times 10^{-2}$ | | | $^3G_5$ | 1564 | $1.19 \times 10^{-2}$ |
| | | $^3G_5$ | 1083 | $1.12 \times 10^{-3}$ | | | $^3F_4$ | 1570 | $4.72 \times 10^{-1}$ |
| | | $^3I_5$ | 1243 | $4.11 \times 10^{-2}$ | $^3F_3$ | 32958 | $^5I_4$ | 303 | $6.96 \times 10^{-7}$ |
| | | $^3I_6$ | 1444 | $6.58 \times 10^{-2}$ | | | $^5F_2$ | 492 | $8.06 \times 10^{-1}$ |
| | | $^3I_7$ | 1558 | $8.96 \times 10^{-2}$ | | | $^5F_3$ | 513 | $6.26 \times 10^{-1}$ |
| $^3F_4$ | 36249 | $^5F_3$ | 439 | $3.21 \times 10^{-1}$ | | | $^5S_2$ | 531 | $8.85 \times 10^{-4}$ |
| | | $^5F_4$ | 458 | $2.3 \times 10^{-1}$ | | | $^5F_4$ | 540 | $4.76 \times 10^{-1}$ |
| | | $^5F_5$ | 489 | 2.97 | | | $\left(^3H,\,^5G\right)_4$ | 642 | $7.74 \times 10^{-1}$ |
| | | $\left(^3H,\,^5G\right)_4$ | 530 | $2.24 \times 10^{-2}$ | | | $^5G_2$ | 651 | $3.61 \times 10^{-2}$ |
| | | $^5G_3$ | 545 | $6.46 \times 10^{-3}$ | | | $^5G_3$ | 664 | $1.03 \times 10^{-1}$ |
| | | $\left(^3H,\,^5G\right)_5$ | 601 | $8.42 \times 10^{-1}$ | | | $^5G_4$ | 774 | 1.61 |
| | | $^5G_4$ | 617 | $4.7 \times 10^{-2}$ | | | $^3G_3$ | 887 | $4.14 \times 10^{-1}$ |
| | | $^3G_3$ | 687 | $7.32 \times 10^{-3}$ | | | $^3D_2$ | 1010 | $5.95 \times 10^{-2}$ |
| | | $^5G_5$ | 696 | 1. | | | $^3G_4$ | 1182 | $1.4 \times 10^{-1}$ |
| | | $^3G_4$ | 851 | $1.49 \times 10^{-1}$ | | | $^3D_3$ | 1377 | $3.75 \times 10^{-1}$ |
| | | $^3D_3$ | 947 | $2.16 \times 10^{-1}$ | | | $\left(^1D,\,^3F\right)_2$ | 1482 | $9.72 \times 10^{-2}$ |
| | | $^3G_5$ | 1084 | $1.16 \times 10^{-1}$ | | | $^3F_4$ | 1691 | $4.68 \times 10^{-2}$ |
| | | $^3F_4$ | 1087 | $6.49 \times 10^{-4}$ | $^5D_4$ | 32302 | $^5I_4$ | 310 | $3.84 \times 10^{-3}$ |
| | | $^3I_5$ | 1243 | $4.97 \times 10^{-3}$ | | | $^5I_5$ | 324 | $1.61 \times 10^{-3}$ |
| | | $^3F_3$ | 1403 | $1.51 \times 10^{-1}$ | | | $^5F_3$ | 531 | $7.45 \times 10^{-3}$ |
| $^1D_2$ | 33653 | $^5F_1$ | 468 | $1.71 \times 10^{-1}$ | | | $^5F_4$ | 560 | $1.97 \times 10^{-2}$ |
| | | $^5F_2$ | 476 | $4.7 \times 10^{-4}$ | | | $^5F_5$ | 606 | $2.19 \times 10^{-1}$ |
| | | $^5F_3$ | 495 | $2.38 \times 10^{-1}$ | | | $\left(^3H,\,^5G\right)_4$ | 670 | $2.76 \times 10^{-2}$ |
| | | $^5S_2$ | 512 | $1.32 \times 10^{-1}$ | | | $^5G_3$ | 694 | $5.55 \times 10^{-2}$ |
| | | $^5G_2$ | 623 | $2.94 \times 10^{-2}$ | | | $\left(^3H,\,^5G\right)_5$ | 788 | $1.53 \times 10^{-1}$ |
| | | $^5G_3$ | 635 | $1.72 \times 10^{-4}$ | | | $^5G_4$ | 815 | $1.8 \times 10^{-1}$ |
| | | $^3G_3$ | 836 | $2.36 \times 10^{-1}$ | | | $^3G_3$ | 942 | $4.54 \times 10^{-2}$ |
| | | $^3D_2$ | 944 | $1.2 \times 10^{-2}$ | | | $^5G_5$ | 960 | $1.55 \times 10^{-1}$ |
| | | $\left(^3P,\,^3D\right)_1$ | 1037 | $6.98 \times 10^{-1}$ | | | $^3G_4$ | 1281 | $9.42 \times 10^{-2}$ |
| | | $^3D_3$ | 1257 | $7.57 \times 10^{-1}$ | | | $^3D_3$ | 1513 | $2.28 \times 10^{-1}$ |
| | | $\left(^1D,\,^3F\right)_2$ | 1344 | $7.22 \times 10^{-3}$ | $^5D_3$ | 31821 | $^5I_4$ | 314 | $4.27 \times 10^{-5}$ |
| $^1G_4$ | 33415 | $^5I_5$ | 313 | $2.08 \times 10^{-3}$ | | | $^5F_2$ | 521 | $1.25 \times 10^{-1}$ |
| | | $^5F_3$ | 501 | $8.48 \times 10^{-2}$ | | | $^5F_3$ | 545 | $1.31 \times 10^{-1}$ |
| | | $^5F_4$ | 527 | $8.61 \times 10^{-2}$ | | | $^5S_2$ | 565 | $5.49 \times 10^{-3}$ |

[a] The emission rate, $A_{md}$, inside a host material with refractive index $n_r$ would be: $A_{md} = A'_{md}\ n_r^3$

TABLE S4: Continued: $Pm^{3+}$ MD spontaneous emission lines between 300 and 1700 nm.

| $SLJ$ | $E_{SLJ}(cm^{-1})$ | $S'L'J'$ | $\lambda$ (nm) | $A'_{md}$ $(s^{-1})$ [a] | $SLJ$ | $E_{SLJ}(cm^{-1})$ | $S'L'J'$ | $\lambda$ (nm) | $A'_{md}$ $(s^{-1})$ [a] |
|---|---|---|---|---|---|---|---|---|---|
| $^5D_3$ | 31821 | $^5F_4$ | 575 | $3.18 \times 10^{-2}$ | $^3F_2$ | 29631 | $^5G_2$ | 831 | 1.59 |
| | | $(^3H,\,^5G)\,_4$ | 692 | $2.94 \times 10^{-2}$ | | | $^5G_3$ | 852 | 2.19 |
| | | $^5G_2$ | 703 | $2.24 \times 10^{-3}$ | | | $^3G_3$ | 1259 | $4.5 \times 10^{-2}$ |
| | | $^5G_3$ | 718 | $2.06 \times 10^{-2}$ | | | $^3D_2$ | 1522 | $4.46 \times 10^{-1}$ |
| | | $^5G_4$ | 849 | $7.65 \times 10^{-2}$ | $^3M_9$ | 29401 | $^5I_8$ | 437 | $1.78 \times 10^{-2}$ |
| | | $^3G_3$ | 987 | $7.66 \times 10^{-2}$ | | | $^3K_8$ | 941 | $7.18 \times 10^{-2}$ |
| | | $^3D_2$ | 1141 | $9.75 \times 10^{-2}$ | $^3I_6$ | 29326 | $^5I_5$ | 359 | 1.18 |
| | | $^3G_4$ | 1366 | $1.53 \times 10^{-2}$ | | | $^5I_6$ | 380 | $7.78 \times 10^{-5}$ |
| | | $^3D_3$ | 1632 | $1.06 \times 10^{-1}$ | | | $^5I_7$ | 407 | 1.32 |
| $^1L_8$ | 31124 | $^5I_7$ | 379 | $4.77 \times 10^{-6}$ | | | $^5F_5$ | 739 | $1.29 \times 10^{-4}$ |
| | | $^5I_8$ | 406 | $7.36 \times 10^{-3}$ | | | $^3K_6$ | 749 | $4.29 \times 10^{-1}$ |
| | | $^3K_7$ | 724 | 2.24 | | | $^3K_7$ | 832 | $7.45 \times 10^{-3}$ |
| | | $^3K_8$ | 809 | $6.08 \times 10^{-1}$ | | | $(^3H,\,^5G)\,_5$ | 1029 | $5.71 \times 10^{-3}$ |
| | | $^3L_7$ | 1321 | $1.25 \times 10^{-2}$ | | | $^5G_5$ | 1344 | $1.6 \times 10^{-2}$ |
| | | $(^3L,\,^3M)\,_8$ | 1474 | $9.8 \times 10^{-1}$ | | | $^5G_6$ | 1400 | $2.48 \times 10^{-2}$ |
| $^5D_2$ | 31078 | $^5F_1$ | 532 | $3. \times 10^{-2}$ | $^3F_3$ | 29121 | $^5I_4$ | 343 | $3.78 \times 10^{-4}$ |
| | | $^5F_2$ | 542 | $6.63 \times 10^{-3}$ | | | $^5F_2$ | 606 | $6.59 \times 10^{-1}$ |
| | | $^5F_3$ | 568 | $1.02 \times 10^{-1}$ | | | $^5F_3$ | 639 | $3.28 \times 10^{-2}$ |
| | | $^5S_2$ | 590 | $2.18 \times 10^{-3}$ | | | $^5S_2$ | 667 | $1.41 \times 10^{-2}$ |
| | | $^5G_2$ | 741 | $2.25 \times 10^{-2}$ | | | $^5F_4$ | 681 | $9.79 \times 10^{-1}$ |
| | | $^5G_3$ | 759 | $1.36 \times 10^{-1}$ | | | $(^3H,\,^5G)\,_4$ | 851 | $6.25 \times 10^{-2}$ |
| | | $^3G_3$ | 1065 | $1.88 \times 10^{-2}$ | | | $^5G_2$ | 867 | $1.55 \times 10^{-2}$ |
| | | $^3D_2$ | 1247 | $3.63 \times 10^{-1}$ | | | $^5G_3$ | 891 | $2.82 \times 10^{-1}$ |
| | | $(^3P,\,^3D)\,_1$ | 1414 | $5.41 \times 10^{-2}$ | | | $^5G_4$ | 1101 | $4.03 \times 10^{-2}$ |
| $^5D_1$ | 30248 | $^5F_1$ | 556 | $2.84 \times 10^{-3}$ | | | $^3G_3$ | 1345 | $1.44 \times 10^{-1}$ |
| | | $^5F_2$ | 567 | $1.72 \times 10^{-1}$ | | | $^3D_2$ | 1649 | $2.02 \times 10^{-1}$ |
| | | $^5S_2$ | 620 | $2.56 \times 10^{-2}$ | $(^3F,\,^3P)\,_2$ | 28583 | $^5F_1$ | 613 | $6.59 \times 10^{-1}$ |
| | | $^5G_2$ | 790 | $6.74 \times 10^{-3}$ | | | $^5F_2$ | 627 | $4.55 \times 10^{-1}$ |
| | | $^3D_2$ | 1391 | $5.24 \times 10^{-2}$ | | | $^5F_3$ | 661 | $1.18 \times 10^{-1}$ |
| | | $(^3P,\,^3D)\,_1$ | 1603 | $1.81 \times 10^{-1}$ | | | $^5S_2$ | 691 | $9.51 \times 10^{-1}$ |
| $^3I_7$ | 29834 | $^5I_6$ | 373 | $5.03 \times 10^{-1}$ | | | $^5G_2$ | 910 | $1.71 \times 10^{-2}$ |
| | | $^5I_7$ | 399 | $5.76 \times 10^{-5}$ | | | $^5G_3$ | 936 | $4.26 \times 10^{-2}$ |
| | | $^5I_8$ | 429 | 2.14 | | | $^3G_3$ | 1450 | $1.21 \times 10^{-1}$ |
| | | $^3K_6$ | 721 | $4.16 \times 10^{-2}$ | $^3I_5$ | 28207 | $^5I_4$ | 355 | 2.13 |
| | | $^3K_7$ | 798 | $3.48 \times 10^{-1}$ | | | $^5I_5$ | 374 | $1.57 \times 10^{-2}$ |
| | | $^3K_8$ | 904 | $2.1 \times 10^{-1}$ | | | $^5I_6$ | 397 | $3.04 \times 10^{-1}$ |
| | | $^5G_6$ | 1307 | $5.03 \times 10^{-2}$ | | | $^5F_4$ | 726 | $4.71 \times 10^{-3}$ |
| | | $^3L_7$ | 1592 | $1.17 \times 10^{-3}$ | | | $^5F_5$ | 806 | $4.8 \times 10^{-4}$ |
| $^5D_0$ | 29716 | $^5F_1$ | 573 | $5.83 \times 10^{-2}$ | | | $^3K_6$ | 817 | $3.26 \times 10^{-1}$ |
| $^3F_2$ | 29631 | $^5F_1$ | 576 | 2.31 | | | $(^3H,\,^5G)\,_4$ | 923 | $2.23 \times 10^{-1}$ |
| | | $^5F_2$ | 588 | $9.33 \times 10^{-1}$ | | | $(^3H,\,^5G)\,_5$ | 1163 | $2.34 \times 10^{-1}$ |
| | | $^5F_3$ | 619 | $4.54 \times 10^{-2}$ | | | $^5G_4$ | 1224 | $6.69 \times 10^{-2}$ |
| | | $^5S_2$ | 645 | $2.6 \times 10^{-2}$ | | | $^5G_5$ | 1582 | $1.03 \times 10^{-1}$ |

[a] The emission rate, $A_{md}$, inside a host material with refractive index $n_r$ would be: $A_{md} = A'_{md}\, n_r^3$

TABLE S4: Continued: $Pm^{3+}$ MD spontaneous emission lines between 300 and 1700 nm.

| $SLJ$ | $E_{SLJ}(cm^{-1})$ | $S'L'J'$ | $\lambda$ (nm) | $A'_{md}$ $(s^{-1})$ [a] | $SLJ$ | $E_{SLJ}(cm^{-1})$ | $S'L'J'$ | $\lambda$ (nm) | $A'_{md}$ $(s^{-1})$ [a] |
|---|---|---|---|---|---|---|---|---|---|
| $^3I_5$ | 28207 | $^5G_6$ | 1660 | $5.35 \times 10^{-2}$ | $^3P_0$ | 25560 | $^5F_1$ | 753 | $1.19 \times 10^{-1}$ |
| $(^3P,\,^3D)\,_1$ | 27821 | $^5F_1$ | 643 | $3.64 \times 10^{-1}$ | $^3G_4$ | 24499 | $^5I_4$ | 408 | $3.71 \times 10^{-1}$ |
| | | $^5F_2$ | 658 | 1.13 | | | $^5I_5$ | 434 | $5.31 \times 10^{-1}$ |
| | | $^5S_2$ | 730 | $6.14 \times 10^{-1}$ | | | $^5F_3$ | 906 | $4.22 \times 10^{-1}$ |
| | | $^5G_2$ | 977 | $3.5 \times 10^{-2}$ | | | $^5F_4$ | 993 | $4.3 \times 10^{-1}$ |
| $(^3M,\,^3L)\,_8$ | 27199 | $^5I_7$ | 445 | $4.55 \times 10^{-2}$ | | | $^5F_5$ | 1149 | $1.19 \times 10^{-1}$ |
| | | $^5I_8$ | 483 | $1.93 \times 10^{-2}$ | | | $(^3H,\,^5G)\,_4$ | 1404 | $8.31 \times 10^{-1}$ |
| | | $^3K_7$ | 1011 | $6.79 \times 10^{-1}$ | | | $^5G_3$ | 1514 | $1.01 \times 10^{-1}$ |
| | | $^3K_8$ | 1186 | $7.93 \times 10^{-2}$ | $(^3L,\,^3M)\,_8$ | 24341 | $^5I_7$ | 510 | $2.85 \times 10^{-1}$ |
| $^3F_4$ | 27046 | $^5I_4$ | 370 | $1.67 \times 10^{-6}$ | | | $^5I_8$ | 561 | $3.84 \times 10^{-1}$ |
| | | $^5I_5$ | 391 | $3.43 \times 10^{-3}$ | | | $^3K_7$ | 1422 | $3.86 \times 10^{-1}$ |
| | | $^5F_3$ | 736 | $6.84 \times 10^{-2}$ | $^3H_6$ | 24011 | $^5I_5$ | 443 | $1.33 \times 10^{-2}$ |
| | | $^5F_4$ | 793 | $1.07 \times 10^{-1}$ | | | $^5I_6$ | 476 | $2.8 \times 10^{-1}$ |
| | | $^5F_5$ | 889 | $6.32 \times 10^{-1}$ | | | $^5I_7$ | 519 | 1.84 |
| | | $(^3H,\,^5G)\,_4$ | 1034 | $3.02 \times 10^{-1}$ | | | $^5F_5$ | 1217 | $1.02 \times 10^{-2}$ |
| | | $^5G_3$ | 1093 | $1.16 \times 10^{-1}$ | | | $^3K_6$ | 1243 | $7.64 \times 10^{-3}$ |
| | | $(^3H,\,^5G)\,_5$ | 1345 | $2.99 \times 10^{-1}$ | | | $^3K_7$ | 1492 | $1.93 \times 10^{-3}$ |
| | | $^5G_4$ | 1427 | $5.14 \times 10^{-3}$ | $(^3P,\,^3D)\,_1$ | 24008 | $^5F_1$ | 852 | $9.66 \times 10^{-1}$ |
| $^3G_5$ | 27022 | $^5I_4$ | 370 | $7.06 \times 10^{-2}$ | | | $^5F_2$ | 879 | $6.52 \times 10^{-1}$ |
| | | $^5I_5$ | 391 | $1.04 \times 10^{-1}$ | | | $^5S_2$ | 1012 | 1.09 |
| | | $^5I_6$ | 416 | $5.16 \times 10^{-1}$ | | | $^5G_2$ | 1558 | $2.41 \times 10^{-2}$ |
| | | $^5F_4$ | 794 | $2.91 \times 10^{-1}$ | $^3L_7$ | 23553 | $^5I_6$ | 487 | $1.49 \times 10^{-1}$ |
| | | $^5F_5$ | 891 | $9.99 \times 10^{-1}$ | | | $^5I_7$ | 532 | $1. \times 10^{-1}$ |
| | | $^3K_6$ | 905 | $3.36 \times 10^{-3}$ | | | $^5I_8$ | 587 | $5.92 \times 10^{-7}$ |
| | | $(^3H,\,^5G)\,_4$ | 1037 | $1.8 \times 10^{-2}$ | | | $^3K_6$ | 1318 | 1.32 |
| | | $(^3H,\,^5G)\,_5$ | 1349 | $2.99 \times 10^{-1}$ | | | $^3K_7$ | 1601 | $7.61 \times 10^{-1}$ |
| | | $^5G_4$ | 1432 | $3.34 \times 10^{-2}$ | $^3D_2$ | 23059 | $^5F_1$ | 927 | $6.28 \times 10^{-1}$ |
| $(^1D,\,^3F)\,_2$ | 26210 | $^5F_1$ | 718 | 1.03 | | | $^5F_2$ | 959 | $1.2 \times 10^{-1}$ |
| | | $^5F_2$ | 736 | $1.1 \times 10^{-1}$ | | | $^5F_3$ | 1042 | 1.62 |
| | | $^5F_3$ | 785 | $3.23 \times 10^{-1}$ | | | $^5S_2$ | 1119 | 1.05 |
| | | $^5S_2$ | 827 | 1.24 | $^5G_6$ | 22183 | $^5I_5$ | 483 | $1.15 \times 10^{-2}$ |
| | | $^5G_2$ | 1160 | $1.6 \times 10^{-2}$ | | | $^5I_6$ | 521 | $1.65 \times 10^{-1}$ |
| | | $^5G_3$ | 1203 | $6.2 \times 10^{-3}$ | | | $^5I_7$ | 574 | $7.22 \times 10^{-1}$ |
| $^3L_9$ | 25711 | $^5I_8$ | 521 | $1.03 \times 10^{-1}$ | | | $^5F_5$ | 1565 | $1.6 \times 10^{-1}$ |
| | | $^3K_8$ | 1441 | 1.44 | | | $^3K_6$ | 1609 | $1.7 \times 10^{-3}$ |
| $^3D_3$ | 25695 | $^5I_4$ | 389 | $1.25 \times 10^{-4}$ | $^5G_5$ | 21885 | $^5I_4$ | 457 | $1. \times 10^{-2}$ |
| | | $^5F_2$ | 765 | $2.89 \times 10^{-2}$ | | | $^5I_5$ | 490 | $6.32 \times 10^{-1}$ |
| | | $^5F_3$ | 818 | $4.6 \times 10^{-2}$ | | | $^5I_6$ | 530 | 1.75 |
| | | $^5S_2$ | 864 | $8.46 \times 10^{-2}$ | | | $^5F_4$ | 1342 | $1.41 \times 10^{-3}$ |
| | | $^5F_4$ | 888 | 1.15 | | | $^5F_5$ | 1641 | $6.04 \times 10^{-2}$ |
| | | $(^3H,\,^5G)\,_4$ | 1202 | $1.24 \times 10^{-1}$ | | | $^3K_6$ | 1690 | $2.59 \times 10^{-5}$ |
| | | $^5G_2$ | 1234 | $5.21 \times 10^{-3}$ | $^3G_3$ | 21688 | $^5I_4$ | 461 | $4.16 \times 10^{-2}$ |
| | | $^5G_3$ | 1282 | $1.13 \times 10^{-1}$ | | | $^5F_2$ | 1104 | $3.35 \times 10^{-1}$ |

[a] The emission rate, $A_{md}$, inside a host material with refractive index $n_r$ would be: $A_{md} = A'_{md}\, n_r^3$

TABLE S4: Continued: $Pm^{3+}$ MD spontaneous emission lines between 300 and 1700 nm.

| $SLJ$ | $E_{SLJ}(cm^{-1})$ | $S'L'J'$ | $\lambda$ (nm) | $A'_{md}$ $(s^{-1})$ [a] | $SLJ$ | $E_{SLJ}(cm^{-1})$ | $S'L'J'$ | $\lambda$ (nm) | $A'_{md}$ $(s^{-1})$ [a] |
|---|---|---|---|---|---|---|---|---|---|
| $^3G_3$ | 21688 | $^5F_3$ | 1216 | $4.46 \times 10^{-1}$ | $(^3H,\, ^5G)\, _4$ | 17376 | $^5I_5$ | 628 | 1.53 |
| | | $^5S_2$ | 1322 | $2.51 \times 10^{-3}$ | $^3K_7$ | 17308 | $^5I_6$ | 699 | 1.7 |
| | | $^5F_4$ | 1378 | $1.14 \times 10^{-3}$ | | | $^5I_7$ | 796 | 1.59 |
| $^5G_4$ | 20038 | $^5I_4$ | 499 | 1.23 | | | $^5I_8$ | 927 | $1.03 \times 10^{-2}$ |
| | | $^5I_5$ | 538 | 1.33 | $^3K_6$ | 15967 | $^5I_5$ | 689 | 1.79 |
| | | $^5F_3$ | 1522 | $4.94 \times 10^{-4}$ | | | $^5I_6$ | 771 | $7.98 \times 10^{-1}$ |
| $(^3H,\, ^5G)\, _5$ | 19610 | $^5I_4$ | 510 | $9.53 \times 10^{-3}$ | | | $^5I_7$ | 892 | $1.49 \times 10^{-3}$ |
| | | $^5I_5$ | 551 | $8.69 \times 10^{-1}$ | $^5F_5$ | 15793 | $^5I_4$ | 633 | $3.9 \times 10^{-4}$ |
| | | $^5I_6$ | 602 | 1.52 | | | $^5I_5$ | 698 | $3.1 \times 10^{-2}$ |
| $^3K_8$ | 18769 | $^5I_7$ | 713 | 1.07 | | | $^5I_6$ | 782 | $3.47 \times 10^{-2}$ |
| | | $^5I_8$ | 816 | 2.45 | $^5F_4$ | 14432 | $^5I_4$ | 693 | $9.71 \times 10^{-2}$ |
| $^5G_3$ | 17896 | $^5I_4$ | 559 | $5.05 \times 10^{-2}$ | | | $^5I_5$ | 771 | $3.59 \times 10^{-2}$ |
| $(^3H,\, ^5G)\, _4$ | 17376 | $^5I_4$ | 575 | 2.47 | $^5F_3$ | 13466 | $^5I_4$ | 743 | $1.55 \times 10^{-3}$ |

[a] The emission rate, $A_{md}$, inside a host material with refractive index $n_r$ would be: $A_{md} = A'_{md}\, n_r^3$

TABLE S5: Calculated $Sm^{3+}$ MD spontaneous emission lines between 300 and 1700 nm.

| $SLJ$ | $E_{SLJ}(cm^{-1})$ | $S'L'J'$ | $\lambda$ (nm) | $A'_{md}$ $(s^{-1})$ [a] | $SLJ$ | $E_{SLJ}(cm^{-1})$ | $S'L'J'$ | $\lambda$ (nm) | $A'_{md}$ $(s^{-1})$ [a] |
|---|---|---|---|---|---|---|---|---|---|
| $^2H_{11/2}$ | 39247 | $^6F_{9/2}$ | 330 | $6.29 \times 10^{-3}$ | $^2F_{7/2}$ | 38706 | $^4F_{5/2}$ | 605 | $2.3 \times 10^{-1}$ |
| | | $^6F_{11/2}$ | 347 | $1.3 \times 10^{-1}$ | | | $^4G_{9/2}$ | 626 | 4.89 |
| | | $^4I_{11/2}$ | 551 | $7.62 \times 10^{-1}$ | | | $(^6P,\,^4P)_{5/2}$ | 673 | $3.58 \times 10^{-3}$ |
| | | $(^4K,\,^4I)_{13/2}$ | 561 | 2.08 | | | $^4F_{7/2}$ | 724 | $9.08 \times 10^{-2}$ |
| | | $^4I_{9/2}$ | 562 | $4.25 \times 10^{-5}$ | | | $^6P_{7/2}$ | 815 | $1.54 \times 10^{-1}$ |
| | | $^4G_{9/2}$ | 606 | $8.28 \times 10^{-1}$ | | | $^4F_{9/2}$ | 886 | $3.49 \times 10^{-4}$ |
| | | $^4L_{13/2}$ | 695 | $4.52 \times 10^{-1}$ | | | $(^4D,\,^6P)_{5/2}$ | 890 | $2.16 \times 10^{-2}$ |
| | | $^4K_{11/2}$ | 697 | $2.62 \times 10^{-2}$ | | | $^4H_{7/2}$ | 1001 | $1.55 \times 10^{-1}$ |
| | | $^4G_{11/2}$ | 734 | $5.62 \times 10^{-1}$ | | | $^4D_{7/2}$ | 1011 | $4.73 \times 10^{-1}$ |
| | | $^4K_{13/2}$ | 777 | $4.91 \times 10^{-2}$ | | | $^4H_{9/2}$ | 1061 | $3.01 \times 10^{-1}$ |
| | | $^4F_{9/2}$ | 846 | $3.92 \times 10^{-2}$ | | | $^4G_{7/2}$ | 1148 | $3.16 \times 10^{-2}$ |
| | | $^4H_{9/2}$ | 1003 | $5.04 \times 10^{-1}$ | | | $^4G_{5/2}$ | 1159 | $2.74 \times 10^{-1}$ |
| | | $^4H_{11/2}$ | 1049 | $7.5 \times 10^{-1}$ | | | $^4G_{9/2}$ | 1163 | $5.1 \times 10^{-7}$ |
| | | $^4G_{9/2}$ | 1094 | $1.56 \times 10^{-1}$ | | | $^4P_{5/2}$ | 1633 | $1.19 \times 10^{-1}$ |
| | | $^4H_{13/2}$ | 1100 | $5.9 \times 10^{-3}$ | $^2M_{17/2}$ | 38464 | $^6H_{15/2}$ | 312 | $6.39 \times 10^{-6}$ |
| | | $^4G_{11/2}$ | 1268 | $4.99 \times 10^{-1}$ | | | $^4M_{15/2}$ | 579 | 3.27 |
| | | $^2K_{13/2}$ | 1642 | $1.4 \times 10^{-3}$ | | | $^4M_{17/2}$ | 627 | $5.58 \times 10^{-2}$ |
| $^2G_{7/2}$ | 39072 | $^6F_{5/2}$ | 311 | $1.79 \times 10^{-3}$ | | | $(^4I,\,^4K)_{15/2}$ | 650 | 1.92 |
| | | $^6F_{7/2}$ | 319 | $5.63 \times 10^{-4}$ | | | $^4M_{19/2}$ | 694 | $7.37 \times 10^{-1}$ |
| | | $^6F_{9/2}$ | 332 | $1.09 \times 10^{-2}$ | | | $(^4L,\,^4I)_{15/2}$ | 747 | 1.23 |
| | | $^4G_{5/2}$ | 477 | $3.4 \times 10^{-2}$ | | | $^4L_{17/2}$ | 798 | 1.08 |
| | | $^4G_{7/2}$ | 529 | $2.01 \times 10^{-3}$ | | | $^4K_{15/2}$ | 950 | $1.7 \times 10^{-1}$ |
| | | $^4I_{9/2}$ | 568 | $8.57 \times 10^{-2}$ | | | $^4K_{17/2}$ | 972 | $2.36 \times 10^{-1}$ |
| | | $^4F_{5/2}$ | 592 | 3.23 | | | $^4L_{19/2}$ | 1083 | $7.47 \times 10^{-4}$ |
| | | $^4G_{9/2}$ | 612 | $1.25 \times 10^{-1}$ | | | $(^2K,\,^2L)_{15/2}$ | 1639 | $5.99 \times 10^{-3}$ |
| | | $(^6P,\,^4P)_{5/2}$ | 657 | $1.75 \times 10^{-1}$ | $(^2P,\,^2D)_{3/2}$ | 38395 | $^6F_{1/2}$ | 311 | $6.16 \times 10^{-2}$ |
| | | $^4F_{7/2}$ | 705 | 2.36 | | | $^6F_{3/2}$ | 313 | $6.56 \times 10^{-2}$ |
| | | $^6P_{7/2}$ | 792 | $4.95 \times 10^{-2}$ | | | $^6F_{5/2}$ | 317 | $4.46 \times 10^{-2}$ |
| | | $^4F_{9/2}$ | 858 | $1.64 \times 10^{-2}$ | | | $^4G_{5/2}$ | 493 | $4.97 \times 10^{-2}$ |
| | | $(^4D,\,^6P)_{5/2}$ | 862 | $7.8 \times 10^{-3}$ | | | $^4F_{3/2}$ | 513 | $5.91 \times 10^{-1}$ |
| | | $^4H_{7/2}$ | 966 | $7.28 \times 10^{-1}$ | | | $^4F_{5/2}$ | 617 | $3.29 \times 10^{-1}$ |
| | | $^4D_{7/2}$ | 975 | $7.69 \times 10^{-3}$ | | | $(^6P,\,^4P)_{5/2}$ | 688 | $2.64 \times 10^{-1}$ |
| | | $^4H_{9/2}$ | 1021 | $6.84 \times 10^{-1}$ | | | $^6P_{3/2}$ | 730 | $2.21 \times 10^{-1}$ |
| | | $^4G_{7/2}$ | 1101 | $6.03 \times 10^{-2}$ | | | $^4D_{1/2}$ | 825 | $5.43 \times 10^{-1}$ |
| | | $^4G_{5/2}$ | 1112 | $7.91 \times 10^{-1}$ | | | $^4D_{3/2}$ | 910 | 2.02 |
| | | $^4G_{9/2}$ | 1116 | $3.42 \times 10^{-1}$ | | | $(^4D,\,^6P)_{5/2}$ | 915 | $7.37 \times 10^{-1}$ |
| | | $^4P_{5/2}$ | 1541 | $2.03 \times 10^{-2}$ | | | $^4G_{5/2}$ | 1203 | $1.45 \times 10^{-2}$ |
| $^2F_{7/2}$ | 38706 | $^6F_{5/2}$ | 314 | $1.61 \times 10^{-1}$ | | | $^4P_{1/2}$ | 1347 | $1.73 \times 10^{-1}$ |
| | | $^6F_{7/2}$ | 323 | $1.1 \times 10^{-1}$ | | | $^4P_{3/2}$ | 1418 | 1.11 |
| | | $^6F_{9/2}$ | 336 | $2.67 \times 10^{-1}$ | $(^2H,\,^4I)_{9/2}$ | 37737 | $^6F_{7/2}$ | 334 | $1.86 \times 10^{-2}$ |
| | | $^4G_{5/2}$ | 486 | $2.84 \times 10^{-1}$ | | | $^6F_{9/2}$ | 348 | $4.47 \times 10^{-2}$ |
| | | $^4G_{7/2}$ | 540 | $4.42 \times 10^{-1}$ | | | $^6F_{11/2}$ | 366 | $5.3 \times 10^{-2}$ |
| | | $^4I_{9/2}$ | 580 | $7.48 \times 10^{-3}$ | | | $^4G_{7/2}$ | 569 | $5.88 \times 10^{-1}$ |

[a] The emission rate, $A_{md}$, inside a host material with refractive index $n_r$ would be: $A_{md} = A'_{md}\, n_r^3$

TABLE S5: Continued: $Sm^{3+}$ MD spontaneous emission lines between 300 and 1700 nm.

| $SLJ$ | $E_{SLJ}(cm^{-1})$ | $S'L'J'$ | $\lambda$ (nm) | $A'_{md}$ $(s^{-1})$ [a] | $SLJ$ | $E_{SLJ}(cm^{-1})$ | $S'L'J'$ | $\lambda$ (nm) | $A'_{md}$ $(s^{-1})$ [a] |
|---|---|---|---|---|---|---|---|---|---|
| $(^2H, ^4I)_{9/2}$ | 37737 | $^4I_{11/2}$ | 601 | $8.79 \times 10^{-1}$ | $^4F_{5/2}$ | 36255 | $^4G_{5/2}$ | 551 | $9.18 \times 10^{-2}$ |
| | | $^4I_{9/2}$ | 614 | 1.34 | | | $^4F_{3/2}$ | 577 | $1.29 \times 10^{-2}$ |
| | | $^4G_{9/2}$ | 667 | $2.66 \times 10^{-1}$ | | | $^4G_{7/2}$ | 622 | $1.95 \times 10^{-1}$ |
| | | $^4F_{7/2}$ | 778 | $1.76 \times 10^{-2}$ | | | $^4F_{5/2}$ | 710 | $2.03 \times 10^{-1}$ |
| | | $^4K_{11/2}$ | 779 | 1.01 | | | $(^6P, ^4P)_{5/2}$ | 806 | $8.48 \times 10^{-2}$ |
| | | $^4G_{11/2}$ | 826 | $5.46 \times 10^{-2}$ | | | $^6P_{3/2}$ | 865 | $1.81 \times 10^{-2}$ |
| | | $^6P_{7/2}$ | 885 | $1.36 \times 10^{-2}$ | | | $^4F_{7/2}$ | 880 | $1.68 \times 10^{-2}$ |
| | | $^4F_{9/2}$ | 969 | $5.09 \times 10^{-1}$ | | | $^6P_{7/2}$ | 1019 | $5.14 \times 10^{-2}$ |
| | | $^4H_{7/2}$ | 1108 | $1.3 \times 10^{-1}$ | | | $^4D_{3/2}$ | 1130 | $4.62 \times 10^{-2}$ |
| | | $^4D_{7/2}$ | 1121 | $1.32 \times 10^{-2}$ | | | $(^4D, ^6P)_{5/2}$ | 1138 | $1.35 \times 10^{-1}$ |
| | | $^4H_{9/2}$ | 1183 | $2.78 \times 10^{-1}$ | | | $^4H_{7/2}$ | 1326 | $4.67 \times 10^{-4}$ |
| | | $^4H_{11/2}$ | 1246 | $2.28 \times 10^{-1}$ | | | $^4D_{7/2}$ | 1344 | $8.22 \times 10^{-2}$ |
| | | $^4G_{7/2}$ | 1291 | $3.75 \times 10^{-1}$ | | | $^4G_{7/2}$ | 1597 | $8.45 \times 10^{-2}$ |
| | | $^4G_{9/2}$ | 1311 | $1.38 \times 10^{-1}$ | | | $^4G_{5/2}$ | 1619 | $5.48 \times 10^{-2}$ |
| | | $^4G_{11/2}$ | 1568 | $1.04 \times 10^{-1}$ | $^4I_{13/2}$ | 36214 | $^6H_{11/2}$ | 307 | $2.83 \times 10^{-2}$ |
| $^2L_{17/2}$ | 37165 | $^6H_{15/2}$ | 326 | $1.33 \times 10^{-3}$ | | | $^6H_{13/2}$ | 321 | $1.04 \times 10^{-1}$ |
| | | $^4M_{15/2}$ | 626 | $5.35 \times 10^{-2}$ | | | $^6H_{15/2}$ | 336 | $1.68 \times 10^{-2}$ |
| | | $^4M_{17/2}$ | 683 | 1.18 | | | $^6F_{11/2}$ | 387 | $3.25 \times 10^{-4}$ |
| | | $(^4I, ^4K)_{15/2}$ | 710 | $2.84 \times 10^{-1}$ | | | $^4I_{11/2}$ | 662 | $2.64 \times 10^{-1}$ |
| | | $^4M_{19/2}$ | 763 | 2.07 | | | $^4M_{15/2}$ | 665 | $8.31 \times 10^{-2}$ |
| | | $(^4L, ^4I)_{15/2}$ | 827 | $4.51 \times 10^{-1}$ | | | $(^4K, ^4I)_{13/2}$ | 675 | $1.1 \times 10^{-1}$ |
| | | $^4L_{17/2}$ | 890 | $5.18 \times 10^{-1}$ | | | $(^4I, ^4K)_{15/2}$ | 761 | $1.34 \times 10^{-1}$ |
| | | $^4K_{15/2}$ | 1084 | 2.4 | | | $^4L_{13/2}$ | 881 | $1.37 \times 10^{-1}$ |
| | | $^4K_{17/2}$ | 1112 | 1.22 | | | $^4K_{11/2}$ | 884 | $4.43 \times 10^{-3}$ |
| | | $^4L_{19/2}$ | 1260 | 2.3 | | | $(^4L, ^4I)_{15/2}$ | 897 | $4.73 \times 10^{-3}$ |
| $^2N_{21/2}$ | 36867 | $^4M_{19/2}$ | 781 | 1.81 | | | $^4G_{11/2}$ | 945 | $2.77 \times 10^{-2}$ |
| | | $^4M_{21/2}$ | 879 | 2.33 | | | $^4K_{13/2}$ | 1016 | $7.83 \times 10^{-2}$ |
| | | $^4L_{19/2}$ | 1309 | $4.21 \times 10^{-2}$ | | | $^4K_{15/2}$ | 1208 | $7.34 \times 10^{-3}$ |
| $^4F_{3/2}$ | 36466 | $^6F_{1/2}$ | 331 | 1.2 | | | $^4H_{11/2}$ | 1538 | $2.13 \times 10^{-3}$ |
| | | $^6F_{3/2}$ | 333 | $4. \times 10^{-1}$ | | | $^4H_{13/2}$ | 1651 | $3.99 \times 10^{-1}$ |
| | | $^6F_{5/2}$ | 338 | $9.1 \times 10^{-2}$ | $^2N_{19/2}$ | 35983 | $^4M_{17/2}$ | 743 | $8.14 \times 10^{-1}$ |
| | | $^4G_{5/2}$ | 545 | $1.11 \times 10^{-2}$ | | | $^4M_{19/2}$ | 839 | $7.23 \times 10^{-1}$ |
| | | $^4F_{3/2}$ | 570 | $6.56 \times 10^{-2}$ | | | $^4M_{21/2}$ | 953 | $3.88 \times 10^{-1}$ |
| | | $^4F_{5/2}$ | 700 | $4.59 \times 10^{-3}$ | | | $^4L_{17/2}$ | 995 | $4.78 \times 10^{-2}$ |
| | | $(^6P, ^4P)_{5/2}$ | 793 | $2.85 \times 10^{-5}$ | | | $^4K_{17/2}$ | 1280 | $1.68 \times 10^{-2}$ |
| | | $^6P_{3/2}$ | 850 | $3.51 \times 10^{-3}$ | | | $^4L_{19/2}$ | 1481 | $1.21 \times 10^{-1}$ |
| | | $^4D_{1/2}$ | 981 | $3.16 \times 10^{-2}$ | $^4I_{15/2}$ | 35853 | $^6H_{13/2}$ | 325 | $1.43 \times 10^{-2}$ |
| | | $^4D_{3/2}$ | 1103 | $5.97 \times 10^{-3}$ | | | $^6H_{15/2}$ | 340 | $2.22 \times 10^{-1}$ |
| | | $(^4D, ^6P)_{5/2}$ | 1112 | $1.01 \times 10^{-2}$ | | | $^4M_{15/2}$ | 682 | $9.13 \times 10^{-3}$ |
| | | $^4G_{5/2}$ | 1566 | $1.17 \times 10^{-1}$ | | | $(^4K, ^4I)_{13/2}$ | 692 | $2.8 \times 10^{-1}$ |
| $^4F_{5/2}$ | 36255 | $^6F_{3/2}$ | 335 | $4.61 \times 10^{-1}$ | | | $^4M_{17/2}$ | 750 | $4.4 \times 10^{-3}$ |
| | | $^6F_{5/2}$ | 340 | $1.53 \times 10^{-1}$ | | | $(^4I, ^4K)_{15/2}$ | 782 | $3.68 \times 10^{-2}$ |
| | | $^6F_{7/2}$ | 351 | $1.23 \times 10^{-1}$ | | | $^4L_{13/2}$ | 910 | $7.47 \times 10^{-3}$ |

[a] The emission rate, $A_{md}$, inside a host material with refractive index $n_r$ would be: $A_{md} = A'_{md}\ n_r^3$

TABLE S5: Continued: $Sm^{3+}$ MD spontaneous emission lines between 300 and 1700 nm.

| $SLJ$ | $E_{SLJ}(cm^{-1})$ | $S'L'J'$ | $\lambda$ (nm) | $A'_{md}$ $(s^{-1})$ [a] | $SLJ$ | $E_{SLJ}(cm^{-1})$ | $S'L'J'$ | $\lambda$ (nm) | $A'_{md}$ $(s^{-1})$ [a] |
|---|---|---|---|---|---|---|---|---|---|
| $^4I_{15/2}$ | 35853 | $(^4L, {^4I})_{15/2}$ | 927 | $6.83 \times 10^{-2}$ | $(^4I, {^4F})_{9/2}$ | 34193 | $^6H_{7/2}$ | 302 | $2.97 \times 10^{-2}$ |
| | | $^4L_{17/2}$ | 1008 | $2.52 \times 10^{-2}$ | | | $^6H_{9/2}$ | 313 | $1.6 \times 10^{-2}$ |
| | | $^4K_{13/2}$ | 1055 | $3.47 \times 10^{-2}$ | | | $^6H_{11/2}$ | 327 | $2.8 \times 10^{-2}$ |
| | | $^4K_{15/2}$ | 1263 | $1.95 \times 10^{-2}$ | | | $^6F_{7/2}$ | 378 | $1.26 \times 10^{-1}$ |
| | | $^4K_{17/2}$ | 1302 | $4.28 \times 10^{-3}$ | | | $^6F_{9/2}$ | 396 | $4.18 \times 10^{-2}$ |
| $^2P_{1/2}$ | 35696 | $^6F_{1/2}$ | 339 | 1.67 | | | $^6F_{11/2}$ | 420 | $3.7 \times 10^{-1}$ |
| | | $^6F_{3/2}$ | 342 | $7.86 \times 10^{-1}$ | | | $^4G_{7/2}$ | 713 | $1.12 \times 10^{-1}$ |
| | | $^4F_{3/2}$ | 596 | $4.94 \times 10^{-1}$ | | | $^4I_{11/2}$ | 764 | $1.91 \times 10^{-1}$ |
| | | $^6P_{3/2}$ | 909 | $4.93 \times 10^{-3}$ | | | $^4I_{9/2}$ | 785 | $1.83 \times 10^{-1}$ |
| | | $^4D_{1/2}$ | 1061 | 1.11 | | | $^4G_{9/2}$ | 873 | $5. \times 10^{-2}$ |
| | | $^4D_{3/2}$ | 1206 | 4.03 | | | $^4F_{7/2}$ | 1075 | $1.88 \times 10^{-2}$ |
| $^4F_{7/2}$ | 35538 | $^6H_{9/2}$ | 301 | $8.16 \times 10^{-5}$ | | | $^4K_{11/2}$ | 1077 | $1.94 \times 10^{-2}$ |
| | | $^6F_{5/2}$ | 349 | $3.59 \times 10^{-1}$ | | | $^4G_{11/2}$ | 1168 | $3.61 \times 10^{-3}$ |
| | | $^6F_{7/2}$ | 360 | $2.56 \times 10^{-2}$ | | | $^6P_{7/2}$ | 1290 | $1.08 \times 10^{-2}$ |
| | | $^6F_{9/2}$ | 376 | $6.74 \times 10^{-1}$ | | | $^4F_{9/2}$ | 1477 | $5.13 \times 10^{-2}$ |
| | | $^4G_{5/2}$ | 574 | $1.71 \times 10^{-3}$ | $^2F_{5/2}$ | 33939 | $^6H_{7/2}$ | 304 | $1.23 \times 10^{-2}$ |
| | | $^4G_{7/2}$ | 651 | $1.51 \times 10^{-2}$ | | | $^6F_{3/2}$ | 363 | $2.44 \times 10^{-1}$ |
| | | $^4I_{9/2}$ | 710 | $1.08 \times 10^{-3}$ | | | $^6F_{5/2}$ | 370 | $1.01 \times 10^{-1}$ |
| | | $^4F_{5/2}$ | 748 | $8.76 \times 10^{-3}$ | | | $^6F_{7/2}$ | 382 | $1.24 \times 10^{-1}$ |
| | | $^4G_{9/2}$ | 782 | $3.67 \times 10^{-2}$ | | | $^4G_{5/2}$ | 632 | 1.46 |
| | | $(^6P, {^4P})_{5/2}$ | 856 | $3.3 \times 10^{-2}$ | | | $^4F_{3/2}$ | 666 | $9.53 \times 10^{-1}$ |
| | | $^4F_{7/2}$ | 939 | $2.01 \times 10^{-2}$ | | | $^4G_{7/2}$ | 726 | 4.43 |
| | | $^6P_{7/2}$ | 1099 | $3.6 \times 10^{-2}$ | | | $^4F_{5/2}$ | 850 | 1.75 |
| | | $^4F_{9/2}$ | 1232 | $1.59 \times 10^{-2}$ | | | $(^6P, {^4P})_{5/2}$ | 991 | $2.69 \times 10^{-1}$ |
| | | $(^4D, {^6P})_{5/2}$ | 1239 | $2.11 \times 10^{-2}$ | | | $^6P_{3/2}$ | 1082 | $9.72 \times 10^{-3}$ |
| | | $^4H_{7/2}$ | 1466 | $5.64 \times 10^{-3}$ | | | $^4F_{7/2}$ | 1105 | $5.51 \times 10^{-2}$ |
| | | $^4D_{7/2}$ | 1487 | $6.53 \times 10^{-2}$ | | | $^6P_{7/2}$ | 1334 | $1.18 \times 10^{-2}$ |
| | | $^4H_{9/2}$ | 1598 | $3.37 \times 10^{-3}$ | | | $^4D_{3/2}$ | 1530 | $3.81 \times 10^{-1}$ |
| $^4I_{11/2}$ | 35523 | $^6H_{9/2}$ | 301 | $2.22 \times 10^{-5}$ | | | $(^4D, {^6P})_{5/2}$ | 1546 | 1.19 |
| | | $^6H_{11/2}$ | 313 | $1.93 \times 10^{-2}$ | $^4F_{9/2}$ | 33661 | $^6H_{7/2}$ | 307 | $9.65 \times 10^{-3}$ |
| | | $^6H_{13/2}$ | 328 | $1.33 \times 10^{-3}$ | | | $^6H_{9/2}$ | 319 | $2.54 \times 10^{-6}$ |
| | | $^6F_{9/2}$ | 377 | $1.32 \times 10^{-2}$ | | | $^6H_{11/2}$ | 333 | $1.19 \times 10^{-1}$ |
| | | $^6F_{11/2}$ | 398 | $6.85 \times 10^{-2}$ | | | $^6F_{7/2}$ | 386 | $4.74 \times 10^{-3}$ |
| | | $^4I_{11/2}$ | 694 | $1.45 \times 10^{-2}$ | | | $^6F_{9/2}$ | 405 | $4.26 \times 10^{-1}$ |
| | | $(^4K, {^4I})_{13/2}$ | 708 | $3.9 \times 10^{-4}$ | | | $^6F_{11/2}$ | 430 | $9.28 \times 10^{-1}$ |
| | | $^4I_{9/2}$ | 711 | $1.18 \times 10^{-1}$ | | | $^4G_{7/2}$ | 741 | $3.09 \times 10^{-1}$ |
| | | $^4G_{9/2}$ | 782 | $1.8 \times 10^{-1}$ | | | $^4I_{11/2}$ | 797 | $1.58 \times 10^{-1}$ |
| | | $^4L_{13/2}$ | 938 | $3.4 \times 10^{-3}$ | | | $^4I_{9/2}$ | 819 | $1.67 \times 10^{-1}$ |
| | | $^4K_{11/2}$ | 942 | $2.29 \times 10^{-1}$ | | | $^4G_{9/2}$ | 916 | $1.57 \times 10^{-1}$ |
| | | $^4G_{11/2}$ | 1011 | $2.09 \times 10^{-1}$ | | | $^4F_{7/2}$ | 1140 | $2.06 \times 10^{-2}$ |
| | | $^4K_{13/2}$ | 1093 | $3.22 \times 10^{-3}$ | | | $^4K_{11/2}$ | 1142 | $3.63 \times 10^{-3}$ |
| | | $^4F_{9/2}$ | 1234 | $5.75 \times 10^{-2}$ | | | $^4G_{11/2}$ | 1245 | $2.11 \times 10^{-1}$ |
| | | $^4H_{9/2}$ | 1602 | $4.37 \times 10^{-3}$ | | | $^6P_{7/2}$ | 1385 | $1.28 \times 10^{-2}$ |

[a] The emission rate, $A_{md}$, inside a host material with refractive index $n_r$ would be: $A_{md} = A'_{md}\ n_r^3$

TABLE S5: Continued: $Sm^{3+}$ MD spontaneous emission lines between 300 and 1700 nm.

| $SLJ$ | $E_{SLJ}(cm^{-1})$ | $S'L'J'$ | $\lambda$ (nm) | $A'_{md}$ $(s^{-1})$ [a] | $SLJ$ | $E_{SLJ}(cm^{-1})$ | $S'L'J'$ | $\lambda$ (nm) | $A'_{md}$ $(s^{-1})$ [a] |
|---|---|---|---|---|---|---|---|---|---|
| $^4F_{9/2}$ | 33661 | $^4F_{9/2}$ | 1603 | $1.37\times10^{-2}$ | $^4G_{11/2}$ | 31358 | $(^4K,\,^4I)_{13/2}$ | 1005 | $4.61\times10^{-2}$ |
| $^2K_{13/2}$ | 33157 | $^6H_{11/2}$ | 339 | $1.18\times10^{-1}$ | | | $^4I_{9/2}$ | 1010 | $1.93\times10^{-3}$ |
| | | $^6H_{13/2}$ | 356 | $1.52\times10^{-1}$ | | | $^4G_{9/2}$ | 1161 | $2.25\times10^{-1}$ |
| | | $^6H_{15/2}$ | 374 | $1.74\times10^{-2}$ | | | $^4L_{13/2}$ | 1540 | $9.67\times10^{-3}$ |
| | | $^6F_{11/2}$ | 439 | $1.75\times10^{-4}$ | | | $^4K_{11/2}$ | 1550 | $1.19\times10^{-2}$ |
| | | $^4I_{11/2}$ | 830 | $9.99\times10^{-1}$ | $^4P_{3/2}$ | 31340 | $^6H_{5/2}$ | 319 | $6.12\times10^{-5}$ |
| | | $^4M_{15/2}$ | 835 | $5.31\times10^{-3}$ | | | $^6F_{1/2}$ | 398 | $1.4\times10^{-2}$ |
| | | $(^4K,\,^4I)_{13/2}$ | 851 | $3.65\times10^{-1}$ | | | $^6F_{3/2}$ | 401 | $1.24\times10^{-3}$ |
| | | $(^4I,\,^4K)_{15/2}$ | 992 | $1.12\times10^{-2}$ | | | $^6F_{5/2}$ | 409 | $4.89\times10^{-1}$ |
| | | $^4L_{13/2}$ | 1206 | 2.28 | | | $^4G_{5/2}$ | 756 | $2.09\times10^{-2}$ |
| | | $^4K_{11/2}$ | 1212 | 2.18 | | | $^4F_{3/2}$ | 805 | $4.32\times10^{-2}$ |
| | | $(^4L,\,^4I)_{15/2}$ | 1237 | $6.32\times10^{-1}$ | | | $^4F_{5/2}$ | 1091 | $1.95\times10^{-2}$ |
| | | $^4G_{11/2}$ | 1328 | $4.59\times10^{-2}$ | | | $(^6P,\,^4P)_{5/2}$ | 1335 | $2.14\times10^{-5}$ |
| | | $^4K_{13/2}$ | 1475 | $1.71\times10^{-2}$ | | | $^6P_{3/2}$ | 1505 | $7.99\times10^{-1}$ |
| $^4P_{5/2}$ | 32581 | $^6H_{5/2}$ | 307 | $6.92\times10^{-4}$ | $^4P_{1/2}$ | 30973 | $^6F_{1/2}$ | 404 | $1.05\times10^{-1}$ |
| | | $^6H_{7/2}$ | 317 | $2.45\times10^{-3}$ | | | $^6F_{3/2}$ | 407 | $9.48\times10^{-2}$ |
| | | $^6F_{3/2}$ | 382 | $2.67\times10^{-2}$ | | | $^4F_{3/2}$ | 830 | $2.82\times10^{-1}$ |
| | | $^6F_{5/2}$ | 389 | $3.09\times10^{-2}$ | | | $^6P_{3/2}$ | 1594 | 2.23 |
| | | $^6F_{7/2}$ | 403 | $8.54\times10^{-1}$ | $^4H_{13/2}$ | 30158 | $^6H_{11/2}$ | 377 | $1.31\times10^{-3}$ |
| | | $^4G_{5/2}$ | 691 | $8.78\times10^{-2}$ | | | $^6H_{13/2}$ | 399 | $2.82\times10^{-2}$ |
| | | $^4F_{3/2}$ | 732 | $6.02\times10^{-2}$ | | | $^6H_{15/2}$ | 422 | $6.74\times10^{-1}$ |
| | | $^4G_{7/2}$ | 806 | $5.64\times10^{-1}$ | | | $^6F_{11/2}$ | 506 | $4.79\times10^{-4}$ |
| | | $^4F_{5/2}$ | 961 | $8.02\times10^{-2}$ | | | $^4I_{11/2}$ | 1105 | $6.67\times10^{-4}$ |
| | | $(^6P,\,^4P)_{5/2}$ | 1145 | $1.47\times10^{-1}$ | | | $^4M_{15/2}$ | 1114 | $3.99\times10^{-2}$ |
| | | $^6P_{3/2}$ | 1269 | $4.34\times10^{-1}$ | | | $(^4K,\,^4I)_{13/2}$ | 1143 | $1.06\times10^{-1}$ |
| | | $^4F_{7/2}$ | 1300 | $3.3\times10^{-1}$ | | | $(^4I,\,^4K)_{15/2}$ | 1411 | $1.1\times10^{-1}$ |
| | | $^6P_{7/2}$ | 1629 | 1.71 | $^4G_{9/2}$ | 30108 | $^6H_{7/2}$ | 344 | $1.19\times10^{-1}$ |
| $(^2K,\,^2L)_{15/2}$ | 32362 | $^6H_{13/2}$ | 366 | $2.02\times10^{-1}$ | | | $^6H_{9/2}$ | 359 | $2.58\times10^{-1}$ |
| | | $^6H_{15/2}$ | 386 | $6.5\times10^{-1}$ | | | $^6H_{11/2}$ | 378 | $8.56\times10^{-1}$ |
| | | $^4M_{15/2}$ | 894 | $3.89\times10^{-1}$ | | | $^6F_{7/2}$ | 447 | 2.03 |
| | | $(^4K,\,^4I)_{13/2}$ | 913 | $6.73\times10^{-1}$ | | | $^6F_{9/2}$ | 473 | 4.53 |
| | | $^4M_{17/2}$ | 1016 | $7.53\times10^{-1}$ | | | $^6F_{11/2}$ | 507 | $3.34\times10^{-1}$ |
| | | $(^4I,\,^4K)_{15/2}$ | 1076 | 4.89 | | | $^4G_{7/2}$ | 1006 | $1.51\times10^{-1}$ |
| | | $^4L_{13/2}$ | 1334 | 2.27 | | | $^4I_{11/2}$ | 1111 | $3.64\times10^{-2}$ |
| | | $(^4L,\,^4I)_{15/2}$ | 1371 | $9.47\times10^{-1}$ | | | $^4I_{9/2}$ | 1156 | $1.64\times10^{-1}$ |
| | | $^4L_{17/2}$ | 1555 | $2.48\times10^{-1}$ | | | $^4G_{9/2}$ | 1358 | $4.15\times10^{-2}$ |
| | | $^4K_{13/2}$ | 1670 | $1.74\times10^{-2}$ | $^4G_{5/2}$ | 30079 | $^6H_{5/2}$ | 332 | $2.28\times10^{-1}$ |
| $^4G_{11/2}$ | 31358 | $^6H_{9/2}$ | 344 | $1.71\times10^{-1}$ | | | $^6H_{7/2}$ | 345 | $2.98\times10^{-1}$ |
| | | $^6H_{11/2}$ | 361 | $1.85\times10^{-1}$ | | | $^6F_{3/2}$ | 423 | 1.22 |
| | | $^6H_{13/2}$ | 380 | $3.04\times10^{-1}$ | | | $^6F_{5/2}$ | 431 | 1.52 |
| | | $^6F_{9/2}$ | 447 | 1.45 | | | $^6F_{7/2}$ | 448 | $2.29\times10^{-1}$ |
| | | $^6F_{11/2}$ | 477 | 7.14 | | | $^4G_{5/2}$ | 836 | $1.32\times10^{-1}$ |
| | | $^4I_{11/2}$ | 976 | $3.46\times10^{-2}$ | | | $^4F_{3/2}$ | 896 | $1.92\times10^{-1}$ |

[a] The emission rate, $A_{md}$, inside a host material with refractive index $n_r$ would be: $A_{md} = A'_{md}\, n_r^3$

TABLE S5: Continued: $Sm^{3+}$ MD spontaneous emission lines between 300 and 1700 nm.

| $SLJ$ | $E_{SLJ}(cm^{-1})$ | $S'L'J'$ | $\lambda$ (nm) | $A'_{md}$ $(s^{-1})$ [a] | $SLJ$ | $E_{SLJ}(cm^{-1})$ | $S'L'J'$ | $\lambda$ (nm) | $A'_{md}$ $(s^{-1})$ [a] |
|---|---|---|---|---|---|---|---|---|---|
| $^4G_{5/2}$ | 30079 | $^4G_{7/2}$ | 1009 | $3.7 \times 10^{-1}$ | $^4D_{7/2}$ | 28813 | $^4I_{9/2}$ | 1359 | $4.74 \times 10^{-4}$ |
| | | $^4F_{5/2}$ | 1266 | $2.13 \times 10^{-2}$ | | | $^4F_{5/2}$ | 1507 | $3.4 \times 10^{-2}$ |
| | | $\left(^6P,\, ^4P\right)_{5/2}$ | 1605 | $1.11 \times 10^{-2}$ | | | $^4G_{9/2}$ | 1647 | $2.1 \times 10^{-2}$ |
| $^4G_{7/2}$ | 29992 | $^6H_{5/2}$ | 333 | $2.81 \times 10^{-5}$ | $^4H_{7/2}$ | 28715 | $^6H_{5/2}$ | 348 | $1.71 \times 10^{-1}$ |
| | | $^6H_{7/2}$ | 346 | $2.16 \times 10^{-1}$ | | | $^6H_{7/2}$ | 362 | $5.86 \times 10^{-2}$ |
| | | $^6H_{9/2}$ | 361 | $7.39 \times 10^{-1}$ | | | $^6H_{9/2}$ | 378 | $1.68 \times 10^{-2}$ |
| | | $^6F_{5/2}$ | 433 | 2.03 | | | $^6F_{5/2}$ | 458 | $1.66 \times 10^{-2}$ |
| | | $^6F_{7/2}$ | 450 | 3.29 | | | $^6F_{7/2}$ | 477 | $1.66 \times 10^{-2}$ |
| | | $^6F_{9/2}$ | 476 | $2.93 \times 10^{-1}$ | | | $^6F_{9/2}$ | 506 | $1.51 \times 10^{-2}$ |
| | | $^4G_{5/2}$ | 842 | $4.81 \times 10^{-1}$ | | | $^4G_{5/2}$ | 943 | $4.16 \times 10^{-1}$ |
| | | $^4G_{7/2}$ | 1018 | $3.6 \times 10^{-2}$ | | | $^4G_{7/2}$ | 1170 | $2.66 \times 10^{-1}$ |
| | | $^4I_{9/2}$ | 1171 | $4.46 \times 10^{-2}$ | | | $^4I_{9/2}$ | 1377 | $1.05 \times 10^{-1}$ |
| | | $^4F_{5/2}$ | 1280 | $1.13 \times 10^{-1}$ | | | $^4F_{5/2}$ | 1530 | $5.96 \times 10^{-2}$ |
| | | $^4G_{9/2}$ | 1379 | $1.97 \times 10^{-1}$ | | | $^4G_{9/2}$ | 1674 | $1.06 \times 10^{-1}$ |
| | | $\left(^6P,\, ^4P\right)_{5/2}$ | 1628 | $6.51 \times 10^{-3}$ | $^4K_{17/2}$ | 28173 | $^6H_{15/2}$ | 460 | $8.06 \times 10^{-2}$ |
| $^4H_{11/2}$ | 29711 | $^6H_{9/2}$ | 364 | $3.38 \times 10^{-1}$ | | | $^4M_{15/2}$ | 1430 | $2.37 \times 10^{-2}$ |
| | | $^6H_{11/2}$ | 383 | $3.88 \times 10^{-2}$ | $^4K_{15/2}$ | 27936 | $^6H_{13/2}$ | 437 | $3.93 \times 10^{-1}$ |
| | | $^6H_{13/2}$ | 406 | 2.79 | | | $^6H_{15/2}$ | 465 | $7.15 \times 10^{-1}$ |
| | | $^6F_{9/2}$ | 482 | $1.81 \times 10^{-3}$ | | | $^4M_{15/2}$ | 1480 | $3.03 \times 10^{-3}$ |
| | | $^6F_{11/2}$ | 518 | $3.05 \times 10^{-2}$ | | | $\left(^4K,\, ^4I\right)_{13/2}$ | 1531 | $1.46 \times 10^{-1}$ |
| | | $^4I_{11/2}$ | 1162 | $1.53 \times 10^{-1}$ | $\left(^4D,\, ^6P\right)_{5/2}$ | 27469 | $^6H_{5/2}$ | 364 | $5.43 \times 10^{-4}$ |
| | | $\left(^4K,\, ^4I\right)_{13/2}$ | 1204 | $1.81 \times 10^{-2}$ | | | $^6H_{7/2}$ | 379 | $1.97 \times 10^{-3}$ |
| | | $^4I_{9/2}$ | 1211 | $2.95 \times 10^{-2}$ | | | $^6F_{3/2}$ | 475 | $3.2 \times 10^{-1}$ |
| | | $^4G_{9/2}$ | 1435 | $7.63 \times 10^{-2}$ | | | $^6F_{5/2}$ | 486 | $1.6 \times 10^{-1}$ |
| $^4H_{9/2}$ | 29282 | $^6H_{7/2}$ | 354 | 1.17 | | | $^6F_{7/2}$ | 507 | 3.28 |
| | | $^6H_{9/2}$ | 370 | $3. \times 10^{-2}$ | | | $^4G_{5/2}$ | 1069 | $1.75 \times 10^{-1}$ |
| | | $^6H_{11/2}$ | 390 | 1.57 | | | $^4F_{3/2}$ | 1169 | $1.87 \times 10^{-1}$ |
| | | $^6F_{7/2}$ | 465 | $2.88 \times 10^{-2}$ | | | $^4G_{7/2}$ | 1370 | $1.04 \times 10^{-1}$ |
| | | $^6F_{9/2}$ | 492 | $7.77 \times 10^{-4}$ | $^4F_{9/2}$ | 27421 | $^6H_{7/2}$ | 379 | $2.28 \times 10^{-2}$ |
| | | $^6F_{11/2}$ | 530 | $1.28 \times 10^{-1}$ | | | $^6H_{9/2}$ | 398 | $4.91 \times 10^{-2}$ |
| | | $^4G_{7/2}$ | 1098 | $3.75 \times 10^{-1}$ | | | $^6H_{11/2}$ | 420 | $4.53 \times 10^{-1}$ |
| | | $^4I_{11/2}$ | 1223 | $6.44 \times 10^{-2}$ | | | $^6F_{7/2}$ | 509 | $6.04 \times 10^{-1}$ |
| | | $^4I_{9/2}$ | 1278 | $5.5 \times 10^{-2}$ | | | $^6F_{9/2}$ | 542 | $7.18 \times 10^{-1}$ |
| | | $^4G_{9/2}$ | 1529 | $2.05 \times 10^{-1}$ | | | $^6F_{11/2}$ | 588 | 3.39 |
| $^4L_{19/2}$ | 29230 | $^4M_{17/2}$ | 1491 | $5.12 \times 10^{-4}$ | | | $^4G_{7/2}$ | 1379 | $4.24 \times 10^{-2}$ |
| $^4D_{7/2}$ | 28813 | $^6H_{5/2}$ | 347 | $2. \times 10^{-4}$ | | | $^4I_{11/2}$ | 1584 | $2.75 \times 10^{-4}$ |
| | | $^6H_{7/2}$ | 360 | $3.63 \times 10^{-6}$ | | | $^4I_{9/2}$ | 1676 | $1.59 \times 10^{-2}$ |
| | | $^6H_{9/2}$ | 377 | $5.15 \times 10^{-3}$ | $^4D_{3/2}$ | 27403 | $^6H_{5/2}$ | 365 | $3.27 \times 10^{-3}$ |
| | | $^6F_{5/2}$ | 456 | $5.05 \times 10^{-2}$ | | | $^6F_{1/2}$ | 472 | $6.88 \times 10^{-1}$ |
| | | $^6F_{7/2}$ | 475 | $1. \times 10^{-1}$ | | | $^6F_{3/2}$ | 476 | $7.09 \times 10^{-1}$ |
| | | $^6F_{9/2}$ | 504 | 2.03 | | | $^6F_{5/2}$ | 487 | 5.44 |
| | | $^4G_{5/2}$ | 935 | $3.05 \times 10^{-2}$ | | | $^4G_{5/2}$ | 1077 | $1.94 \times 10^{-1}$ |
| | | $^4G_{7/2}$ | 1157 | $5.96 \times 10^{-3}$ | | | $^4F_{3/2}$ | 1179 | $2.59 \times 10^{-1}$ |

[a] The emission rate, $A_{md}$, inside a host material with refractive index $n_r$ would be: $A_{md} = A'_{md}\, n_r^3$

TABLE S5: Continued: $Sm^{3+}$ MD spontaneous emission lines between 300 and 1700 nm.

| $SLJ$ | $E_{SLJ}(cm^{-1})$ | $S'L'J'$ | $\lambda$ (nm) | $A'_{md}$ $(s^{-1})$ [a] | $SLJ$ | $E_{SLJ}(cm^{-1})$ | $S'L'J'$ | $\lambda$ (nm) | $A'_{md}$ $(s^{-1})$ [a] |
|---|---|---|---|---|---|---|---|---|---|
| $^6P_{7/2}$ | 26443 | $^6H_{5/2}$ | 378 | $1.73 \times 10^{-3}$ | $^6P_{3/2}$ | 24698 | $^4G_{5/2}$ | 1519 | $2.78 \times 10^{-2}$ |
| | | $^6H_{7/2}$ | 394 | $1.16 \times 10^{-2}$ | $(^6P, ^4P)_{5/2}$ | 23849 | $^6H_{5/2}$ | 419 | $1.55 \times 10^{-2}$ |
| | | $^6H_{9/2}$ | 414 | $8.21 \times 10^{-2}$ | | | $^6H_{7/2}$ | 439 | $5.19 \times 10^{-2}$ |
| | | $^6F_{5/2}$ | 511 | $1.38 \times 10^{-3}$ | | | $^6F_{3/2}$ | 574 | $4.68 \times 10^{-2}$ |
| | | $^6F_{7/2}$ | 535 | $2.45 \times 10^{-1}$ | | | $^6F_{5/2}$ | 589 | $5.24 \times 10^{-1}$ |
| | | $^6F_{9/2}$ | 572 | $5.07 \times 10^{-1}$ | | | $^6F_{7/2}$ | 621 | $8.74 \times 10^{-1}$ |
| | | $^4G_{5/2}$ | 1201 | $1.01 \times 10^{-2}$ | $(^4I, ^4K)_{15/2}$ | 23072 | $^6H_{13/2}$ | 555 | $7.01 \times 10^{-1}$ |
| | | $^4G_{7/2}$ | 1595 | $1.43 \times 10^{-3}$ | | | $^6H_{15/2}$ | 602 | 2.99 |
| $^4K_{13/2}$ | 26375 | $^6H_{11/2}$ | 440 | $5.82 \times 10^{-1}$ | $^4G_{9/2}$ | 22742 | $^6H_{7/2}$ | 461 | $1.18 \times 10^{-2}$ |
| | | $^6H_{13/2}$ | 469 | $6.61 \times 10^{-1}$ | | | $^6H_{9/2}$ | 489 | $6.4 \times 10^{-1}$ |
| | | $^6H_{15/2}$ | 502 | $1.52 \times 10^{-2}$ | | | $^6H_{11/2}$ | 523 | 3.96 |
| | | $^6F_{11/2}$ | 626 | $6.64 \times 10^{-5}$ | | | $^6F_{7/2}$ | 667 | $3.11 \times 10^{-3}$ |
| $^4D_{1/2}$ | 26269 | $^6F_{1/2}$ | 499 | 1.54 | | | $^6F_{9/2}$ | 726 | $2.94 \times 10^{-1}$ |
| | | $^6F_{3/2}$ | 504 | 5.93 | | | $^6F_{11/2}$ | 810 | $6.23 \times 10^{-1}$ |
| | | $^4F_{3/2}$ | 1360 | $2.85 \times 10^{-1}$ | $^4M_{17/2}$ | 22523 | $^6H_{15/2}$ | 622 | $4.76 \times 10^{-3}$ |
| $^4L_{17/2}$ | 25931 | $^6H_{15/2}$ | 513 | $4.89 \times 10^{-2}$ | $^4F_{5/2}$ | 22177 | $^6H_{5/2}$ | 451 | 1.48 |
| $^4G_{11/2}$ | 25628 | $^6H_{9/2}$ | 428 | $2.04 \times 10^{-3}$ | | | $^6H_{7/2}$ | 474 | 2.26 |
| | | $^6H_{11/2}$ | 454 | $8.72 \times 10^{-2}$ | | | $^6F_{3/2}$ | 634 | $9.78 \times 10^{-1}$ |
| | | $^6H_{13/2}$ | 486 | 1.53 | | | $^6F_{5/2}$ | 654 | $1.66 \times 10^{-1}$ |
| | | $^6F_{9/2}$ | 600 | $1.67 \times 10^{-1}$ | | | $^6F_{7/2}$ | 693 | 1.24 |
| | | $^6F_{11/2}$ | 657 | $4.37 \times 10^{-2}$ | $^4I_{9/2}$ | 21456 | $^6H_{7/2}$ | 491 | 1.35 |
| $(^4L, ^4I)_{15/2}$ | 25070 | $^6H_{13/2}$ | 500 | $7.95 \times 10^{-1}$ | | | $^6H_{9/2}$ | 521 | $8.86 \times 10^{-1}$ |
| | | $^6H_{15/2}$ | 537 | 2.16 | | | $^6H_{11/2}$ | 561 | $2.34 \times 10^{-1}$ |
| $^4K_{11/2}$ | 24905 | $^6H_{9/2}$ | 442 | 1.24 | | | $^6F_{7/2}$ | 730 | $1.11 \times 10^{-3}$ |
| | | $^6H_{11/2}$ | 470 | 1.04 | | | $^6F_{9/2}$ | 801 | $2.94 \times 10^{-3}$ |
| | | $^6H_{13/2}$ | 504 | $1.57 \times 10^{-1}$ | | | $^6F_{11/2}$ | 905 | $1.82 \times 10^{-4}$ |
| | | $^6F_{9/2}$ | 627 | $1.28 \times 10^{-3}$ | $(^4K, ^4I)_{13/2}$ | 21406 | $^6H_{11/2}$ | 562 | 1.43 |
| | | $^6F_{11/2}$ | 690 | $3.76 \times 10^{-3}$ | | | $^6H_{13/2}$ | 612 | 2.31 |
| $^4F_{7/2}$ | 24889 | $^6H_{5/2}$ | 402 | $5.34 \times 10^{-2}$ | | | $^6H_{15/2}$ | 669 | $5.77 \times 10^{-2}$ |
| | | $^6H_{7/2}$ | 420 | $4.32 \times 10^{-1}$ | | | $^6F_{11/2}$ | 909 | $2.49 \times 10^{-4}$ |
| | | $^6H_{9/2}$ | 442 | 2.24 | $^4M_{15/2}$ | 21181 | $^6H_{13/2}$ | 621 | $1.18 \times 10^{-1}$ |
| | | $^6F_{5/2}$ | 555 | $6.95 \times 10^{-1}$ | | | $^6H_{15/2}$ | 679 | $5.27 \times 10^{-1}$ |
| | | $^6F_{7/2}$ | 584 | $1.88 \times 10^{-1}$ | $^4I_{11/2}$ | 21107 | $^6H_{9/2}$ | 531 | 1.84 |
| | | $^6F_{9/2}$ | 628 | 2.71 | | | $^6H_{11/2}$ | 572 | 1.68 |
| | | $^4G_{5/2}$ | 1476 | $3.6 \times 10^{-2}$ | | | $^6H_{13/2}$ | 623 | $1.52 \times 10^{-1}$ |
| $^4L_{13/2}$ | 24865 | $^6H_{11/2}$ | 471 | 1.25 | | | $^6F_{9/2}$ | 824 | $1.34 \times 10^{-4}$ |
| | | $^6H_{13/2}$ | 505 | 1.7 | | | $^6F_{11/2}$ | 934 | $2.58 \times 10^{-3}$ |
| | | $^6H_{15/2}$ | 543 | $4.82 \times 10^{-2}$ | $^4G_{7/2}$ | 20172 | $^6H_{5/2}$ | 496 | $2.04 \times 10^{-1}$ |
| | | $^6F_{11/2}$ | 691 | $3.14 \times 10^{-4}$ | | | $^6H_{7/2}$ | 523 | 1.59 |
| $^6P_{3/2}$ | 24698 | $^6H_{5/2}$ | 405 | $5.29 \times 10^{-4}$ | | | $^6H_{9/2}$ | 559 | 4.66 |
| | | $^6F_{1/2}$ | 541 | $9.92 \times 10^{-2}$ | | | $^6F_{5/2}$ | 753 | $4.48 \times 10^{-1}$ |
| | | $^6F_{3/2}$ | 547 | $2.34 \times 10^{-1}$ | | | $^6F_{7/2}$ | 805 | $9.02 \times 10^{-1}$ |
| | | $^6F_{5/2}$ | 561 | $3.83 \times 10^{-1}$ | | | $^6F_{9/2}$ | 892 | $6.6 \times 10^{-1}$ |

[a] The emission rate, $A_{md}$, inside a host material with refractive index $n_r$ would be: $A_{md} = A'_{md}\ n_r^3$

TABLE S5: Continued: $Sm^{3+}$ MD spontaneous emission lines between 300 and 1700 nm.

| $SLJ$ | $E_{SLJ}(cm^{-1})$ | $S'L'J'$ | $\lambda$ (nm) | $A'_{md}$ $(s^{-1})$ [a] | $SLJ$ | $E_{SLJ}(cm^{-1})$ | $S'L'J'$ | $\lambda$ (nm) | $A'_{md}$ $(s^{-1})$ [a] |
|---|---|---|---|---|---|---|---|---|---|
| $^4F_{3/2}$ | 18918 | $^6H_{5/2}$ | 529 | $1.16 \times 10^{-1}$ | $^6F_{11/2}$ | 10402 | $^6H_{9/2}$ | 1230 | $5.77 \times 10^{-5}$ |
| | | $^6F_{1/2}$ | 787 | 3.93 | | | $^6H_{11/2}$ | 1475 | $1.45 \times 10^{-3}$ |
| | | $^6F_{3/2}$ | 800 | 1.64 | $^6F_{9/2}$ | 8964 | $^6H_{7/2}$ | 1267 | $5.4 \times 10^{-5}$ |
| | | $^6F_{5/2}$ | 831 | $1.28 \times 10^{-1}$ | | | $^6H_{9/2}$ | 1495 | $7.92 \times 10^{-3}$ |
| $^4G_{5/2}$ | 18115 | $^6H_{5/2}$ | 552 | 3.79 | $^6F_{7/2}$ | 7756 | $^6H_{5/2}$ | 1289 | $1.03 \times 10^{-3}$ |
| | | $^6H_{7/2}$ | 587 | 3.14 | | | $^6H_{7/2}$ | 1496 | $2.16 \times 10^{-2}$ |
| | | $^6F_{3/2}$ | 855 | 1.65 | $^6F_{5/2}$ | 6883 | $^6H_{5/2}$ | 1453 | $3.35 \times 10^{-2}$ |
| | | $^6F_{5/2}$ | 890 | 1.19 | $^6F_{3/2}$ | 6416 | $^6H_{5/2}$ | 1559 | $1.03 \times 10^{-2}$ |
| | | $^6F_{7/2}$ | 965 | $3.79 \times 10^{-1}$ | | | | | |

[a] The emission rate, $A_{md}$, inside a host material with refractive index $n_r$ would be: $A_{md} = A'_{md}\ n_r^3$

TABLE S6: Calculated $Eu^{3+}$ MD spontaneous emission lines between 300 and 1700 nm.

| $SLJ$ | $E_{SLJ}(cm^{-1})$ | $S'L'J'$ | $\lambda$ (nm) | $A'_{md}$ $(s^{-1})$ [a] | $SLJ$ | $E_{SLJ}(cm^{-1})$ | $S'L'J'$ | $\lambda$ (nm) | $A'_{md}$ $(s^{-1})$ [a] |
|---|---|---|---|---|---|---|---|---|---|
| $({}^5D, {}^5P)_2$ | 39979 | ${}^5D_1$ | 483 | $1.11 \times 10^{-1}$ | ${}^3P_1$ | 38891 | ${}^5D_0$ | 468 | $7.69 \times 10^{-1}$ |
| | | ${}^5D_2$ | 549 | $7.22 \times 10^{-2}$ | | | ${}^5D_1$ | 510 | $1.06 \times 10^{-4}$ |
| | | ${}^5D_3$ | 653 | $1.45 \times 10^{-1}$ | | | ${}^5D_2$ | 583 | $1.6 \times 10^{1}$ |
| | | ${}^5G_2$ | 738 | $4.05 \times 10^{-5}$ | | | ${}^5G_2$ | 802 | $2.47 \times 10^{-4}$ |
| | | ${}^5G_3$ | 750 | $6.43 \times 10^{-3}$ | ${}^5G_2$ | 38784 | ${}^5D_1$ | 512 | $4.86 \times 10^{-1}$ |
| | | ${}^5H_3$ | 1182 | $2.46 \times 10^{-2}$ | | | ${}^5D_2$ | 587 | $6.13 \times 10^{-1}$ |
| | | ${}^5F_2$ | 1489 | $2.08 \times 10^{-1}$ | | | ${}^5D_3$ | 709 | $1.74 \times 10^{-1}$ |
| | | ${}^5F_3$ | 1497 | $1.95 \times 10^{-2}$ | | | ${}^5G_2$ | 809 | $5.56 \times 10^{-1}$ |
| | | ${}^5F_1$ | 1607 | $4.33 \times 10^{-1}$ | | | ${}^5G_3$ | 824 | $3.33 \times 10^{-1}$ |
| $({}^3I, {}^3H)_6$ | 39890 | ${}^5L_6$ | 695 | $7.37 \times 10^{-1}$ | | | ${}^5H_3$ | 1376 | $8.65 \times 10^{-2}$ |
| | | ${}^5L_7$ | 733 | 1.92 | ${}^5K_7$ | 38468 | ${}^5L_6$ | 771 | $6.01 \times 10^{-2}$ |
| | | ${}^5G_5$ | 771 | 1.62 | | | ${}^5L_7$ | 818 | $6.04 \times 10^{-1}$ |
| | | ${}^5G_6$ | 776 | 5.51 | | | ${}^5G_6$ | 872 | $2.78 \times 10^{-4}$ |
| | | ${}^5H_7$ | 1197 | $5.56 \times 10^{-2}$ | | | ${}^5L_8$ | 875 | $4.43 \times 10^{-2}$ |
| | | ${}^5H_6$ | 1224 | $2.5 \times 10^{-1}$ | | | ${}^5H_7$ | 1443 | $8.74 \times 10^{-2}$ |
| | | ${}^5H_5$ | 1234 | $5.19 \times 10^{-2}$ | | | ${}^5H_6$ | 1482 | $2.95 \times 10^{-3}$ |
| ${}^5K_9$ | 39879 | ${}^5L_8$ | 779 | $1.96 \times 10^{-2}$ | ${}^5K_6$ | 37516 | ${}^7F_6$ | 308 | $5.19 \times 10^{-3}$ |
| | | ${}^5L_9$ | 842 | $3.66 \times 10^{-1}$ | | | ${}^5L_6$ | 832 | $8.64 \times 10^{-1}$ |
| | | ${}^5L_{10}$ | 889 | $5.87 \times 10^{-1}$ | | | ${}^5L_7$ | 888 | $2.6 \times 10^{-2}$ |
| ${}^5G_4$ | 39796 | ${}^5D_3$ | 661 | $6.66 \times 10^{-2}$ | | | ${}^5G_5$ | 944 | $4.18 \times 10^{-2}$ |
| | | ${}^5G_3$ | 761 | $4.25 \times 10^{-1}$ | | | ${}^5G_6$ | 951 | $3.38 \times 10^{-1}$ |
| | | ${}^5G_4$ | 772 | $2.32 \times 10^{-2}$ | | | ${}^5H_7$ | 1673 | $2.64 \times 10^{-2}$ |
| | | ${}^5G_5$ | 777 | $3.02 \times 10^{-1}$ | ${}^5K_5$ | 36713 | ${}^7F_5$ | 306 | $1.16 \times 10^{-2}$ |
| | | ${}^5D_4$ | 845 | $9.86 \times 10^{-2}$ | | | ${}^7F_6$ | 316 | $4.9 \times 10^{-5}$ |
| | | ${}^5H_3$ | 1208 | $7.64 \times 10^{-7}$ | | | ${}^5L_6$ | 892 | $9.4 \times 10^{-1}$ |
| | | ${}^5H_4$ | 1238 | $8.79 \times 10^{-2}$ | | | ${}^5G_4$ | 1014 | $1.85 \times 10^{-2}$ |
| | | ${}^5H_5$ | 1248 | $1.44 \times 10^{-2}$ | | | ${}^5G_5$ | 1021 | $3.94 \times 10^{-2}$ |
| | | ${}^5F_3$ | 1539 | $1.19 \times 10^{-2}$ | | | ${}^5G_6$ | 1030 | $4.65 \times 10^{-2}$ |
| | | ${}^5F_4$ | 1669 | $6.64 \times 10^{-1}$ | | | ${}^5D_4$ | 1143 | $5.19 \times 10^{-4}$ |
| ${}^5G_3$ | 39296 | ${}^5D_2$ | 570 | $2.88 \times 10^{-1}$ | $({}^5I, {}^5H)_7$ | 35592 | ${}^7F_6$ | 327 | $2.52 \times 10^{-2}$ |
| | | ${}^5D_3$ | 684 | $3.46 \times 10^{-1}$ | | | ${}^5L_6$ | 991 | $1.09 \times 10^{-2}$ |
| | | ${}^5G_2$ | 777 | $7.66 \times 10^{-2}$ | | | ${}^5L_7$ | 1070 | $2.82 \times 10^{-1}$ |
| | | ${}^5G_3$ | 791 | $6.39 \times 10^{-2}$ | | | ${}^5G_6$ | 1164 | $1.51 \times 10^{-2}$ |
| | | ${}^5G_4$ | 803 | $2.01 \times 10^{-2}$ | | | ${}^5L_8$ | 1170 | $1.54 \times 10^{-2}$ |
| | | ${}^5D_4$ | 882 | $4.42 \times 10^{-2}$ | ${}^5I_8$ | 35313 | ${}^5L_7$ | 1103 | $2.53 \times 10^{-3}$ |
| | | ${}^5H_3$ | 1285 | $5.76 \times 10^{-2}$ | | | ${}^5L_8$ | 1209 | $2.36 \times 10^{-1}$ |
| | | ${}^5H_4$ | 1320 | $6.52 \times 10^{-3}$ | | | ${}^5L_9$ | 1367 | $1.98 \times 10^{-1}$ |
| | | ${}^5F_2$ | 1657 | $9. \times 10^{-2}$ | $({}^5I, {}^5H)_6$ | 34868 | ${}^7F_5$ | 324 | $2.69 \times 10^{-2}$ |
| | | ${}^5F_3$ | 1667 | $8.18 \times 10^{-1}$ | | | ${}^7F_6$ | 335 | $3.01 \times 10^{-2}$ |
| ${}^5K_8$ | 39057 | ${}^5L_7$ | 781 | $4.82 \times 10^{-2}$ | | | ${}^5L_6$ | 1068 | $5.73 \times 10^{-1}$ |
| | | ${}^5L_8$ | 832 | $5.25 \times 10^{-1}$ | | | ${}^5L_7$ | 1160 | $9.03 \times 10^{-3}$ |
| | | ${}^5L_9$ | 904 | $1.26 \times 10^{-1}$ | | | ${}^5G_5$ | 1258 | $2.46 \times 10^{-1}$ |
| | | ${}^5H_7$ | 1330 | $2.95 \times 10^{-2}$ | | | ${}^5G_6$ | 1272 | $5.8 \times 10^{-1}$ |

[a] The emission rate, $A_{md}$, inside a host material with refractive index $n_r$ would be: $A_{md} = A'_{md}\ n_r^3$

TABLE S6: Continued: $Eu^{3+}$ MD spontaneous emission lines between 300 and 1700 nm.

| $SLJ$ | $E_{SLJ}(cm^{-1})$ | $S'L'J'$ | $\lambda$ (nm) | $A'_{md}$ $(s^{-1})$ [a] | $SLJ$ | $E_{SLJ}(cm^{-1})$ | $S'L'J'$ | $\lambda$ (nm) | $A'_{md}$ $(s^{-1})$ [a] |
|---|---|---|---|---|---|---|---|---|---|
| $^5F_5$ | 34522 | $^7F_4$ | 317 | $8.87 \times 10^{-1}$ | $^5F_3$ | 33297 | $^5G_2$ | 1455 | $1.95 \times 10^{-2}$ |
| | | $^7F_5$ | 328 | 1.42 | | | $^5G_3$ | 1505 | $1.33 \times 10^{-1}$ |
| | | $^7F_6$ | 339 | 5.44 | | | $^5G_4$ | 1551 | $1.4 \times 10^{-1}$ |
| | | $^5L_6$ | 1108 | $1.22 \times 10^{-1}$ | $^5F_2$ | 33261 | $^7F_1$ | 304 | 5.49 |
| | | $^5G_4$ | 1303 | $6.71 \times 10^{-2}$ | | | $^7F_2$ | 311 | 2.74 |
| | | $^5G_5$ | 1316 | $5.21 \times 10^{-2}$ | | | $^7F_3$ | 319 | $8.26 \times 10^{-1}$ |
| | | $^5G_6$ | 1330 | $2.91 \times 10^{-2}$ | | | $^5D_1$ | 714 | $2.45 \times 10^{-1}$ |
| | | $^5D_4$ | 1524 | $3.62 \times 10^{-1}$ | | | $^5D_2$ | 869 | $5.85 \times 10^{-1}$ |
| $^5I_4$ | 34492 | $^7F_3$ | 307 | $1.95 \times 10^{-2}$ | | | $^5D_3$ | 1165 | $2.33 \times 10^{-1}$ |
| | | $^7F_4$ | 317 | $1.3 \times 10^{-2}$ | | | $^5G_2$ | 1463 | $2.36 \times 10^{-1}$ |
| | | $^7F_5$ | 328 | $8.85 \times 10^{-2}$ | | | $^5G_3$ | 1513 | $1.75 \times 10^{-2}$ |
| | | $^5D_3$ | 1019 | $2.72 \times 10^{-4}$ | $^5H_5$ | 31785 | $^7F_4$ | 347 | $6.37 \times 10^{-1}$ |
| | | $^5G_3$ | 1275 | $1.28 \times 10^{-1}$ | | | $^7F_5$ | 360 | 1.43 |
| | | $^5G_4$ | 1308 | $9.65 \times 10^{-2}$ | | | $^7F_6$ | 374 | $1.59 \times 10^{-1}$ |
| | | $^5G_5$ | 1321 | $4.44 \times 10^{-2}$ | | | $^5L_6$ | 1591 | $1.13 \times 10^{-1}$ |
| | | $^5D_4$ | 1531 | $4.72 \times 10^{-4}$ | $^5H_6$ | 31721 | $^7F_5$ | 361 | $5.81 \times 10^{-1}$ |
| $(^5I,\, ^5K)_5$ | 34361 | $^7F_4$ | 318 | $3.57 \times 10^{-1}$ | | | $^7F_6$ | 375 | 1.69 |
| | | $^7F_5$ | 329 | $5.73 \times 10^{-1}$ | | | $^5L_6$ | 1608 | $7.63 \times 10^{-2}$ |
| | | $^7F_6$ | 341 | $8.4 \times 10^{-1}$ | $^5H_4$ | 31721 | $^7F_3$ | 336 | $3.84 \times 10^{-1}$ |
| | | $^5L_6$ | 1129 | $5.18 \times 10^{-1}$ | | | $^7F_4$ | 347 | $7.4 \times 10^{-1}$ |
| | | $^5G_4$ | 1331 | $1.8 \times 10^{-1}$ | | | $^7F_5$ | 361 | $1.99 \times 10^{-1}$ |
| | | $^5G_5$ | 1344 | $1.26 \times 10^{-1}$ | | | $^5D_3$ | 1419 | $1.06 \times 10^{-3}$ |
| | | $^5G_6$ | 1359 | $9.49 \times 10^{-4}$ | $^5H_7$ | 31537 | $^7F_6$ | 377 | $1.27 \times 10^{-1}$ |
| | | $^5D_4$ | 1562 | $3.82 \times 10^{-2}$ | | | $^5L_6$ | 1657 | $9.14 \times 10^{-3}$ |
| $^5F_4$ | 33804 | $^7F_3$ | 314 | 3.12 | $^5H_3$ | 31517 | $^7F_2$ | 328 | $8.43 \times 10^{-2}$ |
| | | $^7F_4$ | 324 | 2.68 | | | $^7F_3$ | 338 | $2.02 \times 10^{-1}$ |
| | | $^7F_5$ | 336 | 5.62 | | | $^7F_4$ | 350 | $1.48 \times 10^{-1}$ |
| | | $^5D_3$ | 1095 | $1.16 \times 10^{-2}$ | | | $^5D_2$ | 1024 | $9.06 \times 10^{-6}$ |
| | | $^5G_3$ | 1398 | $2.16 \times 10^{-2}$ | | | $^5D_3$ | 1462 | $1.26 \times 10^{-4}$ |
| | | $^5G_4$ | 1438 | $4.49 \times 10^{-2}$ | $^5D_4$ | 27961 | $^7F_3$ | 384 | $3.5 \times 10^{-2}$ |
| | | $^5G_5$ | 1453 | $8.75 \times 10^{-2}$ | | | $^7F_4$ | 399 | $2.38 \times 10^{-1}$ |
| $^5F_1$ | 33755 | $^7F_2$ | 306 | $4.38 \times 10^{-2}$ | | | $^7F_5$ | 417 | 5.47 |
| | | $^5D_0$ | 616 | $9.36 \times 10^{-1}$ | $^5G_6$ | 27005 | $^7F_5$ | 435 | 1.76 |
| | | $^5D_1$ | 690 | 1.39 | | | $^7F_6$ | 455 | $1.05 \times 10^{1}$ |
| | | $^5D_2$ | 833 | $4.94 \times 10^{-1}$ | $^5G_5$ | 26922 | $^7F_4$ | 417 | 2.52 |
| | | $^5G_2$ | 1364 | $2.53 \times 10^{-1}$ | | | $^7F_5$ | 436 | 8.3 |
| $^3P_0$ | 33559 | $^7F_1$ | 302 | $1.87 \times 10^{-1}$ | | | $^7F_6$ | 457 | $9.66 \times 10^{-1}$ |
| | | $^5D_1$ | 700 | $2.46 \times 10^{1}$ | $^5G_4$ | 26848 | $^7F_3$ | 401 | 2.7 |
| $^5F_3$ | 33297 | $^7F_2$ | 310 | 4.76 | | | $^7F_4$ | 418 | 6.31 |
| | | $^7F_3$ | 319 | 2.81 | | | $^7F_5$ | 438 | $6.31 \times 10^{-1}$ |
| | | $^7F_4$ | 329 | 3.04 | $^5G_3$ | 26652 | $^7F_2$ | 391 | 2.39 |
| | | $^5D_2$ | 866 | $2.32 \times 10^{-2}$ | | | $^7F_3$ | 405 | 4.59 |
| | | $^5D_3$ | 1160 | $2.65 \times 10^{-1}$ | | | $^7F_4$ | 422 | 1.1 |

[a] The emission rate, $A_{md}$, inside a host material with refractive index $n_r$ would be: $A_{md} = A'_{md}\ n_r^3$

TABLE S6: Continued: $Eu^{3+}$ MD spontaneous emission lines between 300 and 1700 nm.

| $SLJ$ | $E_{SLJ}(cm^{-1})$ | $S'L'J'$ | $\lambda$ (nm) | $A'_{md}$ $(s^{-1})$ [a] | $SLJ$ | $E_{SLJ}(cm^{-1})$ | $S'L'J'$ | $\lambda$ (nm) | $A'_{md}$ $(s^{-1})$ [a] |
|---|---|---|---|---|---|---|---|---|---|
| $^5G_2$ | 26423 | $^7F_1$ | 384 | 1.67 | $^5D_3$ | 24675 | $^7F_4$ | 460 | 9.02 |
| | | $^7F_2$ | 394 | 2.49 | $^5D_2$ | 21752 | $^7F_1$ | 468 | $5.37 \times 10^{-1}$ |
| | | $^7F_3$ | 408 | $4.34 \times 10^{-1}$ | | | $^7F_2$ | 483 | $5.8 \times 10^{-3}$ |
| | | $^5D_1$ | 1397 | $2.68 \times 10^{-3}$ | | | $^7F_3$ | 505 | $1.16 \times 10^{1}$ |
| $^5L_7$ | 26250 | $^7F_6$ | 471 | $5.54 \times 10^{-4}$ | $^5D_1$ | 19264 | $^7F_0$ | 519 | 1.4 |
| $^5L_6$ | 25501 | $^7F_5$ | 465 | $3.4 \times 10^{-2}$ | | | $^7F_1$ | 530 | $1.62 \times 10^{-3}$ |
| | | $^7F_6$ | 489 | $2.24 \times 10^{-1}$ | | | $^7F_2$ | 550 | 12.29 |
| $^5D_3$ | 24675 | $^7F_2$ | 424 | $1.35 \times 10^{-1}$ | $^5D_0$ | 17521 | $^7F_1$ | 584 | 14.37 |
| | | $^7F_3$ | 440 | $2.32 \times 10^{-3}$ | | | | | |

[a] The emission rate, $A_{md}$, inside a host material with refractive index $n_r$ would be: $A_{md} = A'_{md}\ n_r^3$

TABLE S7: Calculated $Gd^{3+}$ MD spontaneous emission lines between 300 and 1700 nm.

| $SLJ$ | $E_{SLJ}(cm^{-1})$ | $S'L'J'$ | $\lambda$ (nm) | $A'_{md}$ $(s^{-1})$ [a] | $SLJ$ | $E_{SLJ}(cm^{-1})$ | $S'L'J'$ | $\lambda$ (nm) | $A'_{md}$ $(s^{-1})$ [a] |
|---|---|---|---|---|---|---|---|---|---|
| $^6D_{9/2}$ | 39524 | $^6P_{7/2}$ | 1435 | 1.76 | $^6P_{7/2}$ | 32557 | $^8S_{7/2}$ | 307 | $3.02 \times 10^{1}$ |
| $^6P_{5/2}$ | 33169 | $^8S_{7/2}$ | 301 | $2.36 \times 10^{1}$ | | | | | |

[a] The emission rate, $A_{md}$, inside a host material with refractive index $n_r$ would be: $A_{md} = A'_{md}\ n_r^3$

TABLE S8: Calculated $Tb^{3+}$ MD spontaneous emission lines between 300 and 1700 nm.

| $SLJ$ | $E_{SLJ}(cm^{-1})$ | $S'L'J'$ | $\lambda$ (nm) | $A'_{md}$ $(s^{-1})$ [a] | $SLJ$ | $E_{SLJ}(cm^{-1})$ | $S'L'J'$ | $\lambda$ (nm) | $A'_{md}$ $(s^{-1})$ [a] |
|---|---|---|---|---|---|---|---|---|---|
| $(^5D,\,^3P)_2$ | 39740 | $^5D_3$ | 766 | $1.75 \times 10^{1}$ | $^5F_3$ | 36930 | $^5D_4$ | 623 | $1.98 \times 10^{-2}$ |
| | | $^5D_2$ | 907 | $5.74 \times 10^{-2}$ | | | $^5D_3$ | 977 | $7.02 \times 10^{-1}$ |
| | | $^5G_3$ | 957 | $7.36 \times 10^{-2}$ | | | $^5G_4$ | 1211 | $1.42 \times 10^{-2}$ |
| | | $^5G_2$ | 1005 | $5.36 \times 10^{-4}$ | | | $^5D_2$ | 1217 | $1.07 \times 10^{-2}$ |
| | | $^5D_1$ | 1171 | 1.13 | | | $^5G_3$ | 1310 | $1.69 \times 10^{-2}$ |
| $^5K_9$ | 39358 | $^5L_{10}$ | 825 | 1.56 | | | $^5G_2$ | 1401 | $6.41 \times 10^{-5}$ |
| | | $^5L_9$ | 944 | $5.08 \times 10^{-1}$ | $^5F_4$ | 35884 | $^7F_4$ | 306 | 4.01 |
| | | $^5L_8$ | 998 | $2.51 \times 10^{-2}$ | | | $^7F_3$ | 316 | 1.39 |
| $^5I_5$ | 38127 | $^5D_4$ | 580 | $2.06 \times 10^{-3}$ | | | $^5D_4$ | 667 | 1.39 |
| | | $^5G_6$ | 899 | $1.98 \times 10^{-1}$ | | | $^5D_3$ | 1088 | $2.33 \times 10^{-1}$ |
| | | $^5G_5$ | 1013 | $4.64 \times 10^{-1}$ | | | $^5G_5$ | 1310 | $4.3 \times 10^{-1}$ |
| | | $^5G_4$ | 1058 | $3.23 \times 10^{-1}$ | | | $^5G_4$ | 1387 | $4.27 \times 10^{-2}$ |
| | | $^5L_6$ | 1237 | $4.27 \times 10^{-1}$ | | | $^5G_3$ | 1518 | $2.01 \times 10^{-3}$ |
| $^5I_4$ | 37855 | $^5D_4$ | 589 | $1.99 \times 10^{-2}$ | $^5I_8$ | 35528 | $^5L_9$ | 1479 | $5.83 \times 10^{-1}$ |
| | | $^5D_3$ | 896 | $1.99 \times 10^{-2}$ | | | $^5L_8$ | 1614 | $3.63 \times 10^{-1}$ |
| | | $^5G_5$ | 1041 | $4.3 \times 10^{-3}$ | $^5H_3$ | 35510 | $^7F_4$ | 310 | $1.72 \times 10^{-1}$ |
| | | $^5G_4$ | 1089 | $1.42 \times 10^{-1}$ | | | $^7F_3$ | 320 | $5.98 \times 10^{-1}$ |
| | | $^5G_3$ | 1168 | $3.23 \times 10^{-1}$ | | | $^7F_2$ | 327 | $2.53 \times 10^{-1}$ |
| $^5I_6$ | 37759 | $^5G_6$ | 930 | $5.17 \times 10^{-1}$ | | | $^5D_4$ | 684 | $8.26 \times 10^{-4}$ |
| | | $^5G_5$ | 1052 | $2.66 \times 10^{-1}$ | | | $^5D_3$ | 1134 | $9.85 \times 10^{-3}$ |
| | | $^5L_7$ | 1238 | $1.78 \times 10^{-3}$ | | | $^5G_4$ | 1463 | $1.42 \times 10^{-1}$ |
| | | $^5L_6$ | 1296 | $6.73 \times 10^{-1}$ | | | $^5D_2$ | 1471 | $2.67 \times 10^{-2}$ |
| | | $^5H_7$ | 1690 | $1.46 \times 10^{-2}$ | | | $^5G_3$ | 1609 | 1.35 |
| $^5F_1$ | 37752 | $^7F_2$ | 305 | 2.63 | $^5F_5$ | 35441 | $^7F_4$ | 311 | $6.09 \times 10^{-1}$ |
| | | $^7F_1$ | 310 | $1.44 \times 10^{1}$ | | | $^5D_4$ | 687 | 2.01 |
| | | $^7F_0$ | 312 | 8.81 | | | $^5G_6$ | 1185 | $1.93 \times 10^{-3}$ |
| | | $^5D_2$ | 1106 | $1.47 \times 10^{-1}$ | | | $^5G_5$ | 1391 | $4.81 \times 10^{-5}$ |
| | | $^5G_2$ | 1257 | $2.92 \times 10^{-3}$ | | | $^5G_4$ | 1478 | $1.18 \times 10^{-1}$ |
| | | $^5D_1$ | 1526 | $6.2 \times 10^{-1}$ | $^5H_4$ | 34845 | $^7F_5$ | 304 | $5.59 \times 10^{-1}$ |
| $^5F_2$ | 37444 | $^7F_3$ | 301 | 1.37 | | | $^7F_4$ | 316 | 1.5 |
| | | $^7F_2$ | 308 | $1.01 \times 10^{1}$ | | | $^7F_3$ | 327 | $5.5 \times 10^{-1}$ |
| | | $^7F_1$ | 313 | 4.33 | | | $^5D_4$ | 716 | $2.73 \times 10^{-2}$ |
| | | $^5D_3$ | 930 | $6.74 \times 10^{-1}$ | | | $^5D_3$ | 1227 | $8.25 \times 10^{-3}$ |
| | | $^5D_2$ | 1145 | $7.22 \times 10^{-1}$ | | | $^5G_5$ | 1517 | $5.61 \times 10^{-2}$ |
| | | $^5G_3$ | 1227 | $1.41 \times 10^{-2}$ | | | $^5G_4$ | 1620 | 1.57 |
| | | $^5G_2$ | 1307 | $3.92 \times 10^{-2}$ | $^5H_5$ | 34182 | $^7F_5$ | 311 | 2.88 |
| | | $^5D_1$ | 1602 | $1.57 \times 10^{-5}$ | | | $^7F_4$ | 323 | $8.62 \times 10^{-1}$ |
| $^5I_7$ | 36963 | $^5G_6$ | 1004 | $2.6 \times 10^{-3}$ | | | $^5D_4$ | 752 | $1.51 \times 10^{-5}$ |
| | | $^5L_8$ | 1311 | $6.1 \times 10^{-3}$ | | | $^5G_6$ | 1393 | $1.64 \times 10^{-2}$ |
| | | $^5L_7$ | 1373 | $5.3 \times 10^{-2}$ | | | $^5G_5$ | 1686 | 1.02 |
| | | $^5L_6$ | 1445 | $6.81 \times 10^{-3}$ | $^5H_6$ | 33279 | $^7F_6$ | 300 | 2.71 |
| $^5F_3$ | 36930 | $^7F_3$ | 306 | 6.65 | | | $^7F_5$ | 320 | $7.06 \times 10^{-1}$ |
| | | $^7F_2$ | 313 | 2.48 | | | $^5G_6$ | 1594 | $3.92 \times 10^{-1}$ |

[a] The emission rate, $A_{md}$, inside a host material with refractive index $n_r$ would be: $A_{md} = A'_{md}\, n_r^3$

TABLE S8: Continued: $Tb^{3+}$ MD spontaneous emission lines between 300 and 1700 nm.

| $SLJ$ | $E_{SLJ}(cm^{-1})$ | $S'L'J'$ | $\lambda$ (nm) | $A'_{md}$ $(s^{-1})$ [a] | $SLJ$ | $E_{SLJ}(cm^{-1})$ | $S'L'J'$ | $\lambda$ (nm) | $A'_{md}$ $(s^{-1})$ [a] |
|---|---:|---|---:|---:|---|---:|---|---:|---:|
| $^5D_0$ | 31877 | $^7F_1$ | 378 | $2.92 \times 10^1$ | $^5D_2$ | 28712 | $^7F_1$ | 430 | 7.11 |
| $^5H_7$ | 31843 | $^7F_6$ | 314 | $2.84 \times 10^{-1}$ | $^5G_4$ | 28673 | $^7F_5$ | 375 | 2.01 |
| $^5D_1$ | 31200 | $^7F_2$ | 381 | $2.02 \times 10^1$ | | | $^7F_4$ | 393 | 9.68 |
| | | $^7F_1$ | 388 | $1.39 \times 10^{-1}$ | | | $^7F_3$ | 409 | 2.61 |
| | | $^7F_0$ | 392 | 8.21 | | | $^5D_4$ | 1283 | $9.27 \times 10^{-2}$ |
| $^5L_6$ | 30042 | $^7F_6$ | 333 | $8.5 \times 10^{-1}$ | $^5G_5$ | 28252 | $^7F_6$ | 354 | 2.4 |
| | | $^7F_5$ | 357 | $1.02 \times 10^{-1}$ | | | $^7F_5$ | 381 | $1.45 \times 10^1$ |
| $^5G_2$ | 29794 | $^7F_3$ | 391 | 1.82 | | | $^7F_4$ | 400 | 2.69 |
| | | $^7F_2$ | 403 | 2.49 | | | $^5D_4$ | 1357 | $3.64 \times 10^{-2}$ |
| | | $^7F_1$ | 411 | $7.32 \times 10^{-1}$ | $^5G_6$ | 27004 | $^7F_6$ | 370 | $2.44 \times 10^1$ |
| $^5L_7$ | 29678 | $^7F_6$ | 337 | $2.44 \times 10^{-2}$ | | | $^7F_5$ | 400 | 2.41 |
| $^5G_3$ | 29295 | $^7F_4$ | 384 | 2.49 | $^5D_3$ | 26693 | $^7F_4$ | 427 | $1.55 \times 10^1$ |
| | | $^7F_3$ | 399 | 5.57 | | | $^7F_3$ | 446 | $2.54 \times 10^{-1}$ |
| | | $^7F_2$ | 411 | 1.7 | | | $^7F_2$ | 460 | 4.55 |
| | | $^5D_4$ | 1189 | $1.44 \times 10^{-2}$ | $^5D_4$ | 20881 | $^7F_5$ | 530 | $1.43 \times 10^1$ |
| $^5D_2$ | 28712 | $^7F_3$ | 409 | $1.79 \times 10^1$ | | | $^7F_4$ | 567 | $5.79 \times 10^{-2}$ |
| | | $^7F_2$ | 421 | $2.88 \times 10^{-1}$ | | | $^7F_3$ | 601 | 1.76 |

[a] The emission rate, $A_{md}$, inside a host material with refractive index $n_r$ would be: $A_{md} = A'_{md}\ n_r^3$

TABLE S9: Calculated $Dy^{3+}$ MD spontaneous emission lines between 300 and 1700 nm.

| $SLJ$ | $E_{SLJ}(cm^{-1})$ | $S'L'J'$ | $\lambda$ (nm) | $A'_{md}$ $(s^{-1})$ [a] | $SLJ$ | $E_{SLJ}(cm^{-1})$ | $S'L'J'$ | $\lambda$ (nm) | $A'_{md}$ $(s^{-1})$ [a] |
|---|---|---|---|---|---|---|---|---|---|
| $({}^4G, {}^4P)_{5/2}$ | 38873 | ${}^6H_{7/2}$ | 334 | 5.71 | ${}^4H_{7/2}$ | 37877 | $({}^4D, {}^4G)_{5/2}$ | 1683 | $1.38 \times 10^{-1}$ |
| | | ${}^6H_{5/2}$ | 348 | 5.58 | ${}^4F_{3/2}$ | 37277 | ${}^6H_{5/2}$ | 368 | $3.88 \times 10^{-2}$ |
| | | ${}^6F_{7/2}$ | 355 | 1.01 | | | ${}^6F_{5/2}$ | 397 | $1.57 \times 10^{-1}$ |
| | | ${}^6F_{5/2}$ | 374 | $6.39 \times 10^{-1}$ | | | ${}^6F_{3/2}$ | 410 | $5.93 \times 10^{-1}$ |
| | | ${}^6F_{3/2}$ | 385 | $8.58 \times 10^{-1}$ | | | ${}^6F_{1/2}$ | 419 | $1.59 \times 10^{-1}$ |
| | | ${}^4F_{7/2}$ | 754 | $1.91 \times 10^{-1}$ | | | ${}^6P_{5/2}$ | 944 | $1.76 \times 10^{-1}$ |
| | | ${}^6P_{5/2}$ | 820 | 1.23 | | | $({}^4P, {}^6P)_{3/2}$ | 964 | $1.61 \times 10^{-1}$ |
| | | $({}^4P, {}^6P)_{3/2}$ | 835 | $1.47 \times 10^{-1}$ | | | $({}^4F, {}^4D)_{5/2}$ | 1282 | 1.17 |
| | | ${}^6P_{7/2}$ | 896 | 1.71 | | | ${}^6P_{3/2}$ | 1402 | 2.6 |
| | | $({}^4F, {}^4D)_{5/2}$ | 1064 | 2.06 | ${}^4P_{1/2}$ | 37189 | ${}^6F_{3/2}$ | 412 | 9.28 |
| | | ${}^6P_{3/2}$ | 1146 | $3.79 \times 10^{-2}$ | | | ${}^6F_{1/2}$ | 421 | 6.67 |
| | | $({}^4G, {}^4F)_{7/2}$ | 1366 | $5.76 \times 10^{-1}$ | | | $({}^4P, {}^6P)_{3/2}$ | 972 | $2.24 \times 10^{-1}$ |
| | | $({}^4D, {}^4G)_{5/2}$ | 1442 | $5.57 \times 10^{-1}$ | | | ${}^6P_{3/2}$ | 1419 | 3.53 |
| $({}^4P, {}^4D)_{3/2}$ | 38691 | ${}^6H_{5/2}$ | 350 | $2.88 \times 10^{-3}$ | ${}^4L_{13/2}$ | 36666 | ${}^6H_{11/2}$ | 322 | $5.86 \times 10^{-3}$ |
| | | ${}^6F_{5/2}$ | 376 | 6.62 | | | ${}^6F_{11/2}$ | 342 | $6.97 \times 10^{-4}$ |
| | | ${}^6F_{3/2}$ | 388 | $1.55 \times 10^{-1}$ | | | ${}^4I_{15/2}$ | 716 | $2.04 \times 10^{-3}$ |
| | | ${}^6F_{1/2}$ | 396 | $7.67 \times 10^{-3}$ | | | ${}^4G_{11/2}$ | 765 | $2.25 \times 10^{-2}$ |
| | | ${}^6P_{5/2}$ | 833 | $2.22 \times 10^{-1}$ | | | ${}^4I_{13/2}$ | 942 | $5.89 \times 10^{-1}$ |
| | | $({}^4P, {}^6P)_{3/2}$ | 848 | $1.92 \times 10^{-1}$ | | | ${}^4I_{11/2}$ | 1235 | $8.74 \times 10^{-1}$ |
| | | $({}^4F, {}^4D)_{5/2}$ | 1085 | 1.07 | | | ${}^4M_{15/2}$ | 1402 | $2.86 \times 10^{-1}$ |
| | | ${}^6P_{3/2}$ | 1170 | 5.19 | $({}^4G, {}^4P)_{5/2}$ | 36489 | ${}^6H_{7/2}$ | 363 | 3.01 |
| | | $({}^4D, {}^4P)_{1/2}$ | 1445 | $5.93 \times 10^{-2}$ | | | ${}^6H_{5/2}$ | 379 | 2.38 |
| | | $({}^4D, {}^4G)_{5/2}$ | 1480 | 1.16 | | | ${}^6F_{7/2}$ | 388 | $6.12 \times 10^{-1}$ |
| $({}^2K, {}^2L)_{15/2}$ | 38434 | ${}^4I_{15/2}$ | 635 | 9.75 | | | ${}^6F_{5/2}$ | 410 | $7.99 \times 10^{-1}$ |
| | | ${}^4K_{17/2}$ | 802 | $4.76 \times 10^{-1}$ | | | ${}^6F_{3/2}$ | 424 | 1.46 |
| | | ${}^4I_{13/2}$ | 808 | 2.57 | | | ${}^4F_{7/2}$ | 919 | $4.34 \times 10^{-1}$ |
| | | ${}^4M_{15/2}$ | 1124 | 8.33 | | | ${}^6P_{5/2}$ | 1020 | 3.04 |
| | | ${}^4M_{17/2}$ | 1150 | 3.67 | | | $({}^4P, {}^6P)_{3/2}$ | 1043 | $1.97 \times 10^{-2}$ |
| | | ${}^4K_{15/2}$ | 1318 | $1.97 \times 10^{-1}$ | | | ${}^6P_{7/2}$ | 1139 | 3.36 |
| ${}^4H_{7/2}$ | 37877 | ${}^6H_{9/2}$ | 329 | 2.86 | | | $({}^4F, {}^4D)_{5/2}$ | 1426 | 1.31 |
| | | ${}^6F_{9/2}$ | 345 | $8.79 \times 10^{-1}$ | | | ${}^6P_{3/2}$ | 1576 | $1.49 \times 10^{-1}$ |
| | | ${}^6H_{7/2}$ | 345 | 1.04 | $({}^4H, {}^4G)_{9/2}$ | 36463 | ${}^6H_{11/2}$ | 324 | 1.25 |
| | | ${}^6H_{5/2}$ | 360 | $1.28 \times 10^{1}$ | | | ${}^6F_{11/2}$ | 344 | 2.14 |
| | | ${}^6F_{7/2}$ | 368 | 2.14 | | | ${}^6H_{9/2}$ | 345 | 1.05 |
| | | ${}^6F_{5/2}$ | 388 | $9.02 \times 10^{-1}$ | | | ${}^6F_{9/2}$ | 362 | 6.15 |
| | | ${}^4F_{9/2}$ | 594 | $7.76 \times 10^{-1}$ | | | ${}^6H_{7/2}$ | 363 | 2.76 |
| | | ${}^4F_{7/2}$ | 815 | $3.35 \times 10^{-1}$ | | | ${}^6F_{7/2}$ | 388 | 1.5 |
| | | ${}^6P_{5/2}$ | 893 | $3.74 \times 10^{-3}$ | | | ${}^4F_{9/2}$ | 649 | $4.68 \times 10^{-1}$ |
| | | ${}^6P_{7/2}$ | 983 | $8.81 \times 10^{-2}$ | | | ${}^4G_{11/2}$ | 777 | 1.21 |
| | | $({}^4F, {}^4D)_{5/2}$ | 1191 | $2.14 \times 10^{-1}$ | | | ${}^4F_{7/2}$ | 921 | $1.99 \times 10^{-1}$ |
| | | ${}^4G_{9/2}$ | 1277 | $3.65 \times 10^{-1}$ | | | ${}^6P_{7/2}$ | 1142 | $5.03 \times 10^{-2}$ |
| | | ${}^4I_{9/2}$ | 1403 | $6.28 \times 10^{-3}$ | | | ${}^4I_{11/2}$ | 1267 | $1.43 \times 10^{-1}$ |
| | | $({}^4G, {}^4F)_{7/2}$ | 1581 | $5.8 \times 10^{-1}$ | | | ${}^4G_{9/2}$ | 1558 | $5.47 \times 10^{-1}$ |

[a] The emission rate, $A_{md}$, inside a host material with refractive index $n_r$ would be: $A_{md} = A'_{md}\ n_r^3$

TABLE S9: Continued: $Dy^{3+}$ MD spontaneous emission lines between 300 and 1700 nm.

| $SLJ$ | $E_{SLJ}(cm^{-1})$ | $S'L'J'$ | $\lambda$ (nm) | $A'_{md}$ $(s^{-1})$ [a] | $SLJ$ | $E_{SLJ}(cm^{-1})$ | $S'L'J'$ | $\lambda$ (nm) | $A'_{md}$ $(s^{-1})$ [a] |
|---|---|---|---|---|---|---|---|---|---|
| $^4G_{7/2}$ | 36281 | $^6H_{9/2}$ | 347 | 8.28 | $^4G_{9/2}$ | 34755 | $^4G_{11/2}$ | 896 | 6.64 |
| | | $^6F_{9/2}$ | 365 | 2.76 | | | $^4F_{7/2}$ | 1094 | $5.3 \times 10^{-2}$ |
| | | $^6H_{7/2}$ | 366 | 6.84 | | | $^6P_{7/2}$ | 1419 | $1.74 \times 10^{-5}$ |
| | | $^6H_{5/2}$ | 382 | $3.46 \times 10^{-1}$ | | | $^4I_{11/2}$ | 1617 | $2.21 \times 10^{-1}$ |
| | | $^6F_{7/2}$ | 391 | 3.26 | $(^4F, ^4G)_{5/2}$ | 34079 | $^6H_{7/2}$ | 398 | 1.67 |
| | | $^6F_{5/2}$ | 414 | 1.59 | | | $^6H_{5/2}$ | 417 | $4.08 \times 10^{-1}$ |
| | | $^4F_{9/2}$ | 656 | 3.31 | | | $^6F_{7/2}$ | 428 | 6.72 |
| | | $^4F_{7/2}$ | 937 | $1.02 \times 10^{-1}$ | | | $^6F_{5/2}$ | 455 | $8.54 \times 10^{-1}$ |
| | | $^6P_{5/2}$ | 1042 | $2.63 \times 10^{-2}$ | | | $^6F_{3/2}$ | 472 | 4.48 |
| | | $^6P_{7/2}$ | 1166 | $1.34 \times 10^{-1}$ | | | $^4F_{7/2}$ | 1181 | 1.6 |
| | | $(^4F, ^4D)_{5/2}$ | 1470 | $4.36 \times 10^{-4}$ | | | $^6P_{5/2}$ | 1352 | $2.78 \times 10^{-2}$ |
| | | $^4G_{9/2}$ | 1603 | $6.84 \times 10^{-3}$ | | | $(^4P, ^6P)_{3/2}$ | 1393 | $6.33 \times 10^{-1}$ |
| $^4L_{15/2}$ | 36261 | $^6H_{13/2}$ | 304 | $1.08 \times 10^{-1}$ | | | $^6P_{7/2}$ | 1569 | 1.02 |
| | | $^4I_{15/2}$ | 737 | $1.91 \times 10^{-2}$ | $(^4H, ^4G)_{11/2}$ | 34061 | $^6H_{13/2}$ | 325 | 1.26 |
| | | $^4K_{17/2}$ | 971 | $1.9 \times 10^{-3}$ | | | $^6H_{11/2}$ | 352 | 2.52 |
| | | $^4I_{13/2}$ | 979 | $3.37 \times 10^{-2}$ | | | $^6F_{11/2}$ | 375 | 5.74 |
| | | $^4M_{15/2}$ | 1487 | $4.87 \times 10^{-2}$ | | | $^6H_{9/2}$ | 376 | $9.18 \times 10^{-1}$ |
| | | $^4M_{17/2}$ | 1534 | $5.78 \times 10^{-1}$ | | | $^6F_{9/2}$ | 397 | $4.84 \times 10^{-1}$ |
| $^4K_{11/2}$ | 35631 | $^6H_{13/2}$ | 309 | $5.74 \times 10^{-1}$ | | | $^4F_{9/2}$ | 768 | $2.46 \times 10^{-1}$ |
| | | $^6H_{11/2}$ | 333 | $8.14 \times 10^{-1}$ | | | $^4G_{11/2}$ | 955 | 1.29 |
| | | $^6F_{11/2}$ | 355 | 1.82 | | | $^4I_{13/2}$ | 1248 | 1.09 |
| | | $^6H_{9/2}$ | 355 | $7.52 \times 10^{-1}$ | $^4H_{13/2}$ | 33924 | $^6H_{13/2}$ | 327 | 4.71 |
| | | $^6F_{9/2}$ | 373 | $1.28 \times 10^{-1}$ | | | $^6H_{11/2}$ | 353 | 2.16 |
| | | $^4F_{9/2}$ | 686 | $1.34 \times 10^{-1}$ | | | $^6F_{11/2}$ | 377 | $1.52 \times 10^{-1}$ |
| | | $^4G_{11/2}$ | 831 | $2.99 \times 10^{-4}$ | | | $^4I_{15/2}$ | 890 | 1.73 |
| | | $^4I_{13/2}$ | 1044 | $4.15 \times 10^{-2}$ | | | $^4G_{11/2}$ | 968 | 1.67 |
| | | $^4I_{11/2}$ | 1416 | 1.42 | | | $^4I_{13/2}$ | 1270 | $1.82 \times 10^{-1}$ |
| $^4G_{11/2}$ | 35096 | $^6H_{13/2}$ | 315 | $8.3 \times 10^{-3}$ | $^4D_{7/2}$ | 33836 | $^6H_{9/2}$ | 379 | $9.35 \times 10^{-2}$ |
| | | $^6H_{11/2}$ | 339 | $5.13 \times 10^{-1}$ | | | $^6F_{9/2}$ | 400 | 9.44 |
| | | $^6F_{11/2}$ | 361 | $1.6 \times 10^{1}$ | | | $^6H_{7/2}$ | 401 | $2.07 \times 10^{-1}$ |
| | | $^6H_{9/2}$ | 362 | $4.48 \times 10^{-1}$ | | | $^6H_{5/2}$ | 422 | $2.28 \times 10^{-1}$ |
| | | $^6F_{9/2}$ | 381 | 1.46 | | | $^6F_{7/2}$ | 432 | 1.87 |
| | | $^4F_{9/2}$ | 712 | 1.21 | | | $^6F_{5/2}$ | 460 | 1.82 |
| | | $^4G_{11/2}$ | 869 | $4.62 \times 10^{-1}$ | | | $^4F_{9/2}$ | 782 | 3.89 |
| | | $^4I_{13/2}$ | 1105 | $1.91 \times 10^{-1}$ | | | $^4F_{7/2}$ | 1216 | $1.6 \times 10^{-1}$ |
| | | $^4I_{11/2}$ | 1532 | $8.24 \times 10^{-1}$ | | | $^6P_{5/2}$ | 1398 | $6.41 \times 10^{-1}$ |
| $^4G_{9/2}$ | 34755 | $^6H_{11/2}$ | 343 | 4.41 | | | $^6P_{7/2}$ | 1632 | 1.52 |
| | | $^6F_{11/2}$ | 366 | 1.16 | $^4F_{3/2}$ | 33629 | $^6H_{5/2}$ | 425 | $6.78 \times 10^{-1}$ |
| | | $^6H_{9/2}$ | 366 | 3.53 | | | $^6F_{5/2}$ | 465 | $7.94 \times 10^{-2}$ |
| | | $^6F_{9/2}$ | 386 | 8.45 | | | $^6F_{3/2}$ | 482 | 3.98 |
| | | $^6H_{7/2}$ | 387 | $3.85 \times 10^{-2}$ | | | $^6F_{1/2}$ | 495 | 7.27 |
| | | $^6F_{7/2}$ | 416 | 3.07 | | | $^6P_{5/2}$ | 1440 | $1. \times 10^{-1}$ |
| | | $^4F_{9/2}$ | 729 | $1.03 \times 10^{-5}$ | | | $(^4P, ^6P)_{3/2}$ | 1486 | $1.86 \times 10^{-1}$ |

[a] The emission rate, $A_{md}$, inside a host material with refractive index $n_r$ would be: $A_{md} = A'_{md}\ n_r^3$

TABLE S9: Continued: $Dy^{3+}$ MD spontaneous emission lines between 300 and 1700 nm.

| $SLJ$ | $E_{SLJ}(cm^{-1})$ | $S'L'J'$ | $\lambda$ (nm) | $A'_{md}$ $(s^{-1})$ [a] | $SLJ$ | $E_{SLJ}(cm^{-1})$ | $S'L'J'$ | $\lambda$ (nm) | $A'_{md}$ $(s^{-1})$ [a] |
|---|---|---|---|---|---|---|---|---|---|
| $^4L_{17/2}$ | 33454 | $^4I_{15/2}$ | 929 | $2.38 \times 10^{-3}$ | $^4G_{9/2}$ | 30044 | $^6H_{9/2}$ | 443 | $1.18 \times 10^{-2}$ |
| | | $^4K_{17/2}$ | 1335 | $1.44 \times 10^{-1}$ | | | $^6F_{9/2}$ | 472 | $1.28 \times 10^{-1}$ |
| | | $^4M_{19/2}$ | 1510 | $9. \times 10^{-1}$ | | | $^6H_{7/2}$ | 473 | 3.16 |
| $(^4K, ^4L)_{13/2}$ | 33321 | $^6H_{15/2}$ | 300 | 1.67 | | | $^6F_{7/2}$ | 517 | $5.69 \times 10^{-1}$ |
| | | $^6H_{13/2}$ | 333 | 2.15 | | | $^4F_{9/2}$ | 1111 | 3.19 |
| | | $^6H_{11/2}$ | 361 | 1.1 | | | $^4G_{11/2}$ | 1550 | 6.21 |
| | | $^6F_{11/2}$ | 386 | $2.59 \times 10^{-2}$ | $^4M_{17/2}$ | 29740 | $^6H_{15/2}$ | 336 | $9.98 \times 10^{-2}$ |
| | | $^4I_{15/2}$ | 941 | $4.01 \times 10^{-1}$ | | | $^4I_{15/2}$ | 1419 | $1.73 \times 10^{-2}$ |
| | | $^4G_{11/2}$ | 1028 | $2.36 \times 10^{-2}$ | $^4M_{15/2}$ | 29534 | $^6H_{15/2}$ | 339 | 3.57 |
| | | $^4I_{13/2}$ | 1375 | 3.4 | | | $^6H_{13/2}$ | 381 | $9.02 \times 10^{-1}$ |
| $(^4D, ^4G)_{5/2}$ | 31937 | $^6H_{7/2}$ | 435 | 4.57 | | | $^4I_{15/2}$ | 1461 | 3.65 |
| | | $^6H_{5/2}$ | 458 | 5.09 | $(^4F, ^4D)_{5/2}$ | 29478 | $^6H_{7/2}$ | 486 | 1.24 |
| | | $^6F_{7/2}$ | 471 | 8.11 | | | $^6H_{5/2}$ | 517 | 3.94 |
| | | $^6F_{5/2}$ | 504 | $1.25 \times 10^{-2}$ | | | $^6F_{7/2}$ | 533 | 5.13 |
| | | $^6F_{3/2}$ | 525 | $6.62 \times 10^{-1}$ | | | $^6F_{5/2}$ | 576 | 2.31 |
| | | $^4F_{7/2}$ | 1581 | $4.07 \times 10^{-1}$ | | | $^6F_{3/2}$ | 603 | 1.4 |
| $(^4D, ^4P)_{1/2}$ | 31770 | $^6F_{3/2}$ | 530 | $1.04 \times 10^{1}$ | $^4I_{11/2}$ | 28569 | $^6H_{13/2}$ | 396 | 1.44 |
| | | $^6F_{1/2}$ | 545 | 1.2 | | | $^6H_{11/2}$ | 436 | 5.71 |
| $(^4G, ^4F)_{7/2}$ | 31551 | $^6H_{9/2}$ | 415 | 8.77 | | | $^6F_{11/2}$ | 473 | $4.79 \times 10^{-2}$ |
| | | $^6F_{9/2}$ | 441 | 3.65 | | | $^6H_{9/2}$ | 474 | 3.34 |
| | | $^6H_{7/2}$ | 442 | $7.73 \times 10^{-1}$ | | | $^6F_{9/2}$ | 507 | $2.76 \times 10^{-2}$ |
| | | $^6H_{5/2}$ | 467 | 2.51 | | | $^4F_{9/2}$ | 1329 | $8.06 \times 10^{-4}$ |
| | | $^6F_{7/2}$ | 480 | $7.62 \times 10^{-2}$ | $^6P_{7/2}$ | 27707 | $^6H_{9/2}$ | 494 | $5.74 \times 10^{-1}$ |
| | | $^6F_{5/2}$ | 514 | 1.21 | | | $^6F_{9/2}$ | 530 | 1.36 |
| | | $^4F_{9/2}$ | 952 | $5.08 \times 10^{-3}$ | | | $^6H_{7/2}$ | 532 | $3.21 \times 10^{-1}$ |
| | | $^4F_{7/2}$ | 1683 | $8.66 \times 10^{-1}$ | | | $^6H_{5/2}$ | 569 | $2.16 \times 10^{-1}$ |
| $^4K_{15/2}$ | 30846 | $^6H_{15/2}$ | 324 | 1.43 | | | $^6F_{7/2}$ | 588 | $3.75 \times 10^{-1}$ |
| | | $^6H_{13/2}$ | 363 | $6.4 \times 10^{-1}$ | | | $^6F_{5/2}$ | 641 | 1.4 |
| | | $^4I_{15/2}$ | 1226 | $3.52 \times 10^{-2}$ | | | $^4F_{9/2}$ | 1501 | 2.44 |
| $^4I_{9/2}$ | 30748 | $^6H_{11/2}$ | 398 | 3.02 | $(^4P, ^6P)_{3/2}$ | 26899 | $^6H_{5/2}$ | 596 | $1.82 \times 10^{-3}$ |
| | | $^6F_{11/2}$ | 429 | $3.37 \times 10^{-2}$ | | | $^6F_{5/2}$ | 676 | 5.94 |
| | | $^6H_{9/2}$ | 429 | 2.54 | | | $^6F_{3/2}$ | 714 | $4.07 \times 10^{-1}$ |
| | | $^6F_{9/2}$ | 457 | $4.67 \times 10^{-2}$ | | | $^6F_{1/2}$ | 742 | $8.87 \times 10^{-1}$ |
| | | $^6H_{7/2}$ | 458 | 1.2 | $^6P_{5/2}$ | 26684 | $^6H_{7/2}$ | 563 | $1.08 \times 10^{-1}$ |
| | | $^6F_{7/2}$ | 499 | $1.5 \times 10^{-2}$ | | | $^6H_{5/2}$ | 604 | $2.02 \times 10^{-1}$ |
| | | $^4F_{9/2}$ | 1031 | $4.28 \times 10^{-2}$ | | | $^6F_{7/2}$ | 626 | $3.78 \times 10^{-2}$ |
| | | $^4G_{11/2}$ | 1398 | $4.9 \times 10^{-1}$ | | | $^6F_{5/2}$ | 686 | $4.27 \times 10^{-3}$ |
| $^6P_{3/2}$ | 30144 | $^6H_{5/2}$ | 500 | $5.87 \times 10^{-4}$ | | | $^6F_{3/2}$ | 726 | $9.61 \times 10^{-2}$ |
| | | $^6F_{5/2}$ | 555 | 8.89 | $^4I_{13/2}$ | 26050 | $^6H_{15/2}$ | 384 | 2.65 |
| | | $^6F_{3/2}$ | 580 | $1.5 \times 10^{-1}$ | | | $^6H_{13/2}$ | 440 | 9.99 |
| | | $^6F_{1/2}$ | 598 | 1.79 | | | $^6H_{11/2}$ | 490 | 3.3 |
| $^4G_{9/2}$ | 30044 | $^6H_{11/2}$ | 410 | $1.14 \times 10^{1}$ | | | $^6F_{11/2}$ | 537 | $8.92 \times 10^{-2}$ |
| | | $^6F_{11/2}$ | 442 | $8.79 \times 10^{-1}$ | $^4K_{17/2}$ | 25967 | $^6H_{15/2}$ | 385 | $3.83 \times 10^{-1}$ |

[a] The emission rate, $A_{md}$, inside a host material with refractive index $n_r$ would be: $A_{md} = A'_{md}\ n_r^3$

TABLE S9: Continued: $Dy^{3+}$ MD spontaneous emission lines between 300 and 1700 nm.

| $SLJ$ | $E_{SLJ}(cm^{-1})$ | $S'L'J'$ | $\lambda$ (nm) | $A'_{md}$ $(s^{-1})$ [a] | $SLJ$ | $E_{SLJ}(cm^{-1})$ | $S'L'J'$ | $\lambda$ (nm) | $A'_{md}$ $(s^{-1})$ [a] |
|---|---|---|---|---|---|---|---|---|---|
| $^4F_{7/2}$ | 25610 | $^6H_{9/2}$ | 551 | 2.74 | $^4G_{11/2}$ | 23594 | $^6F_{9/2}$ | 678 | 1.25 |
| | | $^6F_{9/2}$ | 597 | $2.1 \times 10^{-1}$ | $^4I_{15/2}$ | 22691 | $^6H_{15/2}$ | 441 | $1.88 \times 10^{1}$ |
| | | $^6H_{7/2}$ | 599 | 1.76 | | | $^6H_{13/2}$ | 516 | 2.63 |
| | | $^6H_{5/2}$ | 646 | $8.48 \times 10^{-1}$ | $^4F_{9/2}$ | 21045 | $^6H_{11/2}$ | 649 | 3.02 |
| | | $^6F_{7/2}$ | 671 | 1.99 | | | $^6F_{11/2}$ | 734 | $1.17 \times 10^{1}$ |
| | | $^6F_{5/2}$ | 741 | 1.87 | | | $^6H_{9/2}$ | 736 | $6.95 \times 10^{-1}$ |
| $^4G_{11/2}$ | 23594 | $^6H_{13/2}$ | 493 | $1.95 \times 10^{1}$ | | | $^6F_{9/2}$ | 820 | 1.34 |
| | | $^6H_{11/2}$ | 557 | $1.58 \times 10^{-1}$ | | | $^6H_{7/2}$ | 825 | $7.2 \times 10^{-1}$ |
| | | $^6F_{11/2}$ | 619 | 1.14 | | | $^6F_{7/2}$ | 968 | 1.39 |
| | | $^6H_{9/2}$ | 620 | $8.5 \times 10^{-1}$ | | | | | |

[a] The emission rate, $A_{md}$, inside a host material with refractive index $n_r$ would be: $A_{md} = A'_{md}\ n_r^3$

TABLE S10: Calculated $Ho^{3+}$ MD spontaneous emission lines between 300 and 1700 nm.

| $SLJ$ | $E_{SLJ}(cm^{-1})$ | $S'L'J'$ | $\lambda$ (nm) | $A'_{md}$ $(s^{-1})$ [a] | $SLJ$ | $E_{SLJ}(cm^{-1})$ | $S'L'J'$ | $\lambda$ (nm) | $A'_{md}$ $(s^{-1})$ [a] |
|---|---|---|---|---|---|---|---|---|---|
| $^5D_1$ | 39165 | $^5S_2$ | 469 | 2.3 | $^3F_4$ | 38607 | $^5F_3$ | 538 | 6.47 |
| | | $^5F_2$ | 534 | $2.25 \times 10^{-1}$ | | | $(^5G, ^3G)_5$ | 653 | $1.66 \times 10^{1}$ |
| | | $^5F_1$ | 573 | $8.11 \times 10^{-1}$ | | | $^5G_4$ | 745 | 2.43 |
| | | $(^5F, ^5G)_2$ | 886 | 3.73 | | | $(^5G, ^3H)_5$ | 856 | 1.05 |
| | | $^5G_2$ | 1092 | 2.87 | | | $^5G_3$ | 953 | $3.16 \times 10^{-1}$ |
| | | $^3P_1$ | 1607 | 1.67 | | | $(^3F, ^3G)_4$ | 1083 | $9.26 \times 10^{-1}$ |
| $^3M_9$ | 39159 | $^3K_8$ | 542 | $5.34 \times 10^{-3}$ | $^3L_7$ | 37966 | $^5I_7$ | 304 | $2.33 \times 10^{-1}$ |
| | | $^3L_9$ | 972 | 2.48 | | | $^5I_6$ | 339 | $3.1 \times 10^{-1}$ |
| $^5D_3$ | 38728 | $^5I_4$ | 392 | $4.54 \times 10^{-1}$ | | | $^3K_8$ | 580 | 1.14 |
| | | $^5S_2$ | 478 | $3.58 \times 10^{-2}$ | | | $^5G_6$ | 600 | $4.21 \times 10^{-3}$ |
| | | $^5F_4$ | 483 | $5.82 \times 10^{-2}$ | | | $^3K_7$ | 811 | 5.6 |
| | | $^5F_3$ | 534 | $1.35 \times 10^{-1}$ | | | $^3H_6$ | 939 | $7.31 \times 10^{-2}$ |
| | | $^5F_2$ | 547 | $4.11 \times 10^{-1}$ | | | $^3K_6$ | 1199 | 1.35 |
| | | $^5G_4$ | 738 | $6.5 \times 10^{-2}$ | $(^1L, ^3L)_8$ | 37687 | $^5I_7$ | 307 | $5.95 \times 10^{-2}$ |
| | | $(^5F, ^5G)_2$ | 922 | $7.24 \times 10^{-2}$ | | | $^3K_8$ | 589 | 2.93 |
| | | $^5G_3$ | 942 | $1.18 \times 10^{-1}$ | | | $^3K_7$ | 830 | 2.58 |
| | | $(^3F, ^3G)_4$ | 1069 | $3.98 \times 10^{-2}$ | | | $^3L_9$ | 1135 | 2.33 |
| | | $^5G_2$ | 1147 | $9.74 \times 10^{-1}$ | $^3P_2$ | 37409 | $^5S_2$ | 511 | 6.61 |
| $^3I_5$ | 38713 | $^5I_6$ | 331 | 2.88 | | | $^5F_3$ | 575 | 2.89 |
| | | $^5I_5$ | 363 | 4.14 | | | $^5F_2$ | 589 | 4.5 |
| | | $^5I_4$ | 392 | 1.77 | | | $^5F_1$ | 637 | $9.96 \times 10^{-1}$ |
| | | $^5F_5$ | 420 | $5.33 \times 10^{-1}$ | | | $(^5F, ^5G)_2$ | 1049 | 3.74 |
| | | $^5F_4$ | 483 | $1.11 \times 10^{-1}$ | | | $^5G_3$ | 1076 | $4.85 \times 10^{-1}$ |
| | | $^5G_6$ | 574 | $1.91 \times 10^{-1}$ | | | $^5G_2$ | 1351 | $2.74 \times 10^{-1}$ |
| | | $(^5G, ^3G)_5$ | 648 | $1.38 \times 10^{-1}$ | $^3I_7$ | 37258 | $^5I_7$ | 311 | 2.61 |
| | | $^5G_4$ | 739 | $2.59 \times 10^{-1}$ | | | $^5I_6$ | 348 | 1. |
| | | $(^5G, ^3H)_5$ | 848 | $3.95 \times 10^{-4}$ | | | $^3K_8$ | 604 | 4.99 |
| | | $^3H_6$ | 878 | 2.1 | | | $^5G_6$ | 627 | $2.47 \times 10^{-1}$ |
| | | $(^3F, ^3G)_4$ | 1071 | $4.25 \times 10^{-1}$ | | | $^3K_7$ | 860 | 1.19 |
| | | $^3K_6$ | 1100 | 1.07 | | | $^3H_6$ | 1006 | $4.5 \times 10^{-1}$ |
| $^3I_6$ | 38648 | $^5I_6$ | 332 | 3.18 | | | $^3K_6$ | 1310 | $3.6 \times 10^{-2}$ |
| | | $^5I_5$ | 363 | 3.1 | $(^3H, ^3G)_5$ | 36196 | $^5I_6$ | 361 | $1.22 \times 10^{1}$ |
| | | $^5F_5$ | 421 | $6.49 \times 10^{-2}$ | | | $^5I_5$ | 399 | $8.83 \times 10^{-1}$ |
| | | $^5G_6$ | 577 | $2.9 \times 10^{-1}$ | | | $^5I_4$ | 435 | 1.05 |
| | | $(^5G, ^3G)_5$ | 651 | $3.27 \times 10^{-2}$ | | | $^5F_5$ | 470 | $3.69 \times 10^{-1}$ |
| | | $^3K_7$ | 769 | $1.46 \times 10^{-3}$ | | | $^5F_4$ | 550 | $9.82 \times 10^{-1}$ |
| | | $(^5G, ^3H)_5$ | 853 | $5.63 \times 10^{-2}$ | | | $^5G_6$ | 672 | $5.65 \times 10^{-2}$ |
| | | $^3H_6$ | 883 | $4.21 \times 10^{-1}$ | | | $(^5G, ^3G)_5$ | 775 | 2.19 |
| | | $^3K_6$ | 1108 | $9.26 \times 10^{-1}$ | | | $^5G_4$ | 908 | $3.5 \times 10^{-1}$ |
| $^3F_4$ | 38607 | $^5I_5$ | 364 | $8.02 \times 10^{-1}$ | | | $(^5G, ^3H)_5$ | 1078 | 6.22 |
| | | $^5I_4$ | 394 | $5.19 \times 10^{-1}$ | | | $^3H_6$ | 1126 | $1.21 \times 10^{1}$ |
| | | $^5F_5$ | 422 | 6.73 | | | $(^3F, ^3G)_4$ | 1466 | $2.56 \times 10^{-3}$ |
| | | $^5F_4$ | 486 | 5.71 | | | $^3K_6$ | 1522 | $2.22 \times 10^{-2}$ |

[a] The emission rate, $A_{md}$, inside a host material with refractive index $n_r$ would be: $A_{md} = A'_{md}\ n_r^3$

TABLE S10: Continued: $Ho^{3+}$ MD spontaneous emission lines between 300 and 1700 nm.

| $SLJ$ | $E_{SLJ}(cm^{-1})$ | $S'L'J'$ | $\lambda$ (nm) | $A'_{md}$ $(s^{-1})$ [a] | $SLJ$ | $E_{SLJ}(cm^{-1})$ | $S'L'J'$ | $\lambda$ (nm) | $A'_{md}$ $(s^{-1})$ [a] |
|---|---|---|---|---|---|---|---|---|---|
| $^3P_0$ | 35725 | $^5F_1$ | 713 | 1.78 | $^3D_3$ | 32901 | $^5F_2$ | 803 | $4.94 \times 10^{-2}$ |
| $(^3F, ^5G)_2$ | 35562 | $^5S_2$ | 564 | $2.56 \times 10^{-1}$ | | | $^5G_4$ | 1295 | 1.35 |
| | | $^5F_3$ | 643 | $5.05 \times 10^{-2}$ | $^5G_2$ | 30009 | $^5S_2$ | 821 | $5.21 \times 10^{-1}$ |
| | | $^5F_2$ | 661 | 4.26 | | | $^5F_3$ | 1000 | 4.26 |
| | | $^5F_1$ | 721 | 2.63 | | | $^5F_2$ | 1045 | 1.75 |
| | | $(^5F, ^5G)_2$ | 1302 | $2.13 \times 10^{-2}$ | | | $^5F_1$ | 1204 | $4.46 \times 10^{-1}$ |
| | | $^5G_3$ | 1342 | 3.86 | $^3K_6$ | 29625 | $^5I_7$ | 407 | $1.13 \times 10^{-1}$ |
| $(^1G, ^3H)_4$ | 35453 | $^5I_5$ | 411 | 9.86 | | | $^5I_6$ | 473 | 2.78 |
| | | $^5I_4$ | 449 | 5.05 | | | $^5I_5$ | 541 | 3.87 |
| | | $^5F_5$ | 487 | $5.22 \times 10^{-2}$ | | | $^5F_5$ | 680 | $1.11 \times 10^{-1}$ |
| | | $^5F_4$ | 574 | 1.13 | | | $^5G_6$ | 1202 | $2.85 \times 10^{-3}$ |
| | | $^5F_3$ | 647 | $3.79 \times 10^{-1}$ | | | $(^5G, ^3G)_5$ | 1578 | $2.84 \times 10^{-2}$ |
| | | $(^5G, ^3G)_5$ | 822 | 2.48 | $(^3F, ^3G)_4$ | 29374 | $^5I_5$ | 548 | 3.74 |
| | | $^5G_4$ | 974 | $1.28 \times 10^{-1}$ | | | $^5I_4$ | 618 | 7.72 |
| | | $(^5G, ^3H)_5$ | 1172 | $4.62 \times 10^{-1}$ | | | $^5F_5$ | 692 | 4.25 |
| | | $^5G_3$ | 1362 | 1.1 | | | $^5F_4$ | 881 | $1.34 \times 10^{-1}$ |
| | | $(^3F, ^3G)_4$ | 1645 | 2.72 | | | $^5F_3$ | 1067 | $1.59 \times 10^{-2}$ |
| $(^3F, ^3G)_3$ | 34498 | $^5I_4$ | 470 | 1.01 | | | $(^5G, ^3G)_5$ | 1642 | $5.46 \times 10^{-2}$ |
| | | $^5S_2$ | 600 | $1.91 \times 10^{-2}$ | $^3L_9$ | 28873 | $^5I_8$ | 346 | $6.72 \times 10^{-1}$ |
| | | $^5F_4$ | 607 | 1.63 | | | $^3K_8$ | 1226 | 1.73 |
| | | $^5F_3$ | 690 | $1.08 \times 10^{-1}$ | $^5G_3$ | 28112 | $^5I_4$ | 671 | $7.55 \times 10^{-4}$ |
| | | $^5F_2$ | 712 | $3.26 \times 10^{-2}$ | | | $^5S_2$ | 972 | $9.31 \times 10^{-2}$ |
| | | $^5G_4$ | 1073 | 1.55 | | | $^5F_4$ | 992 | $4.85 \times 10^{-2}$ |
| | | $(^5F, ^5G)_2$ | 1511 | $6.09 \times 10^{-1}$ | | | $^5F_3$ | 1233 | $1.37 \times 10^{-5}$ |
| | | $^5G_3$ | 1566 | $1.94 \times 10^{-1}$ | | | $^5F_2$ | 1304 | $2.33 \times 10^{-2}$ |
| $(^5D, ^5G)_4$ | 33877 | $^5I_5$ | 440 | $2.72 \times 10^{-1}$ | $(^5F, ^5G)_2$ | 27879 | $^5S_2$ | 995 | 2.86 |
| | | $^5I_4$ | 484 | 1.35 | | | $^5F_3$ | 1270 | 6.4 |
| | | $^5F_5$ | 528 | $2.17 \times 10^{-1}$ | | | $^5F_2$ | 1345 | $5.38 \times 10^{-1}$ |
| | | $^5F_4$ | 631 | $8.45 \times 10^{-1}$ | | | $^5F_1$ | 1618 | 1.32 |
| | | $^5F_3$ | 721 | $4.48 \times 10^{-1}$ | $^3H_6$ | 27317 | $^5I_7$ | 449 | $2.47 \times 10^{1}$ |
| | | $(^5G, ^3G)_5$ | 944 | $9.71 \times 10^{-1}$ | | | $^5I_6$ | 531 | 1.55 |
| | | $^5G_4$ | 1150 | $9.34 \times 10^{-2}$ | | | $^5I_5$ | 618 | $1.09 \times 10^{-1}$ |
| | | $(^5G, ^3H)_5$ | 1438 | 6.48 | | | $^5F_5$ | 807 | 1.01 |
| $^3L_8$ | 33577 | $^5I_7$ | 351 | $9.43 \times 10^{-1}$ | | | $^5G_6$ | 1663 | $8.18 \times 10^{-1}$ |
| | | $^3K_8$ | 777 | $1.14 \times 10^{1}$ | $(^5G, ^3H)_5$ | 26922 | $^5I_6$ | 543 | 8.35 |
| | | $^3K_7$ | 1259 | $3.46 \times 10^{-1}$ | | | $^5I_5$ | 634 | 2.26 |
| $^3P_1$ | 32942 | $^5S_2$ | 661 | 6.19 | | | $^5I_4$ | 729 | $6.69 \times 10^{-1}$ |
| | | $^5F_2$ | 800 | 5. | | | $^5F_5$ | 833 | 4.26 |
| | | $^5F_1$ | 890 | 4.91 | | | $^5F_4$ | 1125 | $3.98 \times 10^{-1}$ |
| $^3D_3$ | 32901 | $^5I_4$ | 508 | $3.58 \times 10^{-2}$ | $^3K_7$ | 25636 | $^5I_8$ | 390 | 1.4 |
| | | $^5S_2$ | 663 | $9.79 \times 10^{-1}$ | | | $^5I_7$ | 486 | 8.68 |
| | | $^5F_4$ | 672 | $1.23 \times 10^{1}$ | | | $^5I_6$ | 583 | 3.68 |
| | | $^5F_3$ | 775 | $2.64 \times 10^{-1}$ | $^5G_4$ | 25181 | $^5I_5$ | 712 | $3.72 \times 10^{-4}$ |

[a] The emission rate, $A_{md}$, inside a host material with refractive index $n_r$ would be: $A_{md} = A'_{md}\ n_r^3$

TABLE S10: Continued: $Ho^{3+}$ MD spontaneous emission lines between 300 and 1700 nm.

| $SLJ$ | $E_{SLJ}(cm^{-1})$ | $S'L'J'$ | $\lambda$ (nm) | $A'_{md}$ $(s^{-1})$ [a] | $SLJ$ | $E_{SLJ}(cm^{-1})$ | $S'L'J'$ | $\lambda$ (nm) | $A'_{md}$ $(s^{-1})$ [a] |
|---|---|---|---|---|---|---|---|---|---|
| $^5G_4$ | 25181 | $^5I_4$ | 835 | $1.53 \times 10^{-1}$ | $^5G_6$ | 21306 | $^5I_6$ | 781 | $5.64 \times 10^{-1}$ |
| | | $^5F_5$ | 975 | 2.63 | | | $^5I_5$ | 983 | $1.91 \times 10^{-1}$ |
| | | $^5F_4$ | 1398 | $6.7 \times 10^{-2}$ | | | $^5F_5$ | 1566 | $2.73 \times 10^{-2}$ |
| $\left(^5G, {}^3G\right)_5$ | 23286 | $^5I_6$ | 676 | 2.45 | $^3K_8$ | 20715 | $^5I_8$ | 483 | $1.85 \times 10^{1}$ |
| | | $^5I_5$ | 823 | $1.66 \times 10^{-1}$ | | | $^5I_7$ | 639 | 2.71 |
| | | $^5I_4$ | 992 | $8.62 \times 10^{-2}$ | $^5F_3$ | 20005 | $^5I_4$ | 1470 | $3.96 \times 10^{-3}$ |
| | | $^5F_5$ | 1196 | 2.09 | $^5F_4$ | 18030 | $^5I_5$ | 1451 | $6.17 \times 10^{-2}$ |
| $^5G_6$ | 21306 | $^5I_7$ | 616 | 3.89 | $^5F_5$ | 14921 | $^5I_6$ | 1556 | $4.57 \times 10^{-1}$ |

[a] The emission rate, $A_{md}$, inside a host material with refractive index $n_r$ would be: $A_{md} = A'_{md}\ n_r^3$

TABLE S11: Calculated $Er^{3+}$ MD spontaneous emission lines between 300 and 1700 nm.

| $SLJ$ | $E_{SLJ}(cm^{-1})$ | $S'L'J'$ | $\lambda$ (nm) | $A'_{md}$ $(s^{-1})$ [a] | $SLJ$ | $E_{SLJ}(cm^{-1})$ | $S'L'J'$ | $\lambda$ (nm) | $A'_{md}$ $(s^{-1})$ [a] |
|---|---|---|---|---|---|---|---|---|---|
| $^4D_{7/2}$ | 37455 | $(^4I, ^2H)_{9/2}$ | 394 | $6.14 \times 10^{-3}$ | $^2K_{13/2}$ | 32597 | $^4I_{15/2}$ | 307 | $4.03 \times 10^{-1}$ |
| | | $^4F_{9/2}$ | 440 | $1.02 \times 10^{-2}$ | | | $^4I_{13/2}$ | 384 | 5.25 |
| | | $^4F_{7/2}$ | 566 | $2.72 \times 10^{-2}$ | | | $^4I_{11/2}$ | 446 | 3.76 |
| | | $^4F_{5/2}$ | 628 | $7.03 \times 10^{-1}$ | | | $(^2H, ^4G)_{11/2}$ | 712 | $6.97 \times 10^{-2}$ |
| | | $(^2G, ^4F)_{9/2}$ | 733 | $4.68 \times 10^{-1}$ | | | $^4G_{11/2}$ | 1399 | $1.86 \times 10^{-3}$ |
| | | $^4G_{9/2}$ | 904 | $7.5 \times 10^{-1}$ | $^4G_{5/2}$ | 32171 | $^4S_{3/2}$ | 691 | $6.93 \times 10^{-2}$ |
| | | $(^2G, ^4G)_{7/2}$ | 960 | $6.22 \times 10^{-1}$ | | | $^4F_{7/2}$ | 807 | $3.91 \times 10^{-1}$ |
| $^2D_{5/2}$ | 36928 | $^4S_{3/2}$ | 520 | 2.27 | | | $^4F_{5/2}$ | 940 | $1.19 \times 10^{-1}$ |
| | | $^4F_{7/2}$ | 583 | 5.05 | | | $^4F_{3/2}$ | 962 | $1.09 \times 10^{-1}$ |
| | | $^4F_{5/2}$ | 649 | $2.01 \times 10^{-1}$ | $(^2P, ^2D)_{3/2}$ | 30781 | $^4S_{3/2}$ | 764 | 5.55 |
| | | $^4F_{3/2}$ | 660 | $1.91 \times 10^{-1}$ | | | $^4F_{5/2}$ | 1081 | 8.19 |
| | | $(^2G, ^4G)_{7/2}$ | 1011 | $5.07 \times 10^{-1}$ | | | $^4F_{3/2}$ | 1111 | 8.56 |
| | | $(^2P, ^2D)_{3/2}$ | 1627 | 1.41 | $^2K_{15/2}$ | 27315 | $^4I_{15/2}$ | 366 | $1.82 \times 10^{1}$ |
| $(^2H, ^2G)_{9/2}$ | 35679 | $^4I_{11/2}$ | 392 | 5.34 | | | $^4I_{13/2}$ | 481 | 3.78 |
| | | $(^4I, ^2H)_{9/2}$ | 423 | $9.2 \times 10^{-1}$ | $(^2G, ^4G)_{7/2}$ | 27038 | $(^4I, ^2H)_{9/2}$ | 667 | 1.45 |
| | | $^4F_{9/2}$ | 477 | $1.36 \times 10^{-1}$ | | | $^4F_{9/2}$ | 813 | $3.5 \times 10^{-1}$ |
| | | $(^2H, ^4G)_{11/2}$ | 584 | 3.96 | | | $^4F_{7/2}$ | 1378 | $7.68 \times 10^{-1}$ |
| | | $^4F_{7/2}$ | 629 | $7.67 \times 10^{-1}$ | $^4G_{9/2}$ | 26394 | $^4I_{11/2}$ | 616 | $3.52 \times 10^{-1}$ |
| | | $(^2G, ^4F)_{9/2}$ | 843 | $1.12 \times 10^{1}$ | | | $(^4I, ^2H)_{9/2}$ | 697 | 1.04 |
| | | $^4G_{11/2}$ | 978 | $1.19 \times 10^{1}$ | | | $^4F_{9/2}$ | 858 | 2.58 |
| | | $^4G_{9/2}$ | 1077 | 4.11 | | | $(^2H, ^4G)_{11/2}$ | 1276 | $1.22 \times 10^{1}$ |
| | | $(^2G, ^4G)_{7/2}$ | 1157 | $1.41 \times 10^{-2}$ | | | $^4F_{7/2}$ | 1512 | $2. \times 10^{-2}$ |
| $^2D_{5/2}$ | 34353 | $^4S_{3/2}$ | 600 | $5.45 \times 10^{-3}$ | $^4G_{11/2}$ | 25449 | $^4I_{13/2}$ | 529 | $1.24 \times 10^{1}$ |
| | | $^4F_{7/2}$ | 686 | $2. \times 10^{1}$ | | | $^4I_{11/2}$ | 654 | $3.57 \times 10^{-2}$ |
| | | $^4F_{5/2}$ | 780 | 1.67 | | | $(^4I, ^2H)_{9/2}$ | 747 | $2.9 \times 10^{-1}$ |
| | | $^4F_{3/2}$ | 795 | 1.11 | | | $^4F_{9/2}$ | 933 | $7.01 \times 10^{-1}$ |
| | | $(^2G, ^4G)_{7/2}$ | 1367 | $1.85 \times 10^{-1}$ | | | $(^2H, ^4G)_{11/2}$ | 1451 | 2.86 |
| $^4G_{7/2}$ | 32919 | $(^4I, ^2H)_{9/2}$ | 479 | 2.42 | $(^2G, ^4F)_{9/2}$ | 23816 | $^4I_{11/2}$ | 733 | 8.48 |
| | | $^4F_{9/2}$ | 550 | $9.08 \times 10^{-1}$ | | | $(^4I, ^2H)_{9/2}$ | 850 | $1.39 \times 10^{-3}$ |
| | | $^4F_{7/2}$ | 761 | 3.15 | | | $^4F_{9/2}$ | 1101 | $1.04 \times 10^{1}$ |
| | | $^4F_{5/2}$ | 878 | 1.08 | $^4F_{7/2}$ | 19779 | $(^4I, ^2H)_{9/2}$ | 1294 | 3.96 |
| | | $(^2G, ^4F)_{9/2}$ | 1098 | $1.33 \times 10^{-1}$ | $(^2H, ^4G)_{11/2}$ | 18558 | $^4I_{13/2}$ | 832 | $1.49 \times 10^{1}$ |
| | | $^4G_{9/2}$ | 1533 | 6.43 | | | $^4I_{11/2}$ | 1192 | 1.95 |
| $^2P_{1/2}$ | 32649 | $^4S_{3/2}$ | 668 | $1.13 \times 10^{1}$ | | | $(^4I, ^2H)_{9/2}$ | 1537 | $1.47 \times 10^{-1}$ |
| | | $^4F_{3/2}$ | 920 | $1.33 \times 10^{-1}$ | $^4I_{13/2}$ | 6543 | $^4I_{15/2}$ | 1528 | $1.02 \times 10^{1}$ |

[a] The emission rate, $A_{md}$, inside a host material with refractive index $n_r$ would be: $A_{md} = A'_{md}\ n_r^3$

TABLE S12: Calculated $Tm^{3+}$ MD spontaneous emission lines between 300 and 1700 nm.

| $SLJ$ | $E_{SLJ}(cm^{-1})$ | $S'L'J'$ | $\lambda$ (nm) | $A'_{md}$ $(s^{-1})$ [a] | $SLJ$ | $E_{SLJ}(cm^{-1})$ | $S'L'J'$ | $\lambda$ (nm) | $A'_{md}$ $(s^{-1})$ [a] |
|---|---|---|---|---|---|---|---|---|---|
| $\left({}^3P,\,{}^1D\right)_2$ | 37218 | ${}^3F_3$ | 430 | $2.29 \times 10^1$ | ${}^1G_4$ | 20962 | ${}^3F_4$ | 639 | 1.91 |
| | | ${}^3F_2$ | 443 | $3.57 \times 10^{-1}$ | | | ${}^3H_5$ | 784 | $2.26 \times 10^1$ |
| | | $\left({}^3P,\,{}^1D\right)_2$ | 983 | $1.3 \times 10^1$ | | | ${}^3H_4$ | 1167 | 5.6 |
| ${}^3P_1$ | 34665 | ${}^3F_2$ | 500 | 3.96 | | | ${}^3F_3$ | 1431 | $6.49 \times 10^{-1}$ |
| | | $\left({}^3P,\,{}^1D\right)_2$ | 1312 | 4.79 | ${}^3F_3$ | 13973 | ${}^3F_4$ | 1155 | $1.09 \times 10^1$ |
| ${}^1I_6$ | 34212 | ${}^3H_5$ | 385 | 3.51 | ${}^3H_4$ | 12394 | ${}^3F_4$ | 1412 | 3.96 |
| $\left({}^3P,\,{}^1D\right)_2$ | 27046 | ${}^3F_3$ | 765 | $1.4 \times 10^1$ | ${}^3H_5$ | 8205 | ${}^3H_6$ | 1219 | $1.45 \times 10^1$ |
| | | ${}^3F_2$ | 808 | 9.29 | | | | | |

[a] The emission rate, $A_{md}$, inside a host material with refractive index $n_r$ would be: $A_{md} = A'_{md}\ n_r^3$

TABLE S13: Calculated $Yb^{3+}$ MD spontaneous emission lines between 300 and 1700 nm.

| $SLJ$ | $E_{SLJ}(cm^{-1})$ | $S'L'J'$ | $\lambda$ (nm) | $A'_{md}$ $(s^{-1})$ [a] | $SLJ$ | $E_{SLJ}(cm^{-1})$ | $S'L'J'$ | $\lambda$ (nm) | $A'_{md}$ $(s^{-1})$ [a] |
|---|---|---|---|---|---|---|---|---|---|
| ${}^2F_{5/2}$ | 10248 | ${}^2F_{7/2}$ | 976 | $1.66 \times 10^1$ | | | | | |

[a] The emission rate, $A_{md}$, inside a host material with refractive index $n_r$ would be: $A_{md} = A'_{md}\ n_r^3$

TABLE S14: Electric quadrupole ground state absorption lines between 300 and 1700 nm.

| | $SLJ$ | $S'L'J'$ | E(cm$^{-1}$) | $\lambda(nm)$ | $P'_{eq}$ [a] |
|---|---|---|---|---|---|
| $Ce^{3+}$ | $^2F_{5/2}$ | $^2F_{7/2}$ | 2266 | 4414 | $1.02 \times 10^{-13}$ |
| $Pr^{3+}$ | $^3H_4$ | $^3H_5$ | 2092 | 4781 | $4.07 \times 10^{-14}$ |
| | | $^3H_6$ | 4258 | 2348 | $2.58 \times 10^{-16}$ |
| | | $^3F_2$ | 4895 | 2043 | $2.43 \times 10^{-12}$ |
| | | $^3F_3$ | 6290 | 1590 | $6.6 \times 10^{-13}$ |
| | | $^3F_4$ | 6720 | 1488 | $2.34 \times 10^{-13}$ |
| | | $^1G_4$ | 9734 | 1027 | $5.27 \times 10^{-14}$ |
| | | $^1D_2$ | 16815 | 595 | $5.42 \times 10^{-13}$ |
| | | $^1I_6$ | 21302 | 469 | $3.71 \times 10^{-12}$ |
| | | $^3P_2$ | 22467 | 445 | $2.15 \times 10^{-14}$ |
| $Nd^{3+}$ | $^4I_{9/2}$ | $^4I_{11/2}$ | 1829 | 5468 | $3.67 \times 10^{-15}$ |
| | | $^4I_{13/2}$ | 3801 | 2631 | $7.75 \times 10^{-17}$ |
| | | $^2H_{9/2}$ | 12167 | 822 | $5.94 \times 10^{-13}$ |
| | | $^4F_{5/2}$ | 12348 | 810 | $7.62 \times 10^{-14}$ |
| | | $^4F_{7/2}$ | 13277 | 753 | $1.01 \times 10^{-13}$ |
| | | $^4F_{9/2}$ | 14540 | 688 | $6.43 \times 10^{-14}$ |
| | | $^2H_{11/2}$ | 15445 | 647 | $5.76 \times 10^{-15}$ |
| | | $^2G_{7/2}$ | 16892 | 592 | $9.44 \times 10^{-12}$ |
| | | $^4G_{5/2}$ | 17107 | 585 | $1.43 \times 10^{-10}$ |
| | | $^4G_{7/2}$ | 18925 | 528 | $1.48 \times 10^{-11}$ |
| | | $^4G_{9/2}$ | 19266 | 519 | $9.13 \times 10^{-13}$ |
| | | $^2K_{13/2}$ | 19550 | 512 | $1.7 \times 10^{-12}$ |
| | | $^2G_{9/2}$ | 20810 | 481 | $4.84 \times 10^{-13}$ |
| | | $^4G_{11/2}$ | 21354 | 468 | $1.67 \times 10^{-15}$ |
| | | $^2D_{5/2}$ | 23747 | 421 | $4.33 \times 10^{-19}$ |
| | | $^4D_{5/2}$ | 28293 | 353 | $9.7 \times 10^{-14}$ |
| | | $^2I_{11/2}$ | 29454 | 340 | $5.17 \times 10^{-12}$ |
| | | $^4D_{7/2}$ | 30290 | 330 | $5.3 \times 10^{-16}$ |
| | | $^2I_{13/2}$ | 30777 | 325 | $1.81 \times 10^{-13}$ |
| | | $^2H_{9/2}$ | 33253 | 301 | $7.52 \times 10^{-14}$ |
| $Pm^{3+}$ | $^5I_4$ | $^5I_5$ | 1462 | 6841 | $2.35 \times 10^{-15}$ |
| | | $^5I_6$ | 3000 | 3333 | $1.64 \times 10^{-15}$ |
| | | $^5F_2$ | 12626 | 792 | $2.06 \times 10^{-13}$ |
| | | $^5F_3$ | 13466 | 743 | $4.72 \times 10^{-15}$ |
| | | $^5S_2$ | 14122 | 708 | $5.58 \times 10^{-16}$ |
| | | $^5F_4$ | 14432 | 693 | $4.88 \times 10^{-14}$ |
| | | $^5F_5$ | 15793 | 633 | $6.18 \times 10^{-16}$ |
| | | $^3K_6$ | 15967 | 626 | $2.72 \times 10^{-13}$ |
| | | $\left(^3H, ^5G\right)_4$ | 17376 | 575 | $1.42 \times 10^{-12}$ |
| | | $^5G_2$ | 17590 | 569 | $1.23 \times 10^{-10}$ |
| | | $^5G_3$ | 17896 | 559 | $2.67 \times 10^{-11}$ |
| | | $\left(^3H, ^5G\right)_5$ | 19610 | 510 | $3.11 \times 10^{-14}$ |
| | | $^5G_4$ | 20038 | 499 | $1.74 \times 10^{-12}$ |
| $Pm^{3+}$ | $^5I_4$ | $^3G_3$ | 21688 | 461 | $5.03 \times 10^{-12}$ |
| | | $^5G_5$ | 21885 | 457 | $8.79 \times 10^{-14}$ |
| | | $^5G_6$ | 22183 | 451 | $7.49 \times 10^{-19}$ |
| | | $^3D_2$ | 23059 | 434 | $8.72 \times 10^{-13}$ |
| | | $^3H_6$ | 24011 | 416 | $2.66 \times 10^{-15}$ |
| | | $^3G_4$ | 24499 | 408 | $4.64 \times 10^{-13}$ |
| | | $^3D_3$ | 25695 | 389 | $1.65 \times 10^{-13}$ |
| | | $\left(^1D, ^3F\right)_2$ | 26210 | 382 | $1.16 \times 10^{-13}$ |
| | | $^3G_5$ | 27022 | 370 | $9.78 \times 10^{-14}$ |
| | | $^3F_4$ | 27046 | 370 | $2.72 \times 10^{-16}$ |
| | | $^3I_5$ | 28207 | 355 | $3.01 \times 10^{-12}$ |
| | | $\left(^3F, ^3P\right)_2$ | 28583 | 350 | $2.49 \times 10^{-13}$ |
| | | $^3F_3$ | 29121 | 343 | $4.32 \times 10^{-14}$ |
| | | $^3I_6$ | 29326 | 341 | $2.76 \times 10^{-13}$ |
| | | $^3F_2$ | 29631 | 337 | $4.79 \times 10^{-12}$ |
| | | $^5D_2$ | 31078 | 322 | $2.29 \times 10^{-13}$ |
| | | $^5D_3$ | 31821 | 314 | $2.85 \times 10^{-14}$ |
| | | $^5D_4$ | 32302 | 310 | $7.81 \times 10^{-15}$ |
| | | $^3F_3$ | 32958 | 303 | $7.43 \times 10^{-13}$ |
| $Sm^{3+}$ | $^6H_{5/2}$ | $^6H_{7/2}$ | 1069 | 9355 | $1.03 \times 10^{-14}$ |
| | | $^6H_{9/2}$ | 2275 | 4396 | $1.25 \times 10^{-14}$ |
| | | $^6F_{1/2}$ | 6211 | 1610 | $1.92 \times 10^{-12}$ |
| | | $^6F_{3/2}$ | 6416 | 1559 | $1.58 \times 10^{-12}$ |
| | | $^6F_{5/2}$ | 6883 | 1453 | $4.4 \times 10^{-13}$ |
| | | $^6F_{7/2}$ | 7756 | 1289 | $3.68 \times 10^{-14}$ |
| | | $^6F_{9/2}$ | 8964 | 1116 | $5.63 \times 10^{-16}$ |
| | | $^4G_{5/2}$ | 18115 | 552 | $9.77 \times 10^{-14}$ |
| | | $^4F_{3/2}$ | 18918 | 529 | $3.24 \times 10^{-14}$ |
| | | $^4G_{7/2}$ | 20172 | 496 | $1.75 \times 10^{-13}$ |
| | | $^4I_{9/2}$ | 21456 | 466 | $9.61 \times 10^{-13}$ |
| | | $^4F_{5/2}$ | 22177 | 451 | $1.66 \times 10^{-13}$ |
| | | $^4G_{9/2}$ | 22742 | 440 | $3.41 \times 10^{-14}$ |
| | | $\left(^6P, ^4P\right)_{5/2}$ | 23849 | 419 | $7.37 \times 10^{-16}$ |
| | | $^6P_{3/2}$ | 24698 | 405 | $7.05 \times 10^{-15}$ |
| | | $^4F_{7/2}$ | 24889 | 402 | $1.52 \times 10^{-13}$ |
| | | $^4D_{1/2}$ | 26269 | 381 | $1.52 \times 10^{-13}$ |
| | | $^6P_{7/2}$ | 26443 | 378 | $1.1 \times 10^{-15}$ |
| | | $^4D_{3/2}$ | 27403 | 365 | $1.59 \times 10^{-13}$ |
| | | $^4F_{9/2}$ | 27421 | 365 | $4.31 \times 10^{-14}$ |
| | | $\left(^4D, ^6P\right)_{5/2}$ | 27469 | 364 | $5.18 \times 10^{-14}$ |
| | | $^4H_{7/2}$ | 28715 | 348 | $2.37 \times 10^{-12}$ |
| | | $^4D_{7/2}$ | 28813 | 347 | $3.65 \times 10^{-14}$ |
| | | $^4H_{9/2}$ | 29282 | 342 | $3.26 \times 10^{-13}$ |

[a] The oscillator strength, $P_{eq}$, inside a host material with refractive index $n_r$ would be: $P_{eq} = P'_{eq}\ n_r^3$

TABLE S14: Continued: Electric quadrupole ground state absorption lines between 300 and 1700 nm.

| | $SLJ$ | $S'L'J'$ | E($cm^{-1}$) | $\lambda(nm)$ | $P'_{eq}$ [a] | | $SLJ$ | $S'L'J'$ | E($cm^{-1}$) | $\lambda(nm)$ | $P'_{eq}$ [a] |
|---|---|---|---|---|---|---|---|---|---|---|---|
| $Sm^{3+}$ | $^6H_{5/2}$ | $^4G_{7/2}$ | 29992 | 333 | $2.21 \times 10^{-14}$ | $Dy^{3+}$ | $^6H_{15/2}$ | $^4K_{17/2}$ | 25967 | 385 | $2.02 \times 10^{-12}$ |
| | | $^4G_{5/2}$ | 30079 | 332 | $1.84 \times 10^{-13}$ | | | $^4I_{13/2}$ | 26050 | 384 | $6.12 \times 10^{-13}$ |
| | | $^4G_{9/2}$ | 30108 | 332 | $5.63 \times 10^{-15}$ | | | $^4M_{19/2}$ | 26833 | 373 | $4.52 \times 10^{-14}$ |
| | | $^4P_{1/2}$ | 30973 | 323 | $4.23 \times 10^{-15}$ | | | $^4I_{11/2}$ | 28569 | 350 | $1.39 \times 10^{-14}$ |
| | | $^4P_{3/2}$ | 31340 | 319 | $8.29 \times 10^{-16}$ | | | $^4M_{15/2}$ | 29534 | 339 | $4.7 \times 10^{-13}$ |
| | | $^4P_{5/2}$ | 32581 | 307 | $1.72 \times 10^{-15}$ | | | $^4M_{17/2}$ | 29740 | 336 | $5.23 \times 10^{-13}$ |
| $Eu^{3+}$ | $^7F_0$ | $^7F_2$ | 1069 | 9358 | $3.71 \times 10^{-14}$ | | | $^4K_{15/2}$ | 30846 | 324 | $8.18 \times 10^{-13}$ |
| | | $^5D_2$ | 21752 | 460 | $1.99 \times 10^{-12}$ | | | $^4L_{19/2}$ | 30894 | 324 | $1.1 \times 10^{-13}$ |
| | | $^5G_2$ | 26423 | 378 | $2.11 \times 10^{-12}$ | | | $\left(^4K, ^4L\right)_{13/2}$ | 33321 | 300 | $5.92 \times 10^{-13}$ |
| | | $^5F_2$ | 33261 | 301 | $4.06 \times 10^{-12}$ | $Ho^{3+}$ | $^5I_8$ | $^5I_7$ | 5064 | 1975 | $2.74 \times 10^{-14}$ |
| $Gd^{3+}$ | $^8S_{7/2}$ | $^6P_{7/2}$ | 32557 | 307 | $1.12 \times 10^{-12}$ | | | $^5I_6$ | 8495 | 1177 | $5.21 \times 10^{-14}$ |
| | | $^6P_{5/2}$ | 33169 | 301 | $4.84 \times 10^{-13}$ | | | $^3K_8$ | 20715 | 483 | $1.62 \times 10^{-12}$ |
| $Tb^{3+}$ | $^7F_6$ | $^7F_5$ | 1999 | 5003 | $5.83 \times 10^{-14}$ | | | $^5G_6$ | 21306 | 469 | $1.29 \times 10^{-10}$ |
| | | $^7F_4$ | 3249 | 3078 | $4.13 \times 10^{-14}$ | | | $^3K_7$ | 25636 | 390 | $9.38 \times 10^{-13}$ |
| | | $^5D_4$ | 20881 | 479 | $1.18 \times 10^{-13}$ | | | $^3H_6$ | 27317 | 366 | $2.88 \times 10^{-11}$ |
| | | $^5G_6$ | 27004 | 370 | $5.18 \times 10^{-13}$ | | | $^3L_9$ | 28873 | 346 | $3.95 \times 10^{-12}$ |
| | | $^5G_5$ | 28252 | 354 | $3.87 \times 10^{-13}$ | | | $^3K_6$ | 29625 | 338 | $8.01 \times 10^{-13}$ |
| | | $^5G_4$ | 28673 | 349 | $4.25 \times 10^{-14}$ | $Er^{3+}$ | $^4I_{15/2}$ | $^4I_{13/2}$ | 6543 | 1528 | $4.65 \times 10^{-14}$ |
| | | $^5L_8$ | 29334 | 341 | $2.92 \times 10^{-15}$ | | | $^4I_{11/2}$ | 10167 | 984 | $2.84 \times 10^{-13}$ |
| | | $^5L_7$ | 29678 | 337 | $2.08 \times 10^{-13}$ | | | $\left(^2H, ^4G\right)_{11/2}$ | 18558 | 539 | $4.23 \times 10^{-11}$ |
| | | $^5L_6$ | 30042 | 333 | $5.45 \times 10^{-14}$ | | | $^4G_{11/2}$ | 25449 | 393 | $1.13 \times 10^{-10}$ |
| | | $^5H_7$ | 31843 | 314 | $2.5 \times 10^{-12}$ | | | $^2K_{15/2}$ | 27315 | 366 | $3.71 \times 10^{-12}$ |
| | | $^5H_6$ | 33279 | 300 | $1.24 \times 10^{-12}$ | | | $^2K_{13/2}$ | 32597 | 307 | $8.8 \times 10^{-13}$ |
| $Dy^{3+}$ | $^6H_{15/2}$ | $^6H_{13/2}$ | 3316 | 3016 | $8.98 \times 10^{-14}$ | $Tm^{3+}$ | $^3H_6$ | $^3F_4$ | 5314 | 1882 | $7.69 \times 10^{-13}$ |
| | | $^6H_{11/2}$ | 5626 | 1777 | $1.5 \times 10^{-13}$ | | | $^3H_5$ | 8205 | 1219 | $5.5 \times 10^{-13}$ |
| | | $^6F_{11/2}$ | 7429 | 1346 | $3.83 \times 10^{-12}$ | | | $^3H_4$ | 12394 | 807 | $3.98 \times 10^{-12}$ |
| | | $^4I_{15/2}$ | 22691 | 441 | $7.16 \times 10^{-13}$ | | | $^1G_4$ | 20962 | 477 | $3.8 \times 10^{-12}$ |
| | | $^4G_{11/2}$ | 23594 | 424 | $2.89 \times 10^{-14}$ | $Yb^{3+}$ | $^2F_{7/2}$ | $^2F_{5/2}$ | 10248 | 976 | $1.86 \times 10^{-12}$ |

[a] The oscillator strength, $P_{eq}$, inside a host material with refractive index $n_r$ would be: $P_{eq} = P'_{eq}\, n_r^3$

TABLE S15: Calculated $Pr^{3+}$ EQ spontaneous emission lines between 300 and 1700 nm.

| $SLJ$ | $E_{SLJ}(cm^{-1})$ | $S'L'J'$ | $\lambda$ (nm) | $A'_{eq}$ $(s^{-1})$ [a] | $SLJ$ | $E_{SLJ}(cm^{-1})$ | $S'L'J'$ | $\lambda$ (nm) | $A'_{eq}$ $(s^{-1})$ [a] |
|---|---|---|---|---|---|---|---|---|---|
| $^3P_2$ | 22467 | $^3H_4$ | 445 | $4.02 \times 10^{-6}$ | $^3P_1$ | 21288 | $^3F_3$ | 667 | $6.47 \times 10^{-3}$ |
| | | $^3F_2$ | 569 | $2.57 \times 10^{-3}$ | $^3P_0$ | 20633 | $^3F_2$ | 635 | $2.78 \times 10^{-3}$ |
| | | $^3F_3$ | 618 | $7.04 \times 10^{-3}$ | $^1D_2$ | 16815 | $^3H_4$ | 595 | $5.68 \times 10^{-5}$ |
| | | $^3F_4$ | 635 | $6.12 \times 10^{-3}$ | | | $^3F_2$ | 839 | $1.67 \times 10^{-4}$ |
| | | $^1G_4$ | 785 | $3.35 \times 10^{-3}$ | | | $^3F_3$ | 950 | $1.06 \times 10^{-4}$ |
| $^1I_6$ | 21302 | $^3H_4$ | 469 | $1.62 \times 10^{-3}$ | | | $^3F_4$ | 991 | $9.47 \times 10^{-4}$ |
| | | $^3H_5$ | 521 | $2.25 \times 10^{-5}$ | | | $^1G_4$ | 1412 | $8.05 \times 10^{-5}$ |
| | | $^3H_6$ | 587 | $1. \times 10^{-4}$ | $^1G_4$ | 9734 | $^3H_4$ | 1027 | $3.33 \times 10^{-6}$ |
| | | $^3F_4$ | 686 | $2.21 \times 10^{-3}$ | | | $^3H_5$ | 1308 | $1.77 \times 10^{-5}$ |
| | | $^1G_4$ | 865 | $1.98 \times 10^{-3}$ | $^3F_4$ | 6720 | $^3H_4$ | 1488 | $7.06 \times 10^{-6}$ |
| $^3P_1$ | 21288 | $^3F_2$ | 610 | $9.29 \times 10^{-3}$ | $^3F_3$ | 6290 | $^3H_4$ | 1590 | $1.35 \times 10^{-5}$ |

[a] The emission rate, $A_{eq}$, inside a host material with refractive index $n_r$ would be: $A_{eq} = A'_{eq}\ n_r^5$

TABLE S16: Calculated $Nd^{3+}$ EQ spontaneous emission lines between 300 and 1700 nm.

| $SLJ$ | $E_{SLJ}(cm^{-1})$ | $S'L'J'$ | $\lambda$ (nm) | $A'_{eq}$ $(s^{-1})$ [a] | $SLJ$ | $E_{SLJ}(cm^{-1})$ | $S'L'J'$ | $\lambda$ (nm) | $A'_{eq}$ $(s^{-1})$ [a] |
|---|---|---|---|---|---|---|---|---|---|
| $^2F_{5/2}$ | 38707 | $^4F_{3/2}$ | 365 | $8.83 \times 10^{-3}$ | $^2D_{5/2}$ | 34177 | $^2G_{9/2}$ | 748 | $2.54 \times 10^{-3}$ |
| | | $^2H_{9/2}$ | 377 | $6. \times 10^{-2}$ | | | $^2D_{3/2}$ | 766 | $1.66 \times 10^{-2}$ |
| | | $^4F_{5/2}$ | 379 | $4.16 \times 10^{-4}$ | | | $^2P_{1/2}$ | 912 | $8.55 \times 10^{-4}$ |
| | | $^4F_{7/2}$ | 393 | $2.56 \times 10^{-3}$ | | | $^2D_{5/2}$ | 959 | $2.65 \times 10^{-5}$ |
| | | $^4S_{3/2}$ | 395 | $6.15 \times 10^{-4}$ | | | $^2P_{3/2}$ | 1247 | $7.61 \times 10^{-6}$ |
| | | $^4F_{9/2}$ | 414 | $1.72 \times 10^{-2}$ | | | $^4D_{3/2}$ | 1660 | $3.42 \times 10^{-5}$ |
| | | $^2G_{7/2}$ | 458 | $7.7 \times 10^{-3}$ | | | $^4D_{5/2}$ | 1700 | $2.35 \times 10^{-8}$ |
| | | $^4G_{5/2}$ | 463 | $2.43 \times 10^{-5}$ | $^2H_{9/2}$ | 33253 | $^4I_{9/2}$ | 301 | $5.54 \times 10^{-5}$ |
| | | $^4G_{7/2}$ | 506 | $3.72 \times 10^{-3}$ | | | $^4I_{11/2}$ | 318 | $2.99 \times 10^{-4}$ |
| | | $^4G_{9/2}$ | 514 | $4.47 \times 10^{-3}$ | | | $^4I_{13/2}$ | 340 | $5.48 \times 10^{-7}$ |
| | | $^2G_{9/2}$ | 559 | $3.18 \times 10^{-3}$ | | | $^2H_{9/2}$ | 474 | $2.02 \times 10^{-4}$ |
| | | $^2D_{3/2}$ | 569 | $2.09 \times 10^{-2}$ | | | $^4F_{5/2}$ | 478 | $4.78 \times 10^{-5}$ |
| | | $^2P_{1/2}$ | 645 | $3.86 \times 10^{-2}$ | | | $^4F_{7/2}$ | 501 | $1.78 \times 10^{-3}$ |
| | | $^2D_{5/2}$ | 668 | $5.22 \times 10^{-3}$ | | | $^4F_{9/2}$ | 534 | $4.72 \times 10^{-5}$ |
| | | $^2P_{3/2}$ | 797 | $8.42 \times 10^{-3}$ | | | $^2H_{11/2}$ | 562 | $4.47 \times 10^{-9}$ |
| | | $^4D_{3/2}$ | 948 | $3.26 \times 10^{-5}$ | | | $^2G_{7/2}$ | 611 | $9.21 \times 10^{-3}$ |
| | | $^4D_{5/2}$ | 960 | $6.67 \times 10^{-5}$ | | | $^4G_{5/2}$ | 619 | $2.96 \times 10^{-5}$ |
| | | $^4D_{1/2}$ | 986 | $8.68 \times 10^{-4}$ | | | $^4G_{7/2}$ | 698 | $2.26 \times 10^{-3}$ |
| | | $^4D_{7/2}$ | 1188 | $1.01 \times 10^{-7}$ | | | $^4G_{9/2}$ | 715 | $9.66 \times 10^{-5}$ |
| $^2H_{11/2}$ | 34646 | $^4I_{11/2}$ | 305 | $1.02 \times 10^{-4}$ | | | $^2K_{13/2}$ | 730 | $5.74 \times 10^{-3}$ |
| | | $^4I_{13/2}$ | 324 | $5.38 \times 10^{-5}$ | | | $^2G_{9/2}$ | 804 | $2.41 \times 10^{-4}$ |
| | | $^4I_{15/2}$ | 348 | $2.88 \times 10^{-5}$ | | | $^4G_{11/2}$ | 840 | $1.12 \times 10^{-6}$ |
| | | $^2H_{9/2}$ | 445 | $2.4 \times 10^{-3}$ | | | $^2D_{5/2}$ | 1052 | $1.86 \times 10^{-5}$ |
| | | $^4F_{7/2}$ | 468 | $1.13 \times 10^{-4}$ | $^2D_{3/2}$ | 33241 | $^4F_{3/2}$ | 457 | $1.4 \times 10^{-3}$ |
| | | $^4F_{9/2}$ | 497 | $7.71 \times 10^{-4}$ | | | $^4F_{5/2}$ | 479 | $1.05 \times 10^{-3}$ |
| | | $^2H_{11/2}$ | 521 | $1.51 \times 10^{-4}$ | | | $^4F_{7/2}$ | 501 | $1.35 \times 10^{-5}$ |
| | | $^2G_{7/2}$ | 563 | $8.23 \times 10^{-5}$ | | | $^4S_{3/2}$ | 504 | $1.39 \times 10^{-3}$ |
| | | $^4G_{7/2}$ | 636 | $7.58 \times 10^{-6}$ | | | $^2G_{7/2}$ | 612 | $2.38 \times 10^{-3}$ |
| | | $^4G_{9/2}$ | 650 | $3.24 \times 10^{-3}$ | | | $^4G_{5/2}$ | 620 | $2.92 \times 10^{-4}$ |
| | | $^2K_{13/2}$ | 662 | $6.34 \times 10^{-5}$ | | | $^4G_{7/2}$ | 699 | $2.69 \times 10^{-3}$ |
| | | $^2G_{9/2}$ | 723 | $3.77 \times 10^{-3}$ | | | $^2D_{3/2}$ | 825 | $3.9 \times 10^{-6}$ |
| | | $^4G_{11/2}$ | 752 | $9.8 \times 10^{-6}$ | | | $^2P_{1/2}$ | 997 | $2.59 \times 10^{-3}$ |
| | | $^2K_{15/2}$ | 762 | $3.9 \times 10^{-3}$ | | | $^2D_{5/2}$ | 1053 | $2.21 \times 10^{-5}$ |
| $^2D_{5/2}$ | 34177 | $^4F_{3/2}$ | 438 | $1.89 \times 10^{-5}$ | | | $^2P_{3/2}$ | 1412 | $3.84 \times 10^{-4}$ |
| | | $^2H_{9/2}$ | 454 | $1.54 \times 10^{-2}$ | $^2L_{17/2}$ | 31674 | $^4I_{13/2}$ | 359 | $1.42 \times 10^{-3}$ |
| | | $^4F_{5/2}$ | 458 | $4.08 \times 10^{-3}$ | | | $^4I_{15/2}$ | 388 | $2.59 \times 10^{-4}$ |
| | | $^4F_{7/2}$ | 478 | $2.15 \times 10^{-3}$ | | | $^2K_{13/2}$ | 825 | $2.46 \times 10^{-5}$ |
| | | $^4S_{3/2}$ | 481 | $2.91 \times 10^{-3}$ | | | $^2K_{15/2}$ | 986 | $1.31 \times 10^{-4}$ |
| | | $^4F_{9/2}$ | 509 | $1.56 \times 10^{-3}$ | $^2I_{13/2}$ | 30777 | $^4I_{9/2}$ | 325 | $1.6 \times 10^{-4}$ |
| | | $^2G_{7/2}$ | 579 | $4.6 \times 10^{-4}$ | | | $^4I_{11/2}$ | 345 | $1.04 \times 10^{-3}$ |
| | | $^4G_{5/2}$ | 586 | $1.32 \times 10^{-4}$ | | | $^4I_{13/2}$ | 371 | $1.26 \times 10^{-4}$ |
| | | $^4G_{7/2}$ | 656 | $2.63 \times 10^{-4}$ | | | $^4I_{15/2}$ | 402 | $5.09 \times 10^{-4}$ |
| | | $^4G_{9/2}$ | 671 | $4.03 \times 10^{-5}$ | | | $^2H_{9/2}$ | 537 | $1.62 \times 10^{-3}$ |

[a] The emission rate, $A_{eq}$, inside a host material with refractive index $n_r$ would be: $A_{eq} = A'_{eq}\ n_r^5$

TABLE S16: Continued: $Nd^{3+}$ EQ spontaneous emission lines between 300 and 1700 nm.

| $SLJ$ | $E_{SLJ}(cm^{-1})$ | $S'L'J'$ | $\lambda$ (nm) | $A'_{eq}$ $(s^{-1})$ [a] | $SLJ$ | $E_{SLJ}(cm^{-1})$ | $S'L'J'$ | $\lambda$ (nm) | $A'_{eq}$ $(s^{-1})$ [a] |
|---|---|---|---|---|---|---|---|---|---|
| $^2I_{13/2}$ | 30777 | $^4F_{9/2}$ | 616 | $2.13 \times 10^{-5}$ | $^2I_{11/2}$ | 29454 | $^2G_{9/2}$ | 1157 | $2.56 \times 10^{-5}$ |
| | | $^2H_{11/2}$ | 652 | $4.44 \times 10^{-3}$ | | | $^4G_{11/2}$ | 1235 | $2.88 \times 10^{-6}$ |
| | | $^4G_{9/2}$ | 869 | $5.04 \times 10^{-5}$ | | | $^2K_{15/2}$ | 1262 | $1.05 \times 10^{-4}$ |
| | | $^2K_{13/2}$ | 891 | $4.84 \times 10^{-6}$ | $^4D_{1/2}$ | 28569 | $^4F_{3/2}$ | 580 | $3.21 \times 10^{-3}$ |
| | | $^2G_{9/2}$ | 1003 | $2.21 \times 10^{-4}$ | | | $^4F_{5/2}$ | 616 | $1.51 \times 10^{-3}$ |
| | | $^4G_{11/2}$ | 1061 | $7.24 \times 10^{-5}$ | | | $^4S_{3/2}$ | 659 | $1.59 \times 10^{-3}$ |
| | | $^2K_{15/2}$ | 1081 | $2.25 \times 10^{-4}$ | | | $^4G_{5/2}$ | 873 | $7.68 \times 10^{-4}$ |
| $^4D_{7/2}$ | 30290 | $^4I_{9/2}$ | 330 | $2.59 \times 10^{-7}$ | | | $^2D_{3/2}$ | 1344 | $3.94 \times 10^{-5}$ |
| | | $^4I_{11/2}$ | 351 | $2.85 \times 10^{-6}$ | $^4D_{5/2}$ | 28293 | $^4I_{9/2}$ | 353 | $3.1 \times 10^{-5}$ |
| | | $^4F_{3/2}$ | 528 | $2.83 \times 10^{-5}$ | | | $^4F_{3/2}$ | 590 | $8.65 \times 10^{-3}$ |
| | | $^2H_{9/2}$ | 552 | $1.29 \times 10^{-3}$ | | | $^2H_{9/2}$ | 620 | $3.47 \times 10^{-3}$ |
| | | $^4F_{5/2}$ | 557 | $3.39 \times 10^{-3}$ | | | $^4F_{5/2}$ | 627 | $8.25 \times 10^{-3}$ |
| | | $^4F_{7/2}$ | 588 | $7.94 \times 10^{-3}$ | | | $^4F_{7/2}$ | 666 | $2.36 \times 10^{-3}$ |
| | | $^4S_{3/2}$ | 592 | $6.41 \times 10^{-2}$ | | | $^4S_{3/2}$ | 671 | $1.98 \times 10^{-2}$ |
| | | $^4F_{9/2}$ | 635 | $8.73 \times 10^{-3}$ | | | $^4F_{9/2}$ | 727 | $6.21 \times 10^{-4}$ |
| | | $^2H_{11/2}$ | 674 | $1.07 \times 10^{-3}$ | | | $^2G_{7/2}$ | 877 | $6.3 \times 10^{-4}$ |
| | | $^2G_{7/2}$ | 746 | $4.61 \times 10^{-4}$ | | | $^4G_{5/2}$ | 894 | $1.51 \times 10^{-4}$ |
| | | $^4G_{5/2}$ | 759 | $9.32 \times 10^{-6}$ | | | $^4G_{7/2}$ | 1067 | $1.62 \times 10^{-4}$ |
| | | $^4G_{7/2}$ | 880 | $2.43 \times 10^{-5}$ | | | $^4G_{9/2}$ | 1108 | $3.44 \times 10^{-4}$ |
| | | $^4G_{9/2}$ | 907 | $7.7 \times 10^{-4}$ | | | $^2G_{9/2}$ | 1336 | $3.38 \times 10^{-5}$ |
| | | $^2G_{9/2}$ | 1055 | $1.47 \times 10^{-5}$ | | | $^2D_{3/2}$ | 1395 | $1.25 \times 10^{-4}$ |
| | | $^2D_{3/2}$ | 1091 | $1.69 \times 10^{-4}$ | $^4D_{3/2}$ | 28154 | $^4F_{3/2}$ | 595 | $1.06 \times 10^{-2}$ |
| | | $^4G_{11/2}$ | 1119 | $7.13 \times 10^{-4}$ | | | $^4F_{5/2}$ | 633 | $1.46 \times 10^{-3}$ |
| | | $^2D_{5/2}$ | 1528 | $5.69 \times 10^{-6}$ | | | $^4F_{7/2}$ | 672 | $2.36 \times 10^{-3}$ |
| $^2L_{15/2}$ | 30204 | $^4I_{11/2}$ | 352 | $1.68 \times 10^{-3}$ | | | $^4S_{3/2}$ | 677 | $8.75 \times 10^{-3}$ |
| | | $^4I_{13/2}$ | 379 | $1.45 \times 10^{-4}$ | | | $^2G_{7/2}$ | 888 | $4.96 \times 10^{-4}$ |
| | | $^4I_{15/2}$ | 412 | $1.14 \times 10^{-8}$ | | | $^4G_{5/2}$ | 905 | $7.13 \times 10^{-4}$ |
| | | $^2H_{11/2}$ | 678 | $7.27 \times 10^{-6}$ | | | $^4G_{7/2}$ | 1084 | $1.81 \times 10^{-4}$ |
| | | $^2K_{13/2}$ | 939 | $3.55 \times 10^{-4}$ | | | $^2D_{3/2}$ | 1423 | $1.75 \times 10^{-7}$ |
| | | $^4G_{11/2}$ | 1130 | $3.41 \times 10^{-7}$ | $^2P_{3/2}$ | 26157 | $^4F_{3/2}$ | 675 | $5.11 \times 10^{-5}$ |
| | | $^2K_{15/2}$ | 1153 | $3.99 \times 10^{-5}$ | | | $^4F_{5/2}$ | 724 | $1.38 \times 10^{-5}$ |
| $^2I_{11/2}$ | 29454 | $^4I_{9/2}$ | 340 | $3.59 \times 10^{-3}$ | | | $^4F_{7/2}$ | 776 | $1.28 \times 10^{-7}$ |
| | | $^4I_{11/2}$ | 362 | $1.46 \times 10^{-4}$ | | | $^4S_{3/2}$ | 784 | $7.12 \times 10^{-5}$ |
| | | $^4I_{13/2}$ | 390 | $1.42 \times 10^{-4}$ | | | $^2G_{7/2}$ | 1079 | $1.28 \times 10^{-6}$ |
| | | $^4I_{15/2}$ | 425 | $7.65 \times 10^{-5}$ | | | $^4G_{5/2}$ | 1105 | $5.79 \times 10^{-6}$ |
| | | $^2H_{9/2}$ | 578 | $6.22 \times 10^{-3}$ | | | $^4G_{7/2}$ | 1383 | $1.11 \times 10^{-6}$ |
| | | $^4F_{7/2}$ | 618 | $1.2 \times 10^{-4}$ | $^2D_{5/2}$ | 23747 | $^4I_{9/2}$ | 421 | $9.77 \times 10^{-11}$ |
| | | $^4F_{9/2}$ | 671 | $6.62 \times 10^{-4}$ | | | $^4F_{3/2}$ | 806 | $1.11 \times 10^{-5}$ |
| | | $^2H_{11/2}$ | 714 | $1.12 \times 10^{-5}$ | | | $^2H_{9/2}$ | 864 | $1.21 \times 10^{-5}$ |
| | | $^2G_{7/2}$ | 796 | $6.39 \times 10^{-4}$ | | | $^4F_{5/2}$ | 877 | $3.21 \times 10^{-8}$ |
| | | $^4G_{7/2}$ | 950 | $2.43 \times 10^{-4}$ | | | $^4F_{7/2}$ | 955 | $6.32 \times 10^{-6}$ |
| | | $^4G_{9/2}$ | 982 | $5.58 \times 10^{-7}$ | | | $^4S_{3/2}$ | 966 | $3.78 \times 10^{-5}$ |
| | | $^2K_{13/2}$ | 1010 | $3.36 \times 10^{-4}$ | | | $^4F_{9/2}$ | 1086 | $1.8 \times 10^{-7}$ |

[a] The emission rate, $A_{eq}$, inside a host material with refractive index $n_r$ would be: $A_{eq} = A'_{eq}\ n_r^5$

TABLE S16: Continued: $Nd^{3+}$ EQ spontaneous emission lines between 300 and 1700 nm.

| $SLJ$ | $E_{SLJ}(cm^{-1})$ | $S'L'J'$ | $\lambda$ (nm) | $A'_{eq}$ $(s^{-1})$ [a] | $SLJ$ | $E_{SLJ}(cm^{-1})$ | $S'L'J'$ | $\lambda$ (nm) | $A'_{eq}$ $(s^{-1})$ [a] |
|---|---|---|---|---|---|---|---|---|---|
| $^2D_{5/2}$ | 23747 | $^2G_{7/2}$ | 1459 | $1.18\times10^{-6}$ | $^2K_{13/2}$ | 19550 | $^4I_{13/2}$ | 635 | $5.86\times10^{-5}$ |
| | | $^4G_{5/2}$ | 1506 | $5.03\times10^{-7}$ | | | $^4I_{15/2}$ | 734 | $2.12\times10^{-7}$ |
| $^2P_{1/2}$ | 23209 | $^4F_{3/2}$ | 843 | $8.42\times10^{-5}$ | | | $^2H_{9/2}$ | 1354 | $7.33\times10^{-5}$ |
| | | $^4F_{5/2}$ | 921 | $1.72\times10^{-5}$ | $^4G_{9/2}$ | 19266 | $^4I_{9/2}$ | 519 | $2.26\times10^{-4}$ |
| | | $^4S_{3/2}$ | 1019 | $4.34\times10^{-5}$ | | | $^4I_{11/2}$ | 573 | $3.09\times10^{-3}$ |
| | | $^4G_{5/2}$ | 1639 | $3.63\times10^{-6}$ | | | $^4I_{13/2}$ | 647 | $8.12\times10^{-3}$ |
| $^2K_{15/2}$ | 21530 | $^4I_{11/2}$ | 508 | $9.64\times10^{-5}$ | | | $^2H_{9/2}$ | 1409 | $1.23\times10^{-5}$ |
| | | $^4I_{13/2}$ | 564 | $4.09\times10^{-5}$ | | | $^4F_{5/2}$ | 1445 | $1.58\times10^{-4}$ |
| | | $^4I_{15/2}$ | 641 | $1.31\times10^{-4}$ | | | $^4F_{7/2}$ | 1670 | $1.27\times10^{-4}$ |
| | | $^2H_{11/2}$ | 1643 | $2.7\times10^{-5}$ | $^4G_{7/2}$ | 18925 | $^4I_{9/2}$ | 528 | $2.84\times10^{-3}$ |
| $^4G_{11/2}$ | 21354 | $^4I_{9/2}$ | 468 | $6.1\times10^{-7}$ | | | $^4I_{11/2}$ | 585 | $1.26\times10^{-2}$ |
| | | $^4I_{11/2}$ | 512 | $2.43\times10^{-4}$ | | | $^4F_{3/2}$ | 1319 | $3.12\times10^{-4}$ |
| | | $^4I_{13/2}$ | 570 | $2.93\times10^{-3}$ | | | $^2H_{9/2}$ | 1480 | $1.09\times10^{-5}$ |
| | | $^4I_{15/2}$ | 648 | $1.36\times10^{-2}$ | | | $^4F_{5/2}$ | 1520 | $1.67\times10^{-4}$ |
| | | $^2H_{9/2}$ | 1089 | $2.45\times10^{-4}$ | $^4G_{5/2}$ | 17107 | $^4I_{9/2}$ | 585 | $1.68\times10^{-2}$ |
| | | $^4F_{7/2}$ | 1238 | $2.37\times10^{-4}$ | $^2G_{7/2}$ | 16892 | $^4I_{9/2}$ | 592 | $1.44\times10^{-3}$ |
| | | $^4F_{9/2}$ | 1468 | $3.67\times10^{-4}$ | | | $^4I_{11/2}$ | 664 | $3.09\times10^{-3}$ |
| | | $^2H_{11/2}$ | 1692 | $1.01\times10^{-7}$ | $^2H_{11/2}$ | 15445 | $^4I_{9/2}$ | 647 | $1.1\times10^{-6}$ |
| $^2D_{3/2}$ | 21126 | $^4F_{3/2}$ | 1022 | $2.76\times10^{-5}$ | | | $^4I_{11/2}$ | 734 | $3.3\times10^{-5}$ |
| | | $^4F_{5/2}$ | 1139 | $6.91\times10^{-6}$ | | | $^4I_{13/2}$ | 859 | $4.85\times10^{-6}$ |
| | | $^4F_{7/2}$ | 1274 | $1.32\times10^{-6}$ | | | $^4I_{15/2}$ | 1050 | $8.57\times10^{-5}$ |
| | | $^4S_{3/2}$ | 1293 | $1.23\times10^{-5}$ | $^4F_{9/2}$ | 14540 | $^4I_{9/2}$ | 688 | $9.06\times10^{-6}$ |
| $^2G_{9/2}$ | 20810 | $^4I_{9/2}$ | 481 | $1.4\times10^{-4}$ | | | $^4I_{11/2}$ | 787 | $3.71\times10^{-6}$ |
| | | $^4I_{11/2}$ | 527 | $1.51\times10^{-3}$ | | | $^4I_{13/2}$ | 931 | $1.65\times10^{-6}$ |
| | | $^4I_{13/2}$ | 588 | $6.71\times10^{-3}$ | $^4F_{7/2}$ | 13277 | $^4I_{9/2}$ | 753 | $9.52\times10^{-6}$ |
| | | $^2H_{9/2}$ | 1157 | $6.23\times10^{-7}$ | | | $^4I_{11/2}$ | 874 | $2.93\times10^{-6}$ |
| | | $^4F_{5/2}$ | 1182 | $1.8\times10^{-4}$ | $^4F_{5/2}$ | 12348 | $^4I_{9/2}$ | 810 | $4.65\times10^{-6}$ |
| | | $^4F_{7/2}$ | 1327 | $1.59\times10^{-4}$ | $^2H_{9/2}$ | 12167 | $^4I_{9/2}$ | 822 | $5.86\times10^{-5}$ |
| | | $^4F_{9/2}$ | 1595 | $2.72\times10^{-5}$ | | | $^4I_{11/2}$ | 967 | $2.64\times10^{-6}$ |
| $^2K_{13/2}$ | 19550 | $^4I_{9/2}$ | 512 | $6.06\times10^{-4}$ | | | $^4I_{13/2}$ | 1195 | $1.80\times10^{-5}$ |
| | | $^4I_{11/2}$ | 564 | $3.37\times10^{-5}$ | | | | | |

[a] The emission rate, $A_{eq}$, inside a host material with refractive index $n_r$ would be: $A_{eq} = A'_{eq}\ n_r^5$

TABLE S17: Calculated $Pm^{3+}$ EQ spontaneous emission lines between 300 and 1700 nm.

| $SLJ$ | $E_{SLJ}(cm^{-1})$ | $S'L'J'$ | $\lambda$ (nm) | $A'_{eq}$ $(s^{-1})$ [a] | $SLJ$ | $E_{SLJ}(cm^{-1})$ | $S'L'J'$ | $\lambda$ (nm) | $A'_{eq}$ $(s^{-1})$ [a] |
|---|---|---|---|---|---|---|---|---|---|
| $^1I_6$ | 39524 | $^5I_8$ | 303 | $1.36 \times 10^{-4}$ | $^1D_2$ | 39005 | $^3F_3$ | 1012 | $1.25 \times 10^{-5}$ |
| | | $^5F_4$ | 399 | $1.69 \times 10^{-5}$ | | | $^3F_2$ | 1067 | $1.48 \times 10^{-5}$ |
| | | $^5F_5$ | 421 | $8. \times 10^{-6}$ | | | $^5D_0$ | 1077 | $1.4 \times 10^{-6}$ |
| | | $^3K_6$ | 425 | $1.01 \times 10^{-5}$ | | | $^5D_1$ | 1142 | $3.64 \times 10^{-7}$ |
| | | $^3K_7$ | 450 | $1.2 \times 10^{-3}$ | | | $^5D_2$ | 1262 | $1.51 \times 10^{-6}$ |
| | | $(^3H,\, ^5G)_4$ | 452 | $7.53 \times 10^{-4}$ | | | $^5D_3$ | 1392 | $1.64 \times 10^{-7}$ |
| | | $^3K_8$ | 482 | $5.93 \times 10^{-4}$ | | | $^5D_4$ | 1492 | $6.61 \times 10^{-6}$ |
| | | $(^3H,\, ^5G)_5$ | 502 | $3.87 \times 10^{-5}$ | | | $^3F_3$ | 1654 | $2.25 \times 10^{-9}$ |
| | | $^5G_4$ | 513 | $3.69 \times 10^{-4}$ | $^1K_7$ | 38569 | $^5I_8$ | 312 | $4.91 \times 10^{-5}$ |
| | | $^5G_5$ | 567 | $2.37 \times 10^{-5}$ | | | $^5F_5$ | 439 | $4.09 \times 10^{-5}$ |
| | | $^5G_6$ | 577 | $4.3 \times 10^{-4}$ | | | $^3K_6$ | 442 | $9. \times 10^{-5}$ |
| | | $^3L_7$ | 626 | $6.04 \times 10^{-6}$ | | | $^3K_7$ | 470 | $8.66 \times 10^{-8}$ |
| | | $^3H_6$ | 645 | $1.13 \times 10^{-3}$ | | | $^3K_8$ | 505 | $2.94 \times 10^{-5}$ |
| | | $(^3L,\, ^3M)_8$ | 659 | $3.72 \times 10^{-6}$ | | | $(^3H,\, ^5G)_5$ | 527 | $1.59 \times 10^{-4}$ |
| | | $^3G_4$ | 666 | $4.96 \times 10^{-6}$ | | | $^5G_5$ | 599 | $5.48 \times 10^{-5}$ |
| | | $^3G_5$ | 800 | $9.04 \times 10^{-5}$ | | | $^5G_6$ | 610 | $8.08 \times 10^{-6}$ |
| | | $^3F_4$ | 801 | $1.11 \times 10^{-4}$ | | | $^3L_7$ | 666 | $5.36 \times 10^{-6}$ |
| | | $(^3M,\, ^3L)_8$ | 811 | $2.5 \times 10^{-4}$ | | | $^3H_6$ | 687 | $3.2 \times 10^{-5}$ |
| | | $^3I_5$ | 884 | $6.61 \times 10^{-5}$ | | | $(^3L,\, ^3M)_8$ | 703 | $6.73 \times 10^{-5}$ |
| | | $^3I_6$ | 981 | $1.11 \times 10^{-5}$ | | | $^3L_9$ | 778 | $1.81 \times 10^{-4}$ |
| | | $^3I_7$ | 1032 | $3.98 \times 10^{-5}$ | | | $^3G_5$ | 866 | $3.48 \times 10^{-6}$ |
| | | $^1L_8$ | 1190 | $1.32 \times 10^{-5}$ | | | $(^3M,\, ^3L)_8$ | 880 | $1.3 \times 10^{-4}$ |
| | | $^5D_4$ | 1385 | $1.41 \times 10^{-5}$ | | | $^3I_5$ | 965 | $8.8 \times 10^{-7}$ |
| | | $^1G_4$ | 1637 | $4.67 \times 10^{-5}$ | | | $^3I_6$ | 1082 | $3.33 \times 10^{-9}$ |
| $^1D_2$ | 39005 | $^5F_1$ | 374 | $8.43 \times 10^{-5}$ | | | $^3M_9$ | 1091 | $1.15 \times 10^{-7}$ |
| | | $^5F_2$ | 379 | $2.37 \times 10^{-5}$ | | | $^3I_7$ | 1145 | $1.66 \times 10^{-5}$ |
| | | $^5F_3$ | 392 | $2.79 \times 10^{-7}$ | | | $^1L_8$ | 1343 | $8.82 \times 10^{-5}$ |
| | | $^5S_2$ | 402 | $1.18 \times 10^{-5}$ | $(^1H,\, ^3H)_5$ | 37739 | $^5I_7$ | 303 | $6.68 \times 10^{-5}$ |
| | | $^5F_4$ | 407 | $1.07 \times 10^{-6}$ | | | $^5F_3$ | 412 | $7.2 \times 10^{-5}$ |
| | | $(^3H,\, ^5G)_4$ | 462 | $5.96 \times 10^{-5}$ | | | $^5F_4$ | 429 | $3.67 \times 10^{-8}$ |
| | | $^5G_2$ | 467 | $7.03 \times 10^{-6}$ | | | $^5F_5$ | 456 | $6.9 \times 10^{-4}$ |
| | | $^5G_3$ | 474 | $5.09 \times 10^{-6}$ | | | $^3K_6$ | 459 | $1.83 \times 10^{-4}$ |
| | | $^5G_4$ | 527 | $1.21 \times 10^{-4}$ | | | $^3K_7$ | 489 | $2.54 \times 10^{-5}$ |
| | | $^3G_3$ | 577 | $2.78 \times 10^{-6}$ | | | $(^3H,\, ^5G)_4$ | 491 | $3.47 \times 10^{-4}$ |
| | | $^3D_2$ | 627 | $1.25 \times 10^{-4}$ | | | $^5G_3$ | 504 | $4.15 \times 10^{-5}$ |
| | | $(^3P,\, ^3D)_1$ | 667 | $1.96 \times 10^{-5}$ | | | $(^3H,\, ^5G)_5$ | 552 | $2.02 \times 10^{-3}$ |
| | | $^3G_4$ | 689 | $4.13 \times 10^{-5}$ | | | $^5G_4$ | 565 | $1.72 \times 10^{-5}$ |
| | | $^3P_0$ | 744 | $3.09 \times 10^{-4}$ | | | $^3G_3$ | 623 | $1.91 \times 10^{-5}$ |
| | | $^3D_3$ | 751 | $8.71 \times 10^{-6}$ | | | $^5G_5$ | 631 | $7.12 \times 10^{-4}$ |
| | | $(^1D,\, ^3F)_2$ | 782 | $1.34 \times 10^{-4}$ | | | $^5G_6$ | 643 | $1.34 \times 10^{-4}$ |
| | | $^3F_4$ | 836 | $7.97 \times 10^{-5}$ | | | $^3L_7$ | 705 | $2.12 \times 10^{-4}$ |
| | | $(^3P,\, ^3D)_1$ | 894 | $2.32 \times 10^{-4}$ | | | $^3H_6$ | 728 | $3.81 \times 10^{-4}$ |
| | | $(^3F,\, ^3P)_2$ | 960 | $4.62 \times 10^{-5}$ | | | $^3G_4$ | 755 | $6.23 \times 10^{-5}$ |

[a] The emission rate, $A_{eq}$, inside a host material with refractive index $n_r$ would be: $A_{eq} = A'_{eq}\ n_r^5$

TABLE S17: Continued: $Pm^{3+}$ EQ spontaneous emission lines between 300 and 1700 nm.

| $SLJ$ | $E_{SLJ}(cm^{-1})$ | $S'L'J'$ | $\lambda$ (nm) | $A'_{eq}$ $(s^{-1})$ [a] | $SLJ$ | $E_{SLJ}(cm^{-1})$ | $S'L'J'$ | $\lambda$ (nm) | $A'_{eq}$ $(s^{-1})$ [a] |
|---|---|---|---|---|---|---|---|---|---|
| $(^1H, ^3H)_5$ | 37739 | $^3D_3$ | 830 | $8.03 \times 10^{-4}$ | $^3H_4$ | 36389 | $^5G_5$ | 689 | $1.18 \times 10^{-4}$ |
| | | $^3G_5$ | 933 | $4.36 \times 10^{-5}$ | | | $^5G_6$ | 704 | $8.32 \times 10^{-5}$ |
| | | $^3F_4$ | 935 | $1.14 \times 10^{-4}$ | | | $^3D_2$ | 750 | $8.15 \times 10^{-4}$ |
| | | $^3I_5$ | 1049 | $1.15 \times 10^{-5}$ | | | $^3H_6$ | 808 | $9.06 \times 10^{-6}$ |
| | | $^3F_3$ | 1160 | $5.5 \times 10^{-6}$ | | | $^3G_4$ | 841 | $2.93 \times 10^{-5}$ |
| | | $^3I_6$ | 1189 | $7.16 \times 10^{-5}$ | | | $^3D_3$ | 935 | $3.21 \times 10^{-5}$ |
| | | $^3I_7$ | 1265 | $1.57 \times 10^{-6}$ | | | $(^1D, ^3F)_2$ | 982 | $3.53 \times 10^{-4}$ |
| | | $^5D_3$ | 1690 | $2.09 \times 10^{-6}$ | | | $^3G_5$ | 1068 | $4.14 \times 10^{-5}$ |
| $^3H_5$ | 36501 | $^5I_7$ | 315 | $6.8 \times 10^{-6}$ | | | $^3F_4$ | 1070 | $4.41 \times 10^{-6}$ |
| | | $^5F_3$ | 434 | $2.64 \times 10^{-4}$ | | | $^3I_5$ | 1222 | $9.8 \times 10^{-5}$ |
| | | $^5F_4$ | 453 | $4.65 \times 10^{-6}$ | | | $(^3F, ^3P)_2$ | 1281 | $4.22 \times 10^{-5}$ |
| | | $^5F_5$ | 483 | $2.8 \times 10^{-5}$ | | | $^3F_3$ | 1376 | $4.69 \times 10^{-6}$ |
| | | $^3K_6$ | 487 | $6.84 \times 10^{-6}$ | | | $^3I_6$ | 1416 | $9.3 \times 10^{-7}$ |
| | | $^3K_7$ | 521 | $4.83 \times 10^{-4}$ | | | $^3F_2$ | 1480 | $7.52 \times 10^{-6}$ |
| | | $(^3H, ^5G)_4$ | 523 | $8.44 \times 10^{-5}$ | $^3H_6$ | 36252 | $^5I_6$ | 301 | $1.52 \times 10^{-5}$ |
| | | $^5G_3$ | 537 | $2.62 \times 10^{-4}$ | | | $^5I_7$ | 317 | $6.7 \times 10^{-4}$ |
| | | $(^3H, ^5G)_5$ | 592 | $5.93 \times 10^{-4}$ | | | $^5I_8$ | 336 | $1.58 \times 10^{-4}$ |
| | | $^5G_4$ | 607 | $2.66 \times 10^{-4}$ | | | $^5F_4$ | 458 | $5.36 \times 10^{-4}$ |
| | | $^3G_3$ | 675 | $3.6 \times 10^{-5}$ | | | $^5F_5$ | 489 | $3.59 \times 10^{-6}$ |
| | | $^5G_5$ | 684 | $3.98 \times 10^{-4}$ | | | $^3K_6$ | 493 | $6.07 \times 10^{-6}$ |
| | | $^5G_6$ | 698 | $4.95 \times 10^{-7}$ | | | $^3K_7$ | 528 | $7.15 \times 10^{-6}$ |
| | | $^3L_7$ | 772 | $6.98 \times 10^{-5}$ | | | $(^3H, ^5G)_4$ | 530 | $5.4 \times 10^{-4}$ |
| | | $^3H_6$ | 801 | $6.96 \times 10^{-7}$ | | | $^3K_8$ | 572 | $6.95 \times 10^{-4}$ |
| | | $^3G_4$ | 833 | $3.82 \times 10^{-5}$ | | | $(^3H, ^5G)_5$ | 601 | $6.11 \times 10^{-5}$ |
| | | $^3D_3$ | 925 | $3.24 \times 10^{-5}$ | | | $^5G_4$ | 617 | $2.79 \times 10^{-5}$ |
| | | $^3G_5$ | 1055 | $1.27 \times 10^{-5}$ | | | $^5G_5$ | 696 | $9.26 \times 10^{-5}$ |
| | | $^3F_4$ | 1058 | $7.47 \times 10^{-6}$ | | | $^5G_6$ | 711 | $9.69 \times 10^{-5}$ |
| | | $^3I_5$ | 1206 | $1.3 \times 10^{-6}$ | | | $^3L_7$ | 787 | $1.2 \times 10^{-6}$ |
| | | $^3F_3$ | 1355 | $8.06 \times 10^{-5}$ | | | $^3H_6$ | 817 | $2.92 \times 10^{-4}$ |
| | | $^3I_6$ | 1394 | $3.69 \times 10^{-5}$ | | | $(^3L, ^3M)_8$ | 840 | $8.76 \times 10^{-9}$ |
| | | $^3I_7$ | 1500 | $3.99 \times 10^{-8}$ | | | $^3G_4$ | 851 | $3.81 \times 10^{-5}$ |
| $^3H_4$ | 36389 | $^5F_2$ | 421 | $1.31 \times 10^{-4}$ | | | $^3G_5$ | 1083 | $3.39 \times 10^{-5}$ |
| | | $^5F_3$ | 436 | $9.21 \times 10^{-5}$ | | | $^3F_4$ | 1086 | $2.62 \times 10^{-4}$ |
| | | $^5S_2$ | 449 | $3.3 \times 10^{-4}$ | | | $(^3M, ^3L)_8$ | 1105 | $2.58 \times 10^{-5}$ |
| | | $^5F_4$ | 455 | $1.84 \times 10^{-4}$ | | | $^3I_5$ | 1243 | $1.7 \times 10^{-5}$ |
| | | $^5F_5$ | 486 | $5.24 \times 10^{-5}$ | | | $^3I_6$ | 1444 | $1.65 \times 10^{-8}$ |
| | | $^3K_6$ | 490 | $3.1 \times 10^{-4}$ | | | $^3I_7$ | 1558 | $3.4 \times 10^{-5}$ |
| | | $(^3H, ^5G)_4$ | 526 | $4.44 \times 10^{-3}$ | $^3F_4$ | 36249 | $^5I_6$ | 301 | $3.5 \times 10^{-4}$ |
| | | $^5G_2$ | 532 | $4.5 \times 10^{-4}$ | | | $^5F_2$ | 423 | $2.12 \times 10^{-4}$ |
| | | $^5G_3$ | 541 | $2.12 \times 10^{-5}$ | | | $^5F_3$ | 439 | $2.04 \times 10^{-4}$ |
| | | $(^3H, ^5G)_5$ | 596 | $1.69 \times 10^{-4}$ | | | $^5S_2$ | 452 | $8.29 \times 10^{-3}$ |
| | | $^5G_4$ | 612 | $7.68 \times 10^{-4}$ | | | $^5F_4$ | 458 | $1.8 \times 10^{-3}$ |
| | | $^3G_3$ | 680 | $8.99 \times 10^{-5}$ | | | $^5F_5$ | 489 | $2.44 \times 10^{-3}$ |

[a] The emission rate, $A_{eq}$, inside a host material with refractive index $n_r$ would be: $A_{eq} = A'_{eq}\ n_r^5$

TABLE S17: Continued: $Pm^{3+}$ EQ spontaneous emission lines between 300 and 1700 nm.

| $SLJ$ | $E_{SLJ}(cm^{-1})$ | $S'L'J'$ | $\lambda$ (nm) | $A'_{eq}$ $(s^{-1})$ [a] | $SLJ$ | $E_{SLJ}(cm^{-1})$ | $S'L'J'$ | $\lambda$ (nm) | $A'_{eq}$ $(s^{-1})$ [a] |
|---|---|---|---|---|---|---|---|---|---|
| $^3F_4$ | 36249 | $^3K_6$ | 493 | $1.44\times10^{-6}$ | $^1G_4$ | 33415 | $^5F_4$ | 527 | $8.04\times10^{-4}$ |
| | | $(^3H,\,^5G)_4$ | 530 | $5.87\times10^{-7}$ | | | $^5F_5$ | 567 | $7.83\times10^{-4}$ |
| | | $^5G_2$ | 536 | $9.54\times10^{-9}$ | | | $^3K_6$ | 573 | $2.56\times10^{-5}$ |
| | | $^5G_3$ | 545 | $3.67\times10^{-5}$ | | | $(^3H,\,^5G)_4$ | 623 | $6.53\times10^{-5}$ |
| | | $(^3H,\,^5G)_5$ | 601 | $1.59\times10^{-5}$ | | | $^5G_2$ | 632 | $1.53\times10^{-5}$ |
| | | $^5G_4$ | 617 | $9.68\times10^{-5}$ | | | $^5G_3$ | 644 | $1.83\times10^{-5}$ |
| | | $^3G_3$ | 687 | $2.11\times10^{-7}$ | | | $(^3H,\,^5G)_5$ | 724 | $8.72\times10^{-7}$ |
| | | $^5G_5$ | 696 | $1.81\times10^{-4}$ | | | $^5G_4$ | 748 | $2.07\times10^{-6}$ |
| | | $^5G_6$ | 711 | $1.77\times10^{-4}$ | | | $^3G_3$ | 853 | $4.77\times10^{-6}$ |
| | | $^3D_2$ | 758 | $2.58\times10^{-5}$ | | | $^5G_5$ | 867 | $3.6\times10^{-5}$ |
| | | $^3H_6$ | 817 | $1.62\times10^{-3}$ | | | $^5G_6$ | 890 | $9.17\times10^{-5}$ |
| | | $^3G_4$ | 851 | $2.29\times10^{-5}$ | | | $^3D_2$ | 966 | $2.33\times10^{-5}$ |
| | | $^3D_3$ | 947 | $2.58\times10^{-4}$ | | | $^3H_6$ | 1063 | $1.57\times10^{-5}$ |
| | | $(^1D,\,^3F)_2$ | 996 | $7.21\times10^{-6}$ | | | $^3G_4$ | 1122 | $5.7\times10^{-6}$ |
| | | $^3G_5$ | 1084 | $2.13\times10^{-4}$ | | | $^3D_3$ | 1295 | $4.2\times10^{-8}$ |
| | | $^3F_4$ | 1087 | $2.02\times10^{-5}$ | | | $(^1D,\,^3F)_2$ | 1388 | $4.65\times10^{-6}$ |
| | | $^3I_5$ | 1243 | $7.29\times10^{-6}$ | | | $^3G_5$ | 1564 | $9.59\times10^{-6}$ |
| | | $(^3F,\,^3P)_2$ | 1304 | $2.04\times10^{-5}$ | | | $^3F_4$ | 1570 | $1.37\times10^{-5}$ |
| | | $^3F_3$ | 1403 | $3.47\times10^{-7}$ | $^3F_3$ | 32958 | $^5I_4$ | 303 | $4.18\times10^{-4}$ |
| | | $^3I_6$ | 1445 | $8.49\times10^{-7}$ | | | $^5I_5$ | 317 | $9.29\times10^{-4}$ |
| | | $^3F_2$ | 1511 | $2.4\times10^{-6}$ | | | $^5F_1$ | 483 | $6.63\times10^{-7}$ |
| $^1D_2$ | 33653 | $^5F_1$ | 468 | $2.32\times10^{-4}$ | | | $^5F_2$ | 492 | $1.22\times10^{-3}$ |
| | | $^5F_2$ | 476 | $1.58\times10^{-6}$ | | | $^5F_3$ | 513 | $2.94\times10^{-3}$ |
| | | $^5F_3$ | 495 | $1.55\times10^{-5}$ | | | $^5S_2$ | 531 | $5.07\times10^{-3}$ |
| | | $^5S_2$ | 512 | $8.06\times10^{-5}$ | | | $^5F_4$ | 540 | $1.02\times10^{-3}$ |
| | | $^5F_4$ | 520 | $2.04\times10^{-5}$ | | | $^5F_5$ | 583 | $6.38\times10^{-4}$ |
| | | $(^3H,\,^5G)_4$ | 614 | $5.18\times10^{-6}$ | | | $(^3H,\,^5G)_4$ | 642 | $1.27\times10^{-5}$ |
| | | $^5G_2$ | 623 | $2.79\times10^{-5}$ | | | $^5G_2$ | 651 | $9.63\times10^{-5}$ |
| | | $^5G_3$ | 635 | $5.77\times10^{-5}$ | | | $^5G_3$ | 664 | $2.89\times10^{-4}$ |
| | | $^5G_4$ | 734 | $2.07\times10^{-6}$ | | | $(^3H,\,^5G)_5$ | 749 | $3.07\times10^{-4}$ |
| | | $^3G_3$ | 836 | $5.83\times10^{-5}$ | | | $^5G_4$ | 774 | $3.89\times10^{-4}$ |
| | | $^3D_2$ | 944 | $6.83\times10^{-7}$ | | | $^3G_3$ | 887 | $5.11\times10^{-6}$ |
| | | $(^3P,\,^3D)_1$ | 1037 | $2.92\times10^{-6}$ | | | $^5G_5$ | 903 | $8.86\times10^{-4}$ |
| | | $^3G_4$ | 1092 | $3.62\times10^{-5}$ | | | $^3D_2$ | 1010 | $6.68\times10^{-5}$ |
| | | $^3P_0$ | 1236 | $2.78\times10^{-4}$ | | | $(^3P,\,^3D)_1$ | 1117 | $2.61\times10^{-6}$ |
| | | $^3D_3$ | 1257 | $2.06\times10^{-6}$ | | | $^3G_4$ | 1182 | $8.98\times10^{-5}$ |
| | | $(^1D,\,^3F)_2$ | 1344 | $2.25\times10^{-7}$ | | | $^3D_3$ | 1377 | $1.39\times10^{-5}$ |
| | | $^3F_4$ | 1513 | $4.51\times10^{-6}$ | | | $(^1D,\,^3F)_2$ | 1482 | $1.73\times10^{-6}$ |
| $^1G_4$ | 33415 | $^5I_5$ | 313 | $7.82\times10^{-5}$ | | | $^3G_5$ | 1685 | $5.36\times10^{-7}$ |
| | | $^5I_6$ | 329 | $9.68\times10^{-8}$ | | | $^3F_4$ | 1691 | $2.31\times10^{-6}$ |
| | | $^5F_2$ | 481 | $6.\times10^{-6}$ | $^5D_4$ | 32302 | $^5I_4$ | 310 | $5.43\times10^{-6}$ |
| | | $^5F_3$ | 501 | $3.72\times10^{-4}$ | | | $^5I_5$ | 324 | $2.52\times10^{-6}$ |
| | | $^5S_2$ | 518 | $4.63\times10^{-3}$ | | | $^5I_6$ | 341 | $1.59\times10^{-5}$ |

[a] The emission rate, $A_{eq}$, inside a host material with refractive index $n_r$ would be: $A_{eq} = A'_{eq}\ n_r^5$

TABLE S17: Continued: $Pm^{3+}$ EQ spontaneous emission lines between 300 and 1700 nm.

| $SLJ$ | $E_{SLJ}(cm^{-1})$ | $S'L'J'$ | $\lambda$ (nm) | $A'_{eq}$ $(s^{-1})$ [a] | $SLJ$ | $E_{SLJ}(cm^{-1})$ | $S'L'J'$ | $\lambda$ (nm) | $A'_{eq}$ $(s^{-1})$ [a] |
|---|---|---|---|---|---|---|---|---|---|
| $^5D_4$ | 32302 | $^5F_2$ | 508 | $3.9 \times 10^{-5}$ | $^1L_8$ | 31124 | $^3K_8$ | 809 | $3.72 \times 10^{-6}$ |
| | | $^5F_3$ | 531 | $3.54 \times 10^{-3}$ | | | $^5G_6$ | 1118 | $1.87 \times 10^{-8}$ |
| | | $^5S_2$ | 550 | $5.2 \times 10^{-2}$ | | | $^3L_7$ | 1321 | $2.49 \times 10^{-5}$ |
| | | $^5F_4$ | 560 | $8.69 \times 10^{-3}$ | | | $^3H_6$ | 1406 | $1.4 \times 10^{-7}$ |
| | | $^5F_5$ | 606 | $9.48 \times 10^{-3}$ | | | $(^3L, ^3M)_8$ | 1474 | $1.68 \times 10^{-5}$ |
| | | $^3K_6$ | 612 | $1.03 \times 10^{-6}$ | $^5D_2$ | 31078 | $^5I_4$ | 322 | $8.2 \times 10^{-5}$ |
| | | $(^3H, ^5G)_4$ | 670 | $2.83 \times 10^{-6}$ | | | $^5F_1$ | 532 | $1.88 \times 10^{-2}$ |
| | | $^5G_2$ | 680 | $2.33 \times 10^{-6}$ | | | $^5F_2$ | 542 | $1.05 \times 10^{-2}$ |
| | | $^5G_3$ | 694 | $4.73 \times 10^{-5}$ | | | $^5F_3$ | 568 | $6.43 \times 10^{-4}$ |
| | | $(^3H, ^5G)_5$ | 788 | $8.2 \times 10^{-5}$ | | | $^5S_2$ | 590 | $1.49 \times 10^{-2}$ |
| | | $^5G_4$ | 815 | $1.31 \times 10^{-4}$ | | | $^5F_4$ | 601 | $2.66 \times 10^{-3}$ |
| | | $^3G_3$ | 942 | $1.6 \times 10^{-5}$ | | | $(^3H, ^5G)_4$ | 730 | $6.12 \times 10^{-4}$ |
| | | $^5G_5$ | 960 | $1.87 \times 10^{-4}$ | | | $^5G_2$ | 741 | $1.2 \times 10^{-3}$ |
| | | $^5G_6$ | 988 | $8.4 \times 10^{-4}$ | | | $^5G_3$ | 759 | $1.5 \times 10^{-3}$ |
| | | $^3D_2$ | 1082 | $7.43 \times 10^{-6}$ | | | $^5G_4$ | 906 | $7.75 \times 10^{-4}$ |
| | | $^3H_6$ | 1206 | $8.35 \times 10^{-5}$ | | | $^3G_3$ | 1065 | $1.2 \times 10^{-4}$ |
| | | $^3G_4$ | 1281 | $2.54 \times 10^{-6}$ | | | $^3D_2$ | 1247 | $2.92 \times 10^{-9}$ |
| | | $^3D_3$ | 1513 | $1.92 \times 10^{-5}$ | | | $(^3P, ^3D)_1$ | 1414 | $9.25 \times 10^{-6}$ |
| | | $(^1D, ^3F)_2$ | 1641 | $1.17 \times 10^{-6}$ | | | $^3G_4$ | 1520 | $2.05 \times 10^{-6}$ |
| $^5D_3$ | 31821 | $^5I_4$ | 314 | $1.49 \times 10^{-5}$ | $^5D_1$ | 30248 | $^5F_1$ | 556 | $1.58 \times 10^{-2}$ |
| | | $^5I_5$ | 329 | $6.88 \times 10^{-5}$ | | | $^5F_2$ | 567 | $1.17 \times 10^{-6}$ |
| | | $^5F_1$ | 512 | $3.26 \times 10^{-3}$ | | | $^5F_3$ | 596 | $3.05 \times 10^{-3}$ |
| | | $^5F_2$ | 521 | $1.26 \times 10^{-2}$ | | | $^5S_2$ | 620 | $4.07 \times 10^{-3}$ |
| | | $^5F_3$ | 545 | $1.1 \times 10^{-2}$ | | | $^5G_2$ | 790 | $1.62 \times 10^{-3}$ |
| | | $^5S_2$ | 565 | $2.43 \times 10^{-2}$ | | | $^5G_3$ | 810 | $7.95 \times 10^{-4}$ |
| | | $^5F_4$ | 575 | $3.65 \times 10^{-3}$ | | | $^3G_3$ | 1168 | $3.07 \times 10^{-5}$ |
| | | $^5F_5$ | 624 | $1.09 \times 10^{-3}$ | | | $^3D_2$ | 1391 | $2.11 \times 10^{-6}$ |
| | | $(^3H, ^5G)_4$ | 692 | $1.33 \times 10^{-4}$ | | | $(^3P, ^3D)_1$ | 1603 | $4.6 \times 10^{-7}$ |
| | | $^5G_2$ | 703 | $2.88 \times 10^{-4}$ | $^3M_{10}$ | 30010 | $^5I_8$ | 426 | $3.86 \times 10^{-6}$ |
| | | $^5G_3$ | 718 | $4.14 \times 10^{-4}$ | | | $^3K_8$ | 890 | $7.81 \times 10^{-7}$ |
| | | $(^3H, ^5G)_5$ | 819 | $1.43 \times 10^{-3}$ | $^3I_7$ | 29834 | $^5I_5$ | 352 | $4.53 \times 10^{-5}$ |
| | | $^5G_4$ | 849 | $5.59 \times 10^{-4}$ | | | $^5I_6$ | 373 | $2.17 \times 10^{-4}$ |
| | | $^3G_3$ | 987 | $1.33 \times 10^{-4}$ | | | $^5I_7$ | 399 | $2.8 \times 10^{-4}$ |
| | | $^5G_5$ | 1006 | $2.41 \times 10^{-4}$ | | | $^5I_8$ | 429 | $1.04 \times 10^{-3}$ |
| | | $^3D_2$ | 1141 | $1.85 \times 10^{-4}$ | | | $^5F_5$ | 712 | $6.81 \times 10^{-5}$ |
| | | $(^3P, ^3D)_1$ | 1280 | $9.1 \times 10^{-6}$ | | | $^3K_6$ | 721 | $1.21 \times 10^{-6}$ |
| | | $^3G_4$ | 1366 | $8.01 \times 10^{-5}$ | | | $^3K_7$ | 798 | $5.08 \times 10^{-5}$ |
| | | $^3D_3$ | 1632 | $1.9 \times 10^{-6}$ | | | $^3K_8$ | 904 | $5.32 \times 10^{-4}$ |
| $^1L_8$ | 31124 | $^5I_6$ | 356 | $1.8 \times 10^{-4}$ | | | $(^3H, ^5G)_5$ | 978 | $5.9 \times 10^{-5}$ |
| | | $^5I_7$ | 379 | $6.5 \times 10^{-7}$ | | | $^5G_5$ | 1258 | $6.38 \times 10^{-6}$ |
| | | $^5I_8$ | 406 | $2.54 \times 10^{-7}$ | | | $^5G_6$ | 1307 | $2.5 \times 10^{-5}$ |
| | | $^3K_6$ | 660 | $1.07 \times 10^{-4}$ | | | $^3L_7$ | 1592 | $1.33 \times 10^{-7}$ |
| | | $^3K_7$ | 724 | $6. \times 10^{-5}$ | $^5D_0$ | 29716 | $^5F_2$ | 585 | $1.61 \times 10^{-3}$ |

[a] The emission rate, $A_{eq}$, inside a host material with refractive index $n_r$ would be: $A_{eq} = A'_{eq}\ n_r^5$

TABLE S17: Continued: $Pm^{3+}$ EQ spontaneous emission lines between 300 and 1700 nm.

| $SLJ$ | $E_{SLJ}(cm^{-1})$ | $S'L'J'$ | $\lambda$ (nm) | $A'_{eq}$ $(s^{-1})$ [a] | $SLJ$ | $E_{SLJ}(cm^{-1})$ | $S'L'J'$ | $\lambda$ (nm) | $A'_{eq}$ $(s^{-1})$ [a] |
|---|---|---|---|---|---|---|---|---|---|
| $^5D_0$ | 29716 | $^5S_2$ | 641 | $3.28 \times 10^{-4}$ | $^3F_3$ | 29121 | $^5G_2$ | 867 | $3.43 \times 10^{-5}$ |
| | | $^5G_2$ | 825 | $3.14 \times 10^{-4}$ | | | $^5G_3$ | 891 | $9.66 \times 10^{-5}$ |
| | | $^3D_2$ | 1502 | $2.97 \times 10^{-11}$ | | | $(^3H,\, ^5G)\, _5$ | 1051 | $2.38 \times 10^{-5}$ |
| $^3F_2$ | 29631 | $^5I_4$ | 337 | $1.56 \times 10^{-3}$ | | | $^5G_4$ | 1101 | $5.89 \times 10^{-7}$ |
| | | $^5F_1$ | 576 | $1.43 \times 10^{-3}$ | | | $^3G_3$ | 1345 | $1.38 \times 10^{-5}$ |
| | | $^5F_2$ | 588 | $4.13 \times 10^{-5}$ | | | $^5G_5$ | 1382 | $4.46 \times 10^{-7}$ |
| | | $^5F_3$ | 619 | $3.9 \times 10^{-6}$ | | | $^3D_2$ | 1649 | $9.39 \times 10^{-6}$ |
| | | $^5S_2$ | 645 | $2.13 \times 10^{-4}$ | $(^3F,\, ^3P)\, _2$ | 28583 | $^5I_4$ | 350 | $7.54 \times 10^{-5}$ |
| | | $^5F_4$ | 658 | $1.98 \times 10^{-6}$ | | | $^5F_1$ | 613 | $9.53 \times 10^{-4}$ |
| | | $(^3H,\, ^5G)\, _4$ | 816 | $1.01 \times 10^{-3}$ | | | $^5F_2$ | 627 | $1.34 \times 10^{-4}$ |
| | | $^5G_2$ | 831 | $3.36 \times 10^{-6}$ | | | $^5F_3$ | 661 | $7.28 \times 10^{-5}$ |
| | | $^5G_3$ | 852 | $2.69 \times 10^{-6}$ | | | $^5S_2$ | 691 | $3.57 \times 10^{-4}$ |
| | | $^5G_4$ | 1042 | $8.92 \times 10^{-5}$ | | | $^5F_4$ | 707 | $1.05 \times 10^{-4}$ |
| | | $^3G_3$ | 1259 | $8.42 \times 10^{-5}$ | | | $(^3H,\, ^5G)\, _4$ | 892 | $2.55 \times 10^{-5}$ |
| | | $^3D_2$ | 1522 | $2.36 \times 10^{-5}$ | | | $^5G_2$ | 910 | $6.27 \times 10^{-5}$ |
| $^3M_9$ | 29401 | $^5I_7$ | 406 | $6.42 \times 10^{-7}$ | | | $^5G_3$ | 936 | $1.25 \times 10^{-4}$ |
| | | $^5I_8$ | 437 | $8.1 \times 10^{-5}$ | | | $^5G_4$ | 1170 | $4.07 \times 10^{-6}$ |
| | | $^3K_7$ | 827 | $1.34 \times 10^{-5}$ | | | $^3G_3$ | 1450 | $3.03 \times 10^{-5}$ |
| | | $^3K_8$ | 941 | $3.73 \times 10^{-6}$ | $^3I_5$ | 28207 | $^5I_4$ | 355 | $1.95 \times 10^{-3}$ |
| $^3I_6$ | 29326 | $^5I_4$ | 341 | $2.28 \times 10^{-4}$ | | | $^5I_5$ | 374 | $3.07 \times 10^{-4}$ |
| | | $^5I_5$ | 359 | $6.97 \times 10^{-4}$ | | | $^5I_6$ | 397 | $4.51 \times 10^{-4}$ |
| | | $^5I_6$ | 380 | $3.44 \times 10^{-4}$ | | | $^5I_7$ | 426 | $1.45 \times 10^{-4}$ |
| | | $^5I_7$ | 407 | $7.2 \times 10^{-4}$ | | | $^5F_3$ | 678 | $4.89 \times 10^{-5}$ |
| | | $^5I_8$ | 438 | $2.15 \times 10^{-5}$ | | | $^5F_4$ | 726 | $3.73 \times 10^{-5}$ |
| | | $^5F_4$ | 671 | $1.5 \times 10^{-4}$ | | | $^5F_5$ | 806 | $9.43 \times 10^{-8}$ |
| | | $^5F_5$ | 739 | $1.26 \times 10^{-5}$ | | | $^3K_6$ | 817 | $9.02 \times 10^{-4}$ |
| | | $^3K_6$ | 749 | $9.14 \times 10^{-5}$ | | | $^3K_7$ | 918 | $3.95 \times 10^{-5}$ |
| | | $^3K_7$ | 832 | $8.26 \times 10^{-4}$ | | | $(^3H,\, ^5G)\, _4$ | 923 | $2.17 \times 10^{-4}$ |
| | | $(^3H,\, ^5G)\, _4$ | 837 | $2.83 \times 10^{-4}$ | | | $^5G_3$ | 970 | $6.28 \times 10^{-5}$ |
| | | $^3K_8$ | 947 | $4.24 \times 10^{-5}$ | | | $(^3H,\, ^5G)\, _5$ | 1163 | $8.5 \times 10^{-9}$ |
| | | $(^3H,\, ^5G)\, _5$ | 1029 | $1.12 \times 10^{-4}$ | | | $^5G_4$ | 1224 | $4.95 \times 10^{-5}$ |
| | | $^5G_4$ | 1077 | $6.18 \times 10^{-6}$ | | | $^3G_3$ | 1534 | $4.12 \times 10^{-5}$ |
| | | $^5G_5$ | 1344 | $4.62 \times 10^{-5}$ | | | $^5G_5$ | 1582 | $3.71 \times 10^{-8}$ |
| | | $^5G_6$ | 1400 | $8.03 \times 10^{-8}$ | | | $^5G_6$ | 1660 | $3.34 \times 10^{-8}$ |
| $^3F_3$ | 29121 | $^5I_4$ | 343 | $1.9 \times 10^{-5}$ | $(^3P,\, ^3D)\, _1$ | 27821 | $^5F_1$ | 643 | $1.85 \times 10^{-4}$ |
| | | $^5I_5$ | 362 | $8.07 \times 10^{-5}$ | | | $^5F_2$ | 658 | $1.59 \times 10^{-6}$ |
| | | $^5F_1$ | 594 | $2.37 \times 10^{-4}$ | | | $^5F_3$ | 697 | $6.19 \times 10^{-5}$ |
| | | $^5F_2$ | 606 | $5.11 \times 10^{-4}$ | | | $^5S_2$ | 730 | $3.83 \times 10^{-5}$ |
| | | $^5F_3$ | 639 | $1.81 \times 10^{-4}$ | | | $^5G_2$ | 977 | $1.81 \times 10^{-5}$ |
| | | $^5S_2$ | 667 | $7.08 \times 10^{-4}$ | | | $^5G_3$ | 1008 | $1.48 \times 10^{-5}$ |
| | | $^5F_4$ | 681 | $1.89 \times 10^{-4}$ | | | $^3G_3$ | 1630 | $2.59 \times 10^{-6}$ |
| | | $^5F_5$ | 750 | $4.45 \times 10^{-5}$ | $(^3M,\, ^3L)\, _8$ | 27199 | $^5I_6$ | 413 | $5.72 \times 10^{-5}$ |
| | | $(^3H,\, ^5G)\, _4$ | 851 | $1.23 \times 10^{-4}$ | | | $^5I_7$ | 445 | $8.13 \times 10^{-5}$ |

[a] The emission rate, $A_{eq}$, inside a host material with refractive index $n_r$ would be: $A_{eq} = A'_{eq}\ n_r^5$

TABLE S17: Continued: $Pm^{3+}$ EQ spontaneous emission lines between 300 and 1700 nm.

| $SLJ$ | $E_{SLJ}(cm^{-1})$ | $S'L'J'$ | $\lambda$ (nm) | $A'_{eq}$ $(s^{-1})$ [a] | $SLJ$ | $E_{SLJ}(cm^{-1})$ | $S'L'J'$ | $\lambda$ (nm) | $A'_{eq}$ $(s^{-1})$ [a] |
|---|---|---|---|---|---|---|---|---|---|
| $\left(^3M,\, ^3L\right)_8$ | 27199 | $^5I_8$ | 483 | $8.73 \times 10^{-7}$ | $^3L_9$ | 25711 | $^3K_7$ | 1190 | $2.78 \times 10^{-7}$ |
| | | $^3K_6$ | 890 | $1.61 \times 10^{-5}$ | | | $^3K_8$ | 1441 | $4.02 \times 10^{-5}$ |
| | | $^3K_7$ | 1011 | $8.71 \times 10^{-6}$ | $^3D_3$ | 25695 | $^5I_4$ | 389 | $5.65 \times 10^{-5}$ |
| | | $^3K_8$ | 1186 | $6.51 \times 10^{-7}$ | | | $^5I_5$ | 413 | $1.48 \times 10^{-4}$ |
| $^3F_4$ | 27046 | $^5I_4$ | 370 | $1.32 \times 10^{-7}$ | | | $^5F_1$ | 745 | $1.38 \times 10^{-4}$ |
| | | $^5I_5$ | 391 | $1.5 \times 10^{-5}$ | | | $^5F_2$ | 765 | $2.34 \times 10^{-4}$ |
| | | $^5I_6$ | 416 | $7.1 \times 10^{-6}$ | | | $^5F_3$ | 818 | $9.56 \times 10^{-5}$ |
| | | $^5F_2$ | 694 | $1.94 \times 10^{-5}$ | | | $^5S_2$ | 864 | $1.71 \times 10^{-4}$ |
| | | $^5F_3$ | 736 | $1.53 \times 10^{-4}$ | | | $^5F_4$ | 888 | $1.22 \times 10^{-4}$ |
| | | $^5S_2$ | 774 | $1.67 \times 10^{-3}$ | | | $^5F_5$ | 1010 | $5.76 \times 10^{-8}$ |
| | | $^5F_4$ | 793 | $2.04 \times 10^{-4}$ | | | $\left(^3H,\, ^5G\right)_4$ | 1202 | $1.17 \times 10^{-5}$ |
| | | $^5F_5$ | 889 | $2.32 \times 10^{-4}$ | | | $^5G_2$ | 1234 | $3.53 \times 10^{-6}$ |
| | | $^3K_6$ | 903 | $1.68 \times 10^{-8}$ | | | $^5G_3$ | 1282 | $9.5 \times 10^{-6}$ |
| | | $\left(^3H,\, ^5G\right)_4$ | 1034 | $1.9 \times 10^{-5}$ | | | $\left(^3H,\, ^5G\right)_5$ | 1643 | $1.29 \times 10^{-5}$ |
| | | $^5G_2$ | 1058 | $1.89 \times 10^{-6}$ | $^3P_0$ | 25560 | $^5F_2$ | 773 | $1.75 \times 10^{-6}$ |
| | | $^5G_3$ | 1093 | $9.33 \times 10^{-6}$ | | | $^5S_2$ | 874 | $4.73 \times 10^{-9}$ |
| | | $\left(^3H,\, ^5G\right)_5$ | 1345 | $1.01 \times 10^{-5}$ | | | $^5G_2$ | 1255 | $6.25 \times 10^{-8}$ |
| | | $^5G_4$ | 1427 | $1.49 \times 10^{-6}$ | $^3G_4$ | 24499 | $^5I_4$ | 408 | $1.86 \times 10^{-4}$ |
| $^3G_5$ | 27022 | $^5I_4$ | 370 | $5.82 \times 10^{-5}$ | | | $^5I_5$ | 434 | $1.23 \times 10^{-3}$ |
| | | $^5I_5$ | 391 | $8.79 \times 10^{-5}$ | | | $^5I_6$ | 465 | $5.66 \times 10^{-3}$ |
| | | $^5I_6$ | 416 | $5.21 \times 10^{-4}$ | | | $^5F_2$ | 842 | $3.04 \times 10^{-4}$ |
| | | $^5I_7$ | 449 | $4.04 \times 10^{-3}$ | | | $^5F_3$ | 906 | $2.24 \times 10^{-4}$ |
| | | $^5F_3$ | 738 | $2.04 \times 10^{-4}$ | | | $^5S_2$ | 964 | $5.27 \times 10^{-5}$ |
| | | $^5F_4$ | 794 | $2.26 \times 10^{-4}$ | | | $^5F_4$ | 993 | $1.04 \times 10^{-5}$ |
| | | $^5F_5$ | 891 | $2.74 \times 10^{-6}$ | | | $^5F_5$ | 1149 | $8.98 \times 10^{-6}$ |
| | | $^3K_6$ | 905 | $1.19 \times 10^{-5}$ | | | $^3K_6$ | 1172 | $9.23 \times 10^{-7}$ |
| | | $^3K_7$ | 1029 | $1.43 \times 10^{-7}$ | | | $\left(^3H,\, ^5G\right)_4$ | 1404 | $4.22 \times 10^{-6}$ |
| | | $\left(^3H,\, ^5G\right)_4$ | 1037 | $9.51 \times 10^{-6}$ | | | $^5G_2$ | 1447 | $1.32 \times 10^{-7}$ |
| | | $^5G_3$ | 1096 | $2.83 \times 10^{-7}$ | | | $^5G_3$ | 1514 | $2.3 \times 10^{-6}$ |
| | | $\left(^3H,\, ^5G\right)_5$ | 1349 | $2.43 \times 10^{-7}$ | $\left(^3L,\, ^3M\right)_8$ | 24341 | $^5I_6$ | 469 | $2.26 \times 10^{-5}$ |
| | | $^5G_4$ | 1432 | $4.88 \times 10^{-7}$ | | | $^5I_7$ | 510 | $1.12 \times 10^{-4}$ |
| $\left(^1D,\, ^3F\right)_2$ | 26210 | $^5I_4$ | 382 | $2.95 \times 10^{-5}$ | | | $^5I_8$ | 561 | $1.73 \times 10^{-6}$ |
| | | $^5F_1$ | 718 | $6.82 \times 10^{-5}$ | | | $^3K_6$ | 1194 | $1.18 \times 10^{-6}$ |
| | | $^5F_2$ | 736 | $8.43 \times 10^{-7}$ | | | $^3K_7$ | 1422 | $4.19 \times 10^{-5}$ |
| | | $^5F_3$ | 785 | $5.71 \times 10^{-6}$ | $^3H_6$ | 24011 | $^5I_4$ | 416 | $1.48 \times 10^{-6}$ |
| | | $^5S_2$ | 827 | $8.51 \times 10^{-6}$ | | | $^5I_5$ | 443 | $1.56 \times 10^{-5}$ |
| | | $^5F_4$ | 849 | $7.93 \times 10^{-8}$ | | | $^5I_6$ | 476 | $6.02 \times 10^{-5}$ |
| | | $\left(^3H,\, ^5G\right)_4$ | 1132 | $1.74 \times 10^{-7}$ | | | $^5I_7$ | 519 | $1.2 \times 10^{-3}$ |
| | | $^5G_2$ | 1160 | $3.22 \times 10^{-6}$ | | | $^5I_8$ | 572 | $5.69 \times 10^{-3}$ |
| | | $^5G_3$ | 1203 | $5.55 \times 10^{-6}$ | | | $^5F_4$ | 1044 | $8.56 \times 10^{-5}$ |
| | | $^5G_4$ | 1620 | $2.36 \times 10^{-7}$ | | | $^5F_5$ | 1217 | $2.23 \times 10^{-4}$ |
| $^3L_9$ | 25711 | $^5I_7$ | 477 | $1.03 \times 10^{-5}$ | | | $^3K_6$ | 1243 | $5.75 \times 10^{-8}$ |
| | | $^5I_8$ | 521 | $3.11 \times 10^{-4}$ | | | $^3K_7$ | 1492 | $7.54 \times 10^{-7}$ |

[a] The emission rate, $A_{eq}$, inside a host material with refractive index $n_r$ would be: $A_{eq} = A'_{eq}\ n_r^5$

TABLE S17: Continued: $Pm^{3+}$ EQ spontaneous emission lines between 300 and 1700 nm.

| $SLJ$ | $E_{SLJ}(cm^{-1})$ | $S'L'J'$ | $\lambda$ (nm) | $A'_{eq}$ $(s^{-1})$ [a] | $SLJ$ | $E_{SLJ}(cm^{-1})$ | $S'L'J'$ | $\lambda$ (nm) | $A'_{eq}$ $(s^{-1})$ [a] |
|---|---|---|---|---|---|---|---|---|---|
| $^3H_6$ | 24011 | $\left(^3H,\,^5G\right)_4$ | 1507 | $2.7\times10^{-6}$ | | | $^5F_4$ | 1378 | $4.09\times10^{-6}$ |
| $\left(^3P,\,^3D\right)_1$ | 24008 | $^5F_1$ | 852 | $5.42\times10^{-6}$ | | | $^5F_5$ | 1696 | $3.81\times10^{-8}$ |
| | | $^5F_2$ | 879 | $6.67\times10^{-6}$ | $^5G_4$ | 20038 | $^5I_4$ | 499 | $4.67\times10^{-4}$ |
| | | $^5F_3$ | 949 | $2.42\times10^{-7}$ | | | $^5I_5$ | 538 | $4.9\times10^{-3}$ |
| | | $^5S_2$ | 1012 | $6.64\times10^{-7}$ | | | $^5I_6$ | 587 | $9.76\times10^{-3}$ |
| | | $^5G_2$ | 1558 | $2.47\times10^{-6}$ | $^3G_3$ | 21688 | $^5F_2$ | 1349 | $2.68\times10^{-4}$ |
| | | $^5G_3$ | 1636 | $1.29\times10^{-6}$ | | | $^5F_3$ | 1522 | $8.61\times10^{-5}$ |
| $^3L_7$ | 23553 | $^5I_5$ | 453 | $4.25\times10^{-5}$ | | | $^5S_2$ | 1690 | $1.77\times10^{-7}$ |
| | | $^5I_6$ | 487 | $9.52\times10^{-5}$ | $\left(^3H,\,^5G\right)_5$ | 19610 | $^5I_4$ | 510 | $9.73\times10^{-6}$ |
| | | $^5I_7$ | 532 | $2.54\times10^{-7}$ | | | $^5I_5$ | 551 | $4.06\times10^{-4}$ |
| | | $^5I_8$ | 587 | $7.73\times10^{-8}$ | | | $^5I_6$ | 602 | $1.53\times10^{-3}$ |
| | | $^5F_5$ | 1289 | $1.66\times10^{-10}$ | | | $^5I_7$ | 673 | $3.61\times10^{-3}$ |
| | | $^3K_6$ | 1318 | $8.68\times10^{-5}$ | | | $^5F_3$ | 1628 | $6.76\times10^{-5}$ |
| | | $^3K_7$ | 1601 | $9.14\times10^{-6}$ | $^3K_8$ | 18769 | $^5I_6$ | 634 | $5.79\times10^{-6}$ |
| $^3D_2$ | 23059 | $^5I_4$ | 434 | $1.72\times10^{-4}$ | | | $^5I_7$ | 713 | $4.33\times10^{-6}$ |
| | | $^5F_1$ | 927 | $4.49\times10^{-5}$ | | | $^5I_8$ | 816 | $5.92\times10^{-5}$ |
| | | $^5F_2$ | 959 | $6.32\times10^{-6}$ | $^5G_3$ | 17896 | $^5I_4$ | 559 | $4.44\times10^{-3}$ |
| | | $^5F_3$ | 1042 | $1.76\times10^{-5}$ | | | $^5I_5$ | 608 | $8.83\times10^{-3}$ |
| | | $^5S_2$ | 1119 | $3.73\times10^{-6}$ | $^5G_2$ | 17590 | $^5I_4$ | 569 | $1.41\times10^{-2}$ |
| | | $^5F_4$ | 1159 | $1.86\times10^{-7}$ | $\left(^3H,\,^5G\right)_4$ | 17376 | $^5I_4$ | 575 | $2.85\times10^{-4}$ |
| $^5G_6$ | 22183 | $^5I_4$ | 451 | $3.55\times10^{-10}$ | | | $^5I_5$ | 628 | $8.71\times10^{-4}$ |
| | | $^5I_5$ | 483 | $1.16\times10^{-5}$ | | | $^5I_6$ | 696 | $1.57\times10^{-3}$ |
| | | $^5I_6$ | 521 | $3.72\times10^{-4}$ | $^3K_7$ | 17308 | $^5I_5$ | 631 | $1.85\times10^{-5}$ |
| | | $^5I_7$ | 574 | $2.23\times10^{-3}$ | | | $^5I_6$ | 699 | $1.18\times10^{-6}$ |
| | | $^5I_8$ | 638 | $1.04\times10^{-2}$ | | | $^5I_7$ | 796 | $3.19\times10^{-5}$ |
| | | $^5F_4$ | 1290 | $1.74\times10^{-4}$ | | | $^5I_8$ | 927 | $3.29\times10^{-8}$ |
| | | $^5F_5$ | 1565 | $2.22\times10^{-4}$ | $^3K_6$ | 15967 | $^5I_4$ | 626 | $6.68\times10^{-5}$ |
| | | $^3K_6$ | 1609 | $5.09\times10^{-11}$ | | | $^5I_5$ | 689 | $1.27\times10^{-7}$ |
| $^5G_5$ | 21885 | $^5I_4$ | 457 | $3.43\times10^{-5}$ | | | $^5I_6$ | 771 | $1.15\times10^{-5}$ |
| | | $^5I_5$ | 490 | $3.93\times10^{-4}$ | | | $^5I_7$ | 892 | $6.19\times10^{-8}$ |
| | | $^5I_6$ | 530 | $3.89\times10^{-3}$ | | | $^5I_8$ | 1058 | $5.39\times10^{-9}$ |
| | | $^5I_7$ | 584 | $9.59\times10^{-3}$ | $^5F_5$ | 15793 | $^5I_4$ | 633 | $1.26\times10^{-7}$ |
| | | $^5F_3$ | 1188 | $2.53\times10^{-4}$ | | | $^5I_5$ | 698 | $5.43\times10^{-6}$ |
| | | $^5F_4$ | 1342 | $1.91\times10^{-4}$ | | | $^5I_6$ | 782 | $1.75\times10^{-5}$ |
| | | $^5F_5$ | 1641 | $1.98\times10^{-5}$ | | | $^5I_7$ | 906 | $2.3\times10^{-5}$ |
| | | $^3K_6$ | 1690 | $2.71\times10^{-7}$ | $^5F_4$ | 14432 | $^5I_4$ | 693 | $6.78\times10^{-6}$ |
| $^3G_3$ | 21688 | $^5I_4$ | 461 | $1.23\times10^{-3}$ | | | $^5I_5$ | 771 | $1.63\times10^{-5}$ |
| | | $^5I_5$ | 494 | $6.64\times10^{-3}$ | | | $^5I_6$ | 875 | $1.41\times10^{-5}$ |
| | | $^5F_1$ | 1062 | $2.86\times10^{-4}$ | $^5S_2$ | 14122 | $^5I_4$ | 708 | $4.12\times10^{-8}$ |
| | | $^5F_2$ | 1104 | $1.13\times10^{-4}$ | $^5F_3$ | 13466 | $^5I_4$ | 743 | $4.43\times10^{-7}$ |
| | | $^5F_3$ | 1216 | $3.93\times10^{-5}$ | | | $^5I_5$ | 833 | $4.16\times10^{-7}$ |
| | | $^5S_2$ | 1322 | $2.34\times10^{-8}$ | $^5F_2$ | 12626 | $^5I_4$ | 792 | $1.22\times10^{-5}$ |

[a] The emission rate, $A_{eq}$, inside a host material with refractive index $n_r$ would be: $A_{eq} = A'_{eq}\ n_r^5$

TABLE S18: Calculated $Sm^{3+}$ EQ spontaneous emission lines between 300 and 1700 nm.

| $SLJ$ | $E_{SLJ}(cm^{-1})$ | $S'L'J'$ | $\lambda$ (nm) | $A'_{eq}$ $(s^{-1})$ [a] | $SLJ$ | $E_{SLJ}(cm^{-1})$ | $S'L'J'$ | $\lambda$ (nm) | $A'_{eq}$ $(s^{-1})$ [a] |
|---|---|---|---|---|---|---|---|---|---|
| $^2H_{11/2}$ | 39247 | $^6H_{15/2}$ | 305 | $3.94 \times 10^{-6}$ | $^2G_{7/2}$ | 39072 | $^6P_{3/2}$ | 696 | $1.95 \times 10^{-5}$ |
| | | $^6F_{7/2}$ | 318 | $4.91 \times 10^{-4}$ | | | $^4F_{7/2}$ | 705 | $2.99 \times 10^{-6}$ |
| | | $^6F_{9/2}$ | 330 | $8.35 \times 10^{-5}$ | | | $^4K_{11/2}$ | 706 | $1.84 \times 10^{-4}$ |
| | | $^6F_{11/2}$ | 347 | $1.4 \times 10^{-5}$ | | | $^4G_{11/2}$ | 744 | $6.1 \times 10^{-8}$ |
| | | $^4G_{7/2}$ | 524 | $7.32 \times 10^{-4}$ | | | $^6P_{7/2}$ | 792 | $2.05 \times 10^{-6}$ |
| | | $^4I_{11/2}$ | 551 | $5.6 \times 10^{-5}$ | | | $^4D_{3/2}$ | 857 | $2.22 \times 10^{-5}$ |
| | | $^4M_{15/2}$ | 554 | $1.54 \times 10^{-4}$ | | | $^4F_{9/2}$ | 858 | $1.46 \times 10^{-8}$ |
| | | $\left(^4K,\, ^4I\right)_{13/2}$ | 561 | $3.72 \times 10^{-4}$ | | | $\left(^4D,\, ^6P\right)_{5/2}$ | 862 | $6.79 \times 10^{-6}$ |
| | | $^4I_{9/2}$ | 562 | $4.41 \times 10^{-6}$ | | | $^4H_{7/2}$ | 966 | $1.66 \times 10^{-4}$ |
| | | $^4G_{9/2}$ | 606 | $2.81 \times 10^{-5}$ | | | $^4D_{7/2}$ | 975 | $3.24 \times 10^{-7}$ |
| | | $\left(^4I,\, ^4K\right)_{15/2}$ | 618 | $3.55 \times 10^{-4}$ | | | $^4H_{9/2}$ | 1021 | $7.51 \times 10^{-6}$ |
| | | $^4L_{13/2}$ | 695 | $5.69 \times 10^{-7}$ | | | $^4H_{11/2}$ | 1068 | $2.31 \times 10^{-6}$ |
| | | $^4F_{7/2}$ | 696 | $6.79 \times 10^{-6}$ | | | $^4G_{7/2}$ | 1101 | $1.1 \times 10^{-5}$ |
| | | $^4K_{11/2}$ | 697 | $2.11 \times 10^{-4}$ | | | $^4G_{5/2}$ | 1112 | $3.44 \times 10^{-5}$ |
| | | $\left(^4L,\, ^4I\right)_{15/2}$ | 705 | $3.62 \times 10^{-4}$ | | | $^4G_{9/2}$ | 1116 | $6.99 \times 10^{-6}$ |
| | | $^4G_{11/2}$ | 734 | $2.34 \times 10^{-4}$ | | | $^4P_{3/2}$ | 1293 | $8.77 \times 10^{-7}$ |
| | | $^4K_{13/2}$ | 777 | $1.05 \times 10^{-4}$ | | | $^4G_{11/2}$ | 1296 | $6.16 \times 10^{-7}$ |
| | | $^6P_{7/2}$ | 781 | $9.76 \times 10^{-7}$ | | | $^4P_{5/2}$ | 1541 | $3.23 \times 10^{-7}$ |
| | | $^4F_{9/2}$ | 846 | $2.11 \times 10^{-6}$ | $^2F_{7/2}$ | 38706 | $^6F_{3/2}$ | 310 | $1.72 \times 10^{-4}$ |
| | | $^4K_{15/2}$ | 884 | $1.53 \times 10^{-5}$ | | | $^6F_{5/2}$ | 314 | $1.58 \times 10^{-4}$ |
| | | $^4H_{7/2}$ | 950 | $2.36 \times 10^{-6}$ | | | $^6F_{7/2}$ | 323 | $1.74 \times 10^{-5}$ |
| | | $^4D_{7/2}$ | 958 | $1.76 \times 10^{-6}$ | | | $^6F_{9/2}$ | 336 | $1.42 \times 10^{-5}$ |
| | | $^4H_{9/2}$ | 1003 | $3.92 \times 10^{-6}$ | | | $^6F_{11/2}$ | 353 | $2.41 \times 10^{-5}$ |
| | | $^4H_{11/2}$ | 1049 | $7.76 \times 10^{-7}$ | | | $^4G_{5/2}$ | 486 | $4.03 \times 10^{-5}$ |
| | | $^4G_{7/2}$ | 1081 | $1.75 \times 10^{-5}$ | | | $^4F_{3/2}$ | 505 | $5.9 \times 10^{-7}$ |
| | | $^4G_{9/2}$ | 1094 | $2.35 \times 10^{-5}$ | | | $^4G_{7/2}$ | 540 | $3.14 \times 10^{-6}$ |
| | | $^4H_{13/2}$ | 1100 | $1.05 \times 10^{-5}$ | | | $^4I_{11/2}$ | 568 | $1.43 \times 10^{-5}$ |
| | | $^4G_{11/2}$ | 1268 | $2.62 \times 10^{-6}$ | | | $^4I_{9/2}$ | 580 | $3.57 \times 10^{-8}$ |
| | | $\left(^2K,\, ^2L\right)_{15/2}$ | 1452 | $2.15 \times 10^{-5}$ | | | $^4F_{5/2}$ | 605 | $1.22 \times 10^{-4}$ |
| | | $^2K_{13/2}$ | 1642 | $3.96 \times 10^{-9}$ | | | $^4G_{9/2}$ | 626 | $5.48 \times 10^{-6}$ |
| $^2G_{7/2}$ | 39072 | $^6F_{3/2}$ | 306 | $1.25 \times 10^{-5}$ | | | $\left(^6P,\, ^4P\right)_{5/2}$ | 673 | $5.44 \times 10^{-6}$ |
| | | $^6F_{5/2}$ | 311 | $1.41 \times 10^{-4}$ | | | $^6P_{3/2}$ | 714 | $3.62 \times 10^{-6}$ |
| | | $^6F_{7/2}$ | 319 | $9.51 \times 10^{-6}$ | | | $^4F_{7/2}$ | 724 | $3.25 \times 10^{-5}$ |
| | | $^6F_{9/2}$ | 332 | $4.77 \times 10^{-6}$ | | | $^4K_{11/2}$ | 725 | $2.07 \times 10^{-5}$ |
| | | $^6F_{11/2}$ | 349 | $4.07 \times 10^{-6}$ | | | $^4G_{11/2}$ | 765 | $2.2 \times 10^{-6}$ |
| | | $^4G_{5/2}$ | 477 | $4.1 \times 10^{-7}$ | | | $^6P_{7/2}$ | 815 | $1.34 \times 10^{-5}$ |
| | | $^4F_{3/2}$ | 496 | $6.7 \times 10^{-4}$ | | | $^4D_{3/2}$ | 885 | $2.99 \times 10^{-6}$ |
| | | $^4G_{7/2}$ | 529 | $6.44 \times 10^{-4}$ | | | $^4F_{9/2}$ | 886 | $5.12 \times 10^{-6}$ |
| | | $^4I_{11/2}$ | 557 | $6.89 \times 10^{-4}$ | | | $\left(^4D,\, ^6P\right)_{5/2}$ | 890 | $4.81 \times 10^{-6}$ |
| | | $^4I_{9/2}$ | 568 | $2.69 \times 10^{-5}$ | | | $^4H_{7/2}$ | 1001 | $9.01 \times 10^{-6}$ |
| | | $^4F_{5/2}$ | 592 | $1.66 \times 10^{-4}$ | | | $^4D_{7/2}$ | 1011 | $1.28 \times 10^{-5}$ |
| | | $^4G_{9/2}$ | 612 | $4.89 \times 10^{-6}$ | | | $^4H_{9/2}$ | 1061 | $3.11 \times 10^{-8}$ |
| | | $\left(^6P,\, ^4P\right)_{5/2}$ | 657 | $4.11 \times 10^{-5}$ | | | $^4H_{11/2}$ | 1112 | $4.38 \times 10^{-7}$ |

[a] The emission rate, $A_{eq}$, inside a host material with refractive index $n_r$ would be: $A_{eq} = A'_{eq}\ n_r^5$

TABLE S18: Continued: $Sm^{3+}$ EQ spontaneous emission lines between 300 and 1700 nm.

| $SLJ$ | $E_{SLJ}(cm^{-1})$ | $S'L'J'$ | $\lambda$ (nm) | $A'_{eq}$ $(s^{-1})$ [a] | $SLJ$ | $E_{SLJ}(cm^{-1})$ | $S'L'J'$ | $\lambda$ (nm) | $A'_{eq}$ $(s^{-1})$ [a] |
|---|---|---|---|---|---|---|---|---|---|
| $^2F_{7/2}$ | 38706 | $^4G_{7/2}$ | 1148 | $3.2 \times 10^{-7}$ | $(^2H,\,^4I)_{9/2}$ | 37737 | $^6H_{13/2}$ | 306 | $4.23 \times 10^{-5}$ |
| | | $^4G_{5/2}$ | 1159 | $1.17 \times 10^{-6}$ | | | $^6F_{5/2}$ | 324 | $5.35 \times 10^{-4}$ |
| | | $^4G_{9/2}$ | 1163 | $2.25 \times 10^{-6}$ | | | $^6F_{7/2}$ | 334 | $3.54 \times 10^{-4}$ |
| | | $^4P_{3/2}$ | 1358 | $4.36 \times 10^{-6}$ | | | $^6F_{9/2}$ | 348 | $2.35 \times 10^{-5}$ |
| | | $^4G_{11/2}$ | 1361 | $3.01 \times 10^{-8}$ | | | $^6F_{11/2}$ | 366 | $2.58 \times 10^{-6}$ |
| | | $^4P_{5/2}$ | 1633 | $2.05 \times 10^{-7}$ | | | $^4G_{5/2}$ | 510 | $3.02 \times 10^{-3}$ |
| $^2M_{17/2}$ | 38464 | $^6H_{15/2}$ | 312 | $4.86 \times 10^{-8}$ | | | $^4G_{7/2}$ | 569 | $9.29 \times 10^{-6}$ |
| | | $^4M_{15/2}$ | 579 | $8.92 \times 10^{-6}$ | | | $^4I_{11/2}$ | 601 | $1.37 \times 10^{-3}$ |
| | | $(^4K,\,^4I)_{13/2}$ | 586 | $2.97 \times 10^{-5}$ | | | $(^4K,\,^4I)_{13/2}$ | 612 | $3.43 \times 10^{-4}$ |
| | | $^4M_{17/2}$ | 627 | $4.85 \times 10^{-5}$ | | | $^4I_{9/2}$ | 614 | $7.22 \times 10^{-5}$ |
| | | $(^4I,\,^4K)_{15/2}$ | 650 | $3.33 \times 10^{-6}$ | | | $^4F_{5/2}$ | 643 | $1.43 \times 10^{-4}$ |
| | | $^4M_{19/2}$ | 694 | $1.78 \times 10^{-5}$ | | | $^4G_{9/2}$ | 667 | $1.93 \times 10^{-4}$ |
| | | $^4L_{13/2}$ | 735 | $1.02 \times 10^{-5}$ | | | $(^6P,\,^4P)_{5/2}$ | 720 | $2.2 \times 10^{-5}$ |
| | | $(^4L,\,^4I)_{15/2}$ | 747 | $2.49 \times 10^{-5}$ | | | $^4L_{13/2}$ | 777 | $1.67 \times 10^{-4}$ |
| | | $^4M_{21/2}$ | 771 | $4.29 \times 10^{-6}$ | | | $^4F_{7/2}$ | 778 | $2.84 \times 10^{-5}$ |
| | | $^4L_{17/2}$ | 798 | $3.04 \times 10^{-6}$ | | | $^4K_{11/2}$ | 779 | $3.53 \times 10^{-4}$ |
| | | $^4K_{13/2}$ | 827 | $8.68 \times 10^{-5}$ | | | $^4G_{11/2}$ | 826 | $7.09 \times 10^{-6}$ |
| | | $^4K_{15/2}$ | 950 | $4.76 \times 10^{-5}$ | | | $^4K_{13/2}$ | 880 | $7.92 \times 10^{-8}$ |
| | | $^4K_{17/2}$ | 972 | $4.36 \times 10^{-7}$ | | | $^6P_{7/2}$ | 885 | $1.46 \times 10^{-6}$ |
| | | $^4L_{19/2}$ | 1083 | $8.32 \times 10^{-8}$ | | | $^4F_{9/2}$ | 969 | $1.12 \times 10^{-6}$ |
| | | $^4H_{13/2}$ | 1204 | $1.77 \times 10^{-8}$ | | | $(^4D,\,^6P)_{5/2}$ | 974 | $1.59 \times 10^{-7}$ |
| | | $(^2K,\,^2L)_{15/2}$ | 1639 | $8.77 \times 10^{-7}$ | | | $^4H_{7/2}$ | 1108 | $1.1 \times 10^{-5}$ |
| $(^2P,\,^2D)_{3/2}$ | 38395 | $^6F_{1/2}$ | 311 | $6.95 \times 10^{-4}$ | | | $^4D_{7/2}$ | 1121 | $1.85 \times 10^{-6}$ |
| | | $^6F_{3/2}$ | 313 | $8.1 \times 10^{-4}$ | | | $^4H_{9/2}$ | 1183 | $1.88 \times 10^{-6}$ |
| | | $^6F_{5/2}$ | 317 | $1.54 \times 10^{-4}$ | | | $^4H_{11/2}$ | 1246 | $3.7 \times 10^{-6}$ |
| | | $^6F_{7/2}$ | 326 | $5.34 \times 10^{-5}$ | | | $^4G_{7/2}$ | 1291 | $1.13 \times 10^{-5}$ |
| | | $^4G_{5/2}$ | 493 | $2.9 \times 10^{-4}$ | | | $^4G_{5/2}$ | 1306 | $1.65 \times 10^{-5}$ |
| | | $^4F_{3/2}$ | 513 | $1.8 \times 10^{-4}$ | | | $^4G_{9/2}$ | 1311 | $1.01 \times 10^{-5}$ |
| | | $^4G_{7/2}$ | 549 | $8.83 \times 10^{-5}$ | | | $^4H_{13/2}$ | 1320 | $8.5 \times 10^{-8}$ |
| | | $^4F_{5/2}$ | 617 | $1.08 \times 10^{-4}$ | | | $^4G_{11/2}$ | 1568 | $5.21 \times 10^{-8}$ |
| | | $(^6P,\,^4P)_{5/2}$ | 688 | $1.61 \times 10^{-5}$ | $^2L_{17/2}$ | 37165 | $^6H_{13/2}$ | 312 | $4.62 \times 10^{-5}$ |
| | | $^6P_{3/2}$ | 730 | $2.69 \times 10^{-6}$ | | | $^6H_{15/2}$ | 326 | $2.37 \times 10^{-5}$ |
| | | $^4F_{7/2}$ | 740 | $2. \times 10^{-5}$ | | | $^4M_{15/2}$ | 626 | $3.35 \times 10^{-5}$ |
| | | $^4D_{1/2}$ | 825 | $9.29 \times 10^{-5}$ | | | $(^4K,\,^4I)_{13/2}$ | 635 | $1.26 \times 10^{-5}$ |
| | | $^6P_{7/2}$ | 837 | $1.51 \times 10^{-5}$ | | | $^4M_{17/2}$ | 683 | $8.95 \times 10^{-7}$ |
| | | $^4D_{3/2}$ | 910 | $5.08 \times 10^{-7}$ | | | $(^4I,\,^4K)_{15/2}$ | 710 | $4.9 \times 10^{-5}$ |
| | | $(^4D,\,^6P)_{5/2}$ | 915 | $1.61 \times 10^{-6}$ | | | $^4M_{19/2}$ | 763 | $3.39 \times 10^{-4}$ |
| | | $^4H_{7/2}$ | 1033 | $1.08 \times 10^{-7}$ | | | $^4L_{13/2}$ | 813 | $4.34 \times 10^{-6}$ |
| | | $^4D_{7/2}$ | 1044 | $2.12 \times 10^{-5}$ | | | $(^4L,\,^4I)_{15/2}$ | 827 | $2.14 \times 10^{-5}$ |
| | | $^4G_{7/2}$ | 1190 | $9.32 \times 10^{-8}$ | | | $^4M_{21/2}$ | 856 | $9.85 \times 10^{-7}$ |
| | | $^4G_{5/2}$ | 1203 | $1.07 \times 10^{-6}$ | | | $^4L_{17/2}$ | 890 | $6.21 \times 10^{-6}$ |
| | | $^4P_{1/2}$ | 1347 | $4.7 \times 10^{-8}$ | | | $^4K_{13/2}$ | 927 | $2.32 \times 10^{-6}$ |
| | | $^4P_{3/2}$ | 1418 | $4.11 \times 10^{-6}$ | | | $^4K_{15/2}$ | 1084 | $4.13 \times 10^{-5}$ |

[a] The emission rate, $A_{eq}$, inside a host material with refractive index $n_r$ would be: $A_{eq} = A'_{eq}\ n_r^5$

TABLE S18: Continued: $Sm^{3+}$ EQ spontaneous emission lines between 300 and 1700 nm.

| $SLJ$ | $E_{SLJ}(cm^{-1})$ | $S'L'J'$ | $\lambda$ (nm) | $A'_{eq}$ $(s^{-1})$ [a] | $SLJ$ | $E_{SLJ}(cm^{-1})$ | $S'L'J'$ | $\lambda$ (nm) | $A'_{eq}$ $(s^{-1})$ [a] |
|---|---|---|---|---|---|---|---|---|---|
| $^2L_{17/2}$ | 37165 | $^4K_{17/2}$ | 1112 | $1.63 \times 10^{-5}$ | $^4F_{5/2}$ | 36255 | $^6P_{7/2}$ | 1019 | $2.33 \times 10^{-6}$ |
| | | $^4L_{19/2}$ | 1260 | $1.64 \times 10^{-5}$ | | | $^4D_{3/2}$ | 1130 | $2.14 \times 10^{-5}$ |
| | | $^4H_{13/2}$ | 1427 | $7.57 \times 10^{-9}$ | | | $^4F_{9/2}$ | 1132 | $1.84 \times 10^{-8}$ |
| $^2N_{21/2}$ | 36867 | $^4M_{17/2}$ | 697 | $2.19 \times 10^{-5}$ | | | $\left(^4D,\, ^6P\right)_{5/2}$ | 1138 | $4.13 \times 10^{-5}$ |
| | | $^4M_{19/2}$ | 781 | $2.81 \times 10^{-5}$ | | | $^4H_{7/2}$ | 1326 | $7.76 \times 10^{-7}$ |
| | | $^4M_{21/2}$ | 879 | $2.25 \times 10^{-5}$ | | | $^4D_{7/2}$ | 1344 | $9.17 \times 10^{-7}$ |
| | | $^4L_{17/2}$ | 914 | $1.25 \times 10^{-5}$ | | | $^4H_{9/2}$ | 1434 | $1.09 \times 10^{-7}$ |
| | | $^4K_{17/2}$ | 1150 | $1.23 \times 10^{-5}$ | | | $^4G_{7/2}$ | 1597 | $2.74 \times 10^{-6}$ |
| | | $^4L_{19/2}$ | 1309 | $1.51 \times 10^{-6}$ | | | $^4G_{5/2}$ | 1619 | $1.99 \times 10^{-6}$ |
| $^4F_{3/2}$ | 36466 | $^6F_{1/2}$ | 331 | $3.5 \times 10^{-3}$ | | | $^4G_{9/2}$ | 1627 | $1.27 \times 10^{-10}$ |
| | | $^6F_{3/2}$ | 333 | $3.52 \times 10^{-4}$ | $^4I_{13/2}$ | 36214 | $^6H_{11/2}$ | 307 | $6.9 \times 10^{-6}$ |
| | | $^6F_{5/2}$ | 338 | $1.36 \times 10^{-4}$ | | | $^6H_{13/2}$ | 321 | $2.17 \times 10^{-4}$ |
| | | $^6F_{7/2}$ | 348 | $2.41 \times 10^{-5}$ | | | $^6H_{15/2}$ | 336 | $1.8 \times 10^{-5}$ |
| | | $^4G_{5/2}$ | 545 | $2.48 \times 10^{-5}$ | | | $^6F_{9/2}$ | 367 | $1.1 \times 10^{-5}$ |
| | | $^4F_{3/2}$ | 570 | $7.39 \times 10^{-5}$ | | | $^6F_{11/2}$ | 387 | $4.89 \times 10^{-8}$ |
| | | $^4G_{7/2}$ | 614 | $7.69 \times 10^{-6}$ | | | $^4I_{11/2}$ | 662 | $2.9 \times 10^{-6}$ |
| | | $^4F_{5/2}$ | 700 | $3.16 \times 10^{-5}$ | | | $^4M_{15/2}$ | 665 | $4.72 \times 10^{-4}$ |
| | | $\left(^6P,\, ^4P\right)_{5/2}$ | 793 | $1.42 \times 10^{-5}$ | | | $\left(^4K,\, ^4I\right)_{13/2}$ | 675 | $9.93 \times 10^{-6}$ |
| | | $^6P_{3/2}$ | 850 | $1.7 \times 10^{-7}$ | | | $^4I_{9/2}$ | 678 | $3.15 \times 10^{-6}$ |
| | | $^4F_{7/2}$ | 864 | $2.15 \times 10^{-7}$ | | | $^4M_{17/2}$ | 730 | $2.06 \times 10^{-4}$ |
| | | $^4D_{1/2}$ | 981 | $3.02 \times 10^{-4}$ | | | $^4G_{9/2}$ | 742 | $2.78 \times 10^{-4}$ |
| | | $^6P_{7/2}$ | 998 | $3.62 \times 10^{-7}$ | | | $\left(^4I,\, ^4K\right)_{15/2}$ | 761 | $5.48 \times 10^{-4}$ |
| | | $^4D_{3/2}$ | 1103 | $5.38 \times 10^{-5}$ | | | $^4L_{13/2}$ | 881 | $1.43 \times 10^{-4}$ |
| | | $\left(^4D,\, ^6P\right)_{5/2}$ | 1112 | $7.34 \times 10^{-6}$ | | | $^4K_{11/2}$ | 884 | $1.25 \times 10^{-5}$ |
| | | $^4H_{7/2}$ | 1290 | $5.12 \times 10^{-10}$ | | | $\left(^4L,\, ^4I\right)_{15/2}$ | 897 | $1.63 \times 10^{-4}$ |
| | | $^4D_{7/2}$ | 1307 | $6.62 \times 10^{-7}$ | | | $^4G_{11/2}$ | 945 | $6.84 \times 10^{-6}$ |
| | | $^4G_{7/2}$ | 1545 | $2.16 \times 10^{-7}$ | | | $^4L_{17/2}$ | 972 | $6.66 \times 10^{-5}$ |
| | | $^4G_{5/2}$ | 1566 | $3.01 \times 10^{-6}$ | | | $^4K_{13/2}$ | 1016 | $1.08 \times 10^{-4}$ |
| $^4F_{5/2}$ | 36255 | $^6F_{1/2}$ | 333 | $4.32 \times 10^{-3}$ | | | $^4F_{9/2}$ | 1137 | $2.59 \times 10^{-5}$ |
| | | $^6F_{3/2}$ | 335 | $6.33 \times 10^{-4}$ | | | $^4K_{15/2}$ | 1208 | $8.42 \times 10^{-5}$ |
| | | $^6F_{5/2}$ | 340 | $5.91 \times 10^{-4}$ | | | $^4K_{17/2}$ | 1244 | $7.4 \times 10^{-5}$ |
| | | $^6F_{7/2}$ | 351 | $1.92 \times 10^{-8}$ | | | $^4H_{9/2}$ | 1442 | $4.35 \times 10^{-7}$ |
| | | $^6F_{9/2}$ | 366 | $1.23 \times 10^{-5}$ | | | $^4H_{11/2}$ | 1538 | $5.3 \times 10^{-6}$ |
| | | $^4G_{5/2}$ | 551 | $2.49 \times 10^{-5}$ | | | $^4G_{9/2}$ | 1638 | $1.07 \times 10^{-7}$ |
| | | $^4F_{3/2}$ | 577 | $1.69 \times 10^{-4}$ | | | $^4H_{13/2}$ | 1651 | $3.83 \times 10^{-6}$ |
| | | $^4G_{7/2}$ | 622 | $4.89 \times 10^{-5}$ | $^2N_{19/2}$ | 35983 | $^6H_{15/2}$ | 339 | $6.12 \times 10^{-6}$ |
| | | $^4I_{9/2}$ | 676 | $7.9 \times 10^{-6}$ | | | $^4M_{15/2}$ | 676 | $1.13 \times 10^{-6}$ |
| | | $^4F_{5/2}$ | 710 | $8.68 \times 10^{-7}$ | | | $^4M_{17/2}$ | 743 | $7.51 \times 10^{-5}$ |
| | | $^4G_{9/2}$ | 740 | $3.4 \times 10^{-7}$ | | | $\left(^4I,\, ^4K\right)_{15/2}$ | 775 | $4.57 \times 10^{-7}$ |
| | | $\left(^6P,\, ^4P\right)_{5/2}$ | 806 | $3.85 \times 10^{-5}$ | | | $^4M_{19/2}$ | 839 | $4.47 \times 10^{-6}$ |
| | | $^6P_{3/2}$ | 865 | $2.38 \times 10^{-5}$ | | | $\left(^4L,\, ^4I\right)_{15/2}$ | 916 | $2.36 \times 10^{-5}$ |
| | | $^4F_{7/2}$ | 880 | $3.77 \times 10^{-6}$ | | | $^4M_{21/2}$ | 953 | $2.85 \times 10^{-6}$ |
| | | $^4D_{1/2}$ | 1001 | $4.11 \times 10^{-4}$ | | | $^4L_{17/2}$ | 995 | $1.13 \times 10^{-6}$ |

[a] The emission rate, $A_{eq}$, inside a host material with refractive index $n_r$ would be: $A_{eq} = A'_{eq}\ n_r^5$

TABLE S18: Continued: $Sm^{3+}$ EQ spontaneous emission lines between 300 and 1700 nm.

| $SLJ$ | $E_{SLJ}(cm^{-1})$ | $S'L'J'$ | $\lambda$ (nm) | $A'_{eq}$ $(s^{-1})$ [a] | $SLJ$ | $E_{SLJ}(cm^{-1})$ | $S'L'J'$ | $\lambda$ (nm) | $A'_{eq}$ $(s^{-1})$ [a] |
|---|---|---|---|---|---|---|---|---|---|
| $^2N_{19/2}$ | 35983 | $^4K_{15/2}$ | 1243 | $5.94 \times 10^{-8}$ | $^4F_{7/2}$ | 35538 | $^4I_{9/2}$ | 710 | $1.18 \times 10^{-5}$ |
| | | $^4K_{17/2}$ | 1280 | $4.45 \times 10^{-6}$ | | | $^4F_{5/2}$ | 748 | $6.51 \times 10^{-5}$ |
| | | $^4L_{19/2}$ | 1481 | $5.23 \times 10^{-7}$ | | | $^4G_{9/2}$ | 782 | $4.37 \times 10^{-5}$ |
| $^4I_{15/2}$ | 35853 | $^6H_{11/2}$ | 310 | $2.8 \times 10^{-6}$ | | | $(^6P,\, ^4P)\, _{5/2}$ | 856 | $6.57 \times 10^{-6}$ |
| | | $^6H_{13/2}$ | 325 | $2.26 \times 10^{-5}$ | | | $^6P_{3/2}$ | 922 | $2.08 \times 10^{-4}$ |
| | | $^6H_{15/2}$ | 340 | $3.29 \times 10^{-4}$ | | | $^4F_{7/2}$ | 939 | $5.2 \times 10^{-7}$ |
| | | $^6F_{11/2}$ | 393 | $1.41 \times 10^{-5}$ | | | $^4K_{11/2}$ | 940 | $1.73 \times 10^{-6}$ |
| | | $^4I_{11/2}$ | 678 | $4.78 \times 10^{-6}$ | | | $^4G_{11/2}$ | 1009 | $2.72 \times 10^{-9}$ |
| | | $^4M_{15/2}$ | 682 | $8.78 \times 10^{-6}$ | | | $^6P_{7/2}$ | 1099 | $1.4 \times 10^{-5}$ |
| | | $(^4K,\, ^4I)\, _{13/2}$ | 692 | $5.48 \times 10^{-6}$ | | | $^4D_{3/2}$ | 1229 | $1.21 \times 10^{-4}$ |
| | | $^4M_{17/2}$ | 750 | $1.93 \times 10^{-4}$ | | | $^4F_{9/2}$ | 1232 | $1.15 \times 10^{-6}$ |
| | | $(^4I,\, ^4K)\, _{15/2}$ | 782 | $2.06 \times 10^{-5}$ | | | $(^4D,\, ^6P)\, _{5/2}$ | 1239 | $1.38 \times 10^{-5}$ |
| | | $^4M_{19/2}$ | 848 | $1.43 \times 10^{-4}$ | | | $^4H_{7/2}$ | 1466 | $1.02 \times 10^{-7}$ |
| | | $^4L_{13/2}$ | 910 | $5.03 \times 10^{-7}$ | | | $^4D_{7/2}$ | 1487 | $7.73 \times 10^{-6}$ |
| | | $^4K_{11/2}$ | 913 | $2.41 \times 10^{-6}$ | | | $^4H_{9/2}$ | 1598 | $2.85 \times 10^{-8}$ |
| | | $(^4L,\, ^4I)\, _{15/2}$ | 927 | $1.41 \times 10^{-4}$ | $^4I_{11/2}$ | 35523 | $^6H_{9/2}$ | 301 | $1.7 \times 10^{-8}$ |
| | | $^4G_{11/2}$ | 978 | $1.34 \times 10^{-4}$ | | | $^6H_{11/2}$ | 313 | $2.14 \times 10^{-4}$ |
| | | $^4L_{17/2}$ | 1008 | $2.76 \times 10^{-4}$ | | | $^6H_{13/2}$ | 328 | $2.19 \times 10^{-10}$ |
| | | $^4K_{13/2}$ | 1055 | $9.02 \times 10^{-7}$ | | | $^6H_{15/2}$ | 344 | $3.02 \times 10^{-7}$ |
| | | $^4K_{15/2}$ | 1263 | $2.46 \times 10^{-5}$ | | | $^6F_{7/2}$ | 360 | $4.31 \times 10^{-6}$ |
| | | $^4K_{17/2}$ | 1302 | $9.52 \times 10^{-5}$ | | | $^6F_{9/2}$ | 377 | $5.61 \times 10^{-7}$ |
| | | $^4L_{19/2}$ | 1510 | $3. \times 10^{-5}$ | | | $^6F_{11/2}$ | 398 | $1.51 \times 10^{-7}$ |
| | | $^4H_{11/2}$ | 1628 | $1.99 \times 10^{-8}$ | | | $^4G_{7/2}$ | 651 | $3.32 \times 10^{-4}$ |
| $^2P_{1/2}$ | 35696 | $^6F_{3/2}$ | 342 | $3.83 \times 10^{-6}$ | | | $^4I_{11/2}$ | 694 | $8.36 \times 10^{-6}$ |
| | | $^6F_{5/2}$ | 347 | $3.42 \times 10^{-7}$ | | | $^4M_{15/2}$ | 697 | $7.8 \times 10^{-5}$ |
| | | $^4G_{5/2}$ | 569 | $1.81 \times 10^{-5}$ | | | $(^4K,\, ^4I)\, _{13/2}$ | 708 | $8.92 \times 10^{-4}$ |
| | | $^4F_{3/2}$ | 596 | $1.05 \times 10^{-4}$ | | | $^4I_{9/2}$ | 711 | $2. \times 10^{-5}$ |
| | | $^4F_{5/2}$ | 740 | $8.19 \times 10^{-5}$ | | | $^4G_{9/2}$ | 782 | $3.19 \times 10^{-5}$ |
| | | $(^6P,\, ^4P)\, _{5/2}$ | 844 | $1.46 \times 10^{-5}$ | | | $(^4I,\, ^4K)\, _{15/2}$ | 803 | $3.78 \times 10^{-6}$ |
| | | $^6P_{3/2}$ | 909 | $4.67 \times 10^{-10}$ | | | $^4L_{13/2}$ | 938 | $7.6 \times 10^{-5}$ |
| | | $^4D_{3/2}$ | 1206 | $4.86 \times 10^{-6}$ | | | $^4F_{7/2}$ | 940 | $7.04 \times 10^{-5}$ |
| | | $(^4D,\, ^6P)\, _{5/2}$ | 1216 | $4.01 \times 10^{-6}$ | | | $^4K_{11/2}$ | 942 | $2.16 \times 10^{-4}$ |
| $^4F_{7/2}$ | 35538 | $^6H_{9/2}$ | 301 | $3.79 \times 10^{-5}$ | | | $(^4L,\, ^4I)\, _{15/2}$ | 957 | $1.27 \times 10^{-4}$ |
| | | $^6H_{11/2}$ | 313 | $1.8 \times 10^{-4}$ | | | $^4G_{11/2}$ | 1011 | $4.77 \times 10^{-5}$ |
| | | $^6F_{3/2}$ | 343 | $2.1 \times 10^{-3}$ | | | $^4K_{13/2}$ | 1093 | $1.37 \times 10^{-4}$ |
| | | $^6F_{5/2}$ | 349 | $6.59 \times 10^{-4}$ | | | $^6P_{7/2}$ | 1101 | $2.29 \times 10^{-6}$ |
| | | $^6F_{7/2}$ | 360 | $3.32 \times 10^{-4}$ | | | $^4F_{9/2}$ | 1234 | $4.49 \times 10^{-8}$ |
| | | $^6F_{9/2}$ | 376 | $1.27 \times 10^{-4}$ | | | $^4K_{15/2}$ | 1318 | $5.17 \times 10^{-5}$ |
| | | $^6F_{11/2}$ | 398 | $2.2 \times 10^{-6}$ | | | $^4H_{7/2}$ | 1469 | $1.18 \times 10^{-6}$ |
| | | $^4G_{5/2}$ | 574 | $1.53 \times 10^{-4}$ | | | $^4D_{7/2}$ | 1490 | $3.64 \times 10^{-7}$ |
| | | $^4F_{3/2}$ | 602 | $2.76 \times 10^{-4}$ | | | $^4H_{9/2}$ | 1602 | $3.58 \times 10^{-6}$ |
| | | $^4G_{7/2}$ | 651 | $6.48 \times 10^{-6}$ | $(^4I,\, ^4F)\, _{9/2}$ | 34193 | $^6H_{7/2}$ | 302 | $4.62 \times 10^{-6}$ |
| | | $^4I_{11/2}$ | 693 | $5.24 \times 10^{-5}$ | | | $^6H_{9/2}$ | 313 | $5.63 \times 10^{-5}$ |

[a] The emission rate, $A_{eq}$, inside a host material with refractive index $n_r$ would be: $A_{eq} = A'_{eq}\ n_r^5$

TABLE S18: Continued: $Sm^{3+}$ EQ spontaneous emission lines between 300 and 1700 nm.

| $SLJ$ | $E_{SLJ}(cm^{-1})$ | $S'L'J'$ | $\lambda$ (nm) | $A'_{eq}$ $(s^{-1})$ [a] | $SLJ$ | $E_{SLJ}(cm^{-1})$ | $S'L'J'$ | $\lambda$ (nm) | $A'_{eq}$ $(s^{-1})$ [a] |
|---|---|---|---|---|---|---|---|---|---|
| $({}^4I,\,{}^4F)\,_{9/2}$ | 34193 | ${}^6H_{11/2}$ | 327 | $4.31\times10^{-6}$ | ${}^4F_{9/2}$ | 33661 | ${}^6H_{7/2}$ | 307 | $3.\times10^{-5}$ |
| | | ${}^6H_{13/2}$ | 343 | $7.58\times10^{-5}$ | | | ${}^6H_{9/2}$ | 319 | $8.59\times10^{-5}$ |
| | | ${}^6F_{5/2}$ | 366 | $1.37\times10^{-4}$ | | | ${}^6H_{11/2}$ | 333 | $2.\times10^{-5}$ |
| | | ${}^6F_{7/2}$ | 378 | $1.76\times10^{-4}$ | | | ${}^6H_{13/2}$ | 350 | $9.31\times10^{-5}$ |
| | | ${}^6F_{9/2}$ | 396 | $1.43\times10^{-5}$ | | | ${}^6F_{5/2}$ | 373 | $6.4\times10^{-4}$ |
| | | ${}^6F_{11/2}$ | 420 | $6.85\times10^{-5}$ | | | ${}^6F_{7/2}$ | 386 | $2.26\times10^{-4}$ |
| | | ${}^4G_{5/2}$ | 622 | $3.61\times10^{-4}$ | | | ${}^6F_{9/2}$ | 405 | $1.45\times10^{-5}$ |
| | | ${}^4G_{7/2}$ | 713 | $1.28\times10^{-6}$ | | | ${}^6F_{11/2}$ | 430 | $1.67\times10^{-4}$ |
| | | ${}^4I_{11/2}$ | 764 | $3.33\times10^{-4}$ | | | ${}^4G_{5/2}$ | 643 | $6.71\times10^{-5}$ |
| | | $({}^4K,\,{}^4I)\,_{13/2}$ | 782 | $1.27\times10^{-5}$ | | | ${}^4G_{7/2}$ | 741 | $7.82\times10^{-5}$ |
| | | ${}^4I_{9/2}$ | 785 | $1.61\times10^{-4}$ | | | ${}^4I_{11/2}$ | 797 | $6.41\times10^{-7}$ |
| | | ${}^4F_{5/2}$ | 832 | $1.7\times10^{-5}$ | | | $({}^4K,\,{}^4I)\,_{13/2}$ | 816 | $9.61\times10^{-5}$ |
| | | ${}^4G_{9/2}$ | 873 | $4.83\times10^{-5}$ | | | ${}^4I_{9/2}$ | 819 | $6.68\times10^{-5}$ |
| | | $({}^6P,\,{}^4P)\,_{5/2}$ | 967 | $1.12\times10^{-4}$ | | | ${}^4F_{5/2}$ | 871 | $2.02\times10^{-4}$ |
| | | ${}^4L_{13/2}$ | 1072 | $6.15\times10^{-5}$ | | | ${}^4G_{9/2}$ | 916 | $5.02\times10^{-5}$ |
| | | ${}^4F_{7/2}$ | 1075 | $3.09\times10^{-5}$ | | | $({}^6P,\,{}^4P)\,_{5/2}$ | 1019 | $1.1\times10^{-4}$ |
| | | ${}^4K_{11/2}$ | 1077 | $1.23\times10^{-4}$ | | | ${}^4L_{13/2}$ | 1137 | $4.38\times10^{-5}$ |
| | | ${}^4G_{11/2}$ | 1168 | $1.71\times10^{-6}$ | | | ${}^4F_{7/2}$ | 1140 | $2.18\times10^{-5}$ |
| | | ${}^4K_{13/2}$ | 1279 | $3.97\times10^{-5}$ | | | ${}^4K_{11/2}$ | 1142 | $4.65\times10^{-5}$ |
| | | ${}^6P_{7/2}$ | 1290 | $6.68\times10^{-6}$ | | | ${}^4G_{11/2}$ | 1245 | $9.15\times10^{-6}$ |
| | | ${}^4F_{9/2}$ | 1477 | $6.54\times10^{-8}$ | | | ${}^4K_{13/2}$ | 1372 | $6.01\times10^{-6}$ |
| | | $({}^4D,\,{}^6P)\,_{5/2}$ | 1487 | $5.06\times10^{-6}$ | | | ${}^6P_{7/2}$ | 1385 | $1.27\times10^{-5}$ |
| ${}^2F_{5/2}$ | 33939 | ${}^6H_{7/2}$ | 304 | $3.48\times10^{-5}$ | | | ${}^4F_{9/2}$ | 1603 | $6.58\times10^{-7}$ |
| | | ${}^6H_{9/2}$ | 316 | $2.24\times10^{-5}$ | | | $({}^4D,\,{}^6P)\,_{5/2}$ | 1615 | $7.06\times10^{-6}$ |
| | | ${}^6F_{1/2}$ | 361 | $1.53\times10^{-3}$ | ${}^2K_{13/2}$ | 33157 | ${}^6H_{9/2}$ | 324 | $2.33\times10^{-4}$ |
| | | ${}^6F_{3/2}$ | 363 | $1.13\times10^{-3}$ | | | ${}^6H_{11/2}$ | 339 | $1.41\times10^{-4}$ |
| | | ${}^6F_{5/2}$ | 370 | $6.78\times10^{-4}$ | | | ${}^6H_{13/2}$ | 356 | $4.83\times10^{-7}$ |
| | | ${}^6F_{7/2}$ | 382 | $9.3\times10^{-4}$ | | | ${}^6H_{15/2}$ | 374 | $1.01\times10^{-5}$ |
| | | ${}^6F_{9/2}$ | 400 | $6.14\times10^{-4}$ | | | ${}^6F_{9/2}$ | 413 | $4.13\times10^{-6}$ |
| | | ${}^4G_{5/2}$ | 632 | $1.7\times10^{-4}$ | | | ${}^6F_{11/2}$ | 439 | $1.15\times10^{-6}$ |
| | | ${}^4F_{3/2}$ | 666 | $1.26\times10^{-4}$ | | | ${}^4I_{11/2}$ | 830 | $1.81\times10^{-5}$ |
| | | ${}^4G_{7/2}$ | 726 | $3.4\times10^{-5}$ | | | ${}^4M_{15/2}$ | 835 | $4.8\times10^{-5}$ |
| | | ${}^4I_{9/2}$ | 801 | $1.43\times10^{-5}$ | | | $({}^4K,\,{}^4I)\,_{13/2}$ | 851 | $2.53\times10^{-7}$ |
| | | ${}^4F_{5/2}$ | 850 | $5.26\times10^{-5}$ | | | ${}^4I_{9/2}$ | 855 | $9.44\times10^{-6}$ |
| | | ${}^4G_{9/2}$ | 893 | $1.08\times10^{-5}$ | | | ${}^4M_{17/2}$ | 940 | $1.09\times10^{-8}$ |
| | | $({}^6P,\,{}^4P)\,_{5/2}$ | 991 | $2.78\times10^{-6}$ | | | ${}^4G_{9/2}$ | 960 | $2.97\times10^{-6}$ |
| | | ${}^6P_{3/2}$ | 1082 | $9.43\times10^{-7}$ | | | $({}^4I,\,{}^4K)\,_{15/2}$ | 992 | $1.11\times10^{-5}$ |
| | | ${}^4F_{7/2}$ | 1105 | $8.68\times10^{-6}$ | | | ${}^4L_{13/2}$ | 1206 | $7.24\times10^{-6}$ |
| | | ${}^4D_{1/2}$ | 1304 | $3.02\times10^{-6}$ | | | ${}^4K_{11/2}$ | 1212 | $1.4\times10^{-5}$ |
| | | ${}^6P_{7/2}$ | 1334 | $9.92\times10^{-8}$ | | | $({}^4L,\,{}^4I)\,_{15/2}$ | 1237 | $3.05\times10^{-7}$ |
| | | ${}^4D_{3/2}$ | 1530 | $4.48\times10^{-6}$ | | | ${}^4G_{11/2}$ | 1328 | $1.04\times10^{-6}$ |
| | | ${}^4F_{9/2}$ | 1534 | $7.48\times10^{-7}$ | | | ${}^4L_{17/2}$ | 1384 | $1.77\times10^{-6}$ |
| | | $({}^4D,\,{}^6P)\,_{5/2}$ | 1546 | $9.5\times10^{-7}$ | | | ${}^4K_{13/2}$ | 1475 | $2.53\times10^{-9}$ |

[a] The emission rate, $A_{eq}$, inside a host material with refractive index $n_r$ would be: $A_{eq} = A'_{eq}\ n_r^5$

TABLE S18: Continued: $Sm^{3+}$ EQ spontaneous emission lines between 300 and 1700 nm.

| $SLJ$ | $E_{SLJ}(cm^{-1})$ | $S'L'J'$ | $\lambda$ (nm) | $A'_{eq}$ $(s^{-1})$ [a] | $SLJ$ | $E_{SLJ}(cm^{-1})$ | $S'L'J'$ | $\lambda$ (nm) | $A'_{eq}$ $(s^{-1})$ [a] |
|---|---|---|---|---|---|---|---|---|---|
| $^4P_{5/2}$ | 32581 | $^6H_{5/2}$ | 307 | $1.21 \times 10^{-6}$ | | | $^4G_{7/2}$ | 894 | $1.18 \times 10^{-5}$ |
| | | $^6H_{7/2}$ | 317 | $1.6 \times 10^{-9}$ | | | $^4I_{11/2}$ | 976 | $7.5 \times 10^{-7}$ |
| | | $^6H_{9/2}$ | 330 | $3.34 \times 10^{-7}$ | | | $^4M_{15/2}$ | 983 | $9.66 \times 10^{-5}$ |
| | | $^6F_{1/2}$ | 379 | $1.75 \times 10^{-3}$ | | | $\left(^4K,\,^4I\right)_{13/2}$ | 1005 | $1.02 \times 10^{-4}$ |
| | | $^6F_{3/2}$ | 382 | $3.37 \times 10^{-3}$ | | | $^4I_{9/2}$ | 1010 | $7.89 \times 10^{-8}$ |
| | | $^6F_{5/2}$ | 389 | $4.23 \times 10^{-3}$ | | | $^4G_{9/2}$ | 1161 | $2.93 \times 10^{-6}$ |
| | | $^6F_{7/2}$ | 403 | $3.63 \times 10^{-3}$ | | | $\left(^4I,\,^4K\right)_{15/2}$ | 1207 | $1.33 \times 10^{-4}$ |
| | | $^6F_{9/2}$ | 423 | $2.67 \times 10^{-3}$ | | | $^4L_{13/2}$ | 1540 | $3.32 \times 10^{-6}$ |
| | | $^4G_{5/2}$ | 691 | $3.62 \times 10^{-5}$ | | | $^4F_{7/2}$ | 1546 | $1.06 \times 10^{-6}$ |
| | | $^4F_{3/2}$ | 732 | $1.08 \times 10^{-4}$ | | | $^4K_{11/2}$ | 1550 | $5.13 \times 10^{-7}$ |
| | | $^4G_{7/2}$ | 806 | $1.85 \times 10^{-5}$ | | | $\left(^4L,\,^4I\right)_{15/2}$ | 1590 | $1.67 \times 10^{-5}$ |
| | | $^4I_{9/2}$ | 899 | $1.22 \times 10^{-6}$ | $^4P_{3/2}$ | 31340 | $^6H_{5/2}$ | 319 | $3.62 \times 10^{-7}$ |
| | | $^4F_{5/2}$ | 961 | $3.07 \times 10^{-5}$ | | | $^6H_{7/2}$ | 330 | $4.59 \times 10^{-7}$ |
| | | $^4G_{9/2}$ | 1016 | $3.02 \times 10^{-6}$ | | | $^6F_{1/2}$ | 398 | $1.72 \times 10^{-2}$ |
| | | $\left(^6P,\,^4P\right)_{5/2}$ | 1145 | $2.5 \times 10^{-6}$ | | | $^6F_{3/2}$ | 401 | $6.95 \times 10^{-3}$ |
| | | $^6P_{3/2}$ | 1269 | $2.79 \times 10^{-6}$ | $^4G_{11/2}$ | 31358 | $^6F_{5/2}$ | 409 | $2.96 \times 10^{-3}$ |
| | | $^4F_{7/2}$ | 1300 | $2.34 \times 10^{-5}$ | | | $^6F_{7/2}$ | 424 | $1.21 \times 10^{-3}$ |
| | | $^4D_{1/2}$ | 1584 | $2.51 \times 10^{-5}$ | | | $^4G_{5/2}$ | 756 | $6.09 \times 10^{-5}$ |
| | | $^6P_{7/2}$ | 1629 | $5.93 \times 10^{-9}$ | | | $^4F_{3/2}$ | 805 | $2.08 \times 10^{-4}$ |
| $\left(^2K,\,^2L\right)_{15/2}$ | 32362 | $^6H_{11/2}$ | 348 | $3.52 \times 10^{-5}$ | | | $^4G_{7/2}$ | 895 | $8.71 \times 10^{-6}$ |
| | | $^6H_{13/2}$ | 366 | $8.32 \times 10^{-5}$ | | | $^4F_{5/2}$ | 1091 | $4.31 \times 10^{-5}$ |
| | | $^6H_{15/2}$ | 386 | $4.47 \times 10^{-5}$ | | | $\left(^6P,\,^4P\right)_{5/2}$ | 1335 | $3.5 \times 10^{-7}$ |
| | | $^6F_{11/2}$ | 455 | $4.53 \times 10^{-6}$ | | | $^6P_{3/2}$ | 1505 | $5.97 \times 10^{-7}$ |
| | | $^4I_{11/2}$ | 888 | $1.11 \times 10^{-5}$ | | | $^4F_{7/2}$ | 1550 | $5.23 \times 10^{-6}$ |
| | | $^4M_{15/2}$ | 894 | $1.03 \times 10^{-6}$ | $^4P_{1/2}$ | 30973 | $^6H_{5/2}$ | 323 | $9.02 \times 10^{-7}$ |
| | | $\left(^4K,\,^4I\right)_{13/2}$ | 913 | $2.12 \times 10^{-6}$ | | | $^6F_{3/2}$ | 407 | $7.03 \times 10^{-6}$ |
| | | $^4M_{17/2}$ | 1016 | $2.25 \times 10^{-5}$ | | | $^6F_{5/2}$ | 415 | $9.9 \times 10^{-6}$ |
| | | $\left(^4I,\,^4K\right)_{15/2}$ | 1076 | $2.46 \times 10^{-5}$ | | | $^4G_{5/2}$ | 778 | $1.75 \times 10^{-5}$ |
| | | $^4M_{19/2}$ | 1204 | $1.06 \times 10^{-6}$ | | | $^4F_{3/2}$ | 830 | $2.59 \times 10^{-4}$ |
| | | $^4L_{13/2}$ | 1334 | $1.72 \times 10^{-6}$ | | | $^4F_{5/2}$ | 1137 | $4.6 \times 10^{-7}$ |
| | | $^4K_{11/2}$ | 1341 | $8.32 \times 10^{-8}$ | | | $\left(^6P,\,^4P\right)_{5/2}$ | 1404 | $1.76 \times 10^{-6}$ |
| | | $\left(^4L,\,^4I\right)_{15/2}$ | 1371 | $4.13 \times 10^{-6}$ | | | $^6P_{3/2}$ | 1594 | $8.83 \times 10^{-7}$ |
| | | $^4G_{11/2}$ | 1485 | $8.85 \times 10^{-7}$ | $^4H_{13/2}$ | 30158 | $^6H_{9/2}$ | 359 | $6.67 \times 10^{-5}$ |
| | | $^4L_{17/2}$ | 1555 | $2.97 \times 10^{-6}$ | | | $^6H_{11/2}$ | 377 | $1.03 \times 10^{-4}$ |
| | | $^4K_{13/2}$ | 1670 | $7.64 \times 10^{-7}$ | | | $^6H_{13/2}$ | 399 | $4.21 \times 10^{-5}$ |
| $^4G_{11/2}$ | 31358 | $^6H_{7/2}$ | 330 | $3.77 \times 10^{-6}$ | | | $^6H_{15/2}$ | 422 | $1.26 \times 10^{-3}$ |
| | | $^6H_{9/2}$ | 344 | $3.6 \times 10^{-8}$ | | | $^6F_{9/2}$ | 472 | $4.19 \times 10^{-5}$ |
| | | $^6H_{11/2}$ | 361 | $4.25 \times 10^{-5}$ | | | $^6F_{11/2}$ | 506 | $5.62 \times 10^{-6}$ |
| | | $^6H_{13/2}$ | 380 | $6.07 \times 10^{-6}$ | | | $^4I_{11/2}$ | 1105 | $2.73 \times 10^{-6}$ |
| | | $^6H_{15/2}$ | 402 | $5.06 \times 10^{-5}$ | | | $^4M_{15/2}$ | 1114 | $4.48 \times 10^{-5}$ |
| | | $^6F_{7/2}$ | 424 | $1.89 \times 10^{-5}$ | | | $\left(^4K,\,^4I\right)_{13/2}$ | 1143 | $2.03 \times 10^{-5}$ |
| | | $^6F_{9/2}$ | 447 | $1.7 \times 10^{-6}$ | | | $^4I_{9/2}$ | 1149 | $3.67 \times 10^{-7}$ |
| | | $^6F_{11/2}$ | 477 | $6.4 \times 10^{-5}$ | | | $^4M_{17/2}$ | 1310 | $3.84 \times 10^{-6}$ |

[a] The emission rate, $A_{eq}$, inside a host material with refractive index $n_r$ would be: $A_{eq} = A'_{eq}\ n_r^5$

TABLE S18: Continued: $Sm^{3+}$ EQ spontaneous emission lines between 300 and 1700 nm.

| $SLJ$ | $E_{SLJ}(cm^{-1})$ | $S'L'J'$ | $\lambda$ (nm) | $A'_{eq}$ $(s^{-1})$ [a] | $SLJ$ | $E_{SLJ}(cm^{-1})$ | $S'L'J'$ | $\lambda$ (nm) | $A'_{eq}$ $(s^{-1})$ [a] |
|---|---|---|---|---|---|---|---|---|---|
| $^4H_{13/2}$ | 30158 | $^4G_{9/2}$ | 1348 | $2.16 \times 10^{-5}$ | $^4G_{7/2}$ | 29992 | $^4G_{5/2}$ | 842 | $3.68 \times 10^{-6}$ |
| | | $(^4I,\, ^4K)_{15/2}$ | 1411 | $5.85 \times 10^{-5}$ | | | $^4F_{3/2}$ | 903 | $4.08 \times 10^{-5}$ |
| $^4G_{9/2}$ | 30108 | $^6H_{5/2}$ | 332 | $5.67 \times 10^{-6}$ | | | $^4G_{7/2}$ | 1018 | $1.65 \times 10^{-4}$ |
| | | $^6H_{7/2}$ | 344 | $6.2 \times 10^{-6}$ | | | $^4I_{11/2}$ | 1125 | $1.83 \times 10^{-4}$ |
| | | $^6H_{9/2}$ | 359 | $1.28 \times 10^{-5}$ | | | $^4I_{9/2}$ | 1171 | $4.08 \times 10^{-5}$ |
| | | $^6H_{11/2}$ | 378 | $8.64 \times 10^{-6}$ | | | $^4F_{5/2}$ | 1280 | $3.56 \times 10^{-5}$ |
| | | $^6H_{13/2}$ | 399 | $3.43 \times 10^{-5}$ | | | $^4G_{9/2}$ | 1379 | $1.01 \times 10^{-5}$ |
| | | $^6F_{5/2}$ | 431 | $1.4 \times 10^{-4}$ | | | $(^6P,\, ^4P)_{5/2}$ | 1628 | $5.22 \times 10^{-9}$ |
| | | $^6F_{7/2}$ | 447 | $2.87 \times 10^{-7}$ | $^4H_{11/2}$ | 29711 | $^6H_{7/2}$ | 349 | $1.41 \times 10^{-4}$ |
| | | $^6F_{9/2}$ | 473 | $2.59 \times 10^{-5}$ | | | $^6H_{9/2}$ | 364 | $1.67 \times 10^{-4}$ |
| | | $^6F_{11/2}$ | 507 | $7.09 \times 10^{-7}$ | | | $^6H_{11/2}$ | 383 | $1.21 \times 10^{-4}$ |
| | | $^4G_{5/2}$ | 834 | $6.16 \times 10^{-6}$ | | | $^6H_{13/2}$ | 406 | $4.13 \times 10^{-4}$ |
| | | $^4G_{7/2}$ | 1006 | $9.42 \times 10^{-6}$ | | | $^6H_{15/2}$ | 430 | $3.05 \times 10^{-5}$ |
| | | $^4I_{11/2}$ | 1111 | $8.44 \times 10^{-5}$ | | | $^6F_{7/2}$ | 455 | $2.18 \times 10^{-5}$ |
| | | $(^4K,\, ^4I)_{13/2}$ | 1149 | $1.56 \times 10^{-4}$ | | | $^6F_{9/2}$ | 482 | $1.39 \times 10^{-5}$ |
| | | $^4I_{9/2}$ | 1156 | $7.84 \times 10^{-8}$ | | | $^6F_{11/2}$ | 518 | $2.32 \times 10^{-5}$ |
| | | $^4F_{5/2}$ | 1261 | $1.19 \times 10^{-6}$ | | | $^4G_{7/2}$ | 1048 | $7.95 \times 10^{-5}$ |
| | | $^4G_{9/2}$ | 1358 | $6.27 \times 10^{-5}$ | | | $^4I_{11/2}$ | 1162 | $3.05 \times 10^{-5}$ |
| | | $(^6P,\, ^4P)_{5/2}$ | 1598 | $1.34 \times 10^{-5}$ | | | $^4M_{15/2}$ | 1172 | $1.73 \times 10^{-6}$ |
| $^4G_{5/2}$ | 30079 | $^6H_{5/2}$ | 332 | $1.11 \times 10^{-4}$ | | | $(^4K,\, ^4I)_{13/2}$ | 1204 | $1.07 \times 10^{-4}$ |
| | | $^6H_{7/2}$ | 345 | $3.62 \times 10^{-5}$ | | | $^4I_{9/2}$ | 1211 | $2.19 \times 10^{-6}$ |
| | | $^6H_{9/2}$ | 360 | $9.41 \times 10^{-7}$ | | | $^4G_{9/2}$ | 1435 | $4.48 \times 10^{-6}$ |
| | | $^6F_{1/2}$ | 419 | $1.16 \times 10^{-3}$ | | | $(^4I,\, ^4K)_{15/2}$ | 1506 | $6.67 \times 10^{-7}$ |
| | | $^6F_{3/2}$ | 423 | $6.06 \times 10^{-5}$ | $^4H_{9/2}$ | 29282 | $^6H_{5/2}$ | 342 | $3.11 \times 10^{-4}$ |
| | | $^6F_{5/2}$ | 431 | $4.8 \times 10^{-5}$ | | | $^6H_{7/2}$ | 354 | $5.24 \times 10^{-4}$ |
| | | $^6F_{7/2}$ | 448 | $1.04 \times 10^{-5}$ | | | $^6H_{9/2}$ | 370 | $1.1 \times 10^{-4}$ |
| | | $^6F_{9/2}$ | 474 | $4.25 \times 10^{-6}$ | | | $^6H_{11/2}$ | 390 | $9.68 \times 10^{-5}$ |
| | | $^4G_{5/2}$ | 836 | $2.92 \times 10^{-4}$ | | | $^6H_{13/2}$ | 413 | $6.49 \times 10^{-5}$ |
| | | $^4F_{3/2}$ | 896 | $1.16 \times 10^{-4}$ | | | $^6F_{5/2}$ | 446 | $4.77 \times 10^{-5}$ |
| | | $^4G_{7/2}$ | 1009 | $3.09 \times 10^{-5}$ | | | $^6F_{7/2}$ | 465 | $2.11 \times 10^{-5}$ |
| | | $^4I_{9/2}$ | 1160 | $2. \times 10^{-4}$ | | | $^6F_{9/2}$ | 492 | $1.32 \times 10^{-5}$ |
| | | $^4F_{5/2}$ | 1266 | $1.51 \times 10^{-6}$ | | | $^6F_{11/2}$ | 530 | $3. \times 10^{-6}$ |
| | | $^4G_{9/2}$ | 1363 | $4.46 \times 10^{-7}$ | | | $^4G_{5/2}$ | 896 | $1.9 \times 10^{-4}$ |
| | | $(^6P,\, ^4P)_{5/2}$ | 1605 | $8.76 \times 10^{-9}$ | | | $^4G_{7/2}$ | 1098 | $8.07 \times 10^{-6}$ |
| $^4G_{7/2}$ | 29992 | $^6H_{5/2}$ | 333 | $1.77 \times 10^{-5}$ | | | $^4I_{11/2}$ | 1223 | $1.17 \times 10^{-4}$ |
| | | $^6H_{7/2}$ | 346 | $3.71 \times 10^{-5}$ | | | $(^4K,\, ^4I)_{13/2}$ | 1270 | $3.23 \times 10^{-6}$ |
| | | $^6H_{9/2}$ | 361 | $6.31 \times 10^{-5}$ | | | $^4I_{9/2}$ | 1278 | $1.94 \times 10^{-5}$ |
| | | $^6H_{11/2}$ | 379 | $3.55 \times 10^{-6}$ | | | $^4F_{5/2}$ | 1408 | $2.25 \times 10^{-6}$ |
| | | $^6F_{3/2}$ | 424 | $2.72 \times 10^{-4}$ | | | $^4G_{9/2}$ | 1529 | $2.34 \times 10^{-7}$ |
| | | $^6F_{5/2}$ | 433 | $3.06 \times 10^{-5}$ | $^4L_{19/2}$ | 29230 | $^6H_{15/2}$ | 439 | $1.56 \times 10^{-4}$ |
| | | $^6F_{7/2}$ | 450 | $1.85 \times 10^{-8}$ | | | $^4M_{15/2}$ | 1242 | $4.16 \times 10^{-6}$ |
| | | $^6F_{9/2}$ | 476 | $1.51 \times 10^{-6}$ | | | $^4M_{17/2}$ | 1491 | $7.5 \times 10^{-7}$ |
| | | $^6F_{11/2}$ | 510 | $2.07 \times 10^{-10}$ | | | $(^4I,\, ^4K)_{15/2}$ | 1624 | $7.67 \times 10^{-6}$ |

[a] The emission rate, $A_{eq}$, inside a host material with refractive index $n_r$ would be: $A_{eq} = A'_{eq}\ n_r^5$

TABLE S18: Continued: $Sm^{3+}$ EQ spontaneous emission lines between 300 and 1700 nm.

| $SLJ$ | $E_{SLJ}(cm^{-1})$ | $S'L'J'$ | $\lambda$ (nm) | $A'_{eq}$ $(s^{-1})$ [a] | $SLJ$ | $E_{SLJ}(cm^{-1})$ | $S'L'J'$ | $\lambda$ (nm) | $A'_{eq}$ $(s^{-1})$ [a] |
|---|---|---|---|---|---|---|---|---|---|
| $^4D_{7/2}$ | 28813 | $^6H_{5/2}$ | 347 | $2.7\times10^{-5}$ | $(^4D,\,^6P)_{5/2}$ | 27469 | $^6H_{5/2}$ | 364 | $2.6\times10^{-5}$ |
| | | $^6H_{7/2}$ | 360 | $1.29\times10^{-5}$ | | | $^6H_{7/2}$ | 379 | $6.62\times10^{-5}$ |
| | | $^6H_{9/2}$ | 377 | $1.54\times10^{-5}$ | | | $^6H_{9/2}$ | 397 | $1.31\times10^{-5}$ |
| | | $^6H_{11/2}$ | 397 | $1.94\times10^{-6}$ | | | $^6F_{1/2}$ | 470 | $4.79\times10^{-3}$ |
| | | $^6F_{3/2}$ | 446 | $6.12\times10^{-4}$ | | | $^6F_{3/2}$ | 475 | $9.68\times10^{-3}$ |
| | | $^6F_{5/2}$ | 456 | $2.\times10^{-3}$ | | | $^6F_{5/2}$ | 486 | $1.18\times10^{-2}$ |
| | | $^6F_{7/2}$ | 475 | $4.45\times10^{-3}$ | | | $^6F_{7/2}$ | 507 | $1.04\times10^{-2}$ |
| | | $^6F_{9/2}$ | 504 | $7.68\times10^{-3}$ | | | $^6F_{9/2}$ | 540 | $5.06\times10^{-3}$ |
| | | $^6F_{11/2}$ | 543 | $9.14\times10^{-3}$ | | | $^4G_{5/2}$ | 1069 | $5.3\times10^{-5}$ |
| | | $^4G_{5/2}$ | 935 | $4.51\times10^{-6}$ | | | $^4F_{3/2}$ | 1169 | $2.99\times10^{-5}$ |
| | | $^4F_{3/2}$ | 1011 | $2.74\times10^{-7}$ | | | $^4G_{7/2}$ | 1370 | $1.53\times10^{-5}$ |
| | | $^4G_{7/2}$ | 1157 | $1.38\times10^{-5}$ | | | $^4I_{9/2}$ | 1663 | $5.48\times10^{-8}$ |
| | | $^4I_{11/2}$ | 1298 | $8.62\times10^{-8}$ | $^4F_{9/2}$ | 27421 | $^6H_{5/2}$ | 365 | $3.6\times10^{-5}$ |
| | | $^4I_{9/2}$ | 1359 | $4.03\times10^{-7}$ | | | $^6H_{7/2}$ | 379 | $8.77\times10^{-5}$ |
| | | $^4F_{5/2}$ | 1507 | $2.46\times10^{-6}$ | | | $^6H_{9/2}$ | 398 | $1.25\times10^{-5}$ |
| | | $^4G_{9/2}$ | 1647 | $3.78\times10^{-6}$ | | | $^6H_{11/2}$ | 420 | $2.32\times10^{-4}$ |
| $^4H_{7/2}$ | 28715 | $^6H_{5/2}$ | 348 | $1.74\times10^{-3}$ | | | $^6H_{13/2}$ | 447 | $4.17\times10^{-4}$ |
| | | $^6H_{7/2}$ | 362 | $9.2\times10^{-5}$ | | | $^6F_{5/2}$ | 487 | $1.51\times10^{-4}$ |
| | | $^6H_{9/2}$ | 378 | $3.23\times10^{-5}$ | | | $^6F_{7/2}$ | 509 | $1.99\times10^{-5}$ |
| | | $^6H_{11/2}$ | 399 | $6.58\times10^{-6}$ | | | $^6F_{9/2}$ | 542 | $3.3\times10^{-6}$ |
| | | $^6F_{3/2}$ | 448 | $1.36\times10^{-4}$ | | | $^6F_{11/2}$ | 588 | $9.16\times10^{-6}$ |
| | | $^6F_{5/2}$ | 458 | $5.44\times10^{-5}$ | | | $^4G_{5/2}$ | 1075 | $1.85\times10^{-5}$ |
| | | $^6F_{7/2}$ | 477 | $9.12\times10^{-7}$ | | | $^4G_{7/2}$ | 1379 | $2.7\times10^{-6}$ |
| | | $^6F_{9/2}$ | 506 | $4.27\times10^{-5}$ | | | $^4I_{11/2}$ | 1584 | $1.3\times10^{-6}$ |
| | | $^6F_{11/2}$ | 546 | $3.21\times10^{-5}$ | | | $(^4K,\,^4I)_{13/2}$ | 1662 | $3.8\times10^{-9}$ |
| | | $^4G_{5/2}$ | 943 | $3.96\times10^{-5}$ | | | $^4I_{9/2}$ | 1676 | $5.79\times10^{-7}$ |
| | | $^4F_{3/2}$ | 1021 | $1.88\times10^{-4}$ | $^4D_{3/2}$ | 27403 | $^6H_{5/2}$ | 365 | $5.32\times10^{-5}$ |
| | | $^4G_{7/2}$ | 1170 | $2.54\times10^{-7}$ | | | $^6H_{7/2}$ | 380 | $2.11\times10^{-5}$ |
| | | $^4I_{11/2}$ | 1314 | $4.33\times10^{-6}$ | | | $^6F_{1/2}$ | 472 | $1.47\times10^{-2}$ |
| | | $^4I_{9/2}$ | 1377 | $9.1\times10^{-5}$ | | | $^6F_{3/2}$ | 476 | $6.49\times10^{-3}$ |
| | | $^4F_{5/2}$ | 1530 | $1.55\times10^{-5}$ | | | $^6F_{5/2}$ | 487 | $2.9\times10^{-3}$ |
| | | $^4G_{9/2}$ | 1674 | $3.97\times10^{-9}$ | | | $^6F_{7/2}$ | 509 | $5.73\times10^{-4}$ |
| $^4K_{17/2}$ | 28173 | $^6H_{13/2}$ | 433 | $1.16\times10^{-4}$ | | | $^4G_{5/2}$ | 1077 | $5.34\times10^{-5}$ |
| | | $^6H_{15/2}$ | 460 | $2.79\times10^{-4}$ | | | $^4F_{3/2}$ | 1179 | $7.72\times10^{-5}$ |
| | | $^4M_{15/2}$ | 1430 | $6.86\times10^{-8}$ | | | $^4G_{7/2}$ | 1383 | $6.65\times10^{-6}$ |
| | | $(^4K,\,^4I)_{13/2}$ | 1478 | $3.07\times10^{-6}$ | $^6P_{7/2}$ | 26443 | $^6H_{5/2}$ | 378 | $6.82\times10^{-7}$ |
| $^4K_{15/2}$ | 27936 | $^6H_{11/2}$ | 411 | $1.24\times10^{-4}$ | | | $^6H_{7/2}$ | 394 | $1.75\times10^{-6}$ |
| | | $^6H_{13/2}$ | 437 | $3.13\times10^{-4}$ | | | $^6H_{9/2}$ | 414 | $1.28\times10^{-5}$ |
| | | $^6H_{15/2}$ | 465 | $5.86\times10^{-6}$ | | | $^6H_{11/2}$ | 438 | $2.86\times10^{-5}$ |
| | | $^6F_{11/2}$ | 570 | $1.83\times10^{-6}$ | | | $^6F_{3/2}$ | 499 | $6.62\times10^{-4}$ |
| | | $^4I_{11/2}$ | 1464 | $3.5\times10^{-6}$ | | | $^6F_{5/2}$ | 511 | $2.69\times10^{-3}$ |
| | | $^4M_{15/2}$ | 1480 | $8.7\times10^{-7}$ | | | $^6F_{7/2}$ | 535 | $5.68\times10^{-3}$ |
| | | $(^4K,\,^4I)_{13/2}$ | 1531 | $3.61\times10^{-7}$ | | | $^6F_{9/2}$ | 572 | $7.92\times10^{-3}$ |

[a] The emission rate, $A_{eq}$, inside a host material with refractive index $n_r$ would be: $A_{eq} = A'_{eq}\ n_r^5$

TABLE S18: Continued: $Sm^{3+}$ EQ spontaneous emission lines between 300 and 1700 nm.

| $SLJ$ | $E_{SLJ}(cm^{-1})$ | $S'L'J'$ | $\lambda$ (nm) | $A'_{eq}$ $(s^{-1})$ [a] | $SLJ$ | $E_{SLJ}(cm^{-1})$ | $S'L'J'$ | $\lambda$ (nm) | $A'_{eq}$ $(s^{-1})$ [a] |
|---|---|---|---|---|---|---|---|---|---|
| $^6P_{7/2}$ | 26443 | $^6F_{11/2}$ | 623 | $9.38 \times 10^{-3}$ | $^4F_{7/2}$ | 24889 | $^6F_{7/2}$ | 584 | $1.54 \times 10^{-4}$ |
| | | $^4G_{5/2}$ | 1201 | $3.22 \times 10^{-6}$ | | | $^6F_{9/2}$ | 628 | $2.36 \times 10^{-4}$ |
| | | $^4F_{3/2}$ | 1329 | $2.97 \times 10^{-6}$ | | | $^6F_{11/2}$ | 690 | $1.87 \times 10^{-4}$ |
| | | $^4G_{7/2}$ | 1595 | $1.05 \times 10^{-8}$ | | | $^4G_{5/2}$ | 1476 | $7.63 \times 10^{-7}$ |
| $^4K_{13/2}$ | 26375 | $^6H_{9/2}$ | 415 | $1.09 \times 10^{-4}$ | | | $^4F_{3/2}$ | 1675 | $7.81 \times 10^{-6}$ |
| | | $^6H_{11/2}$ | 440 | $1.74 \times 10^{-4}$ | $^4L_{13/2}$ | 24865 | $^6H_{9/2}$ | 443 | $1.43 \times 10^{-5}$ |
| | | $^6H_{13/2}$ | 469 | $5.54 \times 10^{-7}$ | | | $^6H_{11/2}$ | 471 | $6.99 \times 10^{-5}$ |
| | | $^6H_{15/2}$ | 502 | $2.97 \times 10^{-7}$ | | | $^6H_{13/2}$ | 505 | $2.39 \times 10^{-5}$ |
| | | $^6F_{9/2}$ | 574 | $4.33 \times 10^{-7}$ | | | $^6H_{15/2}$ | 543 | $2.18 \times 10^{-9}$ |
| | | $^6F_{11/2}$ | 626 | $1.19 \times 10^{-7}$ | | | $^6F_{9/2}$ | 629 | $1.97 \times 10^{-6}$ |
| $^4D_{1/2}$ | 26269 | $^6H_{5/2}$ | 381 | $2.32 \times 10^{-5}$ | | | $^6F_{11/2}$ | 691 | $3.55 \times 10^{-7}$ |
| | | $^6F_{3/2}$ | 504 | $1.2 \times 10^{-5}$ | $^6P_{3/2}$ | 24698 | $^6H_{5/2}$ | 405 | $1.91 \times 10^{-6}$ |
| | | $^6F_{5/2}$ | 516 | $8.99 \times 10^{-6}$ | | | $^6H_{7/2}$ | 423 | $1.25 \times 10^{-6}$ |
| | | $^4G_{5/2}$ | 1226 | $5.32 \times 10^{-6}$ | | | $^6F_{1/2}$ | 541 | $7.04 \times 10^{-2}$ |
| | | $^4F_{3/2}$ | 1360 | $3.71 \times 10^{-6}$ | | | $^6F_{3/2}$ | 547 | $2.55 \times 10^{-2}$ |
| $^4L_{17/2}$ | 25931 | $^6H_{13/2}$ | 479 | $3.48 \times 10^{-6}$ | | | $^6F_{5/2}$ | 561 | $9.02 \times 10^{-3}$ |
| | | $^6H_{15/2}$ | 513 | $8.68 \times 10^{-5}$ | | | $^6F_{7/2}$ | 590 | $2.16 \times 10^{-3}$ |
| $^4G_{11/2}$ | 25628 | $^6H_{7/2}$ | 407 | $1.22 \times 10^{-5}$ | | | $^4G_{5/2}$ | 1519 | $2.75 \times 10^{-8}$ |
| | | $^6H_{9/2}$ | 428 | $6.99 \times 10^{-5}$ | $^4M_{19/2}$ | 24060 | $^6H_{15/2}$ | 568 | $4.95 \times 10^{-6}$ |
| | | $^6H_{11/2}$ | 454 | $9.89 \times 10^{-7}$ | $(^6P,\,^4P)_{5/2}$ | 23849 | $^6H_{5/2}$ | 419 | $2.8 \times 10^{-7}$ |
| | | $^6H_{13/2}$ | 486 | $9.7 \times 10^{-5}$ | | | $^6H_{7/2}$ | 439 | $3.45 \times 10^{-6}$ |
| | | $^6H_{15/2}$ | 522 | $6.37 \times 10^{-9}$ | | | $^6H_{9/2}$ | 464 | $2.31 \times 10^{-5}$ |
| | | $^6F_{7/2}$ | 560 | $1.05 \times 10^{-4}$ | | | $^6F_{1/2}$ | 567 | $4.69 \times 10^{-3}$ |
| | | $^6F_{9/2}$ | 600 | $9.26 \times 10^{-6}$ | | | $^6F_{3/2}$ | 574 | $7.4 \times 10^{-3}$ |
| | | $^6F_{11/2}$ | 657 | $7.27 \times 10^{-5}$ | | | $^6F_{5/2}$ | 589 | $7.74 \times 10^{-3}$ |
| $(^4L,\,^4I)_{15/2}$ | 25070 | $^6H_{11/2}$ | 466 | $1.89 \times 10^{-6}$ | | | $^6F_{7/2}$ | 621 | $5.42 \times 10^{-3}$ |
| | | $^6H_{13/2}$ | 500 | $8.41 \times 10^{-5}$ | | | $^6F_{9/2}$ | 672 | $2.5 \times 10^{-3}$ |
| | | $^6H_{15/2}$ | 537 | $5.32 \times 10^{-5}$ | $(^4I,\,^4K)_{15/2}$ | 23072 | $^6H_{11/2}$ | 514 | $1.34 \times 10^{-5}$ |
| | | $^6F_{11/2}$ | 682 | $4.79 \times 10^{-6}$ | | | $^6H_{13/2}$ | 555 | $8.3 \times 10^{-7}$ |
| $^4K_{11/2}$ | 24905 | $^6H_{7/2}$ | 420 | $2.56 \times 10^{-4}$ | | | $^6H_{15/2}$ | 602 | $1. \times 10^{-4}$ |
| | | $^6H_{9/2}$ | 442 | $1.38 \times 10^{-4}$ | | | $^6F_{11/2}$ | 789 | $5.79 \times 10^{-6}$ |
| | | $^6H_{11/2}$ | 470 | $1.78 \times 10^{-6}$ | $^4G_{9/2}$ | 22742 | $^6H_{5/2}$ | 440 | $1.96 \times 10^{-5}$ |
| | | $^6H_{13/2}$ | 504 | $7.88 \times 10^{-7}$ | | | $^6H_{7/2}$ | 461 | $6.27 \times 10^{-5}$ |
| | | $^6H_{15/2}$ | 542 | $2.49 \times 10^{-8}$ | | | $^6H_{9/2}$ | 489 | $7.35 \times 10^{-7}$ |
| | | $^6F_{7/2}$ | 583 | $7.63 \times 10^{-7}$ | | | $^6H_{11/2}$ | 523 | $5.92 \times 10^{-6}$ |
| | | $^6F_{9/2}$ | 627 | $1.69 \times 10^{-7}$ | | | $^6H_{13/2}$ | 566 | $7.84 \times 10^{-5}$ |
| | | $^6F_{11/2}$ | 690 | $5.09 \times 10^{-7}$ | | | $^6F_{5/2}$ | 631 | $1.38 \times 10^{-4}$ |
| $^4F_{7/2}$ | 24889 | $^6H_{5/2}$ | 402 | $8.37 \times 10^{-5}$ | | | $^6F_{7/2}$ | 667 | $3.32 \times 10^{-8}$ |
| | | $^6H_{7/2}$ | 420 | $1.65 \times 10^{-6}$ | | | $^6F_{9/2}$ | 726 | $6.68 \times 10^{-5}$ |
| | | $^6H_{9/2}$ | 442 | $1.43 \times 10^{-4}$ | | | $^6F_{11/2}$ | 810 | $2.03 \times 10^{-6}$ |
| | | $^6H_{11/2}$ | 470 | $3.57 \times 10^{-4}$ | $^4M_{17/2}$ | 22523 | $^6H_{13/2}$ | 573 | $6.24 \times 10^{-7}$ |
| | | $^6F_{3/2}$ | 541 | $2.47 \times 10^{-4}$ | | | $^6H_{15/2}$ | 622 | $3.95 \times 10^{-6}$ |
| | | $^6F_{5/2}$ | 555 | $1.43 \times 10^{-4}$ | $^4F_{5/2}$ | 22177 | $^6H_{5/2}$ | 451 | $5.43 \times 10^{-5}$ |

[a] The emission rate, $A_{eq}$, inside a host material with refractive index $n_r$ would be: $A_{eq} = A'_{eq}\ n_r^5$

TABLE S18: Continued: $Sm^{3+}$ EQ spontaneous emission lines between 300 and 1700 nm.

| $SLJ$ | $E_{SLJ}(cm^{-1})$ | $S'L'J'$ | $\lambda$ (nm) | $A'_{eq}$ $(s^{-1})$ [a] | $SLJ$ | $E_{SLJ}(cm^{-1})$ | $S'L'J'$ | $\lambda$ (nm) | $A'_{eq}$ $(s^{-1})$ [a] |
|---|---|---|---|---|---|---|---|---|---|
| $^4F_{5/2}$ | 22177 | $^6H_{7/2}$ | 474 | $5.12 \times 10^{-5}$ | $^4G_{7/2}$ | 20172 | $^6H_{5/2}$ | 496 | $6.32 \times 10^{-5}$ |
| | | $^6H_{9/2}$ | 502 | $2.26 \times 10^{-4}$ | | | $^6H_{7/2}$ | 523 | $7. \times 10^{-6}$ |
| | | $^6F_{1/2}$ | 626 | $3.15 \times 10^{-4}$ | | | $^6H_{9/2}$ | 559 | $1.04 \times 10^{-6}$ |
| | | $^6F_{3/2}$ | 634 | $3. \times 10^{-4}$ | | | $^6H_{11/2}$ | 604 | $1.48 \times 10^{-4}$ |
| | | $^6F_{5/2}$ | 654 | $1.94 \times 10^{-4}$ | | | $^6F_{3/2}$ | 727 | $1.17 \times 10^{-4}$ |
| | | $^6F_{7/2}$ | 693 | $1.44 \times 10^{-4}$ | | | $^6F_{5/2}$ | 753 | $7.66 \times 10^{-6}$ |
| | | $^6F_{9/2}$ | 757 | $4.93 \times 10^{-5}$ | | | $^6F_{7/2}$ | 805 | $5.13 \times 10^{-5}$ |
| $^4I_{9/2}$ | 21456 | $^6H_{5/2}$ | 466 | $4.92 \times 10^{-4}$ | | | $^6F_{9/2}$ | 892 | $1.46 \times 10^{-6}$ |
| | | $^6H_{7/2}$ | 491 | $7.19 \times 10^{-5}$ | | | $^6F_{11/2}$ | 1024 | $8.46 \times 10^{-7}$ |
| | | $^6H_{9/2}$ | 521 | $1.69 \times 10^{-6}$ | $^4F_{3/2}$ | 18918 | $^6H_{5/2}$ | 529 | $5.15 \times 10^{-6}$ |
| | | $^6H_{11/2}$ | 561 | $2.36 \times 10^{-7}$ | | | $^6H_{7/2}$ | 560 | $2. \times 10^{-4}$ |
| | | $^6H_{13/2}$ | 610 | $8.16 \times 10^{-8}$ | | | $^6F_{1/2}$ | 787 | $2.82 \times 10^{-6}$ |
| | | $^6F_{5/2}$ | 686 | $5.4 \times 10^{-6}$ | | | $^6F_{3/2}$ | 800 | $1.57 \times 10^{-5}$ |
| | | $^6F_{7/2}$ | 730 | $2.62 \times 10^{-7}$ | | | $^6F_{5/2}$ | 831 | $1.82 \times 10^{-7}$ |
| | | $^6F_{9/2}$ | 801 | $2.87 \times 10^{-9}$ | | | $^6F_{7/2}$ | 896 | $2.72 \times 10^{-7}$ |
| | | $^6F_{11/2}$ | 905 | $8.6 \times 10^{-12}$ | $^4G_{5/2}$ | 18115 | $^6H_{5/2}$ | 552 | $2.14 \times 10^{-5}$ |
| $(^4K,{}^4I)_{13/2}$ | 21406 | $^6H_{9/2}$ | 523 | $6.86 \times 10^{-6}$ | | | $^6H_{7/2}$ | 587 | $1.2 \times 10^{-6}$ |
| | | $^6H_{11/2}$ | 562 | $3.34 \times 10^{-8}$ | | | $^6H_{9/2}$ | 631 | $1.32 \times 10^{-4}$ |
| | | $^6H_{13/2}$ | 612 | $4.68 \times 10^{-5}$ | | | $^6F_{1/2}$ | 840 | $5.58 \times 10^{-5}$ |
| | | $^6H_{15/2}$ | 669 | $1.36 \times 10^{-7}$ | | | $^6F_{3/2}$ | 855 | $1.18 \times 10^{-5}$ |
| | | $^6F_{9/2}$ | 804 | $1.88 \times 10^{-6}$ | | | $^6F_{5/2}$ | 890 | $3.97 \times 10^{-5}$ |
| | | $^6F_{11/2}$ | 909 | $2.78 \times 10^{-7}$ | | | $^6F_{7/2}$ | 965 | $2.45 \times 10^{-7}$ |
| $^4M_{15/2}$ | 21181 | $^6H_{11/2}$ | 570 | $1.82 \times 10^{-6}$ | | | $^6F_{9/2}$ | 1093 | $1.19 \times 10^{-6}$ |
| | | $^6H_{13/2}$ | 621 | $7.75 \times 10^{-7}$ | $^6F_{11/2}$ | 10402 | $^6H_{7/2}$ | 1071 | $2.42 \times 10^{-8}$ |
| | | $^6H_{15/2}$ | 679 | $1.42 \times 10^{-5}$ | | | $^6H_{9/2}$ | 1230 | $5.6 \times 10^{-7}$ |
| | | $^6F_{11/2}$ | 928 | $6.58 \times 10^{-7}$ | | | $^6H_{11/2}$ | 1475 | $3.29 \times 10^{-6}$ |
| $^4I_{11/2}$ | 21107 | $^6H_{7/2}$ | 499 | $1.34 \times 10^{-5}$ | $^6F_{9/2}$ | 8964 | $^6H_{5/2}$ | 1116 | $5.03 \times 10^{-8}$ |
| | | $^6H_{9/2}$ | 531 | $1.11 \times 10^{-5}$ | | | $^6H_{7/2}$ | 1267 | $1.4 \times 10^{-6}$ |
| | | $^6H_{11/2}$ | 572 | $1.96 \times 10^{-5}$ | | | $^6H_{9/2}$ | 1495 | $7.48 \times 10^{-6}$ |
| | | $^6H_{13/2}$ | 623 | $2.15 \times 10^{-9}$ | $^6F_{7/2}$ | 7756 | $^6H_{5/2}$ | 1289 | $1.97 \times 10^{-6}$ |
| | | $^6H_{15/2}$ | 682 | $9.92 \times 10^{-9}$ | | | $^6H_{7/2}$ | 1496 | $1.15 \times 10^{-5}$ |
| | | $^6F_{7/2}$ | 749 | $1.95 \times 10^{-9}$ | $^6F_{5/2}$ | 6883 | $^6H_{5/2}$ | 1453 | $1.39 \times 10^{-5}$ |
| | | $^6F_{9/2}$ | 824 | $7.81 \times 10^{-8}$ | $^6F_{3/2}$ | 6416 | $^6H_{5/2}$ | 1559 | $2.9 \times 10^{-5}$ |
| | | $^6F_{11/2}$ | 934 | $2.17 \times 10^{-8}$ | $^6F_{1/2}$ | 6211 | $^6H_{5/2}$ | 1610 | $1.64 \times 10^{-5}$ |

[a] The emission rate, $A_{eq}$, inside a host material with refractive index $n_r$ would be: $A_{eq} = A'_{eq}\ n_r^5$

TABLE S19: Calculated $Eu^{3+}$ EQ spontaneous emission lines between 300 and 1700 nm.

| $SLJ$ | $E_{SLJ}(cm^{-1})$ | $S'L'J'$ | $\lambda$ (nm) | $A'_{eq}$ $(s^{-1})$ [a] | $SLJ$ | $E_{SLJ}(cm^{-1})$ | $S'L'J'$ | $\lambda$ (nm) | $A'_{eq}$ $(s^{-1})$ [a] |
|---|---|---|---|---|---|---|---|---|---|
| $({}^5D,{}^5P)_2$ | 39979 | ${}^5D_0$ | 445 | $1.67\times10^{-1}$ | ${}^5G_4$ | 39796 | ${}^5H_6$ | 1238 | $1.06\times10^{-5}$ |
| | | ${}^5D_1$ | 483 | $1.41\times10^{-2}$ | | | ${}^5H_5$ | 1248 | $7.41\times10^{-5}$ |
| | | ${}^5D_2$ | 549 | $2.25\times10^{-3}$ | | | ${}^5F_2$ | 1530 | $8.98\times10^{-6}$ |
| | | ${}^5D_3$ | 653 | $3.55\times10^{-5}$ | | | ${}^5F_3$ | 1539 | $4.08\times10^{-6}$ |
| | | ${}^5G_2$ | 738 | $3.42\times10^{-4}$ | | | ${}^5F_4$ | 1669 | $4.18\times10^{-6}$ |
| | | ${}^5G_3$ | 750 | $1.55\times10^{-6}$ | ${}^5G_3$ | 39296 | ${}^5D_1$ | 499 | $2.29\times10^{-4}$ |
| | | ${}^5G_4$ | 762 | $8.02\times10^{-6}$ | | | ${}^5D_2$ | 570 | $3.49\times10^{-3}$ |
| | | ${}^5D_4$ | 832 | $1.87\times10^{-5}$ | | | ${}^5D_3$ | 684 | $1.25\times10^{-9}$ |
| | | ${}^5H_3$ | 1182 | $6.77\times10^{-6}$ | | | ${}^5G_2$ | 777 | $9.82\times10^{-4}$ |
| | | ${}^5H_4$ | 1211 | $3.64\times10^{-6}$ | | | ${}^5G_3$ | 791 | $4.58\times10^{-4}$ |
| | | ${}^5F_2$ | 1489 | $9.94\times10^{-5}$ | | | ${}^5G_4$ | 803 | $4.6\times10^{-4}$ |
| | | ${}^5F_3$ | 1497 | $2.86\times10^{-5}$ | | | ${}^5G_5$ | 808 | $6.61\times10^{-6}$ |
| | | ${}^3P_0$ | 1558 | $2.36\times10^{-5}$ | | | ${}^5D_4$ | 882 | $3.4\times10^{-6}$ |
| | | ${}^5F_1$ | 1607 | $6.22\times10^{-5}$ | | | ${}^5H_3$ | 1285 | $6.54\times10^{-6}$ |
| | | ${}^5F_4$ | 1619 | $1.53\times10^{-7}$ | | | ${}^5H_4$ | 1320 | $2.41\times10^{-5}$ |
| $({}^3I,{}^3H)_6$ | 39890 | ${}^5L_6$ | 695 | $2.18\times10^{-4}$ | | | ${}^5H_5$ | 1331 | $2.21\times10^{-6}$ |
| | | ${}^5L_7$ | 733 | $6.85\times10^{-4}$ | | | ${}^5F_2$ | 1657 | $8.58\times10^{-6}$ |
| | | ${}^5G_4$ | 767 | $7.08\times10^{-5}$ | | | ${}^5F_3$ | 1667 | $3.13\times10^{-7}$ |
| | | ${}^5G_5$ | 771 | $1.04\times10^{-5}$ | ${}^5K_8$ | 39057 | ${}^5L_6$ | 738 | $1.45\times10^{-6}$ |
| | | ${}^5G_6$ | 776 | $7.69\times10^{-7}$ | | | ${}^5L_7$ | 781 | $1.38\times10^{-5}$ |
| | | ${}^5L_8$ | 778 | $8.61\times10^{-5}$ | | | ${}^5G_6$ | 830 | $1.72\times10^{-5}$ |
| | | ${}^5D_4$ | 838 | $9.39\times10^{-6}$ | | | ${}^5L_8$ | 832 | $3.93\times10^{-4}$ |
| | | ${}^5H_7$ | 1197 | $4.13\times10^{-6}$ | | | ${}^5L_9$ | 904 | $2.07\times10^{-3}$ |
| | | ${}^5H_4$ | 1224 | $1.88\times10^{-5}$ | | | ${}^5L_{10}$ | 960 | $5.5\times10^{-7}$ |
| | | ${}^5H_6$ | 1224 | $1.75\times10^{-6}$ | | | ${}^5H_7$ | 1330 | $6.5\times10^{-7}$ |
| | | ${}^5H_5$ | 1234 | $1.49\times10^{-5}$ | | | ${}^5H_6$ | 1363 | $4.82\times10^{-5}$ |
| | | ${}^5F_4$ | 1643 | $5.04\times10^{-7}$ | ${}^3P_1$ | 38891 | ${}^5D_1$ | 510 | $5.93\times10^{-6}$ |
| ${}^5K_9$ | 39879 | ${}^5L_7$ | 734 | $1.52\times10^{-6}$ | | | ${}^5D_2$ | 583 | $4.88\times10^{-11}$ |
| | | ${}^5L_8$ | 779 | $5.62\times10^{-6}$ | | | ${}^5D_3$ | 703 | $5.15\times10^{-6}$ |
| | | ${}^5L_9$ | 842 | $2.6\times10^{-4}$ | | | ${}^5G_2$ | 802 | $6.07\times10^{-6}$ |
| | | ${}^5L_{10}$ | 889 | $2.71\times10^{-3}$ | | | ${}^5G_3$ | 817 | $1.68\times10^{-6}$ |
| | | ${}^5H_7$ | 1199 | $1.33\times10^{-4}$ | | | ${}^5H_3$ | 1356 | $5.62\times10^{-8}$ |
| ${}^5G_4$ | 39796 | ${}^5D_2$ | 554 | $1.13\times10^{-3}$ | ${}^5G_2$ | 38784 | ${}^5D_0$ | 470 | $2.77\times10^{-4}$ |
| | | ${}^5D_3$ | 661 | $5.67\times10^{-4}$ | | | ${}^5D_1$ | 512 | $7.31\times10^{-3}$ |
| | | ${}^5L_6$ | 700 | $3.97\times10^{-5}$ | | | ${}^5D_2$ | 587 | $3.24\times10^{-5}$ |
| | | ${}^5G_2$ | 748 | $1.29\times10^{-4}$ | | | ${}^5D_3$ | 709 | $6.95\times10^{-6}$ |
| | | ${}^5G_3$ | 761 | $1.17\times10^{-3}$ | | | ${}^5G_2$ | 809 | $7.73\times10^{-4}$ |
| | | ${}^5G_4$ | 772 | $7.87\times10^{-4}$ | | | ${}^5G_3$ | 824 | $3.7\times10^{-4}$ |
| | | ${}^5G_5$ | 777 | $3.4\times10^{-4}$ | | | ${}^5G_4$ | 838 | $1.82\times10^{-5}$ |
| | | ${}^5G_6$ | 782 | $5.98\times10^{-6}$ | | | ${}^5D_4$ | 924 | $4.76\times10^{-7}$ |
| | | ${}^5D_4$ | 845 | $4.8\times10^{-6}$ | | | ${}^5H_3$ | 1376 | $1.22\times10^{-5}$ |
| | | ${}^5H_3$ | 1208 | $7.26\times10^{-9}$ | | | ${}^5H_4$ | 1416 | $1.54\times10^{-6}$ |
| | | ${}^5H_4$ | 1238 | $1.49\times10^{-5}$ | ${}^5K_7$ | 38468 | ${}^5L_6$ | 771 | $9.94\times10^{-6}$ |

[a] The emission rate, $A_{eq}$, inside a host material with refractive index $n_r$ would be: $A_{eq} = A'_{eq}\ n_r^5$

TABLE S19: Continued: $Eu^{3+}$ EQ spontaneous emission lines between 300 and 1700 nm.

| $SLJ$ | $E_{SLJ}(cm^{-1})$ | $S'L'J'$ | $\lambda$ (nm) | $A'_{eq}$ $(s^{-1})$ [a] | $SLJ$ | $E_{SLJ}(cm^{-1})$ | $S'L'J'$ | $\lambda$ (nm) | $A'_{eq}$ $(s^{-1})$ [a] |
|---|---|---|---|---|---|---|---|---|---|
| $^5K_7$ | 38468 | $^5L_7$ | 818 | $3.85 \times 10^{-4}$ | $(^5I,\, ^5H)_6$ | 34868 | $^7F_5$ | 324 | $3.1 \times 10^{-4}$ |
| | | $^5G_5$ | 866 | $5.99 \times 10^{-7}$ | | | $^7F_6$ | 335 | $4.87 \times 10^{-5}$ |
| | | $^5G_6$ | 872 | $1.05 \times 10^{-6}$ | | | $^5L_6$ | 1068 | $2.6 \times 10^{-5}$ |
| | | $^5L_8$ | 875 | $2.04 \times 10^{-3}$ | | | $^5L_7$ | 1160 | $1.04 \times 10^{-4}$ |
| | | $^5L_9$ | 955 | $7.63 \times 10^{-7}$ | | | $^5G_4$ | 1247 | $4.01 \times 10^{-5}$ |
| | | $^5H_7$ | 1443 | $1.06 \times 10^{-5}$ | | | $^5G_5$ | 1258 | $3.03 \times 10^{-8}$ |
| | | $^5H_6$ | 1482 | $2. \times 10^{-9}$ | | | $^5G_6$ | 1272 | $3.95 \times 10^{-7}$ |
| | | $^5H_5$ | 1496 | $2.29 \times 10^{-5}$ | | | $^5L_8$ | 1278 | $5.31 \times 10^{-5}$ |
| $^5K_6$ | 37516 | $^7F_6$ | 308 | $5.11 \times 10^{-7}$ | | | $^5D_4$ | 1448 | $5.47 \times 10^{-7}$ |
| | | $^5L_6$ | 832 | $1.82 \times 10^{-4}$ | $^5F_5$ | 34522 | $^7F_3$ | 307 | $7.28 \times 10^{-6}$ |
| | | $^5L_7$ | 888 | $1.52 \times 10^{-3}$ | | | $^7F_4$ | 317 | $1.74 \times 10^{-4}$ |
| | | $^5G_4$ | 937 | $2.19 \times 10^{-5}$ | | | $^7F_5$ | 328 | $4.18 \times 10^{-4}$ |
| | | $^5G_5$ | 944 | $1.46 \times 10^{-7}$ | | | $^7F_6$ | 339 | $1.67 \times 10^{-3}$ |
| | | $^5G_6$ | 951 | $1.58 \times 10^{-5}$ | | | $^5D_3$ | 1015 | $3.54 \times 10^{-5}$ |
| | | $^5L_8$ | 955 | $7.29 \times 10^{-6}$ | | | $^5L_6$ | 1108 | $2.99 \times 10^{-6}$ |
| | | $^5D_4$ | 1047 | $4.78 \times 10^{-7}$ | | | $^5L_7$ | 1209 | $1.88 \times 10^{-5}$ |
| | | $^5H_7$ | 1673 | $1.01 \times 10^{-10}$ | | | $^5G_3$ | 1271 | $4.6 \times 10^{-6}$ |
| $^5K_5$ | 36713 | $^7F_5$ | 306 | $2. \times 10^{-6}$ | | | $^5G_4$ | 1303 | $4.45 \times 10^{-9}$ |
| | | $^7F_6$ | 316 | $1.48 \times 10^{-7}$ | | | $^5G_5$ | 1316 | $1.56 \times 10^{-5}$ |
| | | $^5D_3$ | 831 | $2.57 \times 10^{-7}$ | | | $^5G_6$ | 1330 | $1.48 \times 10^{-4}$ |
| | | $^5L_6$ | 892 | $1.71 \times 10^{-3}$ | | | $^5D_4$ | 1524 | $5.79 \times 10^{-7}$ |
| | | $^5L_7$ | 956 | $6.07 \times 10^{-6}$ | $^5I_4$ | 34492 | $^7F_3$ | 307 | $6.6 \times 10^{-5}$ |
| | | $^5G_3$ | 994 | $1.76 \times 10^{-5}$ | | | $^7F_4$ | 317 | $3.41 \times 10^{-5}$ |
| | | $^5G_4$ | 1014 | $4.91 \times 10^{-7}$ | | | $^7F_5$ | 328 | $1.86 \times 10^{-6}$ |
| | | $^5G_5$ | 1021 | $2.59 \times 10^{-6}$ | | | $^7F_6$ | 340 | $2.2 \times 10^{-6}$ |
| | | $^5G_6$ | 1030 | $2.29 \times 10^{-5}$ | | | $^5D_2$ | 785 | $4.03 \times 10^{-6}$ |
| | | $^5D_4$ | 1143 | $7.9 \times 10^{-9}$ | | | $^5D_3$ | 1019 | $1.27 \times 10^{-7}$ |
| $(^5I,\, ^5H)_7$ | 35592 | $^7F_5$ | 317 | $5.95 \times 10^{-4}$ | | | $^5L_6$ | 1112 | $1.1 \times 10^{-4}$ |
| | | $^7F_6$ | 327 | $3.16 \times 10^{-4}$ | | | $^5G_2$ | 1239 | $4.78 \times 10^{-5}$ |
| | | $^5L_6$ | 991 | $1.18 \times 10^{-6}$ | | | $^5G_3$ | 1275 | $6.74 \times 10^{-7}$ |
| | | $^5L_7$ | 1070 | $3.25 \times 10^{-5}$ | | | $^5G_4$ | 1308 | $1.05 \times 10^{-7}$ |
| | | $^5G_5$ | 1153 | $9.02 \times 10^{-5}$ | | | $^5G_5$ | 1321 | $1.68 \times 10^{-6}$ |
| | | $^5G_6$ | 1164 | $5.64 \times 10^{-10}$ | | | $^5G_6$ | 1336 | $2.23 \times 10^{-6}$ |
| | | $^5L_8$ | 1170 | $8.03 \times 10^{-5}$ | | | $^5D_4$ | 1531 | $1.01 \times 10^{-8}$ |
| | | $^5L_9$ | 1317 | $5.95 \times 10^{-5}$ | $(^5I,\, ^5K)_5$ | 34361 | $^7F_3$ | 308 | $3.11 \times 10^{-4}$ |
| $^5I_8$ | 35313 | $^7F_6$ | 330 | $5.52 \times 10^{-4}$ | | | $^7F_4$ | 318 | $1.55 \times 10^{-4}$ |
| | | $^5L_6$ | 1019 | $4.45 \times 10^{-6}$ | | | $^7F_5$ | 329 | $4.15 \times 10^{-6}$ |
| | | $^5L_7$ | 1103 | $1.19 \times 10^{-7}$ | | | $^7F_6$ | 341 | $3.41 \times 10^{-4}$ |
| | | $^5G_6$ | 1204 | $1.04 \times 10^{-4}$ | | | $^5D_3$ | 1032 | $7.24 \times 10^{-6}$ |
| | | $^5L_8$ | 1209 | $7.14 \times 10^{-6}$ | | | $^5L_6$ | 1129 | $1.71 \times 10^{-4}$ |
| | | $^5L_9$ | 1367 | $1.66 \times 10^{-5}$ | | | $^5L_7$ | 1233 | $4.68 \times 10^{-5}$ |
| | | $^5L_{10}$ | 1498 | $4.87 \times 10^{-5}$ | | | $^5G_3$ | 1297 | $2.83 \times 10^{-5}$ |
| $(^5I,\, ^5H)_6$ | 34868 | $^7F_4$ | 313 | $4.08 \times 10^{-4}$ | | | $^5G_4$ | 1331 | $7.59 \times 10^{-9}$ |

[a] The emission rate, $A_{eq}$, inside a host material with refractive index $n_r$ would be: $A_{eq} = A'_{eq}\ n_r^5$

TABLE S19: Continued: $Eu^{3+}$ EQ spontaneous emission lines between 300 and 1700 nm.

| $SLJ$ | $E_{SLJ}(cm^{-1})$ | $S'L'J'$ | $\lambda$ (nm) | $A'_{eq}$ $(s^{-1})$ [a] | $SLJ$ | $E_{SLJ}(cm^{-1})$ | $S'L'J'$ | $\lambda$ (nm) | $A'_{eq}$ $(s^{-1})$ [a] |
|---|---|---|---|---|---|---|---|---|---|
| $\left({}^5I,\, {}^5K\right)_5$ | 34361 | ${}^5G_5$ | 1344 | $3.37 \times 10^{-6}$ | ${}^5F_2$ | 33261 | ${}^5D_0$ | 635 | $1.26 \times 10^{-2}$ |
| | | ${}^5G_6$ | 1359 | $1.16 \times 10^{-5}$ | | | ${}^5D_1$ | 714 | $3.49 \times 10^{-5}$ |
| | | ${}^5D_4$ | 1562 | $9.76 \times 10^{-8}$ | | | ${}^5D_2$ | 869 | $3.99 \times 10^{-5}$ |
| ${}^5F_4$ | 33804 | ${}^7F_2$ | 305 | $1.99 \times 10^{-4}$ | | | ${}^5D_3$ | 1165 | $2.38 \times 10^{-6}$ |
| | | ${}^7F_3$ | 314 | $2.05 \times 10^{-5}$ | | | ${}^5G_2$ | 1463 | $3.15 \times 10^{-5}$ |
| | | ${}^7F_4$ | 324 | $4.06 \times 10^{-4}$ | | | ${}^5G_3$ | 1513 | $2.22 \times 10^{-5}$ |
| | | ${}^7F_5$ | 336 | $3.53 \times 10^{-4}$ | | | ${}^5G_4$ | 1559 | $2.85 \times 10^{-6}$ |
| | | ${}^7F_6$ | 348 | $1.79 \times 10^{-4}$ | ${}^5H_5$ | 31785 | ${}^7F_3$ | 335 | $4.45 \times 10^{-4}$ |
| | | ${}^5D_2$ | 830 | $3.27 \times 10^{-4}$ | | | ${}^7F_4$ | 347 | $8.65 \times 10^{-4}$ |
| | | ${}^5D_3$ | 1095 | $7.29 \times 10^{-6}$ | | | ${}^7F_5$ | 360 | $1.67 \times 10^{-5}$ |
| | | ${}^5L_6$ | 1204 | $3.16 \times 10^{-7}$ | | | ${}^7F_6$ | 374 | $5.07 \times 10^{-6}$ |
| | | ${}^5G_2$ | 1355 | $7.55 \times 10^{-7}$ | | | ${}^5D_3$ | 1406 | $3.86 \times 10^{-8}$ |
| | | ${}^5G_3$ | 1398 | $3.78 \times 10^{-7}$ | | | ${}^5L_6$ | 1591 | $2.22 \times 10^{-6}$ |
| | | ${}^5G_4$ | 1438 | $2.01 \times 10^{-5}$ | ${}^5H_6$ | 31721 | ${}^7F_4$ | 347 | $2.3 \times 10^{-4}$ |
| | | ${}^5G_5$ | 1453 | $6.5 \times 10^{-5}$ | | | ${}^7F_5$ | 361 | $7.18 \times 10^{-4}$ |
| | | ${}^5G_6$ | 1471 | $2.67 \times 10^{-6}$ | | | ${}^7F_6$ | 375 | $7.65 \times 10^{-6}$ |
| ${}^5F_1$ | 33755 | ${}^7F_2$ | 306 | $1. \times 10^{-4}$ | | | ${}^5L_6$ | 1608 | $1.38 \times 10^{-6}$ |
| | | ${}^7F_3$ | 314 | $4.13 \times 10^{-6}$ | ${}^5H_4$ | 31721 | ${}^7F_2$ | 326 | $7.29 \times 10^{-4}$ |
| | | ${}^5D_1$ | 690 | $3.6 \times 10^{-4}$ | | | ${}^7F_3$ | 336 | $9.45 \times 10^{-4}$ |
| | | ${}^5D_2$ | 833 | $1.97 \times 10^{-5}$ | | | ${}^7F_4$ | 347 | $1.06 \times 10^{-4}$ |
| | | ${}^5D_3$ | 1101 | $3.31 \times 10^{-7}$ | | | ${}^7F_5$ | 361 | $1.21 \times 10^{-7}$ |
| | | ${}^5G_2$ | 1364 | $3.45 \times 10^{-5}$ | | | ${}^7F_6$ | 375 | $5.41 \times 10^{-7}$ |
| | | ${}^5G_3$ | 1408 | $4.26 \times 10^{-6}$ | | | ${}^5D_2$ | 1003 | $3.73 \times 10^{-10}$ |
| ${}^3P_0$ | 33559 | ${}^7F_2$ | 308 | $4.35 \times 10^{-5}$ | | | ${}^5D_3$ | 1419 | $2.85 \times 10^{-7}$ |
| | | ${}^5D_2$ | 847 | $1.29 \times 10^{-7}$ | | | ${}^5L_6$ | 1608 | $2.57 \times 10^{-6}$ |
| | | ${}^5G_2$ | 1401 | $3.62 \times 10^{-8}$ | ${}^5H_7$ | 31537 | ${}^7F_5$ | 363 | $9.59 \times 10^{-5}$ |
| ${}^5F_3$ | 33297 | ${}^7F_1$ | 304 | $1.49 \times 10^{-3}$ | | | ${}^7F_6$ | 377 | $4.31 \times 10^{-4}$ |
| | | ${}^7F_2$ | 310 | $2.41 \times 10^{-5}$ | | | ${}^5L_6$ | 1657 | $1.41 \times 10^{-10}$ |
| | | ${}^7F_3$ | 319 | $4.83 \times 10^{-4}$ | ${}^5H_3$ | 31517 | ${}^7F_1$ | 321 | $7.49 \times 10^{-4}$ |
| | | ${}^7F_4$ | 329 | $4.52 \times 10^{-5}$ | | | ${}^7F_2$ | 328 | $7.43 \times 10^{-4}$ |
| | | ${}^7F_5$ | 341 | $7.02 \times 10^{-5}$ | | | ${}^7F_3$ | 338 | $1.42 \times 10^{-4}$ |
| | | ${}^5D_1$ | 713 | $1.59 \times 10^{-3}$ | | | ${}^7F_4$ | 350 | $1.81 \times 10^{-6}$ |
| | | ${}^5D_2$ | 866 | $2.7 \times 10^{-5}$ | | | ${}^7F_5$ | 363 | $2.68 \times 10^{-7}$ |
| | | ${}^5D_3$ | 1160 | $4.22 \times 10^{-6}$ | | | ${}^5D_1$ | 816 | $8.72 \times 10^{-9}$ |
| | | ${}^5G_2$ | 1455 | $2.53 \times 10^{-6}$ | | | ${}^5D_2$ | 1024 | $1.55 \times 10^{-6}$ |
| | | ${}^5G_3$ | 1505 | $2.19 \times 10^{-5}$ | | | ${}^5D_3$ | 1462 | $1.51 \times 10^{-7}$ |
| | | ${}^5G_4$ | 1551 | $2.84 \times 10^{-5}$ | ${}^5D_4$ | 27961 | ${}^7F_2$ | 372 | $1.4 \times 10^{-4}$ |
| | | ${}^5G_5$ | 1569 | $2.71 \times 10^{-6}$ | | | ${}^7F_3$ | 384 | $3.47 \times 10^{-5}$ |
| ${}^5F_2$ | 33261 | ${}^7F_0$ | 301 | $1.5 \times 10^{-2}$ | | | ${}^7F_4$ | 399 | $1.03 \times 10^{-4}$ |
| | | ${}^7F_1$ | 304 | $3.52 \times 10^{-5}$ | | | ${}^7F_5$ | 417 | $3.77 \times 10^{-4}$ |
| | | ${}^7F_2$ | 311 | $7.19 \times 10^{-4}$ | | | ${}^7F_6$ | 436 | $5.82 \times 10^{-5}$ |
| | | ${}^7F_3$ | 319 | $4.82 \times 10^{-6}$ | | | ${}^5D_2$ | 1611 | $2.35 \times 10^{-6}$ |
| | | ${}^7F_4$ | 330 | $1.93 \times 10^{-5}$ | ${}^5L_8$ | 27043 | ${}^7F_6$ | 454 | $1.05 \times 10^{-6}$ |

[a] The emission rate, $A_{eq}$, inside a host material with refractive index $n_r$ would be: $A_{eq} = A'_{eq}\ n_r^5$

TABLE S19: Continued: $Eu^{3+}$ EQ spontaneous emission lines between 300 and 1700 nm.

| $SLJ$ | $E_{SLJ}(cm^{-1})$ | $S'L'J'$ | $\lambda$ (nm) | $A'_{eq}$ $(s^{-1})$ [a] | $SLJ$ | $E_{SLJ}(cm^{-1})$ | $S'L'J'$ | $\lambda$ (nm) | $A'_{eq}$ $(s^{-1})$ [a] |
|---|---|---|---|---|---|---|---|---|---|
| $^5G_6$ | 27005 | $^7F_4$ | 415 | $1.5 \times 10^{-5}$ | $^5G_2$ | 26423 | $^7F_4$ | 426 | $2.32 \times 10^{-7}$ |
| | | $^7F_5$ | 435 | $4.55 \times 10^{-5}$ | | | $^5D_0$ | 1123 | $6.12 \times 10^{-4}$ |
| | | $^7F_6$ | 455 | $5.06 \times 10^{-4}$ | | | $^5D_1$ | 1397 | $3.13 \times 10^{-5}$ |
| $^5G_5$ | 26922 | $^7F_3$ | 400 | $3.75 \times 10^{-6}$ | $^5L_7$ | 26250 | $^7F_5$ | 449 | $2.34 \times 10^{-8}$ |
| | | $^7F_4$ | 417 | $4.43 \times 10^{-5}$ | | | $^7F_6$ | 471 | $5.98 \times 10^{-7}$ |
| | | $^7F_5$ | 436 | $1.59 \times 10^{-4}$ | $^5L_6$ | 25501 | $^7F_4$ | 443 | $3.36 \times 10^{-7}$ |
| | | $^7F_6$ | 457 | $5.18 \times 10^{-5}$ | | | $^7F_5$ | 465 | $2.01 \times 10^{-7}$ |
| $^5G_4$ | 26848 | $^7F_2$ | 388 | $1.01 \times 10^{-5}$ | | | $^7F_6$ | 489 | $9.16 \times 10^{-6}$ |
| | | $^7F_3$ | 401 | $8.91 \times 10^{-5}$ | $^5D_3$ | 24675 | $^7F_1$ | 412 | $4.8 \times 10^{-4}$ |
| | | $^7F_4$ | 418 | $1.87 \times 10^{-5}$ | | | $^7F_2$ | 424 | $6.95 \times 10^{-5}$ |
| | | $^7F_5$ | 438 | $5.78 \times 10^{-5}$ | | | $^7F_3$ | 440 | $1.61 \times 10^{-4}$ |
| | | $^7F_6$ | 458 | $7.43 \times 10^{-8}$ | | | $^7F_4$ | 460 | $2.61 \times 10^{-4}$ |
| $^5G_3$ | 26652 | $^7F_1$ | 381 | $3.3 \times 10^{-4}$ | | | $^7F_5$ | 484 | $6.08 \times 10^{-6}$ |
| | | $^7F_2$ | 391 | $1.98 \times 10^{-4}$ | $^5D_2$ | 21752 | $^7F_0$ | 460 | $3.14 \times 10^{-3}$ |
| | | $^7F_3$ | 405 | $1.07 \times 10^{-7}$ | | | $^7F_1$ | 468 | $4.91 \times 10^{-5}$ |
| | | $^7F_4$ | 422 | $3.8 \times 10^{-6}$ | | | $^7F_2$ | 483 | $2.21 \times 10^{-4}$ |
| | | $^7F_5$ | 441 | $6.41 \times 10^{-7}$ | | | $^7F_3$ | 505 | $1.14 \times 10^{-4}$ |
| | | $^5D_1$ | 1354 | $4.18 \times 10^{-5}$ | | | $^7F_4$ | 531 | $4.57 \times 10^{-5}$ |
| $^5G_2$ | 26423 | $^7F_0$ | 378 | $4.92 \times 10^{-3}$ | $^5D_1$ | 19264 | $^7F_1$ | 530 | $3.22 \times 10^{-4}$ |
| | | $^7F_1$ | 384 | $7.87 \times 10^{-4}$ | | | $^7F_2$ | 550 | $2.89 \times 10^{-5}$ |
| | | $^7F_2$ | 394 | $5.31 \times 10^{-5}$ | | | $^7F_3$ | 577 | $5.45 \times 10^{-5}$ |
| | | $^7F_3$ | 408 | $3.31 \times 10^{-9}$ | $^5D_0$ | 17521 | $^7F_2$ | 608 | $2.28 \times 10^{-5}$ |

[a] The emission rate, $A_{eq}$, inside a host material with refractive index $n_r$ would be: $A_{eq} = A'_{eq}\ n_r^5$

TABLE S20: Calculated $Gd^{3+}$ EQ spontaneous emission lines between 300 and 1700 nm.

| $SLJ$ | $E_{SLJ}(cm^{-1})$ | $S'L'J'$ | $\lambda$ (nm) | $A'_{eq}$ $(s^{-1})$ [a] | $SLJ$ | $E_{SLJ}(cm^{-1})$ | $S'L'J'$ | $\lambda$ (nm) | $A'_{eq}$ $(s^{-1})$ [a] |
|---|---|---|---|---|---|---|---|---|---|
| $^6D_{9/2}$ | 39524 | $^6P_{7/2}$ | 1435 | $6.13 \times 10^{-5}$ | $^6P_{5/2}$ | 33169 | $^8S_{7/2}$ | 301 | $2.66 \times 10^{-4}$ |
| | | $^6P_{5/2}$ | 1574 | $7.45 \times 10^{-5}$ | $^6P_{7/2}$ | 32557 | $^8S_{7/2}$ | 307 | $7.9 \times 10^{-4}$ |

[a] The emission rate, $A_{eq}$, inside a host material with refractive index $n_r$ would be: $A_{eq} = A'_{eq}\ n_r^5$

TABLE S21: Calculated $Tb^{3+}$ EQ spontaneous emission lines between 300 and 1700 nm.

| $SLJ$ | $E_{SLJ}(cm^{-1})$ | $S'L'J'$ | $\lambda$ (nm) | $A'_{eq}$ $(s^{-1})$ [a] | $SLJ$ | $E_{SLJ}(cm^{-1})$ | $S'L'J'$ | $\lambda$ (nm) | $A'_{eq}$ $(s^{-1})$ [a] |
|---|---|---|---|---|---|---|---|---|---|
| $(^5D,\,^3P)_2$ | 39740 | $^5D_4$ | 530 | $1.52\times10^{-3}$ | $^5F_1$ | 37752 | $^5D_2$ | 1106 | $1.79\times10^{-8}$ |
| | | $^5D_3$ | 766 | $2.94\times10^{-6}$ | | | $^5G_3$ | 1182 | $4.58\times10^{-5}$ |
| | | $^5G_4$ | 904 | $2.87\times10^{-5}$ | | | $^5G_2$ | 1257 | $5.59\times10^{-5}$ |
| | | $^5D_2$ | 907 | $7.53\times10^{-5}$ | | | $^5D_1$ | 1526 | $6.12\times10^{-7}$ |
| | | $^5G_3$ | 957 | $1.14\times10^{-7}$ | $^5F_2$ | 37444 | $^7F_3$ | 301 | $4.56\times10^{-5}$ |
| | | $^5G_2$ | 1005 | $2.58\times10^{-6}$ | | | $^7F_2$ | 308 | $2.98\times10^{-4}$ |
| | | $^5D_1$ | 1171 | $1.59\times10^{-5}$ | | | $^7F_1$ | 313 | $5.54\times10^{-6}$ |
| | | $^5D_0$ | 1272 | $1.35\times10^{-6}$ | | | $^7F_0$ | 315 | $5.61\times10^{-3}$ |
| $^5K_9$ | 39358 | $^5L_{10}$ | 825 | $3.11\times10^{-3}$ | | | $^5D_4$ | 604 | $4.33\times10^{-5}$ |
| | | $^5L_9$ | 944 | $1.89\times10^{-4}$ | | | $^5D_3$ | 930 | $3.22\times10^{-7}$ |
| | | $^5L_8$ | 998 | $2.71\times10^{-6}$ | | | $^5G_4$ | 1140 | $7.33\times10^{-5}$ |
| | | $^5L_7$ | 1033 | $3.9\times10^{-6}$ | | | $^5D_2$ | 1145 | $8.99\times10^{-6}$ |
| | | $^5H_7$ | 1331 | $1.49\times10^{-5}$ | | | $^5G_3$ | 1227 | $1.66\times10^{-5}$ |
| $^5I_5$ | 38127 | $^5D_4$ | 580 | $1.36\times10^{-6}$ | | | $^5G_2$ | 1307 | $8.37\times10^{-5}$ |
| | | $^5D_3$ | 875 | $2.85\times10^{-6}$ | | | $^5D_1$ | 1602 | $1.19\times10^{-6}$ |
| | | $^5G_6$ | 899 | $8.71\times10^{-7}$ | $^5I_7$ | 36963 | $^5G_6$ | 1004 | $3.18\times10^{-5}$ |
| | | $^5G_5$ | 1013 | $4.4\times10^{-6}$ | | | $^5G_5$ | 1148 | $2.35\times10^{-5}$ |
| | | $^5G_4$ | 1058 | $6.08\times10^{-5}$ | | | $^5L_9$ | 1220 | $2.52\times10^{-5}$ |
| | | $^5G_3$ | 1132 | $9.56\times10^{-5}$ | | | $^5L_8$ | 1311 | $5.29\times10^{-5}$ |
| | | $^5L_7$ | 1184 | $2.03\times10^{-5}$ | | | $^5L_7$ | 1373 | $8.47\times10^{-6}$ |
| | | $^5L_6$ | 1237 | $6.36\times10^{-5}$ | | | $^5L_6$ | 1445 | $4.45\times10^{-7}$ |
| | | $^5H_7$ | 1591 | $5.52\times10^{-7}$ | $^5F_3$ | 36930 | $^7F_3$ | 306 | $4.88\times10^{-4}$ |
| $^5I_4$ | 37855 | $^7F_2$ | 304 | $1.22\times10^{-4}$ | | | $^7F_2$ | 313 | $1.04\times10^{-5}$ |
| | | $^5D_4$ | 589 | $8.03\times10^{-8}$ | | | $^7F_1$ | 318 | $1.3\times10^{-3}$ |
| | | $^5D_3$ | 896 | $3.81\times10^{-7}$ | | | $^5D_4$ | 623 | $1.09\times10^{-4}$ |
| | | $^5G_6$ | 922 | $1.31\times10^{-6}$ | | | $^5D_3$ | 977 | $9.35\times10^{-6}$ |
| | | $^5G_5$ | 1041 | $6.45\times10^{-10}$ | | | $^5G_5$ | 1152 | $7.1\times10^{-5}$ |
| | | $^5G_4$ | 1089 | $2.2\times10^{-6}$ | | | $^5G_4$ | 1211 | $1.26\times10^{-5}$ |
| | | $^5D_2$ | 1094 | $1.64\times10^{-6}$ | | | $^5D_2$ | 1217 | $2.32\times10^{-6}$ |
| | | $^5G_3$ | 1168 | $2.34\times10^{-5}$ | | | $^5G_3$ | 1310 | $6.28\times10^{-5}$ |
| | | $^5G_2$ | 1241 | $1.08\times10^{-4}$ | | | $^5G_2$ | 1401 | $2.67\times10^{-5}$ |
| | | $^5L_6$ | 1280 | $3.73\times10^{-5}$ | $^5F_4$ | 35884 | $^7F_4$ | 306 | $1.26\times10^{-3}$ |
| $^5I_6$ | 37759 | $^5D_4$ | 593 | $3.83\times10^{-6}$ | | | $^7F_3$ | 316 | $9.92\times10^{-7}$ |
| | | $^5G_6$ | 930 | $1.46\times10^{-5}$ | | | $^7F_2$ | 323 | $3.24\times10^{-4}$ |
| | | $^5G_5$ | 1052 | $5.2\times10^{-5}$ | | | $^5D_4$ | 667 | $1.69\times10^{-4}$ |
| | | $^5G_4$ | 1101 | $5.84\times10^{-5}$ | | | $^5D_3$ | 1088 | $1.63\times10^{-5}$ |
| | | $^5L_8$ | 1187 | $1.5\times10^{-5}$ | | | $^5G_6$ | 1126 | $6.9\times10^{-5}$ |
| | | $^5L_7$ | 1238 | $6.26\times10^{-5}$ | | | $^5G_5$ | 1310 | $1.16\times10^{-5}$ |
| | | $^5L_6$ | 1296 | $1.06\times10^{-5}$ | | | $^5G_4$ | 1387 | $4.35\times10^{-5}$ |
| | | $^5H_7$ | 1690 | $1.6\times10^{-6}$ | | | $^5D_2$ | 1394 | $5.76\times10^{-6}$ |
| $^5F_1$ | 37752 | $^7F_2$ | 305 | $6.85\times10^{-5}$ | | | $^5G_3$ | 1518 | $1.52\times10^{-5}$ |
| | | $^7F_1$ | 310 | $3.95\times10^{-4}$ | | | $^5G_2$ | 1642 | $1.53\times10^{-6}$ |
| | | $^5D_3$ | 904 | $1.69\times10^{-8}$ | $^5I_8$ | 35528 | $^5G_6$ | 1173 | $1.18\times10^{-5}$ |

[a] The emission rate, $A_{eq}$, inside a host material with refractive index $n_r$ would be: $A_{eq} = A'_{eq}\ n_r^5$

TABLE S21: Continued: $Tb^{3+}$ EQ spontaneous emission lines between 300 and 1700 nm.

| $SLJ$ | $E_{SLJ}(cm^{-1})$ | $S'L'J'$ | $\lambda$ (nm) | $A'_{eq}$ $(s^{-1})$ [a] | $SLJ$ | $E_{SLJ}(cm^{-1})$ | $S'L'J'$ | $\lambda$ (nm) | $A'_{eq}$ $(s^{-1})$ [a] |
|---|---|---|---|---|---|---|---|---|---|
| $^5I_8$ | 35528 | $^5L_{10}$ | 1207 | $4.78 \times 10^{-5}$ | $^5D_0$ | 31877 | $^7F_2$ | 372 | $8.2 \times 10^{-5}$ |
| | | $^5L_9$ | 1479 | $3.12 \times 10^{-5}$ | $^5H_7$ | 31843 | $^7F_6$ | 314 | $1.95 \times 10^{-3}$ |
| | | $^5L_8$ | 1614 | $2.54 \times 10^{-6}$ | | | $^7F_5$ | 335 | $8.33 \times 10^{-4}$ |
| $^5H_3$ | 35510 | $^7F_4$ | 310 | $5. \times 10^{-5}$ | $^5D_1$ | 31200 | $^7F_3$ | 371 | $1.61 \times 10^{-4}$ |
| | | $^7F_3$ | 320 | $1.54 \times 10^{-4}$ | | | $^7F_2$ | 381 | $1.47 \times 10^{-4}$ |
| | | $^7F_2$ | 327 | $2.41 \times 10^{-4}$ | | | $^7F_1$ | 388 | $6.85 \times 10^{-4}$ |
| | | $^7F_1$ | 333 | $2.28 \times 10^{-4}$ | $^5L_6$ | 30042 | $^7F_6$ | 333 | $3.28 \times 10^{-5}$ |
| | | $^5D_4$ | 684 | $8.46 \times 10^{-8}$ | | | $^7F_5$ | 357 | $9.56 \times 10^{-7}$ |
| | | $^5D_3$ | 1134 | $1.31 \times 10^{-7}$ | | | $^7F_4$ | 373 | $2.35 \times 10^{-6}$ |
| | | $^5G_5$ | 1378 | $1.96 \times 10^{-7}$ | | | $^5D_4$ | 1092 | $2.54 \times 10^{-6}$ |
| | | $^5G_4$ | 1463 | $9.67 \times 10^{-7}$ | $^5G_2$ | 29794 | $^7F_4$ | 377 | $2.83 \times 10^{-6}$ |
| | | $^5D_2$ | 1471 | $1.91 \times 10^{-7}$ | | | $^7F_3$ | 391 | $4.67 \times 10^{-6}$ |
| | | $^5G_3$ | 1609 | $1.78 \times 10^{-7}$ | | | $^7F_2$ | 403 | $2.39 \times 10^{-7}$ |
| $^5F_5$ | 35441 | $^7F_4$ | 311 | $3.83 \times 10^{-7}$ | | | $^7F_1$ | 411 | $1.47 \times 10^{-4}$ |
| | | $^7F_3$ | 321 | $1.28 \times 10^{-4}$ | | | $^7F_0$ | 415 | $2.37 \times 10^{-3}$ |
| | | $^5D_4$ | 687 | $4.91 \times 10^{-4}$ | | | $^5D_4$ | 1122 | $2.48 \times 10^{-7}$ |
| | | $^5D_3$ | 1143 | $1.85 \times 10^{-6}$ | $^5L_7$ | 29678 | $^7F_6$ | 337 | $1.41 \times 10^{-4}$ |
| | | $^5G_6$ | 1185 | $7.38 \times 10^{-5}$ | | | $^7F_5$ | 361 | $6.12 \times 10^{-5}$ |
| | | $^5G_5$ | 1391 | $4.08 \times 10^{-5}$ | $^5L_8$ | 29334 | $^7F_6$ | 341 | $2.19 \times 10^{-6}$ |
| | | $^5G_4$ | 1478 | $6.65 \times 10^{-6}$ | $^5G_3$ | 29295 | $^7F_5$ | 366 | $9.58 \times 10^{-6}$ |
| | | $^5G_3$ | 1627 | $1.12 \times 10^{-6}$ | | | $^7F_4$ | 384 | $3.12 \times 10^{-5}$ |
| $^5H_4$ | 34845 | $^7F_5$ | 304 | $1.3 \times 10^{-4}$ | | | $^7F_3$ | 399 | $3.87 \times 10^{-9}$ |
| | | $^7F_4$ | 316 | $2.57 \times 10^{-4}$ | | | $^7F_2$ | 411 | $2.92 \times 10^{-4}$ |
| | | $^7F_3$ | 327 | $3.08 \times 10^{-4}$ | | | $^7F_1$ | 419 | $8.2 \times 10^{-4}$ |
| | | $^7F_2$ | 335 | $1.98 \times 10^{-4}$ | | | $^5D_4$ | 1189 | $5.34 \times 10^{-7}$ |
| | | $^5D_4$ | 716 | $5.12 \times 10^{-8}$ | $^5D_2$ | 28712 | $^7F_4$ | 393 | $6.7 \times 10^{-5}$ |
| | | $^5D_3$ | 1227 | $2.34 \times 10^{-7}$ | | | $^7F_3$ | 409 | $3.1 \times 10^{-4}$ |
| | | $^5G_6$ | 1275 | $2.68 \times 10^{-7}$ | | | $^7F_2$ | 421 | $1.81 \times 10^{-4}$ |
| | | $^5G_5$ | 1517 | $6.57 \times 10^{-7}$ | | | $^7F_1$ | 430 | $2.78 \times 10^{-4}$ |
| | | $^5G_4$ | 1620 | $2.64 \times 10^{-7}$ | | | $^7F_0$ | 435 | $3.83 \times 10^{-3}$ |
| | | $^5D_2$ | 1631 | $5.3 \times 10^{-8}$ | | | $^5D_4$ | 1277 | $6.92 \times 10^{-6}$ |
| $^5H_5$ | 34182 | $^7F_5$ | 311 | $4.95 \times 10^{-4}$ | $^5G_4$ | 28673 | $^7F_6$ | 349 | $1.61 \times 10^{-5}$ |
| | | $^7F_4$ | 323 | $5.53 \times 10^{-4}$ | | | $^7F_5$ | 375 | $8.13 \times 10^{-5}$ |
| | | $^7F_3$ | 334 | $3.08 \times 10^{-4}$ | | | $^7F_4$ | 393 | $4.48 \times 10^{-6}$ |
| | | $^5D_4$ | 752 | $1.92 \times 10^{-9}$ | | | $^7F_3$ | 409 | $4.52 \times 10^{-4}$ |
| | | $^5D_3$ | 1335 | $9.77 \times 10^{-7}$ | | | $^7F_2$ | 422 | $5.63 \times 10^{-4}$ |
| | | $^5G_6$ | 1393 | $9.23 \times 10^{-7}$ | | | $^5D_4$ | 1283 | $1.37 \times 10^{-7}$ |
| | | $^5G_5$ | 1686 | $1.6 \times 10^{-7}$ | $^5G_5$ | 28252 | $^7F_6$ | 354 | $1.74 \times 10^{-4}$ |
| $^5H_6$ | 33279 | $^7F_6$ | 300 | $9.13 \times 10^{-4}$ | | | $^7F_5$ | 381 | $3.1 \times 10^{-5}$ |
| | | $^7F_5$ | 320 | $1.05 \times 10^{-3}$ | | | $^7F_4$ | 400 | $5.93 \times 10^{-4}$ |
| | | $^7F_4$ | 333 | $5.96 \times 10^{-4}$ | | | $^7F_3$ | 417 | $4.76 \times 10^{-4}$ |
| | | $^5D_4$ | 807 | $8.81 \times 10^{-6}$ | | | $^5D_4$ | 1357 | $1.65 \times 10^{-6}$ |
| | | $^5G_6$ | 1594 | $1.4 \times 10^{-7}$ | $^5G_6$ | 27004 | $^7F_6$ | 370 | $2.52 \times 10^{-4}$ |

[a] The emission rate, $A_{eq}$, inside a host material with refractive index $n_r$ would be: $A_{eq} = A'_{eq}\ n_r^5$

TABLE S21: Continued: $Tb^{3+}$ EQ spontaneous emission lines between 300 and 1700 nm.

| $SLJ$ | $E_{SLJ}(cm^{-1})$ | $S'L'J'$ | $\lambda$ (nm) | $A'_{eq}$ $(s^{-1})$ [a] | $SLJ$ | $E_{SLJ}(cm^{-1})$ | $S'L'J'$ | $\lambda$ (nm) | $A'_{eq}$ $(s^{-1})$ [a] |
|---|---|---|---|---|---|---|---|---|---|
| $^5G_6$ | 27004 | $^7F_5$ | 400 | $4.02 \times 10^{-4}$ | $^5D_3$ | 26693 | $^7F_1$ | 471 | $4.95 \times 10^{-4}$ |
| | | $^7F_4$ | 421 | $3.81 \times 10^{-4}$ | $^5D_4$ | 20881 | $^7F_6$ | 479 | $2.38 \times 10^{-5}$ |
| | | $^5D_4$ | 1633 | $1.78 \times 10^{-5}$ | | | $^7F_5$ | 530 | $2.96 \times 10^{-4}$ |
| $^5D_3$ | 26693 | $^7F_5$ | 405 | $3.45 \times 10^{-5}$ | | | $^7F_4$ | 567 | $5.55 \times 10^{-6}$ |
| | | $^7F_4$ | 427 | $4.64 \times 10^{-4}$ | | | $^7F_3$ | 601 | $6.70 \times 10^{-5}$ |
| | | $^7F_3$ | 446 | $7.37 \times 10^{-5}$ | | | $^7F_2$ | 628 | $5.43 \times 10^{-5}$ |
| | | $^7F_2$ | 460 | $2.35 \times 10^{-4}$ | | | | | |

[a] The emission rate, $A_{eq}$, inside a host material with refractive index $n_r$ would be: $A_{eq} = A'_{eq}\ n_r^5$

TABLE S22: Calculated $Dy^{3+}$ EQ spontaneous emission lines between 300 and 1700 nm.

| $SLJ$ | $E_{SLJ}(cm^{-1})$ | $S'L'J'$ | $\lambda$ (nm) | $A'_{eq}$ $(s^{-1})$ [a] | $SLJ$ | $E_{SLJ}(cm^{-1})$ | $S'L'J'$ | $\lambda$ (nm) | $A'_{eq}$ $(s^{-1})$ [a] |
|---|---|---|---|---|---|---|---|---|---|
| $({}^4G,\,{}^4P)_{5/2}$ | 38873 | ${}^6H_{9/2}$ | 318 | $4.94\times10^{-5}$ | $({}^2K,\,{}^2L)_{15/2}$ | 38434 | ${}^4M_{15/2}$ | 1124 | $3.89\times10^{-5}$ |
| | | ${}^6F_{9/2}$ | 333 | $3.78\times10^{-3}$ | | | ${}^4M_{17/2}$ | 1150 | $5.22\times10^{-6}$ |
| | | ${}^6H_{7/2}$ | 334 | $6.1\times10^{-5}$ | | | ${}^4K_{15/2}$ | 1318 | $2.7\times10^{-6}$ |
| | | ${}^6H_{5/2}$ | 348 | $2.91\times10^{-6}$ | | | ${}^4L_{19/2}$ | 1326 | $1.51\times10^{-8}$ |
| | | ${}^6F_{7/2}$ | 355 | $3.81\times10^{-3}$ | ${}^4H_{7/2}$ | 37877 | ${}^6H_{11/2}$ | 310 | $6.\times10^{-5}$ |
| | | ${}^6F_{5/2}$ | 374 | $1.08\times10^{-3}$ | | | ${}^6F_{11/2}$ | 328 | $8.44\times10^{-7}$ |
| | | ${}^6F_{3/2}$ | 385 | $2.03\times10^{-3}$ | | | ${}^6H_{9/2}$ | 329 | $1.3\times10^{-6}$ |
| | | ${}^6F_{1/2}$ | 393 | $2.08\times10^{-3}$ | | | ${}^6F_{9/2}$ | 345 | $1.52\times10^{-4}$ |
| | | ${}^4F_{9/2}$ | 561 | $2.26\times10^{-4}$ | | | ${}^6H_{7/2}$ | 345 | $3.52\times10^{-4}$ |
| | | ${}^4F_{7/2}$ | 754 | $1.46\times10^{-4}$ | | | ${}^6H_{5/2}$ | 360 | $7.93\times10^{-4}$ |
| | | ${}^6P_{5/2}$ | 820 | $3.96\times10^{-5}$ | | | ${}^6F_{7/2}$ | 368 | $3.32\times10^{-6}$ |
| | | $({}^4P,\,{}^6P)_{3/2}$ | 835 | $3.21\times10^{-5}$ | | | ${}^6F_{5/2}$ | 388 | $3.01\times10^{-6}$ |
| | | ${}^6P_{7/2}$ | 896 | $6.4\times10^{-9}$ | | | ${}^6F_{3/2}$ | 400 | $2.45\times10^{-7}$ |
| | | $({}^4F,\,{}^4D)_{5/2}$ | 1064 | $2.05\times10^{-5}$ | | | ${}^4F_{9/2}$ | 594 | $3.77\times10^{-5}$ |
| | | ${}^4G_{9/2}$ | 1133 | $3.05\times10^{-5}$ | | | ${}^4G_{11/2}$ | 700 | $2.05\times10^{-6}$ |
| | | ${}^6P_{3/2}$ | 1146 | $9.15\times10^{-6}$ | | | ${}^4F_{7/2}$ | 815 | $2.61\times10^{-6}$ |
| | | ${}^4I_{9/2}$ | 1231 | $1.13\times10^{-5}$ | | | ${}^6P_{5/2}$ | 893 | $7.61\times10^{-7}$ |
| | | $({}^4G,\,{}^4F)_{7/2}$ | 1366 | $2.37\times10^{-7}$ | | | $({}^4P,\,{}^6P)_{3/2}$ | 911 | $3.28\times10^{-5}$ |
| | | $({}^4D,\,{}^4P)_{1/2}$ | 1408 | $4.69\times10^{-5}$ | | | ${}^6P_{7/2}$ | 983 | $2.61\times10^{-7}$ |
| | | $({}^4D,\,{}^4G)_{5/2}$ | 1442 | $1.42\times10^{-6}$ | | | ${}^4I_{11/2}$ | 1074 | $1.65\times10^{-4}$ |
| $({}^4P,\,{}^4D)_{3/2}$ | 38691 | ${}^6H_{7/2}$ | 336 | $6.47\times10^{-6}$ | | | $({}^4F,\,{}^4D)_{5/2}$ | 1191 | $3.39\times10^{-5}$ |
| | | ${}^6H_{5/2}$ | 350 | $6.19\times10^{-5}$ | | | ${}^4G_{9/2}$ | 1277 | $1.28\times10^{-5}$ |
| | | ${}^6F_{7/2}$ | 357 | $1.75\times10^{-3}$ | | | ${}^6P_{3/2}$ | 1293 | $3.65\times10^{-6}$ |
| | | ${}^6F_{5/2}$ | 376 | $4.1\times10^{-3}$ | | | ${}^4I_{9/2}$ | 1403 | $1.03\times10^{-5}$ |
| | | ${}^6F_{3/2}$ | 388 | $3.15\times10^{-3}$ | | | $({}^4G,\,{}^4F)_{7/2}$ | 1581 | $3.49\times10^{-6}$ |
| | | ${}^6F_{1/2}$ | 396 | $9.74\times10^{-3}$ | | | $({}^4D,\,{}^4G)_{5/2}$ | 1683 | $1.37\times10^{-5}$ |
| | | ${}^4F_{7/2}$ | 764 | $5.28\times10^{-6}$ | ${}^4F_{3/2}$ | 37277 | ${}^6H_{7/2}$ | 353 | $2.73\times10^{-6}$ |
| | | ${}^6P_{5/2}$ | 833 | $9.98\times10^{-8}$ | | | ${}^6H_{5/2}$ | 368 | $1.13\times10^{-5}$ |
| | | $({}^4P,\,{}^6P)_{3/2}$ | 848 | $2.06\times10^{-4}$ | | | ${}^6F_{7/2}$ | 376 | $3.56\times10^{-4}$ |
| | | ${}^6P_{7/2}$ | 910 | $3.84\times10^{-5}$ | | | ${}^6F_{5/2}$ | 397 | $4.64\times10^{-4}$ |
| | | $({}^4F,\,{}^4D)_{5/2}$ | 1085 | $2.12\times10^{-6}$ | | | ${}^6F_{3/2}$ | 410 | $4.65\times10^{-3}$ |
| | | ${}^6P_{3/2}$ | 1170 | $7.26\times10^{-5}$ | | | ${}^6F_{1/2}$ | 419 | $1.41\times10^{-5}$ |
| | | $({}^4G,\,{}^4F)_{7/2}$ | 1401 | $4.03\times10^{-6}$ | | | ${}^4F_{7/2}$ | 857 | $1.23\times10^{-5}$ |
| | | $({}^4D,\,{}^4P)_{1/2}$ | 1445 | $6.7\times10^{-6}$ | | | ${}^6P_{5/2}$ | 944 | $6.69\times10^{-8}$ |
| | | $({}^4D,\,{}^4G)_{5/2}$ | 1480 | $1.27\times10^{-6}$ | | | $({}^4P,\,{}^6P)_{3/2}$ | 964 | $4.3\times10^{-5}$ |
| $({}^2K,\,{}^2L)_{15/2}$ | 38434 | ${}^6H_{11/2}$ | 305 | $7.02\times10^{-5}$ | | | ${}^6P_{7/2}$ | 1045 | $1.\times10^{-5}$ |
| | | ${}^6F_{11/2}$ | 323 | $9.58\times10^{-6}$ | | | $({}^4F,\,{}^4D)_{5/2}$ | 1282 | $3.97\times10^{-6}$ |
| | | ${}^4I_{15/2}$ | 635 | $6.71\times10^{-5}$ | | | ${}^6P_{3/2}$ | 1402 | $2.52\times10^{-6}$ |
| | | ${}^4G_{11/2}$ | 674 | $2.27\times10^{-5}$ | ${}^4P_{1/2}$ | 37189 | ${}^6H_{5/2}$ | 369 | $3.27\times10^{-5}$ |
| | | ${}^4K_{17/2}$ | 802 | $4.76\times10^{-5}$ | | | ${}^6F_{5/2}$ | 399 | $3.73\times10^{-5}$ |
| | | ${}^4I_{13/2}$ | 808 | $1.28\times10^{-7}$ | | | ${}^6F_{3/2}$ | 412 | $2.23\times10^{-4}$ |
| | | ${}^4M_{19/2}$ | 862 | $6.54\times10^{-6}$ | | | ${}^6P_{5/2}$ | 952 | $7.79\times10^{-6}$ |
| | | ${}^4I_{11/2}$ | 1014 | $5.95\times10^{-6}$ | | | $({}^4P,\,{}^6P)_{3/2}$ | 972 | $1.64\times10^{-6}$ |

[a] The emission rate, $A_{eq}$, inside a host material with refractive index $n_r$ would be: $A_{eq} = A'_{eq}\ n_r^5$

TABLE S22: Continued: $Dy^{3+}$ EQ spontaneous emission lines between 300 and 1700 nm.

| $SLJ$ | $E_{SLJ}(cm^{-1})$ | $S'L'J'$ | $\lambda$ (nm) | $A'_{eq}$ $(s^{-1})$ [a] | $SLJ$ | $E_{SLJ}(cm^{-1})$ | $S'L'J'$ | $\lambda$ (nm) | $A'_{eq}$ $(s^{-1})$ [a] |
|---|---|---|---|---|---|---|---|---|---|
| $^4P_{1/2}$ | 37189 | $(^4F,\,^4D)_{5/2}$ | 1297 | $5.48\times10^{-6}$ | $(^4H,\,^4G)_{9/2}$ | 36463 | $^4F_{7/2}$ | 921 | $1.24\times10^{-4}$ |
| | | $^6P_{3/2}$ | 1419 | $6.51\times10^{-7}$ | | | $^4I_{13/2}$ | 960 | $4.29\times10^{-4}$ |
| $^4L_{13/2}$ | 36666 | $^6H_{11/2}$ | 322 | $8.36\times10^{-5}$ | | | $^6P_{5/2}$ | 1023 | $3.\times10^{-6}$ |
| | | $^6F_{11/2}$ | 342 | $4.88\times10^{-7}$ | | | $^6P_{7/2}$ | 1142 | $1.08\times10^{-5}$ |
| | | $^6H_{9/2}$ | 342 | $1.78\times10^{-4}$ | | | $^4I_{11/2}$ | 1267 | $4.76\times10^{-6}$ |
| | | $^6F_{9/2}$ | 360 | $3.47\times10^{-6}$ | | | $(^4F,\,^4D)_{5/2}$ | 1432 | $7.32\times10^{-9}$ |
| | | $^4F_{9/2}$ | 640 | $6.84\times10^{-6}$ | | | $^4G_{9/2}$ | 1558 | $2.49\times10^{-6}$ |
| | | $^4I_{15/2}$ | 716 | $5.04\times10^{-5}$ | $^4G_{7/2}$ | 36281 | $^6H_{11/2}$ | 326 | $3.09\times10^{-5}$ |
| | | $^4G_{11/2}$ | 765 | $3.06\times10^{-6}$ | | | $^6F_{11/2}$ | 347 | $9.06\times10^{-4}$ |
| | | $^4K_{17/2}$ | 935 | $1.44\times10^{-5}$ | | | $^6H_{9/2}$ | 347 | $6.25\times10^{-5}$ |
| | | $^4I_{13/2}$ | 942 | $7.11\times10^{-8}$ | | | $^6F_{9/2}$ | 365 | $5.69\times10^{-4}$ |
| | | $^4I_{11/2}$ | 1235 | $8.53\times10^{-6}$ | | | $^6H_{7/2}$ | 366 | $2.09\times10^{-4}$ |
| | | $^4M_{15/2}$ | 1402 | $2.23\times10^{-5}$ | | | $^6H_{5/2}$ | 382 | $4.01\times10^{-6}$ |
| | | $^4M_{17/2}$ | 1444 | $4.98\times10^{-6}$ | | | $^6F_{7/2}$ | 391 | $2.97\times10^{-4}$ |
| | | $^4G_{9/2}$ | 1510 | $6.34\times10^{-7}$ | | | $^6F_{5/2}$ | 414 | $6.46\times10^{-5}$ |
| | | $^4I_{9/2}$ | 1690 | $1.36\times10^{-5}$ | | | $^6F_{3/2}$ | 428 | $2.71\times10^{-5}$ |
| $(^4G,\,^4P)_{5/2}$ | 36489 | $^6H_{9/2}$ | 344 | $3.25\times10^{-6}$ | | | $^4F_{9/2}$ | 656 | $6.89\times10^{-6}$ |
| | | $^6F_{9/2}$ | 362 | $3.3\times10^{-3}$ | | | $^4G_{11/2}$ | 788 | $5.4\times10^{-6}$ |
| | | $^6H_{7/2}$ | 363 | $7.1\times10^{-5}$ | | | $^4F_{7/2}$ | 937 | $3.07\times10^{-5}$ |
| | | $^6H_{5/2}$ | 379 | $1.44\times10^{-4}$ | | | $^6P_{5/2}$ | 1042 | $4.39\times10^{-9}$ |
| | | $^6F_{7/2}$ | 388 | $4.26\times10^{-3}$ | | | $(^4P,\,^6P)_{3/2}$ | 1066 | $6.09\times10^{-5}$ |
| | | $^6F_{5/2}$ | 410 | $3.77\times10^{-3}$ | | | $^6P_{7/2}$ | 1166 | $4.64\times10^{-6}$ |
| | | $^6F_{3/2}$ | 424 | $6.84\times10^{-4}$ | | | $^4I_{11/2}$ | 1297 | $1.42\times10^{-5}$ |
| | | $^6F_{1/2}$ | 433 | $7.14\times10^{-4}$ | | | $(^4F,\,^4D)_{5/2}$ | 1470 | $2.76\times10^{-6}$ |
| | | $^4F_{9/2}$ | 648 | $5.58\times10^{-4}$ | | | $^4G_{9/2}$ | 1603 | $4.2\times10^{-6}$ |
| | | $^4F_{7/2}$ | 919 | $9.87\times10^{-7}$ | | | $^6P_{3/2}$ | 1629 | $4.58\times10^{-6}$ |
| | | $^6P_{5/2}$ | 1020 | $3.96\times10^{-6}$ | $^4L_{15/2}$ | 36261 | $^6H_{13/2}$ | 304 | $2.14\times10^{-4}$ |
| | | $(^4P,\,^6P)_{3/2}$ | 1043 | $1.52\times10^{-4}$ | | | $^6H_{11/2}$ | 326 | $4.63\times10^{-5}$ |
| | | $^6P_{7/2}$ | 1139 | $5.36\times10^{-6}$ | | | $^6F_{11/2}$ | 347 | $1.57\times10^{-7}$ |
| | | $(^4F,\,^4D)_{5/2}$ | 1426 | $1.04\times10^{-5}$ | | | $^4I_{15/2}$ | 737 | $1.17\times10^{-5}$ |
| | | $^4G_{9/2}$ | 1552 | $1.71\times10^{-7}$ | | | $^4G_{11/2}$ | 789 | $3.31\times10^{-7}$ |
| | | $^6P_{3/2}$ | 1576 | $7.03\times10^{-6}$ | | | $^4K_{17/2}$ | 971 | $2.07\times10^{-5}$ |
| $(^4H,\,^4G)_{9/2}$ | 36463 | $^6H_{13/2}$ | 302 | $2.85\times10^{-4}$ | | | $^4I_{13/2}$ | 979 | $4.13\times10^{-5}$ |
| | | $^6H_{11/2}$ | 324 | $2.44\times10^{-5}$ | | | $^4M_{19/2}$ | 1061 | $1.3\times10^{-5}$ |
| | | $^6F_{11/2}$ | 344 | $9.04\times10^{-5}$ | | | $^4I_{11/2}$ | 1300 | $1.15\times10^{-5}$ |
| | | $^6H_{9/2}$ | 345 | $2.73\times10^{-4}$ | | | $^4M_{15/2}$ | 1487 | $3.63\times10^{-6}$ |
| | | $^6F_{9/2}$ | 362 | $8.37\times10^{-5}$ | | | $^4M_{17/2}$ | 1534 | $2.92\times10^{-5}$ |
| | | $^6H_{7/2}$ | 363 | $4.03\times10^{-4}$ | $^4K_{11/2}$ | 35631 | $^6H_{13/2}$ | 309 | $7.33\times10^{-5}$ |
| | | $^6H_{5/2}$ | 380 | $7.53\times10^{-5}$ | | | $^6H_{11/2}$ | 333 | $2.62\times10^{-4}$ |
| | | $^6F_{7/2}$ | 388 | $9.4\times10^{-5}$ | | | $^6F_{11/2}$ | 355 | $3.73\times10^{-5}$ |
| | | $^6F_{5/2}$ | 411 | $3.9\times10^{-5}$ | | | $^6H_{9/2}$ | 355 | $1.28\times10^{-4}$ |
| | | $^4F_{9/2}$ | 649 | $1.83\times10^{-6}$ | | | $^6F_{9/2}$ | 373 | $3.58\times10^{-5}$ |
| | | $^4G_{11/2}$ | 777 | $9.92\times10^{-6}$ | | | $^6H_{7/2}$ | 374 | $1.35\times10^{-4}$ |

[a] The emission rate, $A_{eq}$, inside a host material with refractive index $n_r$ would be: $A_{eq} = A'_{eq}\ n_r^5$

TABLE S22: Continued: $Dy^{3+}$ EQ spontaneous emission lines between 300 and 1700 nm.

| $SLJ$ | $E_{SLJ}(cm^{-1})$ | $S'L'J'$ | $\lambda$ (nm) | $A'_{eq}$ $(s^{-1})$ [a] | $SLJ$ | $E_{SLJ}(cm^{-1})$ | $S'L'J'$ | $\lambda$ (nm) | $A'_{eq}$ $(s^{-1})$ [a] |
|---|---|---|---|---|---|---|---|---|---|
| $^4K_{11/2}$ | 35631 | $^6F_{7/2}$ | 401 | $4.45\times10^{-6}$ | $(^4F,\,^4G)_{5/2}$ | 34079 | $^6F_{7/2}$ | 428 | $3.88\times10^{-6}$ |
| | | $^4F_{9/2}$ | 686 | $2.05\times10^{-5}$ | | | $^6F_{5/2}$ | 455 | $1.57\times10^{-4}$ |
| | | $^4I_{15/2}$ | 773 | $6.75\times10^{-5}$ | | | $^6F_{3/2}$ | 472 | $4.2\times10^{-4}$ |
| | | $^4G_{11/2}$ | 831 | $1.84\times10^{-5}$ | | | $^6F_{1/2}$ | 484 | $5.39\times10^{-5}$ |
| | | $^4F_{7/2}$ | 998 | $5.11\times10^{-6}$ | | | $^4F_{9/2}$ | 767 | $2.69\times10^{-5}$ |
| | | $^4I_{13/2}$ | 1044 | $9.24\times10^{-6}$ | | | $^4F_{7/2}$ | 1181 | $8.31\times10^{-6}$ |
| | | $^6P_{7/2}$ | 1262 | $7.\times10^{-7}$ | | | $^6P_{5/2}$ | 1352 | $3.67\times10^{-6}$ |
| | | $^4I_{11/2}$ | 1416 | $6.43\times10^{-7}$ | | | $(^4P,\,^6P)_{3/2}$ | 1393 | $2.2\times10^{-6}$ |
| | | $^4M_{15/2}$ | 1640 | $2.27\times10^{-8}$ | | | $^6P_{7/2}$ | 1569 | $2.3\times10^{-7}$ |
| $^4G_{11/2}$ | 35096 | $^6H_{13/2}$ | 315 | $4.36\times10^{-5}$ | $(^4H,\,^4G)_{11/2}$ | 34061 | $^6H_{13/2}$ | 325 | $2.73\times10^{-4}$ |
| | | $^6H_{11/2}$ | 339 | $7.8\times10^{-4}$ | | | $^6H_{11/2}$ | 352 | $6.01\times10^{-4}$ |
| | | $^6F_{11/2}$ | 361 | $1.15\times10^{-4}$ | | | $^6F_{11/2}$ | 375 | $1.12\times10^{-4}$ |
| | | $^6H_{9/2}$ | 362 | $1.47\times10^{-4}$ | | | $^6H_{9/2}$ | 376 | $3.54\times10^{-4}$ |
| | | $^6F_{9/2}$ | 381 | $4.95\times10^{-4}$ | | | $^6F_{9/2}$ | 397 | $1.34\times10^{-4}$ |
| | | $^6H_{7/2}$ | 382 | $2.04\times10^{-5}$ | | | $^6H_{7/2}$ | 398 | $1.28\times10^{-5}$ |
| | | $^6F_{7/2}$ | 410 | $7.16\times10^{-5}$ | | | $^6F_{7/2}$ | 428 | $9.7\times10^{-5}$ |
| | | $^4F_{9/2}$ | 712 | $2.02\times10^{-4}$ | | | $^4F_{9/2}$ | 768 | $1.79\times10^{-4}$ |
| | | $^4I_{15/2}$ | 806 | $2.55\times10^{-4}$ | | | $^4I_{15/2}$ | 880 | $6.31\times10^{-4}$ |
| | | $^4G_{11/2}$ | 869 | $2.05\times10^{-4}$ | | | $^4G_{11/2}$ | 955 | $2.91\times10^{-8}$ |
| | | $^4F_{7/2}$ | 1054 | $7.49\times10^{-5}$ | | | $^4F_{7/2}$ | 1183 | $8.46\times10^{-6}$ |
| | | $^4I_{13/2}$ | 1105 | $8.2\times10^{-5}$ | | | $^4I_{13/2}$ | 1248 | $1.76\times10^{-5}$ |
| | | $^6P_{7/2}$ | 1353 | $3.56\times10^{-6}$ | | | $^6P_{7/2}$ | 1574 | $9.31\times10^{-8}$ |
| | | $^4I_{11/2}$ | 1532 | $6.14\times10^{-7}$ | $^4H_{13/2}$ | 33924 | $^6H_{13/2}$ | 327 | $1.87\times10^{-3}$ |
| $^4G_{9/2}$ | 34755 | $^6H_{13/2}$ | 318 | $5.06\times10^{-5}$ | | | $^6H_{11/2}$ | 353 | $5.77\times10^{-5}$ |
| | | $^6H_{11/2}$ | 343 | $1.01\times10^{-5}$ | | | $^6F_{11/2}$ | 377 | $3.09\times10^{-5}$ |
| | | $^6F_{11/2}$ | 366 | $5.4\times10^{-7}$ | | | $^6H_{9/2}$ | 378 | $3.89\times10^{-6}$ |
| | | $^6H_{9/2}$ | 366 | $3.54\times10^{-4}$ | | | $^6F_{9/2}$ | 399 | $2.61\times10^{-5}$ |
| | | $^6F_{9/2}$ | 386 | $4.38\times10^{-6}$ | | | $^4F_{9/2}$ | 776 | $2.09\times10^{-4}$ |
| | | $^6H_{7/2}$ | 387 | $1.48\times10^{-5}$ | | | $^4I_{15/2}$ | 890 | $3.34\times10^{-4}$ |
| | | $^6H_{5/2}$ | 406 | $4.31\times10^{-7}$ | | | $^4G_{11/2}$ | 968 | $8.54\times10^{-5}$ |
| | | $^6F_{7/2}$ | 416 | $2.44\times10^{-4}$ | | | $^4K_{17/2}$ | 1257 | $4.02\times10^{-5}$ |
| | | $^6F_{5/2}$ | 442 | $7.55\times10^{-6}$ | | | $^4I_{13/2}$ | 1270 | $6.11\times10^{-6}$ |
| | | $^4F_{9/2}$ | 729 | $7.9\times10^{-5}$ | $^4D_{7/2}$ | 33836 | $^6H_{11/2}$ | 354 | $5.24\times10^{-4}$ |
| | | $^4G_{11/2}$ | 896 | $2.61\times10^{-5}$ | | | $^6F_{11/2}$ | 379 | $8.13\times10^{-3}$ |
| | | $^4F_{7/2}$ | 1094 | $5.9\times10^{-5}$ | | | $^6H_{9/2}$ | 379 | $1.91\times10^{-4}$ |
| | | $^4I_{13/2}$ | 1149 | $2.84\times10^{-5}$ | | | $^6F_{9/2}$ | 400 | $3.01\times10^{-3}$ |
| | | $^6P_{5/2}$ | 1239 | $2.13\times10^{-6}$ | | | $^6H_{7/2}$ | 401 | $1.74\times10^{-5}$ |
| | | $^6P_{7/2}$ | 1419 | $7.32\times10^{-6}$ | | | $^6H_{5/2}$ | 422 | $4.39\times10^{-6}$ |
| | | $^4I_{11/2}$ | 1617 | $1.97\times10^{-5}$ | | | $^6F_{7/2}$ | 432 | $9.75\times10^{-4}$ |
| $(^4F,\,^4G)_{5/2}$ | 34079 | $^6H_{9/2}$ | 376 | $7.83\times10^{-4}$ | | | $^6F_{5/2}$ | 460 | $1.73\times10^{-4}$ |
| | | $^6F_{9/2}$ | 396 | $1.68\times10^{-4}$ | | | $^6F_{3/2}$ | 478 | $1.9\times10^{-4}$ |
| | | $^6H_{7/2}$ | 398 | $1.84\times10^{-5}$ | | | $^4F_{9/2}$ | 782 | $1.47\times10^{-4}$ |
| | | $^6H_{5/2}$ | 417 | $4.84\times10^{-7}$ | | | $^4G_{11/2}$ | 976 | $1.03\times10^{-4}$ |

[a] The emission rate, $A_{eq}$, inside a host material with refractive index $n_r$ would be: $A_{eq} = A'_{eq}\ n_r^5$

TABLE S22: Continued: $Dy^{3+}$ EQ spontaneous emission lines between 300 and 1700 nm.

| $SLJ$ | $E_{SLJ}(cm^{-1})$ | $S'L'J'$ | $\lambda$ (nm) | $A'_{eq}$ $(s^{-1})$ [a] | $SLJ$ | $E_{SLJ}(cm^{-1})$ | $S'L'J'$ | $\lambda$ (nm) | $A'_{eq}$ $(s^{-1})$ [a] |
|---|---|---|---|---|---|---|---|---|---|
| $^4D_{7/2}$ | 33836 | $^4F_{7/2}$ | 1216 | $1.74\times10^{-7}$ | $(^4D, ^4P)_{1/2}$ | 31770 | $^6F_{3/2}$ | 530 | $2.43\times10^{-6}$ |
| | | $^6P_{5/2}$ | 1398 | $8.03\times10^{-7}$ | $(^4G, ^4F)_{7/2}$ | 31551 | $^6H_{11/2}$ | 386 | $5.36\times10^{-4}$ |
| | | $(^4P, ^6P)_{3/2}$ | 1442 | $4.42\times10^{-6}$ | | | $^6F_{11/2}$ | 415 | $9.03\times10^{-8}$ |
| | | $^6P_{7/2}$ | 1632 | $3.49\times10^{-6}$ | | | $^6H_{9/2}$ | 415 | $7.05\times10^{-5}$ |
| $^4F_{3/2}$ | 33629 | $^6H_{7/2}$ | 405 | $4.03\times10^{-4}$ | | | $^6F_{9/2}$ | 441 | $2.35\times10^{-4}$ |
| | | $^6H_{5/2}$ | 425 | $1.72\times10^{-4}$ | | | $^6H_{7/2}$ | 442 | $4.98\times10^{-5}$ |
| | | $^6F_{7/2}$ | 436 | $3.87\times10^{-5}$ | | | $^6H_{5/2}$ | 467 | $4.57\times10^{-7}$ |
| | | $^6F_{5/2}$ | 465 | $3.42\times10^{-4}$ | | | $^6F_{7/2}$ | 480 | $7.63\times10^{-5}$ |
| | | $^6F_{3/2}$ | 482 | $1.32\times10^{-4}$ | | | $^6F_{5/2}$ | 514 | $7.48\times10^{-5}$ |
| | | $^6F_{1/2}$ | 495 | $7.09\times10^{-4}$ | | | $^6F_{3/2}$ | 536 | $4.77\times10^{-4}$ |
| | | $^4F_{7/2}$ | 1247 | $2.67\times10^{-6}$ | | | $^4F_{9/2}$ | 952 | $7.45\times10^{-6}$ |
| | | $^6P_{5/2}$ | 1440 | $1.04\times10^{-8}$ | | | $^4G_{11/2}$ | 1257 | $6.07\times10^{-9}$ |
| | | $(^4P, ^6P)_{3/2}$ | 1486 | $3.46\times10^{-10}$ | | | $^4F_{7/2}$ | 1683 | $2.91\times10^{-9}$ |
| | | $^6P_{7/2}$ | 1688 | $8.88\times10^{-7}$ | $^4L_{19/2}$ | 30894 | $^6H_{15/2}$ | 324 | $8.71\times10^{-5}$ |
| $^4L_{17/2}$ | 33454 | $^6H_{13/2}$ | 332 | $1.55\times10^{-6}$ | | | $^4I_{15/2}$ | 1219 | $7.8\times10^{-7}$ |
| | | $^4I_{15/2}$ | 929 | $2.13\times10^{-5}$ | $^4K_{15/2}$ | 30846 | $^6H_{15/2}$ | 324 | $5.19\times10^{-4}$ |
| | | $^4M_{21/2}$ | 1227 | $1.53\times10^{-5}$ | | | $^6H_{13/2}$ | 363 | $6.39\times10^{-4}$ |
| | | $^4K_{17/2}$ | 1335 | $5.24\times10^{-6}$ | | | $^6H_{11/2}$ | 397 | $2.45\times10^{-4}$ |
| | | $^4I_{13/2}$ | 1351 | $2.02\times10^{-6}$ | | | $^6F_{11/2}$ | 427 | $1.53\times10^{-6}$ |
| | | $^4M_{19/2}$ | 1510 | $2.4\times10^{-5}$ | | | $^4I_{15/2}$ | 1226 | $6.5\times10^{-6}$ |
| $(^4K, ^4L)_{13/2}$ | 33321 | $^6H_{15/2}$ | 300 | $3.84\times10^{-4}$ | | | $^4G_{11/2}$ | 1379 | $8.23\times10^{-8}$ |
| | | $^6H_{13/2}$ | 333 | $2.32\times10^{-4}$ | $^4I_{9/2}$ | 30748 | $^6H_{13/2}$ | 365 | $9.52\times10^{-6}$ |
| | | $^6H_{11/2}$ | 361 | $3.51\times10^{-4}$ | | | $^6H_{11/2}$ | 398 | $7.75\times10^{-6}$ |
| | | $^6F_{11/2}$ | 386 | $8.44\times10^{-6}$ | | | $^6F_{11/2}$ | 429 | $5.55\times10^{-6}$ |
| | | $^6H_{9/2}$ | 387 | $1.1\times10^{-4}$ | | | $^6H_{9/2}$ | 429 | $4.16\times10^{-5}$ |
| | | $^6F_{9/2}$ | 409 | $4.68\times10^{-6}$ | | | $^6F_{9/2}$ | 457 | $1.23\times10^{-5}$ |
| | | $^4F_{9/2}$ | 815 | $2.05\times10^{-6}$ | | | $^6H_{7/2}$ | 458 | $3.69\times10^{-5}$ |
| | | $^4I_{15/2}$ | 941 | $1.39\times10^{-6}$ | | | $^6H_{5/2}$ | 485 | $2.\times10^{-4}$ |
| | | $^4G_{11/2}$ | 1028 | $3.53\times10^{-8}$ | | | $^6F_{7/2}$ | 499 | $7.69\times10^{-6}$ |
| | | $^4K_{17/2}$ | 1360 | $9.92\times10^{-8}$ | | | $^6F_{5/2}$ | 537 | $4.03\times10^{-5}$ |
| | | $^4I_{13/2}$ | 1375 | $2.4\times10^{-7}$ | | | $^4F_{9/2}$ | 1031 | $3.15\times10^{-7}$ |
| $(^4D, ^4G)_{5/2}$ | 31937 | $^6H_{9/2}$ | 409 | $1.73\times10^{-6}$ | | | $^4G_{11/2}$ | 1398 | $1.12\times10^{-9}$ |
| | | $^6F_{9/2}$ | 433 | $1.24\times10^{-5}$ | $^6P_{3/2}$ | 30144 | $^6H_{7/2}$ | 471 | $2.36\times10^{-5}$ |
| | | $^6H_{7/2}$ | 435 | $1.07\times10^{-4}$ | | | $^6H_{5/2}$ | 500 | $1.38\times10^{-5}$ |
| | | $^6H_{5/2}$ | 458 | $2.6\times10^{-5}$ | | | $^6F_{7/2}$ | 515 | $1.81\times10^{-3}$ |
| | | $^6F_{7/2}$ | 471 | $1.07\times10^{-8}$ | | | $^6F_{5/2}$ | 555 | $3.47\times10^{-3}$ |
| | | $^6F_{5/2}$ | 504 | $1.41\times10^{-5}$ | | | $^6F_{3/2}$ | 580 | $6.09\times10^{-3}$ |
| | | $^6F_{3/2}$ | 525 | $4.11\times10^{-6}$ | | | $^6F_{1/2}$ | 598 | $1.73\times10^{-2}$ |
| | | $^6F_{1/2}$ | 540 | $1.15\times10^{-3}$ | $^4G_{9/2}$ | 30044 | $^6H_{13/2}$ | 374 | $2.82\times10^{-4}$ |
| | | $^4F_{9/2}$ | 918 | $4.81\times10^{-5}$ | | | $^6H_{11/2}$ | 410 | $6.57\times10^{-5}$ |
| | | $^4F_{7/2}$ | 1581 | $2.77\times10^{-8}$ | | | $^6F_{11/2}$ | 442 | $4.39\times10^{-5}$ |
| $(^4D, ^4P)_{1/2}$ | 31770 | $^6H_{5/2}$ | 462 | $3.03\times10^{-5}$ | | | $^6H_{9/2}$ | 443 | $1.53\times10^{-4}$ |
| | | $^6F_{5/2}$ | 509 | $4.25\times10^{-5}$ | | | $^6F_{9/2}$ | 472 | $2.78\times10^{-4}$ |

[a] The emission rate, $A_{eq}$, inside a host material with refractive index $n_r$ would be: $A_{eq} = A'_{eq}\ n_r^5$

TABLE S22: Continued: $Dy^{3+}$ EQ spontaneous emission lines between 300 and 1700 nm.

| $SLJ$ | $E_{SLJ}(cm^{-1})$ | $S'L'J'$ | $\lambda$ (nm) | $A'_{eq}$ $(s^{-1})$ [a] | $SLJ$ | $E_{SLJ}(cm^{-1})$ | $S'L'J'$ | $\lambda$ (nm) | $A'_{eq}$ $(s^{-1})$ [a] |
|---|---|---|---|---|---|---|---|---|---|
| $^4G_{9/2}$ | 30044 | $^6H_{7/2}$ | 473 | $3.73 \times 10^{-6}$ | $(^4P,\,^6P)_{3/2}$ | 26899 | $^6H_{7/2}$ | 556 | $5.97 \times 10^{-6}$ |
| | | $^6H_{5/2}$ | 502 | $2.46 \times 10^{-5}$ | | | $^6H_{5/2}$ | 596 | $1.55 \times 10^{-5}$ |
| | | $^6F_{7/2}$ | 517 | $4.46 \times 10^{-6}$ | | | $^6F_{7/2}$ | 618 | $4.02 \times 10^{-4}$ |
| | | $^6F_{5/2}$ | 558 | $3.43 \times 10^{-4}$ | | | $^6F_{5/2}$ | 676 | $1.2 \times 10^{-3}$ |
| | | $^4F_{9/2}$ | 1111 | $1.47 \times 10^{-6}$ | | | $^6F_{3/2}$ | 714 | $2.52 \times 10^{-3}$ |
| | | $^4G_{11/2}$ | 1550 | $5.34 \times 10^{-7}$ | | | $^6F_{1/2}$ | 742 | $4.24 \times 10^{-3}$ |
| $^4M_{17/2}$ | 29740 | $^6H_{15/2}$ | 336 | $3.47 \times 10^{-4}$ | $^4M_{19/2}$ | 26833 | $^6H_{15/2}$ | 373 | $2.71 \times 10^{-5}$ |
| | | $^6H_{13/2}$ | 378 | $6.47 \times 10^{-5}$ | $^6P_{5/2}$ | 26684 | $^6H_{9/2}$ | 520 | $9.98 \times 10^{-6}$ |
| | | $^4I_{15/2}$ | 1419 | $1.64 \times 10^{-6}$ | | | $^6F_{9/2}$ | 561 | $6.04 \times 10^{-3}$ |
| $^4M_{15/2}$ | 29534 | $^6H_{15/2}$ | 339 | $2.73 \times 10^{-4}$ | | | $^6H_{7/2}$ | 563 | $7.99 \times 10^{-9}$ |
| | | $^6H_{13/2}$ | 381 | $9.73 \times 10^{-5}$ | | | $^6H_{5/2}$ | 604 | $3.33 \times 10^{-6}$ |
| | | $^6H_{11/2}$ | 418 | $1.99 \times 10^{-6}$ | | | $^6F_{7/2}$ | 626 | $5.25 \times 10^{-3}$ |
| | | $^6F_{11/2}$ | 452 | $2.22 \times 10^{-6}$ | | | $^6F_{5/2}$ | 686 | $3.51 \times 10^{-3}$ |
| | | $^4I_{15/2}$ | 1461 | $2.21 \times 10^{-6}$ | | | $^6F_{3/2}$ | 726 | $2.02 \times 10^{-3}$ |
| | | $^4G_{11/2}$ | 1683 | $4.06 \times 10^{-7}$ | | | $^6F_{1/2}$ | 754 | $9.9 \times 10^{-4}$ |
| $(^4F,\,^4D)_{5/2}$ | 29478 | $^6H_{9/2}$ | 454 | $1.86 \times 10^{-4}$ | $^4I_{13/2}$ | 26050 | $^6H_{15/2}$ | 384 | $2.42 \times 10^{-4}$ |
| | | $^6F_{9/2}$ | 485 | $5.53 \times 10^{-4}$ | | | $^6H_{13/2}$ | 440 | $4.98 \times 10^{-5}$ |
| | | $^6H_{7/2}$ | 486 | $2.8 \times 10^{-8}$ | | | $^6H_{11/2}$ | 490 | $5.76 \times 10^{-5}$ |
| | | $^6H_{5/2}$ | 517 | $1.78 \times 10^{-4}$ | | | $^6F_{11/2}$ | 537 | $3.71 \times 10^{-6}$ |
| | | $^6F_{7/2}$ | 533 | $6.52 \times 10^{-4}$ | | | $^6H_{9/2}$ | 538 | $2.27 \times 10^{-4}$ |
| | | $^6F_{5/2}$ | 576 | $2.57 \times 10^{-4}$ | | | $^6F_{9/2}$ | 581 | $1.31 \times 10^{-5}$ |
| | | $^6F_{3/2}$ | 603 | $5.27 \times 10^{-4}$ | $^4K_{17/2}$ | 25967 | $^6H_{15/2}$ | 385 | $1.02 \times 10^{-3}$ |
| | | $^6F_{1/2}$ | 623 | $1.58 \times 10^{-4}$ | | | $^6H_{13/2}$ | 441 | $2. \times 10^{-4}$ |
| | | $^4F_{9/2}$ | 1186 | $2.57 \times 10^{-5}$ | $^4F_{7/2}$ | 25610 | $^6H_{11/2}$ | 500 | $7.24 \times 10^{-4}$ |
| $^4I_{11/2}$ | 28569 | $^6H_{15/2}$ | 350 | $5.66 \times 10^{-6}$ | | | $^6F_{11/2}$ | 550 | $2.24 \times 10^{-3}$ |
| | | $^6H_{13/2}$ | 396 | $5.42 \times 10^{-5}$ | | | $^6H_{9/2}$ | 551 | $3.29 \times 10^{-5}$ |
| | | $^6H_{11/2}$ | 436 | $5.66 \times 10^{-5}$ | | | $^6F_{9/2}$ | 597 | $1. \times 10^{-3}$ |
| | | $^6F_{11/2}$ | 473 | $1.54 \times 10^{-7}$ | | | $^6H_{7/2}$ | 599 | $5.84 \times 10^{-5}$ |
| | | $^6H_{9/2}$ | 474 | $1.71 \times 10^{-7}$ | | | $^6H_{5/2}$ | 646 | $1.72 \times 10^{-5}$ |
| | | $^6F_{9/2}$ | 507 | $4.16 \times 10^{-6}$ | | | $^6F_{7/2}$ | 671 | $1.94 \times 10^{-4}$ |
| | | $^6H_{7/2}$ | 509 | $3.17 \times 10^{-4}$ | | | $^6F_{5/2}$ | 741 | $1.14 \times 10^{-4}$ |
| | | $^6F_{7/2}$ | 560 | $8.67 \times 10^{-7}$ | | | $^6F_{3/2}$ | 787 | $9.7 \times 10^{-7}$ |
| | | $^4F_{9/2}$ | 1329 | $1.63 \times 10^{-6}$ | $^4G_{11/2}$ | 23594 | $^6H_{15/2}$ | 424 | $8.05 \times 10^{-6}$ |
| $^6P_{7/2}$ | 27707 | $^6H_{11/2}$ | 453 | $3.11 \times 10^{-4}$ | | | $^6H_{13/2}$ | 493 | $2.2 \times 10^{-5}$ |
| | | $^6F_{11/2}$ | 493 | $2.25 \times 10^{-2}$ | | | $^6H_{11/2}$ | 557 | $6.22 \times 10^{-6}$ |
| | | $^6H_{9/2}$ | 494 | $3.69 \times 10^{-5}$ | | | $^6F_{11/2}$ | 619 | $1.4 \times 10^{-4}$ |
| | | $^6F_{9/2}$ | 530 | $8.29 \times 10^{-3}$ | | | $^6H_{9/2}$ | 620 | $2.66 \times 10^{-6}$ |
| | | $^6H_{7/2}$ | 532 | $1.44 \times 10^{-5}$ | | | $^6F_{9/2}$ | 678 | $4.2 \times 10^{-5}$ |
| | | $^6H_{5/2}$ | 569 | $8.15 \times 10^{-6}$ | | | $^6H_{7/2}$ | 682 | $1.05 \times 10^{-6}$ |
| | | $^6F_{7/2}$ | 588 | $2.63 \times 10^{-3}$ | | | $^6F_{7/2}$ | 776 | $6.58 \times 10^{-5}$ |
| | | $^6F_{5/2}$ | 641 | $6.45 \times 10^{-4}$ | $^4I_{15/2}$ | 22691 | $^6H_{15/2}$ | 441 | $2.46 \times 10^{-4}$ |
| | | $^6F_{3/2}$ | 676 | $2.78 \times 10^{-4}$ | | | $^6H_{13/2}$ | 516 | $7.62 \times 10^{-5}$ |
| | | $^4F_{9/2}$ | 1501 | $4.37 \times 10^{-6}$ | | | $^6H_{11/2}$ | 586 | $8.98 \times 10^{-5}$ |

[a] The emission rate, $A_{eq}$, inside a host material with refractive index $n_r$ would be: $A_{eq} = A'_{eq}\ n_r^5$

TABLE S22: Continued: $Dy^{3+}$ EQ spontaneous emission lines between 300 and 1700 nm.

| $SLJ$ | $E_{SLJ}(cm^{-1})$ | $S'L'J'$ | $\lambda$ (nm) | $A'_{eq}$ $(s^{-1})$ [a] | $SLJ$ | $E_{SLJ}(cm^{-1})$ | $S'L'J'$ | $\lambda$ (nm) | $A'_{eq}$ $(s^{-1})$ [a] |
|---|---|---|---|---|---|---|---|---|---|
| $^4I_{15/2}$ | 22691 | $^6F_{11/2}$ | 655 | $1.44 \times 10^{-5}$ | $^4F_{9/2}$ | 21045 | $^6H_{7/2}$ | 825 | $4.38 \times 10^{-6}$ |
| $^4F_{9/2}$ | 21045 | $^6H_{13/2}$ | 564 | $3.99 \times 10^{-4}$ | | | $^6H_{5/2}$ | 916 | $8.89 \times 10^{-8}$ |
| | | $^6H_{11/2}$ | 649 | $5.73 \times 10^{-5}$ | | | $^6F_{7/2}$ | 968 | $6.49 \times 10^{-8}$ |
| | | $^6F_{11/2}$ | 734 | $1.06 \times 10^{-5}$ | | | $^6F_{5/2}$ | 1119 | $8.92 \times 10^{-6}$ |
| | | $^6H_{9/2}$ | 736 | $1.28 \times 10^{-5}$ | $^6F_{11/2}$ | 7429 | $^6H_{15/2}$ | 1346 | $1.06 \times 10^{-4}$ |
| | | $^6F_{9/2}$ | 820 | $2.04 \times 10^{-6}$ | | | | | |

[a] The emission rate, $A_{eq}$, inside a host material with refractive index $n_r$ would be: $A_{eq} = A'_{eq}\ n_r^5$

TABLE S23: Calculated $Ho^{3+}$ EQ spontaneous emission lines between 300 and 1700 nm.

| $SLJ$ | $E_{SLJ}(cm^{-1})$ | $S'L'J'$ | $\lambda$ (nm) | $A'_{eq}$ $(s^{-1})$ [a] | $SLJ$ | $E_{SLJ}(cm^{-1})$ | $S'L'J'$ | $\lambda$ (nm) | $A'_{eq}$ $(s^{-1})$ [a] |
|---|---|---|---|---|---|---|---|---|---|
| $^5D_1$ | 39165 | $^5S_2$ | 469 | $3.33 \times 10^{-3}$ | $^3I_6$ | 38648 | $^5I_5$ | 363 | $2.22 \times 10^{-3}$ |
| | | $^5F_3$ | 522 | $1.63 \times 10^{-3}$ | | | $^5I_4$ | 393 | $2.53 \times 10^{-4}$ |
| | | $^5F_2$ | 534 | $6.98 \times 10^{-4}$ | | | $^5F_5$ | 421 | $3.18 \times 10^{-4}$ |
| | | $^5F_1$ | 573 | $3.95 \times 10^{-3}$ | | | $^5F_4$ | 485 | $1.62 \times 10^{-5}$ |
| | | $\left(^5F,\,^5G\right)_2$ | 886 | $1.05 \times 10^{-4}$ | | | $^3K_8$ | 558 | $1.98 \times 10^{-3}$ |
| | | $^5G_3$ | 905 | $1.67 \times 10^{-4}$ | | | $^5G_6$ | 577 | $6.44 \times 10^{-5}$ |
| | | $^5G_2$ | 1092 | $6.18 \times 10^{-5}$ | | | $\left(^5G,\,^3G\right)_5$ | 651 | $2.95 \times 10^{-4}$ |
| | | $^3D_3$ | 1596 | $6.17 \times 10^{-7}$ | | | $^5G_4$ | 743 | $1.92 \times 10^{-4}$ |
| | | $^3P_1$ | 1607 | $3.18 \times 10^{-9}$ | | | $^3K_7$ | 769 | $4.4 \times 10^{-4}$ |
| $^3M_9$ | 39159 | $^3K_8$ | 542 | $1.48 \times 10^{-4}$ | | | $\left(^5G,\,^3H\right)_5$ | 853 | $1.65 \times 10^{-4}$ |
| | | $^3K_7$ | 739 | $4.28 \times 10^{-7}$ | | | $^3H_6$ | 883 | $6.96 \times 10^{-5}$ |
| | | $^3L_9$ | 972 | $1.22 \times 10^{-5}$ | | | $\left(^3F,\,^3G\right)_4$ | 1078 | $9.78 \times 10^{-6}$ |
| $^5D_3$ | 38728 | $^5I_5$ | 362 | $2.57 \times 10^{-3}$ | | | $^3K_6$ | 1108 | $2.33 \times 10^{-5}$ |
| | | $^5I_4$ | 392 | $1.21 \times 10^{-4}$ | $^3F_4$ | 38607 | $^5I_6$ | 332 | $6.71 \times 10^{-5}$ |
| | | $^5F_5$ | 420 | $4.41 \times 10^{-3}$ | | | $^5I_5$ | 364 | $2.77 \times 10^{-5}$ |
| | | $^5S_2$ | 478 | $1.2 \times 10^{-2}$ | | | $^5I_4$ | 394 | $1.72 \times 10^{-5}$ |
| | | $^5F_4$ | 483 | $3.4 \times 10^{-3}$ | | | $^5F_5$ | 422 | $1.35 \times 10^{-4}$ |
| | | $^5F_3$ | 534 | $2.34 \times 10^{-3}$ | | | $^5S_2$ | 481 | $5.96 \times 10^{-5}$ |
| | | $^5F_2$ | 547 | $1.1 \times 10^{-2}$ | | | $^5F_4$ | 486 | $2.13 \times 10^{-5}$ |
| | | $^5F_1$ | 587 | $1.09 \times 10^{-3}$ | | | $^5F_3$ | 538 | $4.1 \times 10^{-5}$ |
| | | $\left(^5G,\,^3G\right)_5$ | 648 | $1.45 \times 10^{-3}$ | | | $^5F_2$ | 551 | $1.23 \times 10^{-5}$ |
| | | $^5G_4$ | 738 | $2.57 \times 10^{-4}$ | | | $^5G_6$ | 578 | $5.07 \times 10^{-4}$ |
| | | $\left(^5G,\,^3H\right)_5$ | 847 | $3.77 \times 10^{-4}$ | | | $\left(^5G,\,^3G\right)_5$ | 653 | $5.16 \times 10^{-4}$ |
| | | $\left(^5F,\,^5G\right)_2$ | 922 | $1.72 \times 10^{-5}$ | | | $^5G_4$ | 745 | $1.99 \times 10^{-4}$ |
| | | $^5G_3$ | 942 | $5.58 \times 10^{-5}$ | | | $\left(^5G,\,^3H\right)_5$ | 856 | $4.42 \times 10^{-4}$ |
| | | $\left(^3F,\,^3G\right)_4$ | 1069 | $1.69 \times 10^{-6}$ | | | $^3H_6$ | 886 | $1.95 \times 10^{-4}$ |
| | | $^5G_2$ | 1147 | $1.9 \times 10^{-5}$ | | | $\left(^5F,\,^5G\right)_2$ | 932 | $1.03 \times 10^{-4}$ |
| $^3I_5$ | 38713 | $^5I_6$ | 331 | $2.74 \times 10^{-8}$ | | | $^5G_3$ | 953 | $2.35 \times 10^{-5}$ |
| | | $^5I_5$ | 363 | $8.05 \times 10^{-4}$ | | | $\left(^3F,\,^3G\right)_4$ | 1083 | $2.2 \times 10^{-5}$ |
| | | $^5I_4$ | 392 | $1.5 \times 10^{-3}$ | | | $^3K_6$ | 1113 | $1.02 \times 10^{-6}$ |
| | | $^5F_5$ | 420 | $1.74 \times 10^{-4}$ | | | $^5G_2$ | 1163 | $2.86 \times 10^{-5}$ |
| | | $^5F_4$ | 483 | $3.55 \times 10^{-5}$ | $^3L_7$ | 37966 | $^5I_7$ | 304 | $8.95 \times 10^{-5}$ |
| | | $^5F_3$ | 535 | $9.87 \times 10^{-5}$ | | | $^5I_6$ | 339 | $4.15 \times 10^{-4}$ |
| | | $^5G_6$ | 574 | $3. \times 10^{-5}$ | | | $^5I_5$ | 373 | $3.49 \times 10^{-4}$ |
| | | $\left(^5G,\,^3G\right)_5$ | 648 | $5.75 \times 10^{-5}$ | | | $^5F_5$ | 434 | $2.38 \times 10^{-5}$ |
| | | $^5G_4$ | 739 | $5.99 \times 10^{-7}$ | | | $^3K_8$ | 580 | $1.59 \times 10^{-5}$ |
| | | $^3K_7$ | 765 | $9. \times 10^{-5}$ | | | $^5G_6$ | 600 | $7.86 \times 10^{-7}$ |
| | | $\left(^5G,\,^3H\right)_5$ | 848 | $6.57 \times 10^{-5}$ | | | $\left(^5G,\,^3G\right)_5$ | 681 | $3.19 \times 10^{-6}$ |
| | | $^3H_6$ | 878 | $4.85 \times 10^{-5}$ | | | $^3K_7$ | 811 | $3.26 \times 10^{-5}$ |
| | | $^5G_3$ | 943 | $2.24 \times 10^{-6}$ | | | $\left(^5G,\,^3H\right)_5$ | 906 | $7.43 \times 10^{-7}$ |
| | | $\left(^3F,\,^3G\right)_4$ | 1071 | $3.09 \times 10^{-5}$ | | | $^3H_6$ | 939 | $7.19 \times 10^{-6}$ |
| | | $^3K_6$ | 1100 | $1.12 \times 10^{-4}$ | | | $^3L_9$ | 1100 | $2.66 \times 10^{-6}$ |
| $^3I_6$ | 38648 | $^5I_6$ | 332 | $1.22 \times 10^{-3}$ | | | $^3K_6$ | 1199 | $3.99 \times 10^{-5}$ |

[a] The emission rate, $A_{eq}$, inside a host material with refractive index $n_r$ would be: $A_{eq} = A'_{eq}\ n_r^5$

TABLE S23: Continued: $Ho^{3+}$ EQ spontaneous emission lines between 300 and 1700 nm.

| $SLJ$ | $E_{SLJ}(cm^{-1})$ | $S'L'J'$ | $\lambda$ (nm) | $A'_{eq}$ $(s^{-1})$ [a] | $SLJ$ | $E_{SLJ}(cm^{-1})$ | $S'L'J'$ | $\lambda$ (nm) | $A'_{eq}$ $(s^{-1})$ [a] |
|---|---|---|---|---|---|---|---|---|---|
| $\left(^1L,\,^3L\right)_8$ | 37687 | $^5I_7$ | 307 | $4.86\times10^{-4}$ | $\left(^3H,\,^3G\right)_5$ | 36196 | $^3H_6$ | 1126 | $1.49\times10^{-5}$ |
| | | $^5I_6$ | 343 | $5.8\times10^{-5}$ | | | $^5G_3$ | 1237 | $2.29\times10^{-9}$ |
| | | $^3K_8$ | 589 | $2.52\times10^{-4}$ | | | $\left(^3F,\,^3G\right)_4$ | 1466 | $1.37\times10^{-6}$ |
| | | $^5G_6$ | 610 | $3.67\times10^{-7}$ | | | $^3K_6$ | 1522 | $8.45\times10^{-7}$ |
| | | $^3K_7$ | 830 | $3.1\times10^{-5}$ | $^3P_0$ | 35725 | $^5S_2$ | 559 | $3.85\times10^{-6}$ |
| | | $^3H_6$ | 964 | $2.6\times10^{-6}$ | | | $^5F_2$ | 654 | $1.44\times10^{-5}$ |
| | | $^3L_9$ | 1135 | $2.\times10^{-5}$ | | | $\left(^5F,\,^5G\right)_2$ | 1274 | $8.19\times10^{-7}$ |
| | | $^3K_6$ | 1240 | $1.24\times10^{-5}$ | $\left(^3F,\,^5G\right)_2$ | 35562 | $^5I_4$ | 447 | $2.51\times10^{-3}$ |
| $^3P_2$ | 37409 | $^5I_4$ | 413 | $4.02\times10^{-5}$ | | | $^5S_2$ | 564 | $1.59\times10^{-3}$ |
| | | $^5S_2$ | 511 | $2.01\times10^{-3}$ | | | $^5F_4$ | 570 | $3.79\times10^{-4}$ |
| | | $^5F_4$ | 516 | $1.98\times10^{-4}$ | | | $^5F_3$ | 643 | $1.41\times10^{-4}$ |
| | | $^5F_3$ | 575 | $1.99\times10^{-4}$ | | | $^5F_2$ | 661 | $2.22\times10^{-5}$ |
| | | $^5F_2$ | 589 | $1.29\times10^{-4}$ | | | $^5F_1$ | 721 | $2.12\times10^{-3}$ |
| | | $^5F_1$ | 637 | $5.26\times10^{-4}$ | | | $^5G_4$ | 963 | $3.71\times10^{-5}$ |
| | | $^5G_4$ | 818 | $8.83\times10^{-5}$ | | | $\left(^5F,\,^5G\right)_2$ | 1302 | $3.74\times10^{-5}$ |
| | | $\left(^5F,\,^5G\right)_2$ | 1049 | $3.79\times10^{-7}$ | | | $^5G_3$ | 1342 | $4.72\times10^{-6}$ |
| | | $^5G_3$ | 1076 | $2.1\times10^{-5}$ | | | $\left(^3F,\,^3G\right)_4$ | 1616 | $5.14\times10^{-6}$ |
| | | $\left(^3F,\,^3G\right)_4$ | 1245 | $1.57\times10^{-5}$ | $\left(^1G,\,^3H\right)_4$ | 35453 | $^5I_6$ | 371 | $5.7\times10^{-3}$ |
| | | $^5G_2$ | 1351 | $4.09\times10^{-6}$ | | | $^5I_5$ | 411 | $2.97\times10^{-4}$ |
| $^3I_7$ | 37258 | $^5I_7$ | 311 | $5.95\times10^{-4}$ | | | $^5I_4$ | 449 | $7.21\times10^{-5}$ |
| | | $^5I_6$ | 348 | $1.24\times10^{-3}$ | | | $^5F_5$ | 487 | $2.72\times10^{-3}$ |
| | | $^5I_5$ | 383 | $9.85\times10^{-6}$ | | | $^5S_2$ | 567 | $3.23\times10^{-3}$ |
| | | $^5F_5$ | 448 | $7.08\times10^{-4}$ | | | $^5F_4$ | 574 | $1.73\times10^{-3}$ |
| | | $^3K_8$ | 604 | $1.27\times10^{-3}$ | | | $^5F_3$ | 647 | $4.68\times10^{-5}$ |
| | | $^5G_6$ | 627 | $9.78\times10^{-5}$ | | | $^5F_2$ | 666 | $4.99\times10^{-4}$ |
| | | $\left(^5G,\,^3G\right)_5$ | 716 | $1.89\times10^{-4}$ | | | $^5G_6$ | 707 | $2.89\times10^{-4}$ |
| | | $^3K_7$ | 860 | $1.95\times10^{-5}$ | | | $\left(^5G,\,^3G\right)_5$ | 822 | $5.4\times10^{-5}$ |
| | | $\left(^5G,\,^3H\right)_5$ | 968 | $1.4\times10^{-5}$ | | | $^5G_4$ | 974 | $2.26\times10^{-6}$ |
| | | $^3H_6$ | 1006 | $1.52\times10^{-4}$ | | | $\left(^5G,\,^3H\right)_5$ | 1172 | $2.59\times10^{-6}$ |
| | | $^3L_9$ | 1193 | $7.86\times10^{-5}$ | | | $^3H_6$ | 1229 | $9.78\times10^{-6}$ |
| | | $^3K_6$ | 1310 | $1.82\times10^{-6}$ | | | $\left(^5F,\,^5G\right)_2$ | 1320 | $1.1\times10^{-6}$ |
| $\left(^3H,\,^3G\right)_5$ | 36196 | $^5I_7$ | 321 | $8.77\times10^{-3}$ | | | $^5G_3$ | 1362 | $3.01\times10^{-7}$ |
| | | $^5I_6$ | 361 | $1.08\times10^{-3}$ | | | $\left(^3F,\,^3G\right)_4$ | 1645 | $2.96\times10^{-7}$ |
| | | $^5I_5$ | 399 | $1.23\times10^{-5}$ | $\left(^3F,\,^3G\right)_3$ | 34498 | $^5I_5$ | 428 | $6.65\times10^{-4}$ |
| | | $^5I_4$ | 435 | $3.07\times10^{-4}$ | | | $^5I_4$ | 470 | $1.45\times10^{-4}$ |
| | | $^5F_5$ | 470 | $1.3\times10^{-5}$ | | | $^5F_5$ | 511 | $4.19\times10^{-4}$ |
| | | $^5F_4$ | 550 | $5.79\times10^{-4}$ | | | $^5S_2$ | 600 | $2.24\times10^{-3}$ |
| | | $^5F_3$ | 618 | $5.27\times10^{-5}$ | | | $^5F_4$ | 607 | $3.03\times10^{-4}$ |
| | | $^5G_6$ | 672 | $1.05\times10^{-5}$ | | | $^5F_3$ | 690 | $5.65\times10^{-4}$ |
| | | $\left(^5G,\,^3G\right)_5$ | 775 | $3.11\times10^{-5}$ | | | $^5F_2$ | 712 | $5.39\times10^{-4}$ |
| | | $^5G_4$ | 908 | $2.2\times10^{-6}$ | | | $^5F_1$ | 781 | $2.94\times10^{-4}$ |
| | | $^3K_7$ | 947 | $6.32\times10^{-6}$ | | | $\left(^5G,\,^3G\right)_5$ | 892 | $5.98\times10^{-5}$ |
| | | $\left(^5G,\,^3H\right)_5$ | 1078 | $1.52\times10^{-7}$ | | | $^5G_4$ | 1073 | $5.53\times10^{-5}$ |

[a] The emission rate, $A_{eq}$, inside a host material with refractive index $n_r$ would be: $A_{eq} = A'_{eq}\ n_r^5$

TABLE S23: Continued: $Ho^{3+}$ EQ spontaneous emission lines between 300 and 1700 nm.

| $SLJ$ | $E_{SLJ}(cm^{-1})$ | $S'L'J'$ | $\lambda$ (nm) | $A'_{eq}$ $(s^{-1})$ [a] | $SLJ$ | $E_{SLJ}(cm^{-1})$ | $S'L'J'$ | $\lambda$ (nm) | $A'_{eq}$ $(s^{-1})$ [a] |
|---|---|---|---|---|---|---|---|---|---|
| $\left(^3F,\,^3G\right)_3$ | 34498 | $\left(^5G,\,^3H\right)_5$ | 1320 | $2.2\times10^{-5}$ | $^5G_2$ | 30009 | $^5F_2$ | 1045 | $2.51\times10^{-4}$ |
| | | $\left(^5F,\,^5G\right)_2$ | 1511 | $3.69\times10^{-7}$ | | | $^5F_1$ | 1204 | $2.73\times10^{-4}$ |
| | | $^5G_3$ | 1566 | $3.66\times10^{-6}$ | $^3K_6$ | 29625 | $^5I_8$ | 338 | $3.58\times10^{-4}$ |
| $^3M_{10}$ | 34003 | $^3K_8$ | 753 | $4.74\times10^{-5}$ | | | $^5I_7$ | 407 | $4.61\times10^{-5}$ |
| $\left(^5D,\,^5G\right)_4$ | 33877 | $^5I_6$ | 394 | $6.69\times10^{-3}$ | | | $^5I_6$ | 473 | $4.59\times10^{-5}$ |
| | | $^5I_5$ | 440 | $1.5\times10^{-3}$ | | | $^5I_5$ | 541 | $1.98\times10^{-6}$ |
| | | $^5I_4$ | 484 | $2.82\times10^{-5}$ | | | $^5I_4$ | 609 | $7.13\times10^{-5}$ |
| | | $^5F_5$ | 528 | $5.34\times10^{-3}$ | | | $^5F_5$ | 680 | $4.36\times10^{-6}$ |
| | | $^5S_2$ | 623 | $7.83\times10^{-3}$ | | | $^5F_4$ | 862 | $1.24\times10^{-7}$ |
| | | $^5F_4$ | 631 | $3.71\times10^{-4}$ | | | $^3K_8$ | 1122 | $5.68\times10^{-7}$ |
| | | $^5F_3$ | 721 | $1.22\times10^{-3}$ | | | $^5G_6$ | 1202 | $2.64\times10^{-7}$ |
| | | $^5F_2$ | 744 | $3.\times10^{-5}$ | | | $\left(^5G,\,^3G\right)_5$ | 1578 | $9.04\times10^{-8}$ |
| | | $^5G_6$ | 795 | $1.23\times10^{-3}$ | $\left(^3F,\,^3G\right)_4$ | 29374 | $^5I_6$ | 479 | $2.35\times10^{-3}$ |
| | | $\left(^5G,\,^3G\right)_5$ | 944 | $2.49\times10^{-6}$ | | | $^5I_5$ | 548 | $2.42\times10^{-6}$ |
| | | $^5G_4$ | 1150 | $7.21\times10^{-6}$ | | | $^5I_4$ | 618 | $1.67\times10^{-5}$ |
| | | $\left(^5G,\,^3H\right)_5$ | 1438 | $2.4\times10^{-5}$ | | | $^5F_5$ | 692 | $7.12\times10^{-4}$ |
| | | $^3H_6$ | 1524 | $2.47\times10^{-9}$ | | | $^5S_2$ | 866 | $7.62\times10^{-4}$ |
| | | $\left(^5F,\,^5G\right)_2$ | 1667 | $2.48\times10^{-5}$ | | | $^5F_4$ | 881 | $2.78\times10^{-4}$ |
| $^3L_8$ | 33577 | $^5I_7$ | 351 | $7.09\times10^{-4}$ | | | $^5F_3$ | 1067 | $7.43\times10^{-7}$ |
| | | $^5I_6$ | 399 | $1.34\times10^{-4}$ | | | $^5F_2$ | 1120 | $3.83\times10^{-5}$ |
| | | $^3K_8$ | 777 | $8.98\times10^{-5}$ | | | $^5G_6$ | 1239 | $4.07\times10^{-5}$ |
| | | $^5G_6$ | 815 | $5.53\times10^{-7}$ | | | $\left(^5G,\,^3G\right)_5$ | 1642 | $6.04\times10^{-6}$ |
| | | $^3K_7$ | 1259 | $3.1\times10^{-5}$ | $^3L_9$ | 28873 | $^5I_8$ | 346 | $2.45\times10^{-3}$ |
| | | $^3H_6$ | 1598 | $3.45\times10^{-8}$ | | | $^5I_7$ | 420 | $1.44\times10^{-4}$ |
| $^3P_1$ | 32942 | $^5S_2$ | 661 | $1.55\times10^{-5}$ | | | $^3K_8$ | 1226 | $7.45\times10^{-5}$ |
| | | $^5F_3$ | 773 | $1.65\times10^{-5}$ | $^5G_3$ | 28112 | $^5I_5$ | 589 | $5.98\times10^{-3}$ |
| | | $^5F_2$ | 800 | $7.03\times10^{-9}$ | | | $^5I_4$ | 671 | $1.06\times10^{-3}$ |
| | | $^5F_1$ | 890 | $1.89\times10^{-6}$ | | | $^5F_5$ | 758 | $3.65\times10^{-5}$ |
| $^3D_3$ | 32901 | $^5I_5$ | 459 | $3.03\times10^{-4}$ | | | $^5S_2$ | 972 | $6.05\times10^{-5}$ |
| | | $^5I_4$ | 508 | $8.29\times10^{-5}$ | | | $^5F_4$ | 992 | $6.94\times10^{-5}$ |
| | | $^5F_5$ | 556 | $1.9\times10^{-5}$ | | | $^5F_3$ | 1233 | $1.81\times10^{-4}$ |
| | | $^5S_2$ | 663 | $2.47\times10^{-4}$ | | | $^5F_2$ | 1304 | $7.04\times10^{-5}$ |
| | | $^5F_4$ | 672 | $1.73\times10^{-4}$ | | | $^5F_1$ | 1560 | $1.67\times10^{-4}$ |
| | | $^5F_3$ | 775 | $3.42\times10^{-4}$ | $\left(^5F,\,^5G\right)_2$ | 27879 | $^5I_4$ | 681 | $8.67\times10^{-4}$ |
| | | $^5F_2$ | 803 | $2.93\times10^{-5}$ | | | $^5S_2$ | 995 | $1.31\times10^{-5}$ |
| | | $^5F_1$ | 893 | $7.31\times10^{-5}$ | | | $^5F_4$ | 1015 | $9.77\times10^{-6}$ |
| | | $\left(^5G,\,^3G\right)_5$ | 1040 | $7.54\times10^{-5}$ | | | $^5F_3$ | 1270 | $1.77\times10^{-5}$ |
| | | $^5G_4$ | 1295 | $9.84\times10^{-6}$ | | | $^5F_2$ | 1345 | $2.73\times10^{-5}$ |
| | | $\left(^5G,\,^3H\right)_5$ | 1673 | $2.29\times10^{-6}$ | | | $^5F_1$ | 1618 | $1.76\times10^{-5}$ |
| $^5G_2$ | 30009 | $^5I_4$ | 595 | $3.41\times10^{-3}$ | $^3H_6$ | 27317 | $^5I_8$ | 366 | $1.1\times10^{-2}$ |
| | | $^5S_2$ | 821 | $2.7\times10^{-4}$ | | | $^5I_7$ | 449 | $7.26\times10^{-4}$ |
| | | $^5F_4$ | 835 | $4.99\times10^{-6}$ | | | $^5I_6$ | 531 | $1.59\times10^{-7}$ |
| | | $^5F_3$ | 1000 | $1.76\times10^{-5}$ | | | $^5I_5$ | 618 | $1.04\times10^{-5}$ |

[a] The emission rate, $A_{eq}$, inside a host material with refractive index $n_r$ would be: $A_{eq} = A'_{eq}\ n_r^5$

TABLE S23: Continued: $Ho^{3+}$ EQ spontaneous emission lines between 300 and 1700 nm.

| $SLJ$ | $E_{SLJ}(cm^{-1})$ | $S'L'J'$ | $\lambda$ (nm) | $A'_{eq}$ $(s^{-1})$ [a] | $SLJ$ | $E_{SLJ}(cm^{-1})$ | $S'L'J'$ | $\lambda$ (nm) | $A'_{eq}$ $(s^{-1})$ [a] |
|---|---|---|---|---|---|---|---|---|---|
| $^3H_6$ | 27317 | $^5I_4$ | 708 | $4.37 \times 10^{-7}$ | $(^5G,\,^3G)\ 5$ | 23286 | $^5I_7$ | 549 | $6.59 \times 10^{-3}$ |
| | | $^5F_5$ | 807 | $2.07 \times 10^{-4}$ | | | $^5I_6$ | 676 | $6.94 \times 10^{-4}$ |
| | | $^5F_4$ | 1077 | $8.33 \times 10^{-6}$ | | | $^5I_5$ | 823 | $6.68 \times 10^{-6}$ |
| | | $^3K_8$ | 1515 | $5.22 \times 10^{-6}$ | | | $^5I_4$ | 992 | $3.11 \times 10^{-8}$ |
| | | $^5G_6$ | 1663 | $2.18 \times 10^{-6}$ | | | $^5F_5$ | 1196 | $1.36 \times 10^{-4}$ |
| $(^5G,\,^3H)\ 5$ | 26922 | $^5I_7$ | 458 | $1.41 \times 10^{-2}$ | $^5G_6$ | 21306 | $^5I_8$ | 469 | $2.99 \times 10^{-2}$ |
| | | $^5I_6$ | 543 | $9.58 \times 10^{-4}$ | | | $^5I_7$ | 616 | $9.94 \times 10^{-4}$ |
| | | $^5I_5$ | 634 | $2.58 \times 10^{-5}$ | | | $^5I_6$ | 781 | $2.3 \times 10^{-5}$ |
| | | $^5I_4$ | 729 | $2.34 \times 10^{-5}$ | | | $^5I_5$ | 983 | $2.28 \times 10^{-5}$ |
| | | $^5F_5$ | 833 | $1.4 \times 10^{-4}$ | | | $^5I_4$ | 1234 | $2.67 \times 10^{-7}$ |
| | | $^5F_4$ | 1125 | $1.91 \times 10^{-4}$ | | | $^5F_5$ | 1566 | $1.31 \times 10^{-4}$ |
| | | $^5F_3$ | 1446 | $4.07 \times 10^{-5}$ | $^3K_8$ | 20715 | $^5I_8$ | 483 | $4.63 \times 10^{-4}$ |
| $^3K_7$ | 25636 | $^5I_8$ | 390 | $3.62 \times 10^{-4}$ | | | $^5I_7$ | 639 | $1.6 \times 10^{-5}$ |
| | | $^5I_7$ | 486 | $1.39 \times 10^{-4}$ | | | $^5I_6$ | 818 | $2.11 \times 10^{-5}$ |
| | | $^5I_6$ | 583 | $1.88 \times 10^{-5}$ | $^5F_2$ | 20444 | $^5I_4$ | 1381 | $1.41 \times 10^{-7}$ |
| | | $^5I_5$ | 690 | $5.84 \times 10^{-5}$ | $^5F_3$ | 20005 | $^5I_5$ | 1128 | $6.96 \times 10^{-8}$ |
| | | $^5F_5$ | 933 | $2.15 \times 10^{-6}$ | | | $^5I_4$ | 1470 | $9.92 \times 10^{-9}$ |
| $^5G_4$ | 25181 | $^5I_6$ | 599 | $5.08 \times 10^{-3}$ | $^5F_4$ | 18030 | $^5I_6$ | 1049 | $2.39 \times 10^{-7}$ |
| | | $^5I_5$ | 712 | $9.41 \times 10^{-4}$ | | | $^5I_5$ | 1451 | $1.75 \times 10^{-7}$ |
| | | $^5I_4$ | 835 | $4.28 \times 10^{-5}$ | $^5F_5$ | 14921 | $^5I_7$ | 1015 | $7.41 \times 10^{-6}$ |
| | | $^5F_5$ | 975 | $2.3 \times 10^{-5}$ | | | $^5I_6$ | 1556 | $7.71 \times 10^{-7}$ |
| | | $^5S_2$ | 1359 | $2.08 \times 10^{-5}$ | $^5I_5$ | 11137 | $^5I_7$ | 1647 | $1.14 \times 10^{-7}$ |
| | | $^5F_4$ | 1398 | $8.64 \times 10^{-5}$ | $^5I_6$ | 8495 | $^5I_8$ | 1177 | $1.92 \times 10^{-6}$ |

[a] The emission rate, $A_{eq}$, inside a host material with refractive index $n_r$ would be: $A_{eq} = A'_{eq}\ n_r^5$

TABLE S24: Calculated $Er^{3+}$ EQ spontaneous emission lines between 300 and 1700 nm.

| $SLJ$ | $E_{SLJ}(cm^{-1})$ | $S'L'J'$ | $\lambda$ (nm) | $A'_{eq}$ $(s^{-1})$ [a] | $SLJ$ | $E_{SLJ}(cm^{-1})$ | $S'L'J'$ | $\lambda$ (nm) | $A'_{eq}$ $(s^{-1})$ [a] |
|---|---|---|---|---|---|---|---|---|---|
| $^4D_{7/2}$ | 37455 | $^4I_{11/2}$ | 366 | $9.15\times10^{-4}$ | $^4G_{7/2}$ | 32919 | $^4I_{11/2}$ | 440 | $1.46\times10^{-2}$ |
| | | $(^4I,\,^2H)_{9/2}$ | 394 | $9.65\times10^{-3}$ | | | $(^4I,\,^2H)_{9/2}$ | 479 | $5.76\times10^{-4}$ |
| | | $^4F_{9/2}$ | 440 | $1.34\times10^{-2}$ | | | $^4F_{9/2}$ | 550 | $3.82\times10^{-8}$ |
| | | $^4S_{3/2}$ | 506 | $4.5\times10^{-2}$ | | | $^4S_{3/2}$ | 657 | $3.19\times10^{-4}$ |
| | | $(^2H,\,^4G)_{11/2}$ | 529 | $8.63\times10^{-3}$ | | | $(^2H,\,^4G)_{11/2}$ | 696 | $1.6\times10^{-4}$ |
| | | $^4F_{7/2}$ | 566 | $4.71\times10^{-3}$ | | | $^4F_{7/2}$ | 761 | $5.5\times10^{-4}$ |
| | | $^4F_{5/2}$ | 628 | $7.78\times10^{-4}$ | | | $^4F_{5/2}$ | 878 | $7.12\times10^{-4}$ |
| | | $^4F_{3/2}$ | 638 | $2.44\times10^{-3}$ | | | $^4F_{3/2}$ | 897 | $2.83\times10^{-4}$ |
| | | $(^2G,\,^4F)_{9/2}$ | 733 | $6.46\times10^{-4}$ | | | $(^2G,\,^4F)_{9/2}$ | 1098 | $4.38\times10^{-5}$ |
| | | $^4G_{11/2}$ | 833 | $5.09\times10^{-4}$ | | | $^4G_{11/2}$ | 1339 | $4.41\times10^{-7}$ |
| | | $^4G_{9/2}$ | 904 | $2.32\times10^{-4}$ | | | $^4G_{9/2}$ | 1533 | $8.19\times10^{-8}$ |
| | | $(^2G,\,^4G)_{7/2}$ | 960 | $1.99\times10^{-5}$ | $^2P_{1/2}$ | 32649 | $^4S_{3/2}$ | 668 | $5.21\times10^{-5}$ |
| | | $(^2P,\,^2D)_{3/2}$ | 1498 | $3.09\times10^{-5}$ | | | $^4F_{5/2}$ | 899 | $8.7\times10^{-6}$ |
| $^2D_{5/2}$ | 36928 | $(^4I,\,^2H)_{9/2}$ | 402 | $3.27\times10^{-3}$ | | | $^4F_{3/2}$ | 920 | $6.93\times10^{-5}$ |
| | | $^4F_{9/2}$ | 451 | $5.8\times10^{-3}$ | $^2K_{13/2}$ | 32597 | $^4I_{15/2}$ | 307 | $5.45\times10^{-4}$ |
| | | $^4S_{3/2}$ | 520 | $1.72\times10^{-2}$ | | | $^4I_{13/2}$ | 384 | $3.84\times10^{-4}$ |
| | | $^4F_{7/2}$ | 583 | $1.05\times10^{-3}$ | | | $^4I_{11/2}$ | 446 | $9.73\times10^{-5}$ |
| | | $^4F_{5/2}$ | 649 | $1.89\times10^{-3}$ | | | $(^4I,\,^2H)_{9/2}$ | 487 | $1.31\times10^{-3}$ |
| | | $^4F_{3/2}$ | 660 | $3.26\times10^{-3}$ | | | $^4F_{9/2}$ | 560 | $4.45\times10^{-5}$ |
| | | $(^2G,\,^4F)_{9/2}$ | 763 | $2.71\times10^{-4}$ | | | $(^2H,\,^4G)_{11/2}$ | 712 | $2.75\times10^{-5}$ |
| | | $^4G_{9/2}$ | 949 | $1.04\times10^{-4}$ | | | $(^2G,\,^4F)_{9/2}$ | 1139 | $1.48\times10^{-5}$ |
| | | $(^2G,\,^4G)_{7/2}$ | 1011 | $1.67\times10^{-4}$ | | | $^4G_{11/2}$ | 1399 | $4.38\times10^{-6}$ |
| | | $(^2P,\,^2D)_{3/2}$ | 1627 | $2.28\times10^{-5}$ | | | $^4G_{9/2}$ | 1612 | $6.35\times10^{-7}$ |
| $(^2H,\,^2G)_{9/2}$ | 35679 | $^4I_{13/2}$ | 343 | $1.19\times10^{-2}$ | $^4G_{5/2}$ | 32171 | $(^4I,\,^2H)_{9/2}$ | 497 | $9.08\times10^{-3}$ |
| | | $^4I_{11/2}$ | 392 | $4.56\times10^{-4}$ | | | $^4F_{9/2}$ | 574 | $2.65\times10^{-3}$ |
| | | $(^4I,\,^2H)_{9/2}$ | 423 | $3.07\times10^{-4}$ | | | $^4S_{3/2}$ | 691 | $8.26\times10^{-4}$ |
| | | $^4F_{9/2}$ | 477 | $1.22\times10^{-4}$ | | | $^4F_{7/2}$ | 807 | $8.98\times10^{-5}$ |
| | | $(^2H,\,^4G)_{11/2}$ | 584 | $9.38\times10^{-5}$ | | | $^4F_{5/2}$ | 940 | $6.44\times10^{-4}$ |
| | | $^4F_{7/2}$ | 629 | $5.55\times10^{-4}$ | | | $^4F_{3/2}$ | 962 | $1.31\times10^{-3}$ |
| | | $^4F_{5/2}$ | 707 | $1.59\times10^{-4}$ | | | $(^2G,\,^4F)_{9/2}$ | 1197 | $5.34\times10^{-6}$ |
| | | $(^2G,\,^4F)_{9/2}$ | 843 | $1.6\times10^{-4}$ | $(^2P,\,^2D)_{3/2}$ | 30781 | $^4S_{3/2}$ | 764 | $7.59\times10^{-4}$ |
| | | $^4G_{11/2}$ | 978 | $5.05\times10^{-5}$ | | | $^4F_{7/2}$ | 909 | $2.48\times10^{-5}$ |
| | | $^4G_{9/2}$ | 1077 | $3.31\times10^{-6}$ | | | $^4F_{5/2}$ | 1081 | $1.34\times10^{-5}$ |
| | | $(^2G,\,^4G)_{7/2}$ | 1157 | $3.42\times10^{-6}$ | | | $^4F_{3/2}$ | 1111 | $1.96\times10^{-5}$ |
| $^2D_{5/2}$ | 34353 | $(^4I,\,^2H)_{9/2}$ | 448 | $8.68\times10^{-4}$ | $^2K_{15/2}$ | 27315 | $^4I_{15/2}$ | 366 | $1.85\times10^{-3}$ |
| | | $^4F_{9/2}$ | 510 | $8.57\times10^{-4}$ | | | $^4I_{13/2}$ | 481 | $8.32\times10^{-8}$ |
| | | $^4S_{3/2}$ | 600 | $2.82\times10^{-3}$ | | | $^4I_{11/2}$ | 583 | $5.91\times10^{-4}$ |
| | | $^4F_{7/2}$ | 686 | $1.39\times10^{-4}$ | | | $(^2H,\,^4G)_{11/2}$ | 1142 | $3.89\times10^{-5}$ |
| | | $^4F_{5/2}$ | 780 | $3.69\times10^{-4}$ | $(^2G,\,^4G)_{7/2}$ | 27038 | $^4I_{11/2}$ | 593 | $3.57\times10^{-3}$ |
| | | $^4F_{3/2}$ | 795 | $3.56\times10^{-4}$ | | | $(^4I,\,^2H)_{9/2}$ | 667 | $8.78\times10^{-4}$ |
| | | $(^2G,\,^4F)_{9/2}$ | 949 | $2.97\times10^{-5}$ | | | $^4F_{9/2}$ | 813 | $4.83\times10^{-6}$ |
| | | $^4G_{9/2}$ | 1256 | $4.37\times10^{-5}$ | | | $^4S_{3/2}$ | 1070 | $1.56\times10^{-4}$ |
| | | $(^2G,\,^4G)_{7/2}$ | 1367 | $1.3\times10^{-5}$ | | | $(^2H,\,^4G)_{11/2}$ | 1179 | $2.67\times10^{-7}$ |

[a] The emission rate, $A_{eq}$, inside a host material with refractive index $n_r$ would be: $A_{eq} = A'_{eq}\ n_r^5$

TABLE S24: Continued: $Er^{3+}$ EQ spontaneous emission lines between 300 and 1700 nm.

| $SLJ$ | $E_{SLJ}(cm^{-1})$ | $S'L'J'$ | $\lambda$ (nm) | $A'_{eq}$ $(s^{-1})$ [a] | $SLJ$ | $E_{SLJ}(cm^{-1})$ | $S'L'J'$ | $\lambda$ (nm) | $A'_{eq}$ $(s^{-1})$ [a] |
|---|---|---|---|---|---|---|---|---|---|
| $(^2G, ^4G)_{7/2}$ | 27038 | $^4F_{7/2}$ | 1378 | $2.84 \times 10^{-5}$ | $(^2G, ^4F)_{9/2}$ | 23816 | $^4I_{11/2}$ | 733 | $1.27 \times 10^{-4}$ |
| $^4G_{9/2}$ | 26394 | $^4I_{13/2}$ | 504 | $1.49 \times 10^{-2}$ | | | $(^4I, ^2H)_{9/2}$ | 850 | $3.06 \times 10^{-5}$ |
| | | $^4I_{11/2}$ | 616 | $5.82 \times 10^{-4}$ | | | $^4F_{9/2}$ | 1101 | $2.29 \times 10^{-6}$ |
| | | $(^4I, ^2H)_{9/2}$ | 697 | $6.06 \times 10^{-5}$ | $^4F_{5/2}$ | 21527 | $(^4I, ^2H)_{9/2}$ | 1055 | $3.61 \times 10^{-6}$ |
| | | $^4F_{9/2}$ | 858 | $4.12 \times 10^{-4}$ | | | $^4F_{9/2}$ | 1472 | $7.21 \times 10^{-9}$ |
| | | $(^2H, ^4G)_{11/2}$ | 1276 | $3.97 \times 10^{-6}$ | $^4F_{7/2}$ | 19779 | $^4I_{11/2}$ | 1040 | $1.15 \times 10^{-6}$ |
| | | $^4F_{7/2}$ | 1512 | $1.03 \times 10^{-4}$ | | | $(^4I, ^2H)_{9/2}$ | 1294 | $3.92 \times 10^{-6}$ |
| $^4G_{11/2}$ | 25449 | $^4I_{15/2}$ | 393 | $3.66 \times 10^{-2}$ | $(^2H, ^4G)_{11/2}$ | 18558 | $^4I_{15/2}$ | 539 | $7.28 \times 10^{-3}$ |
| | | $^4I_{13/2}$ | 529 | $1.18 \times 10^{-3}$ | | | $^4I_{13/2}$ | 832 | $3.96 \times 10^{-5}$ |
| | | $^4I_{11/2}$ | 654 | $4.73 \times 10^{-6}$ | | | $^4I_{11/2}$ | 1192 | $1.14 \times 10^{-5}$ |
| | | $(^4I, ^2H)_{9/2}$ | 747 | $3.98 \times 10^{-4}$ | | | $(^4I, ^2H)_{9/2}$ | 1537 | $3.42 \times 10^{-5}$ |
| | | $^4F_{9/2}$ | 933 | $5.33 \times 10^{-4}$ | $^4F_{9/2}$ | 14735 | $^4I_{13/2}$ | 1221 | $1.76 \times 10^{-6}$ |
| | | $(^2H, ^4G)_{11/2}$ | 1451 | $1.81 \times 10^{-8}$ | $^4I_{11/2}$ | 10167 | $^4I_{15/2}$ | 984 | $1.47 \times 10^{-5}$ |
| $(^2G, ^4F)_{9/2}$ | 23816 | $^4I_{13/2}$ | 579 | $7.45 \times 10^{-4}$ | $^4I_{13/2}$ | 6543 | $^4I_{15/2}$ | 1528 | $1.16 \times 10^{-6}$ |

[a] The emission rate, $A_{eq}$, inside a host material with refractive index $n_r$ would be: $A_{eq} = A'_{eq}\ n_r^5$

TABLE S25: Calculated $Tm^{3+}$ EQ spontaneous emission lines between 300 and 1700 nm.

| $SLJ$ | $E_{SLJ}(cm^{-1})$ | $S'L'J'$ | $\lambda$ (nm) | $A'_{eq}$ $(s^{-1})$ [a] | $SLJ$ | $E_{SLJ}(cm^{-1})$ | $S'L'J'$ | $\lambda$ (nm) | $A'_{eq}$ $(s^{-1})$ [a] |
|---|---|---|---|---|---|---|---|---|---|
| $(^3P, ^1D)_2$ | 37218 | $^3F_4$ | 313 | $1.5 \times 10^{-2}$ | $(^3P, ^1D)_2$ | 27046 | $^3H_4$ | 683 | $4.79 \times 10^{-4}$ |
| | | $^3H_4$ | 403 | $1.19 \times 10^{-2}$ | | | $^3F_3$ | 765 | $5.93 \times 10^{-4}$ |
| | | $^3F_3$ | 430 | $6.5 \times 10^{-3}$ | | | $^3F_2$ | 808 | $3.11 \times 10^{-4}$ |
| | | $^3F_2$ | 443 | $2.17 \times 10^{-4}$ | | | $^1G_4$ | 1644 | $5.71 \times 10^{-6}$ |
| | | $^1G_4$ | 615 | $3.62 \times 10^{-3}$ | $^1G_4$ | 20962 | $^3H_6$ | 477 | $7.70 \times 10^{-4}$ |
| | | $(^3P, ^1D)_2$ | 983 | $2.36 \times 10^{-8}$ | | | $^3F_4$ | 639 | $3.19 \times 10^{-5}$ |
| $^3P_1$ | 34665 | $^3F_3$ | 483 | $1.07 \times 10^{-2}$ | | | $^3H_5$ | 784 | $1.48 \times 10^{-4}$ |
| | | $^3F_2$ | 500 | $4.17 \times 10^{-3}$ | | | $^3H_4$ | 1167 | $6.46 \times 10^{-5}$ |
| | | $(^3P, ^1D)_2$ | 1312 | $1.23 \times 10^{-4}$ | | | $^3F_3$ | 1431 | $2.72 \times 10^{-6}$ |
| $^1I_6$ | 34212 | $^3F_4$ | 346 | $1.5 \times 10^{-2}$ | | $^3F_2$ | | 1587 | $2.64 \times 10^{-6}$ |
| | | $^3H_5$ | 385 | $9.88 \times 10^{-5}$ | $^3F_2$ | 14662 | $^3F_4$ | 1070 | $1.04 \times 10^{-4}$ |
| | | $^3H_4$ | 458 | $4.61 \times 10^{-3}$ | $^3F_3$ | 13973 | $^3F_4$ | 1155 | $1.04 \times 10^{-6}$ |
| | | $^1G_4$ | 755 | $1.12 \times 10^{-3}$ | $^3H_4$ | 12394 | $^3F_4$ | 807 | $2.82 \times 10^{-4}$ |
| $^3P_0$ | 33721 | $^3F_2$ | 525 | $2.95 \times 10^{-3}$ | | | $^3H_6$ | 1412 | $1.92 \times 10^{-5}$ |
| | | $(^3P, ^1D)_2$ | 1498 | $1.72 \times 10^{-6}$ | $^3H_5$ | 8205 | $^3H_6$ | 1219 | $2.09 \times 10^{-5}$ |
| $(^3P, ^1D)_2$ | 27046 | $^3F_4$ | 460 | $1.5 \times 10^{-2}$ | | | | | |

[a] The emission rate, $A_{eq}$, inside a host material with refractive index $n_r$ would be: $A_{eq} = A'_{eq}\ n_r^5$

TABLE S26: Calculated $Yb^{3+}$ EQ spontaneous emission lines between 300 and 1700 nm.

| $SLJ$ | $E_{SLJ}(cm^{-1})$ | $S'L'J'$ | $\lambda$ (nm) | $A'_{eq}$ $(s^{-1})$ [a] | $SLJ$ | $E_{SLJ}(cm^{-1})$ | $S'L'J'$ | $\lambda$ (nm) | $A'_{eq}$ $(s^{-1})$ [a] |
|---|---|---|---|---|---|---|---|---|---|
| $^2F_{5/2}$ | 10248 | $^2F_{7/2}$ | 976 | $9.76 \times 10^{-5}$ | | | | | |

[a] The emission rate, $A_{eq}$, inside a host material with refractive index $n_r$ would be: $A_{eq} = A'_{eq}\ n_r^5$
